# Supplementary material for: Identification in Tree-shaped Linear Structural Causal Models
Source: arXiv:2203.01852 ancillary file (2022-03-04)

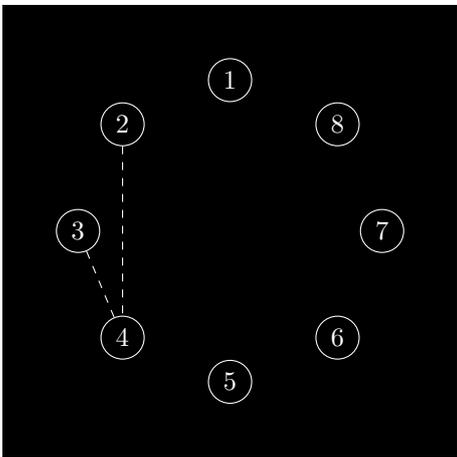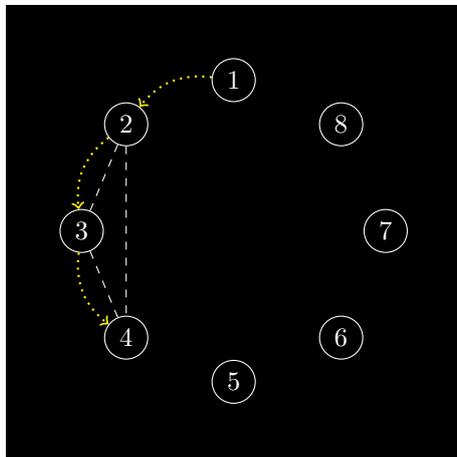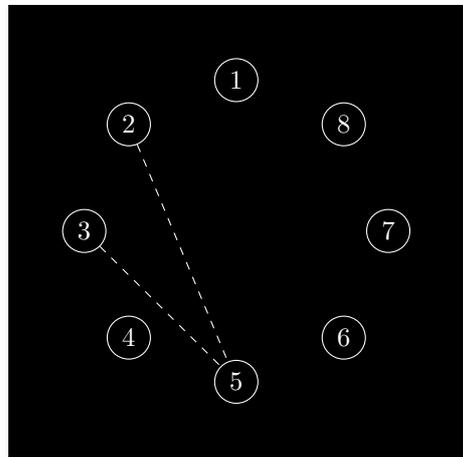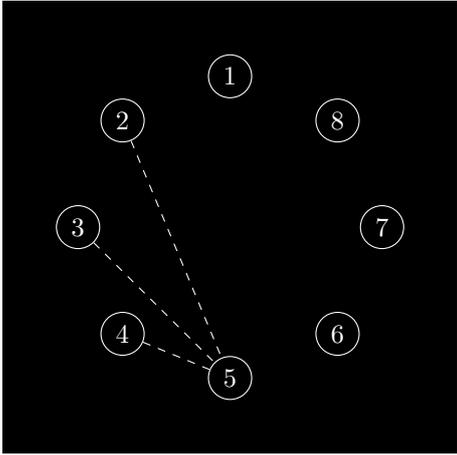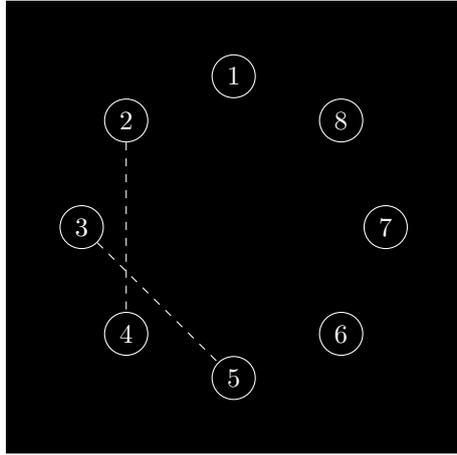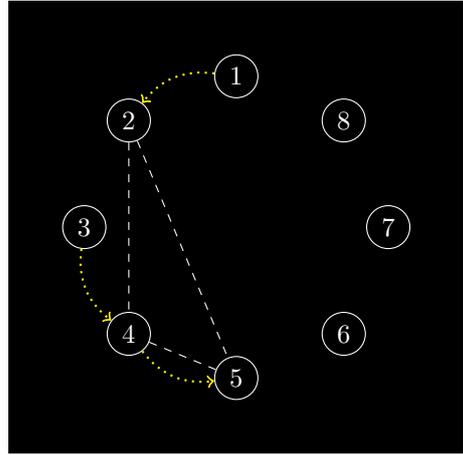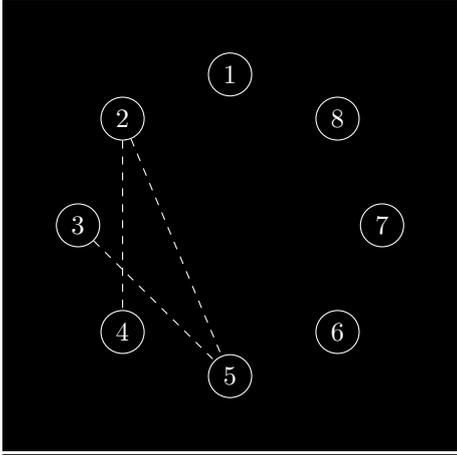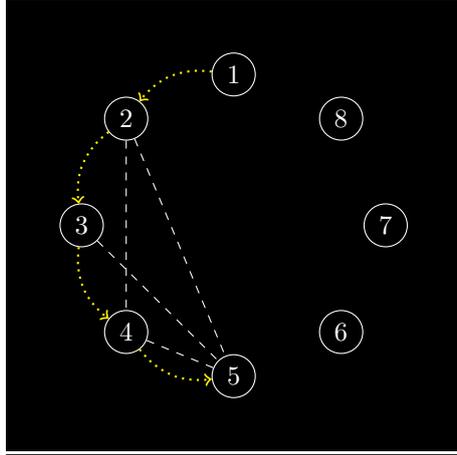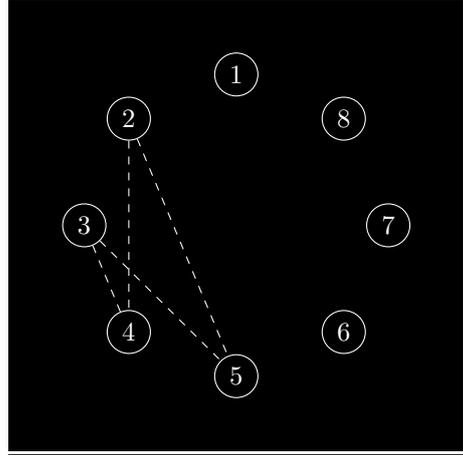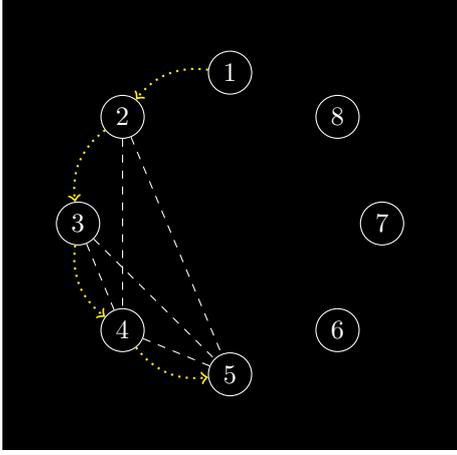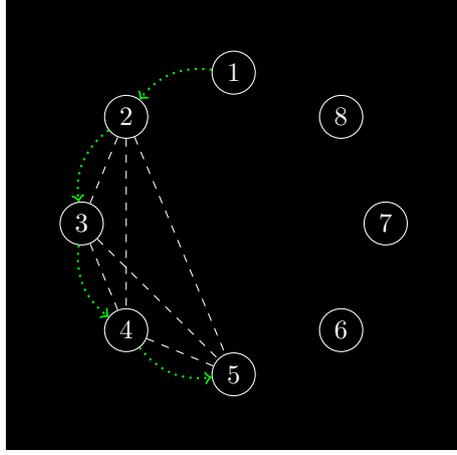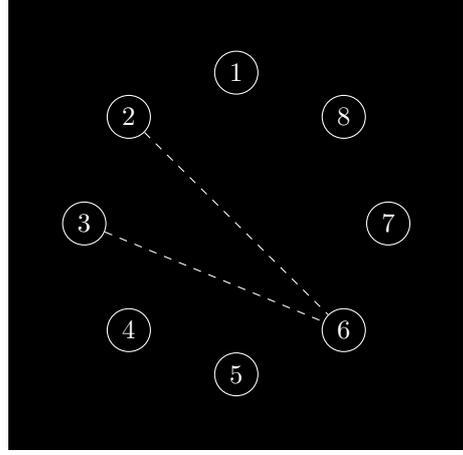

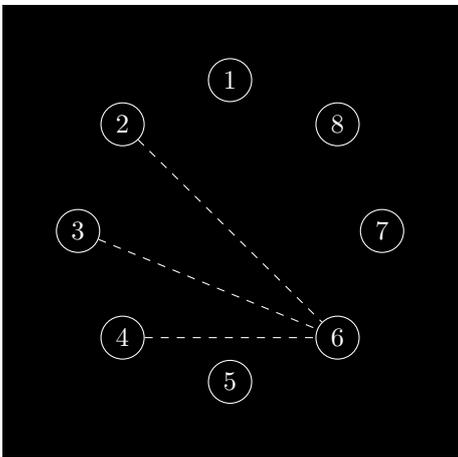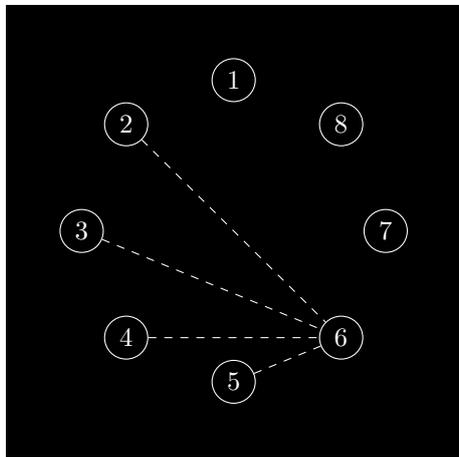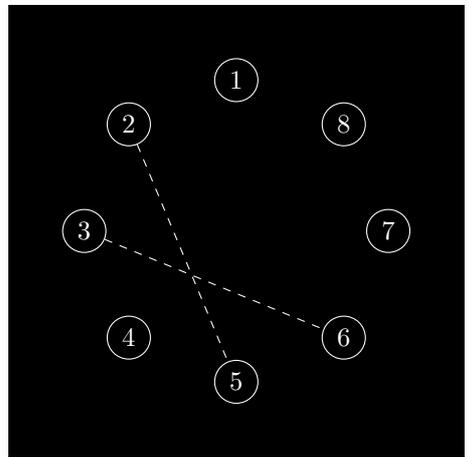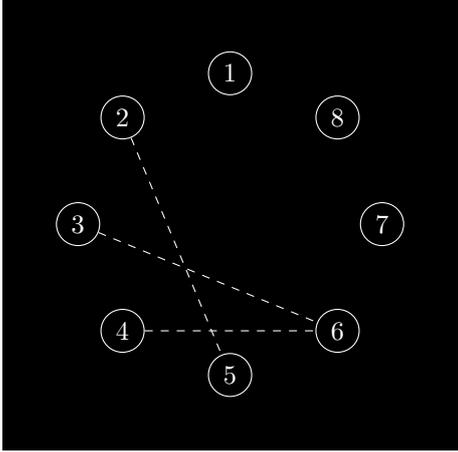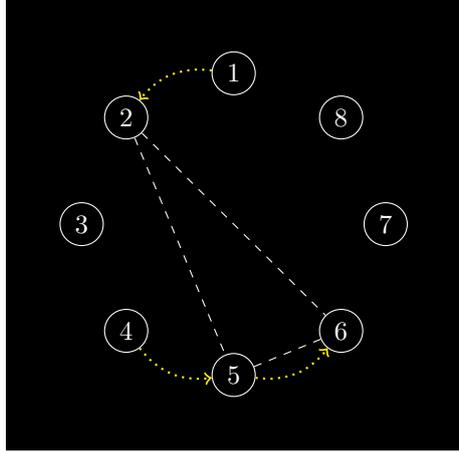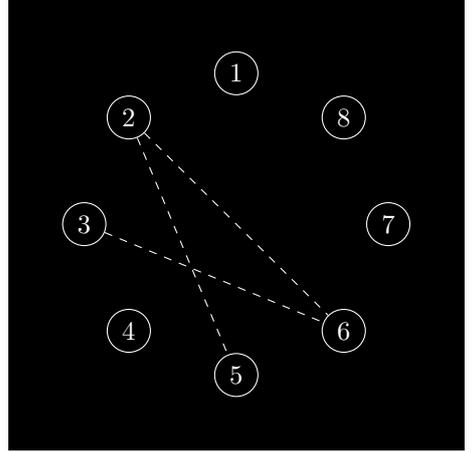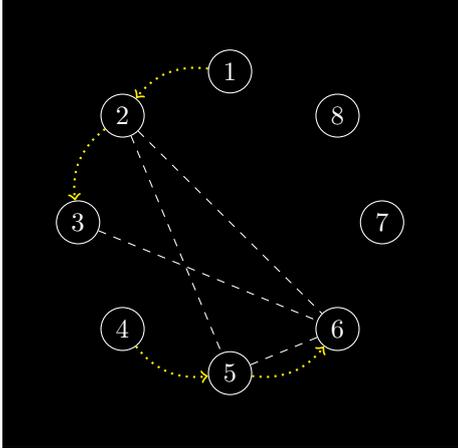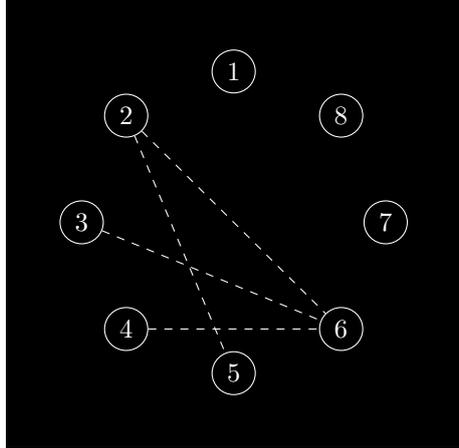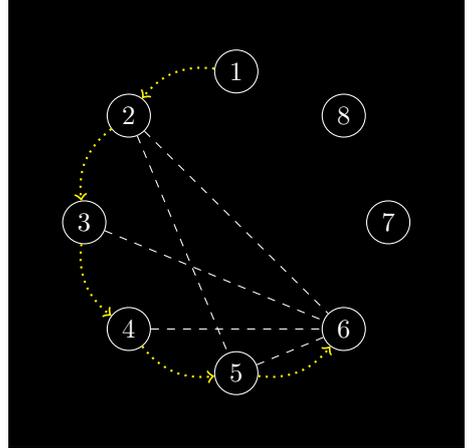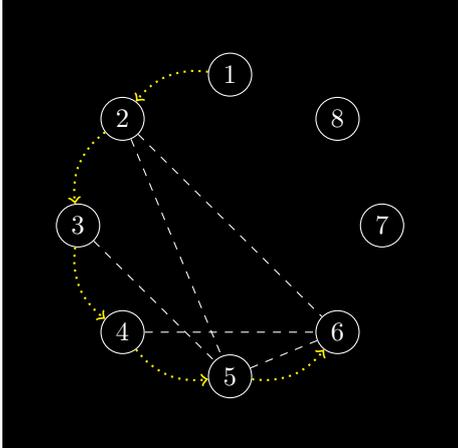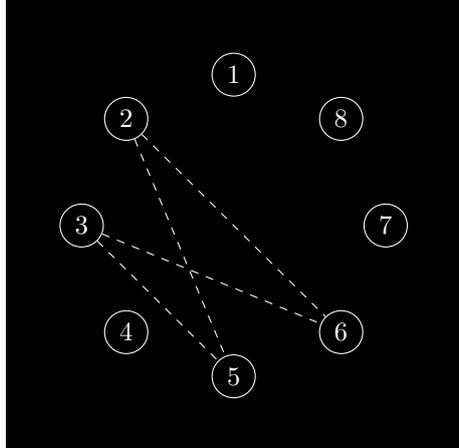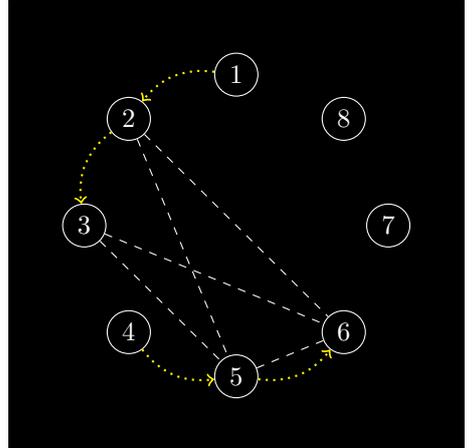

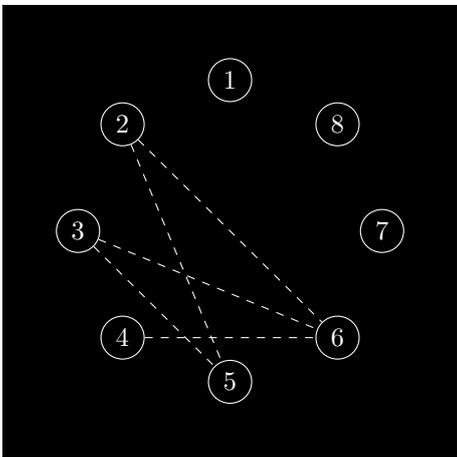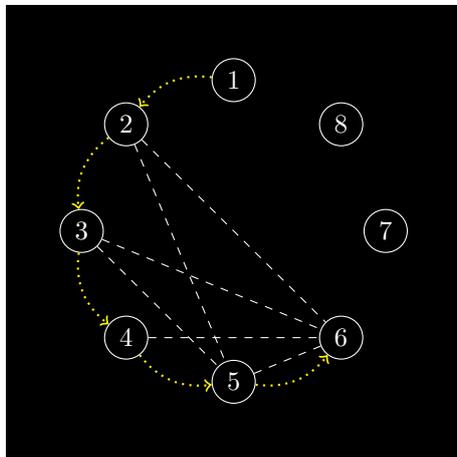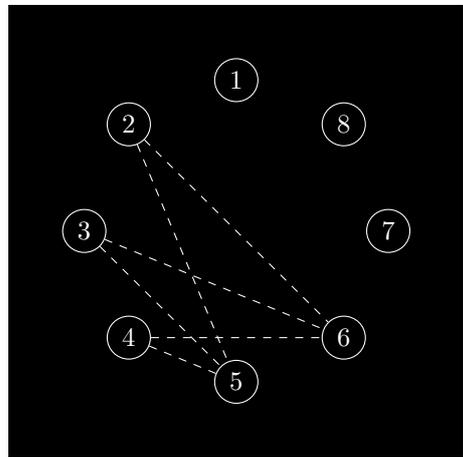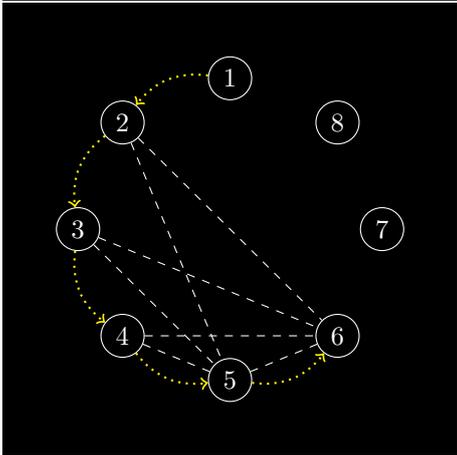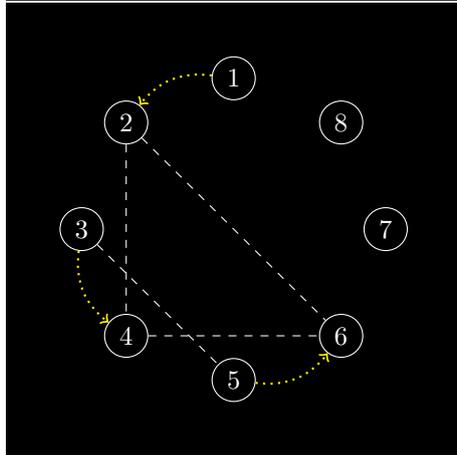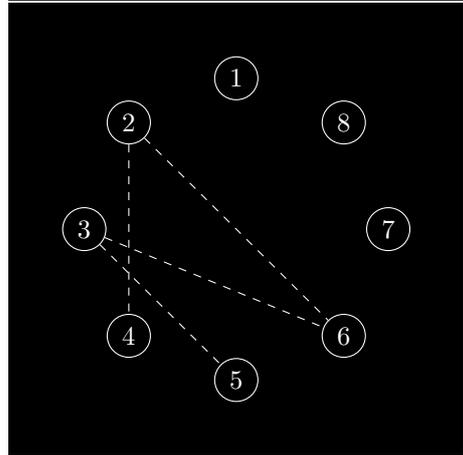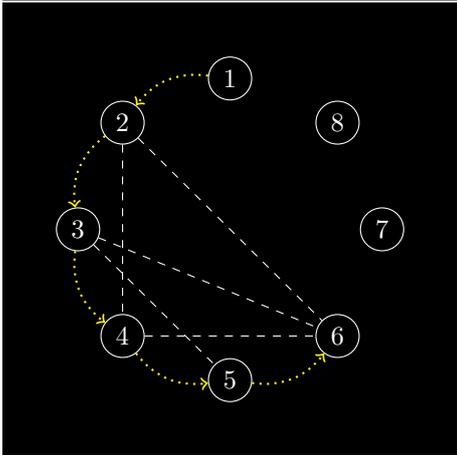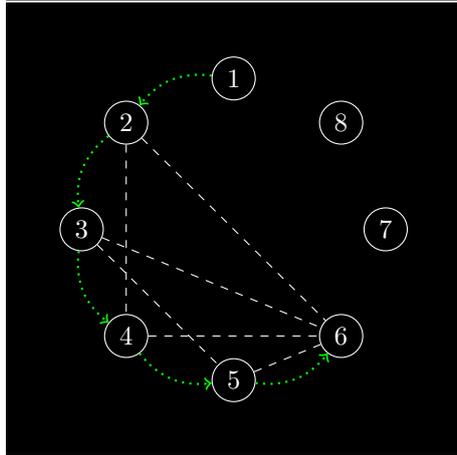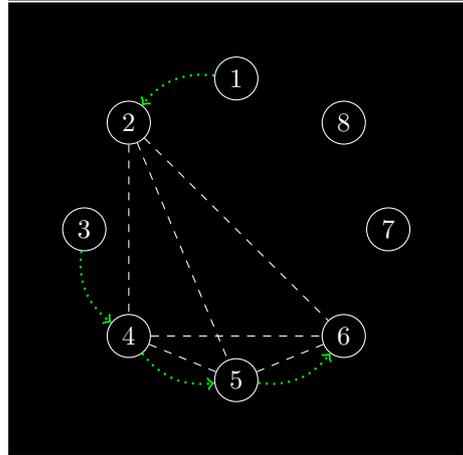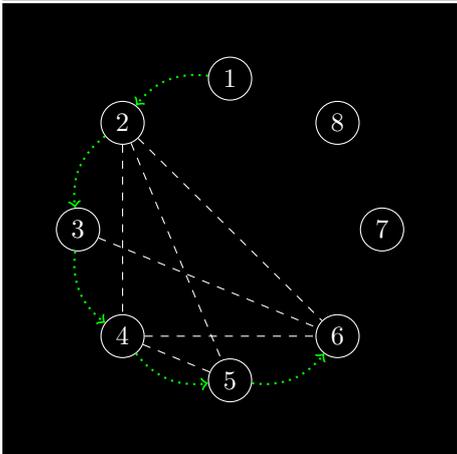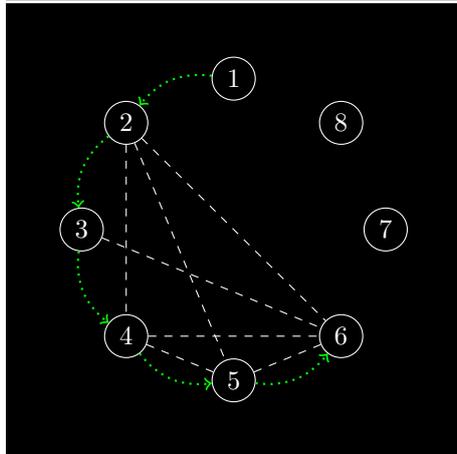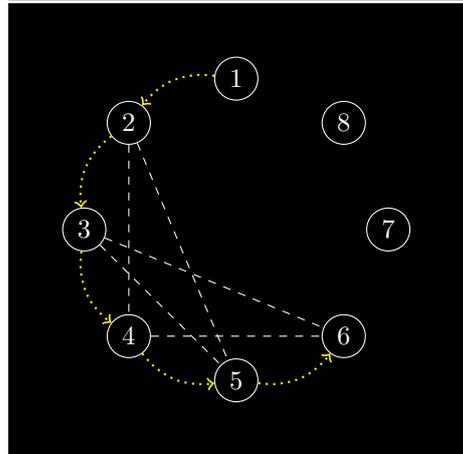

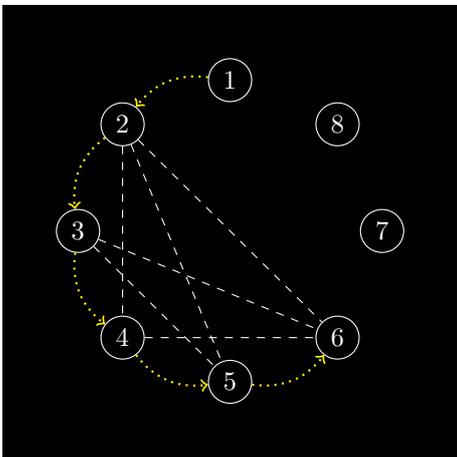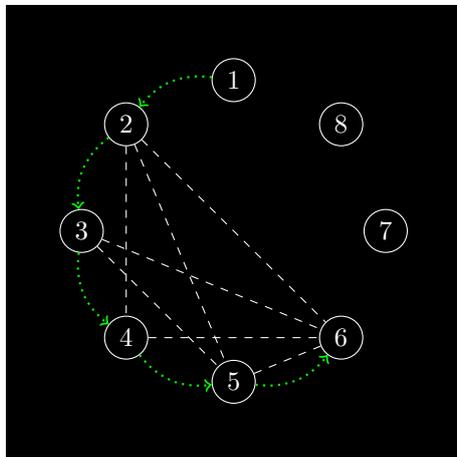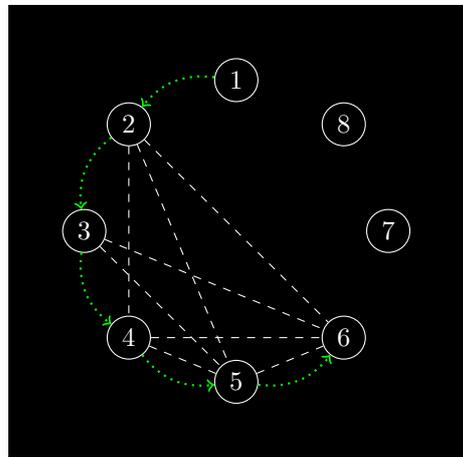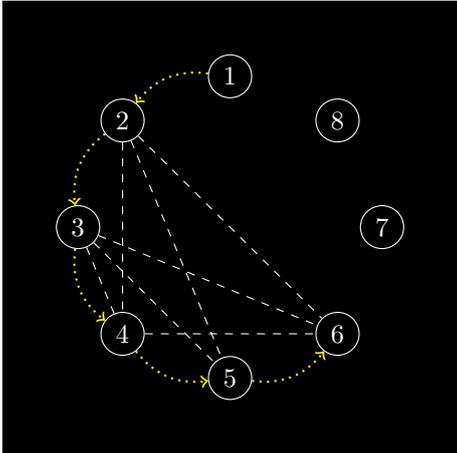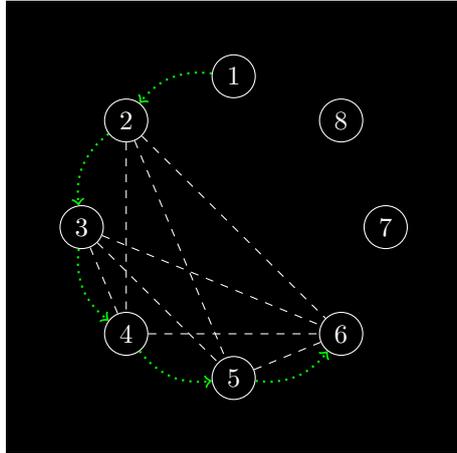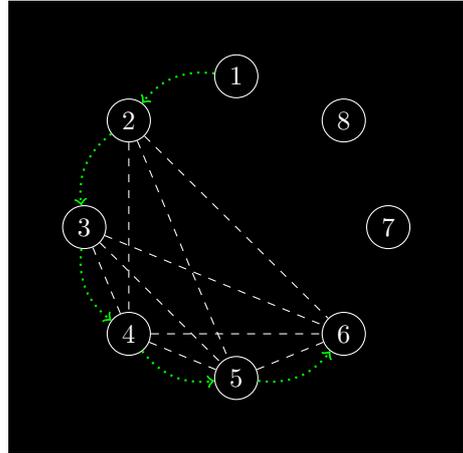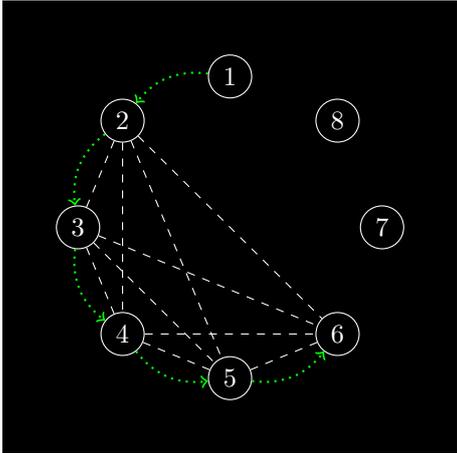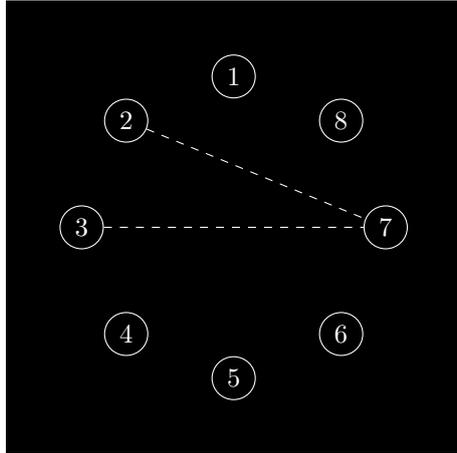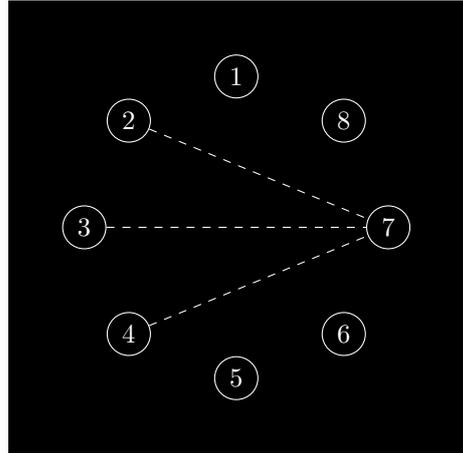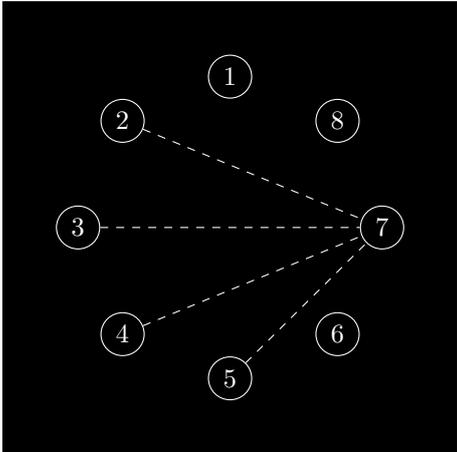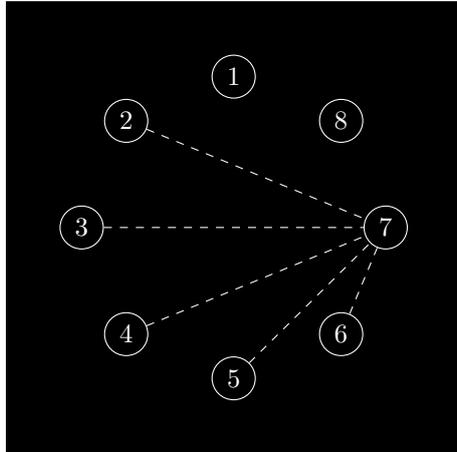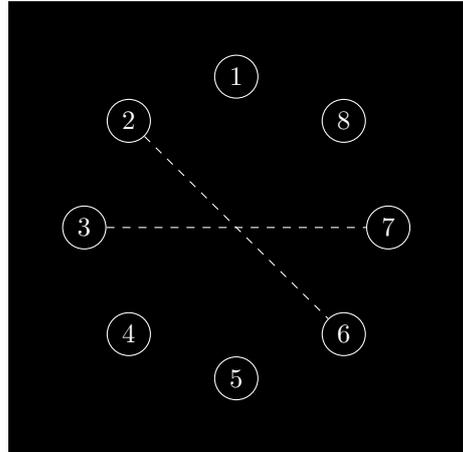

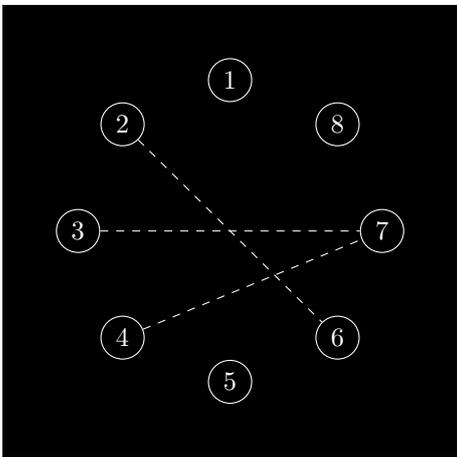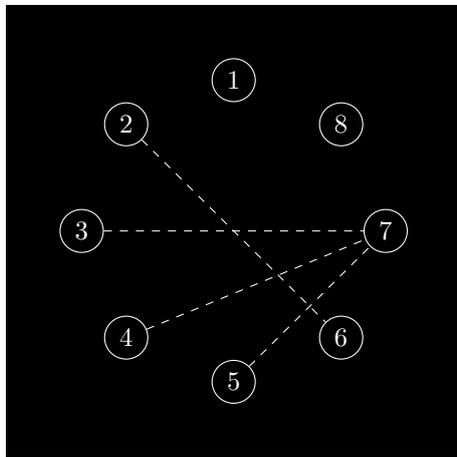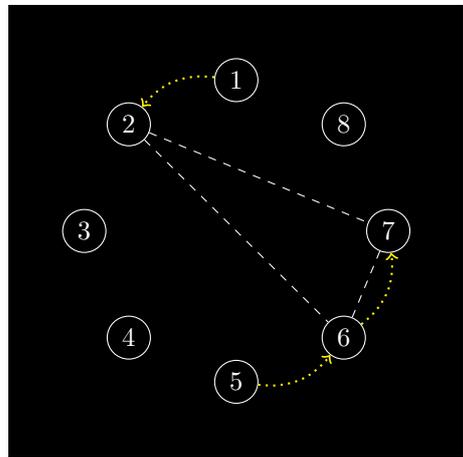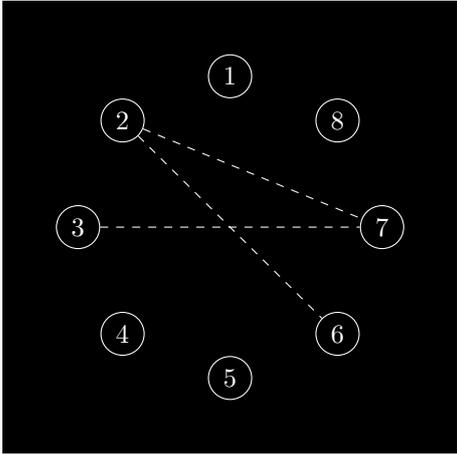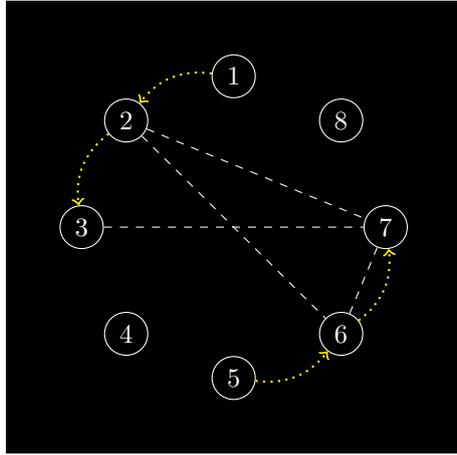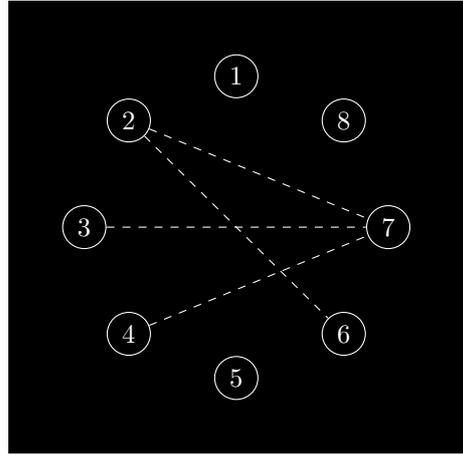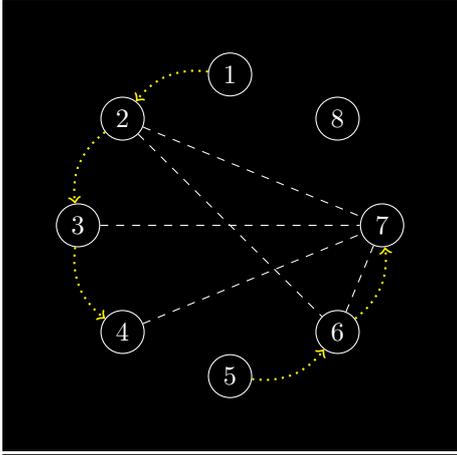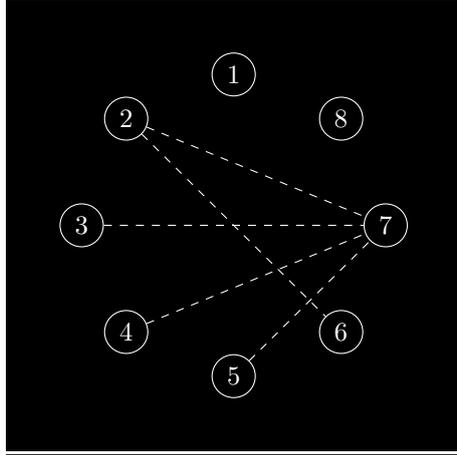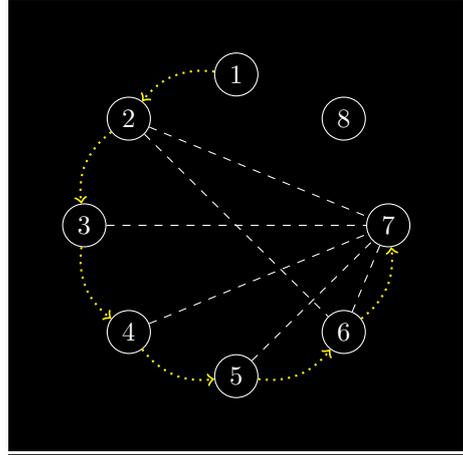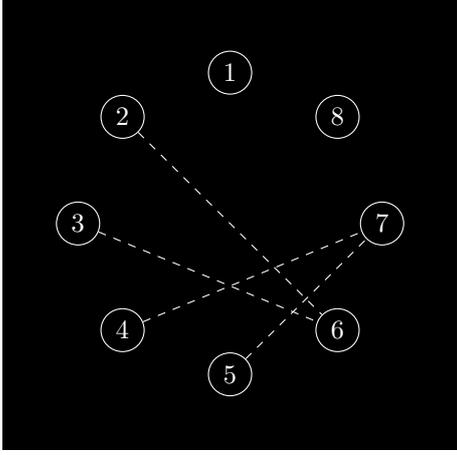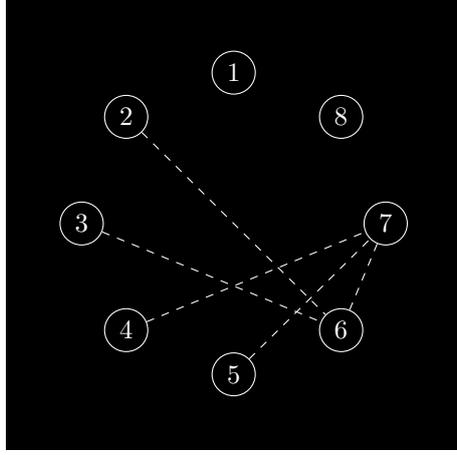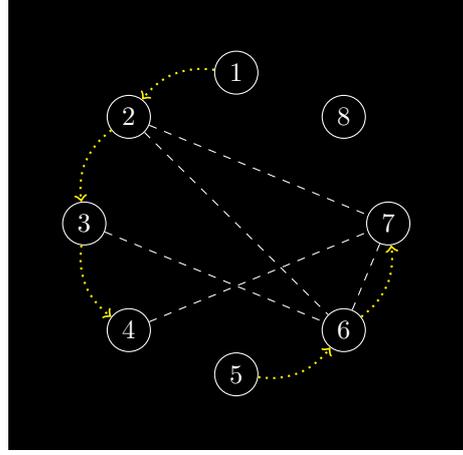

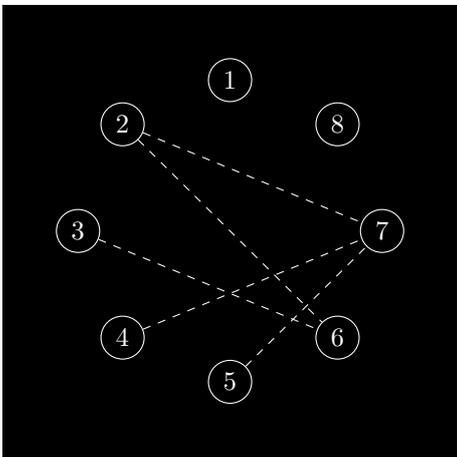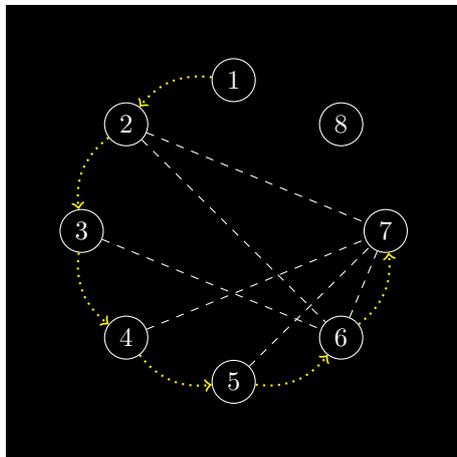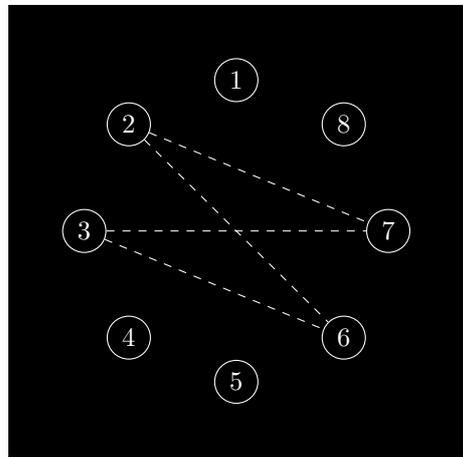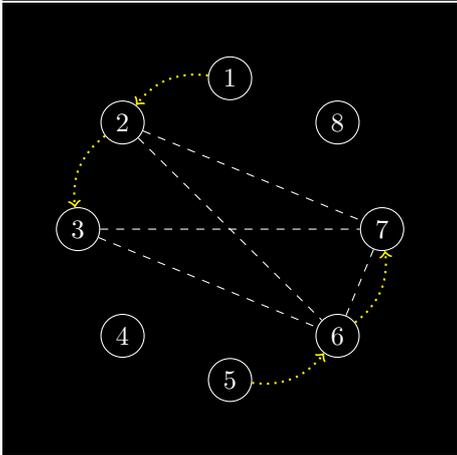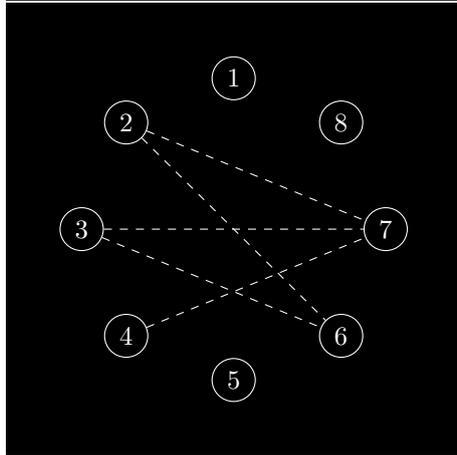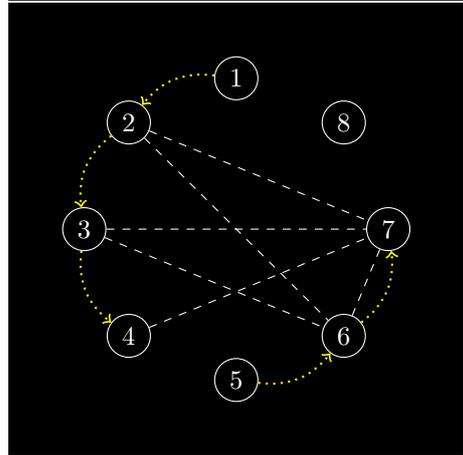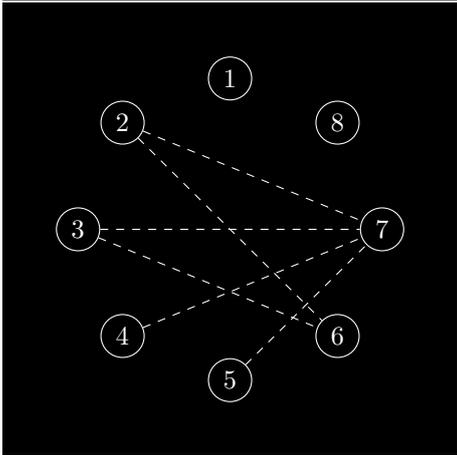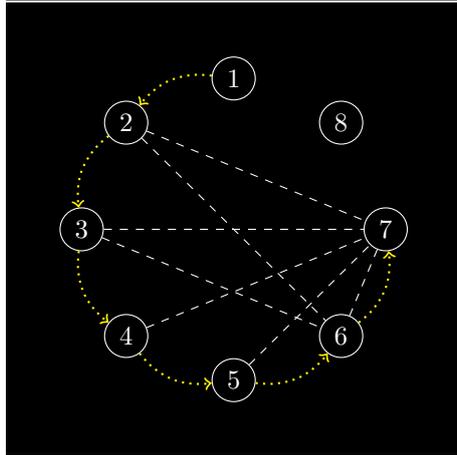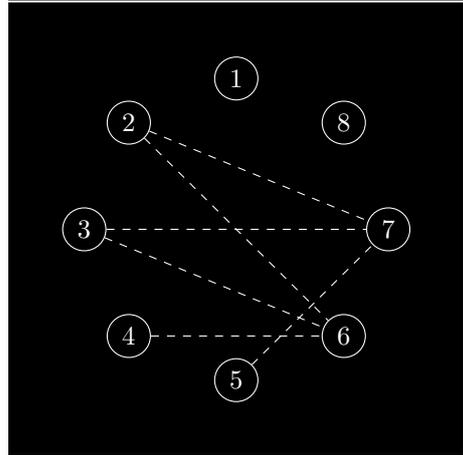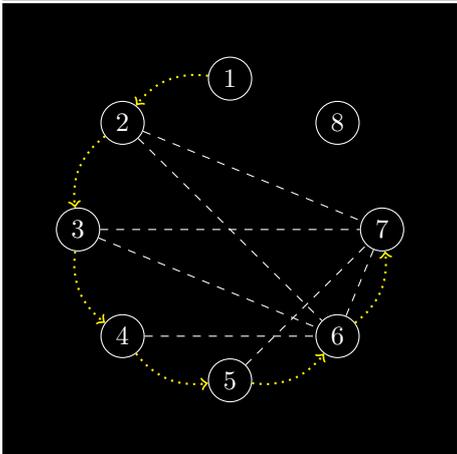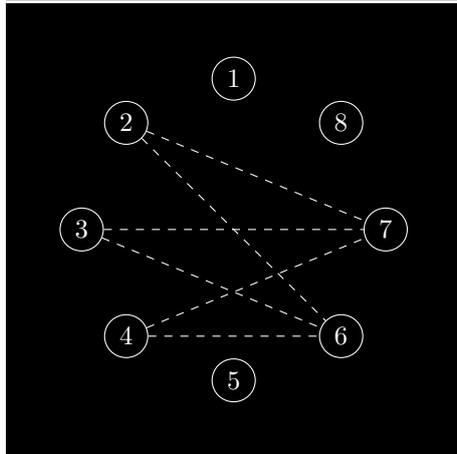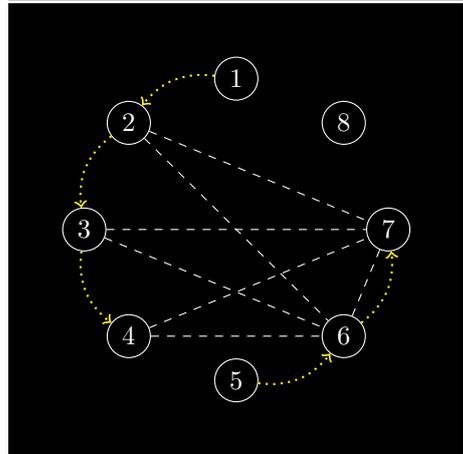

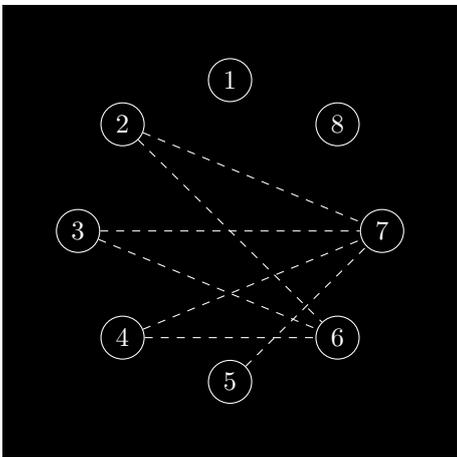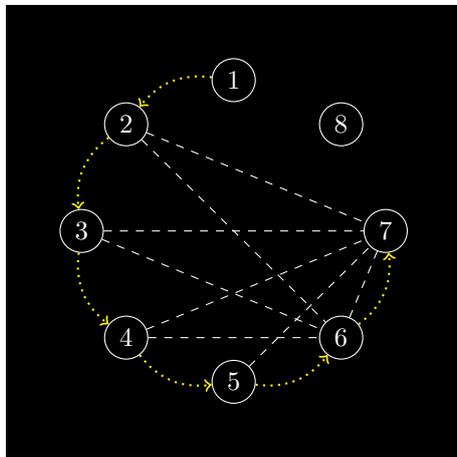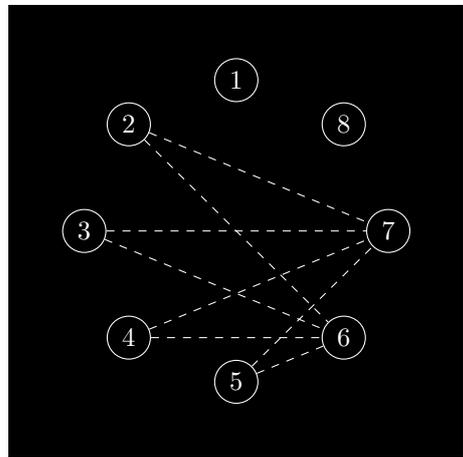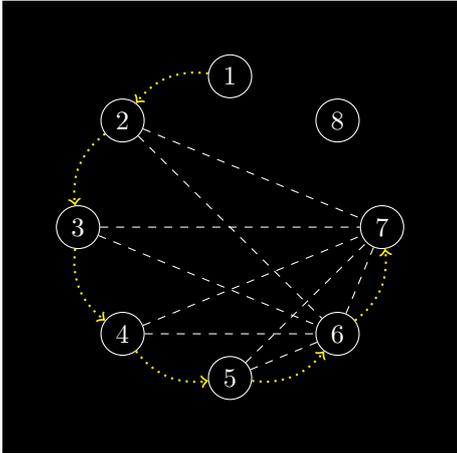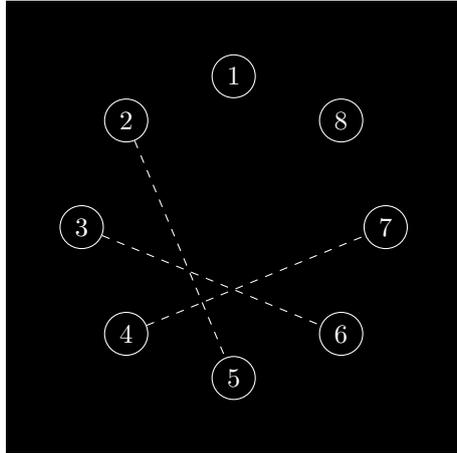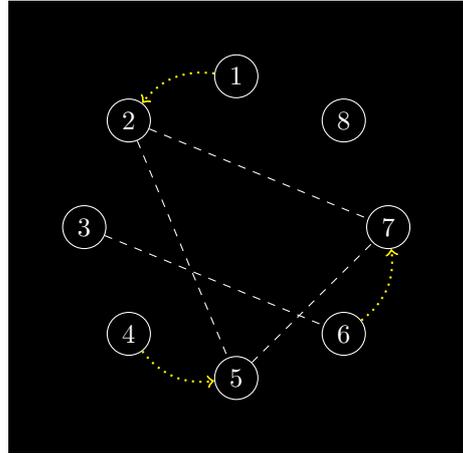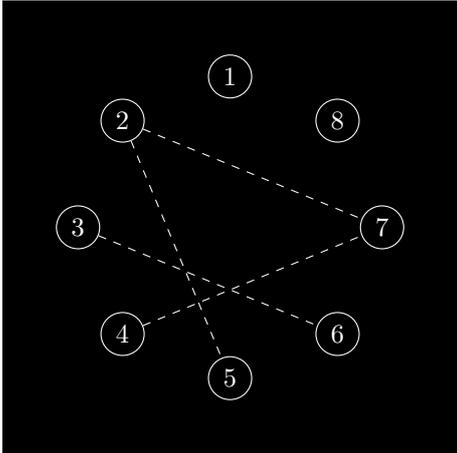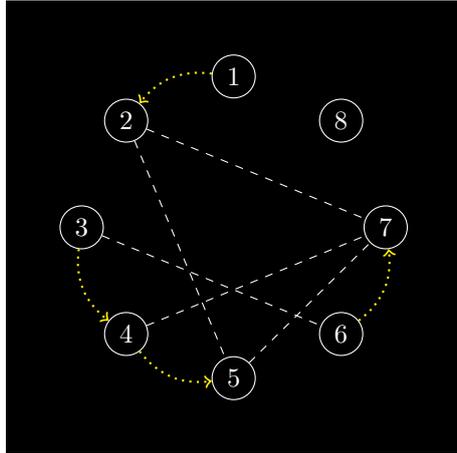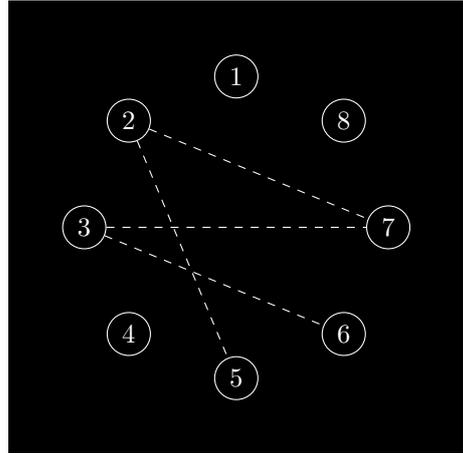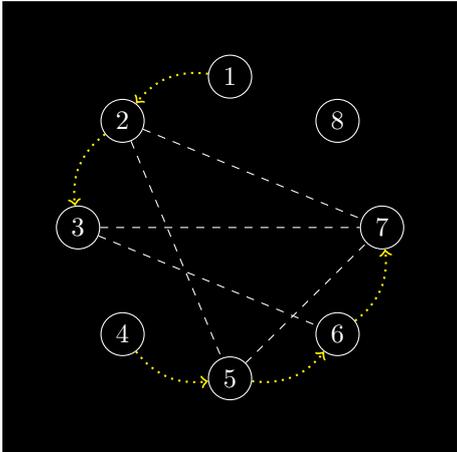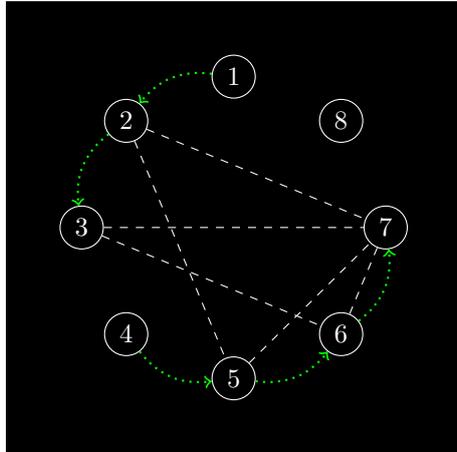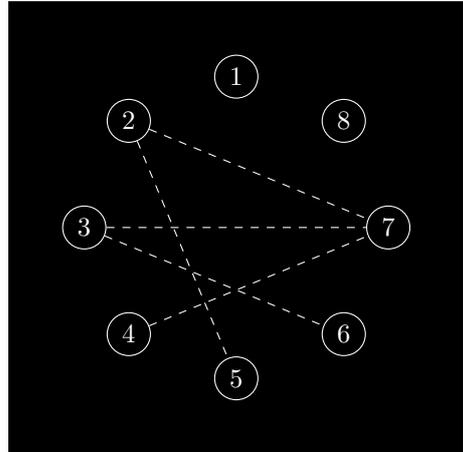

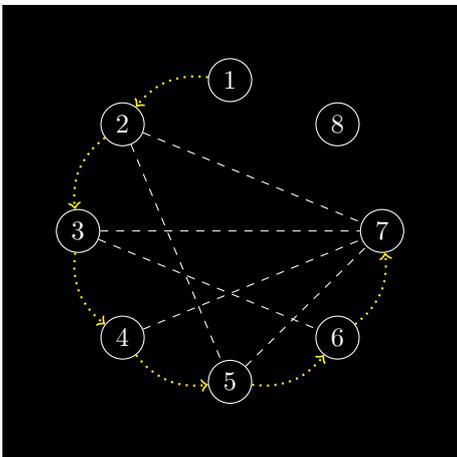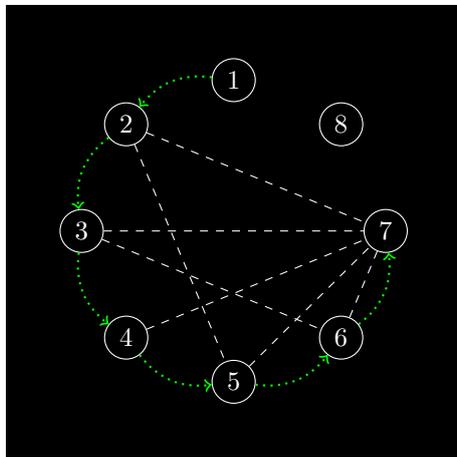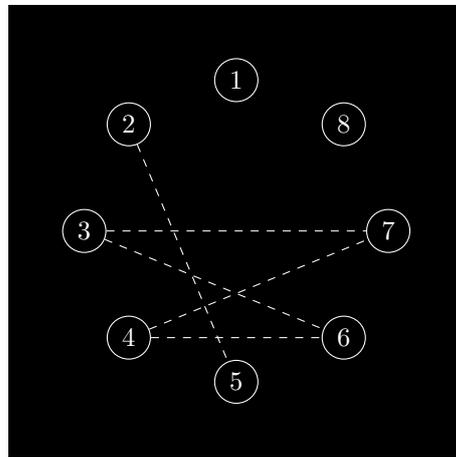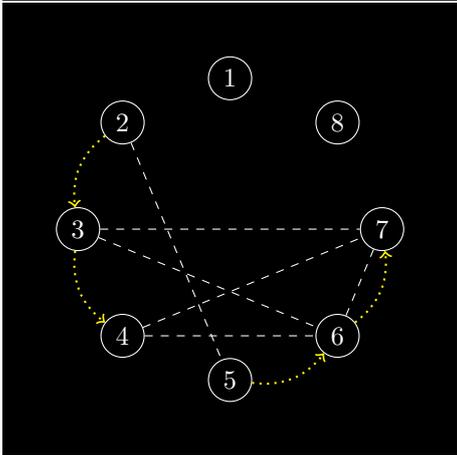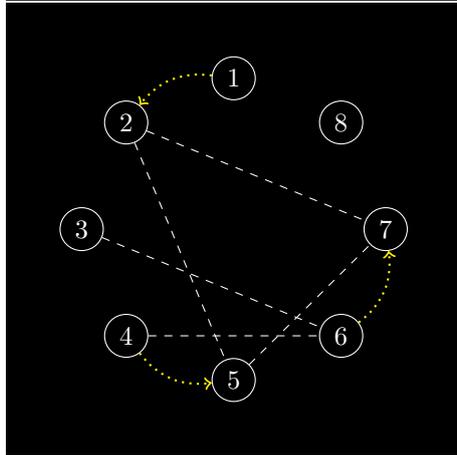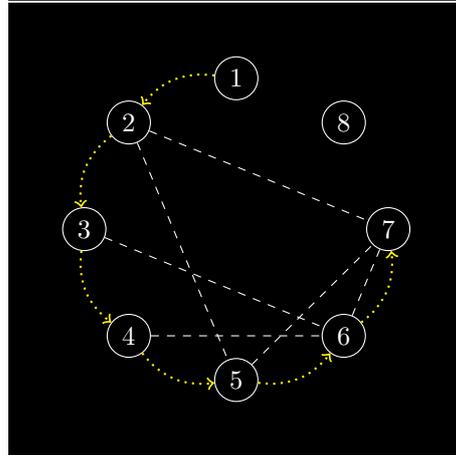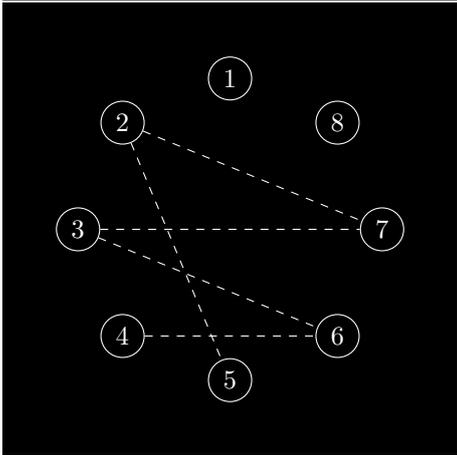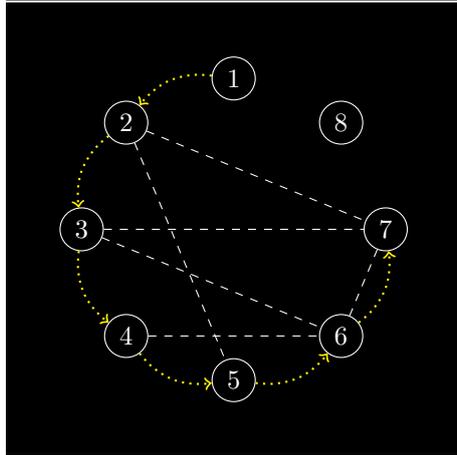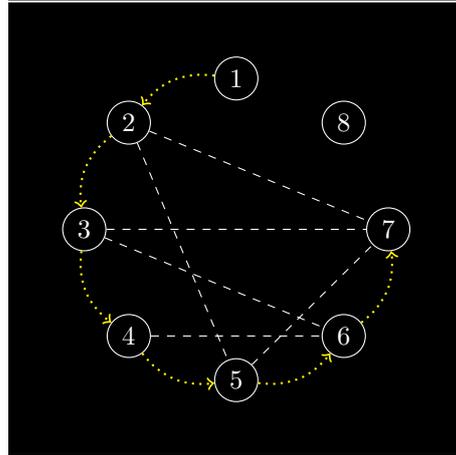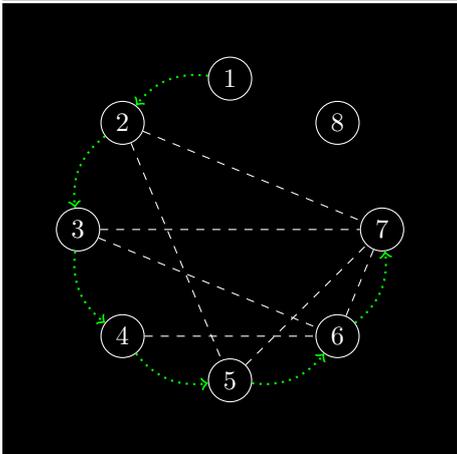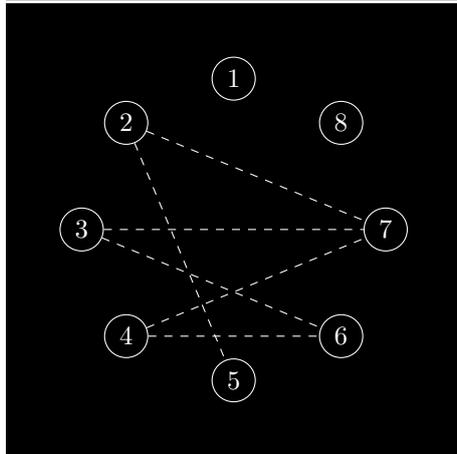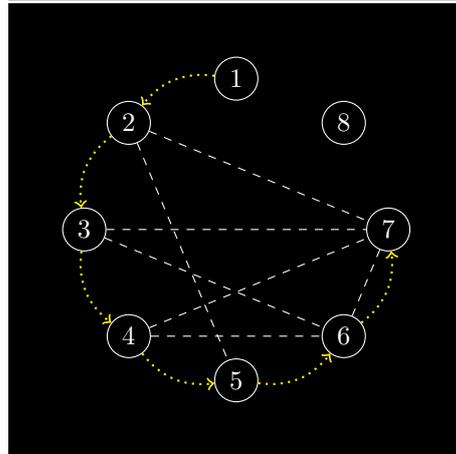

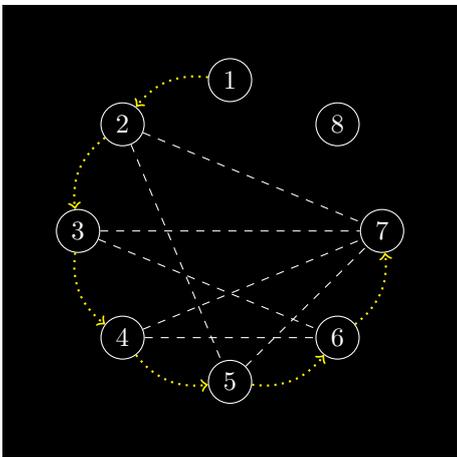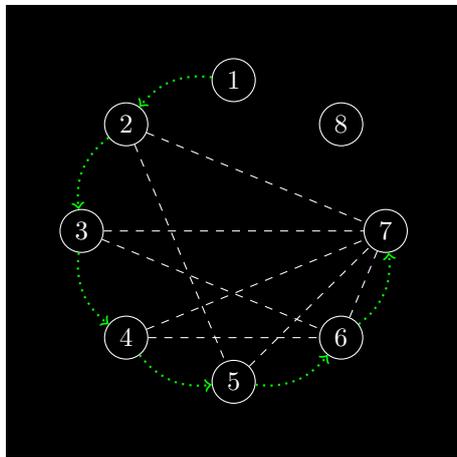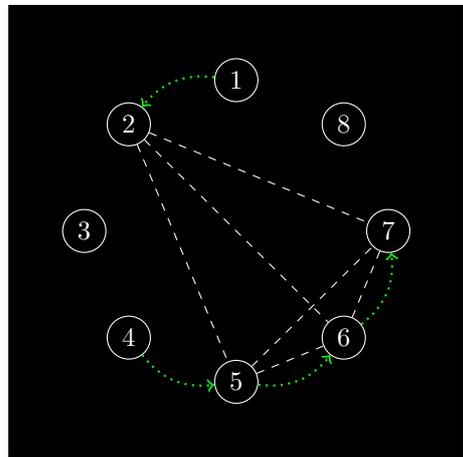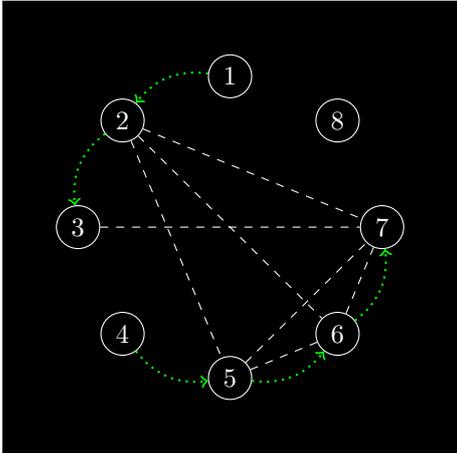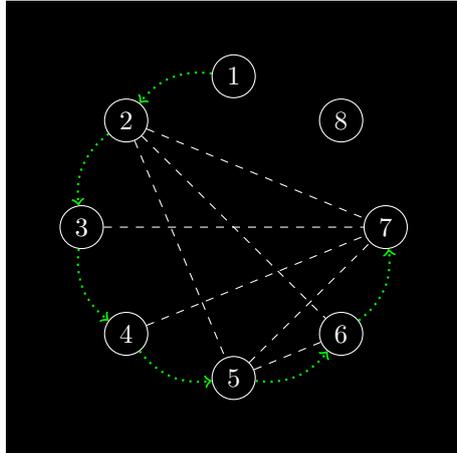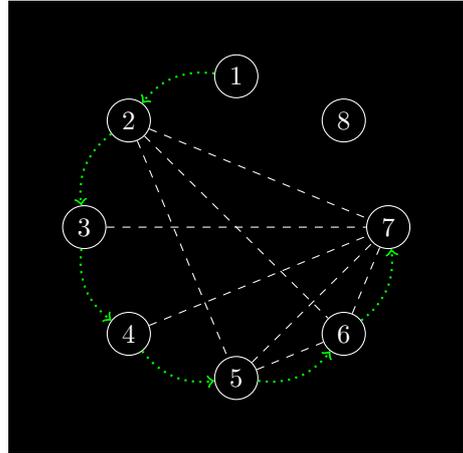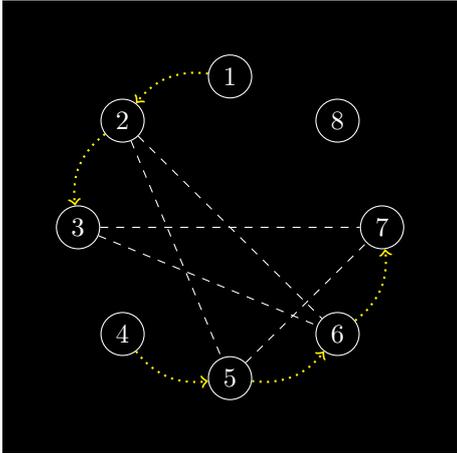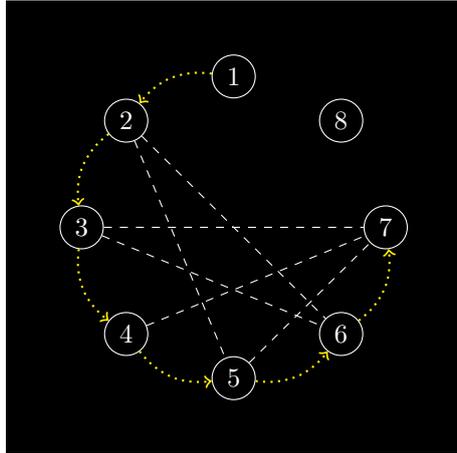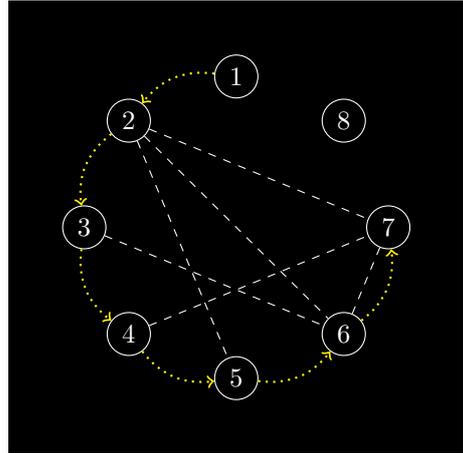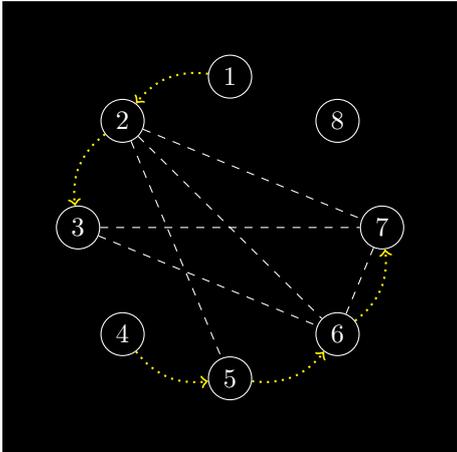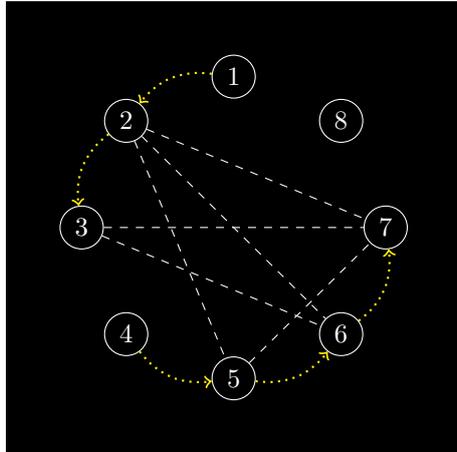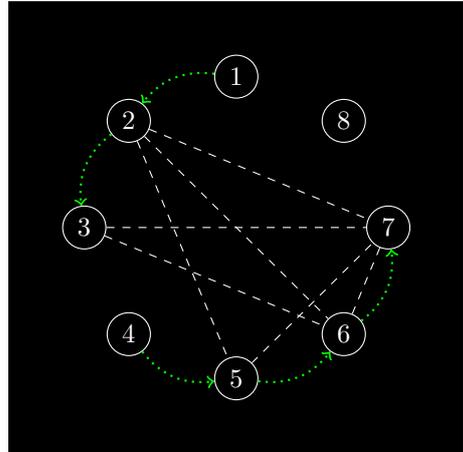

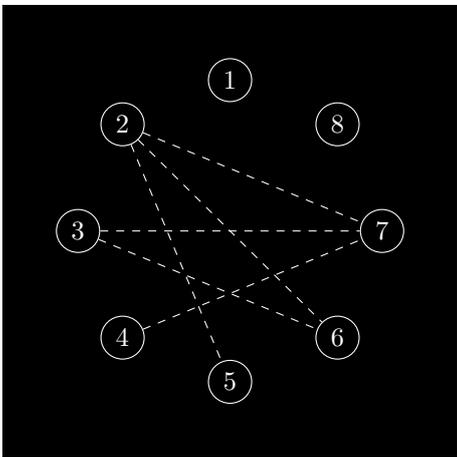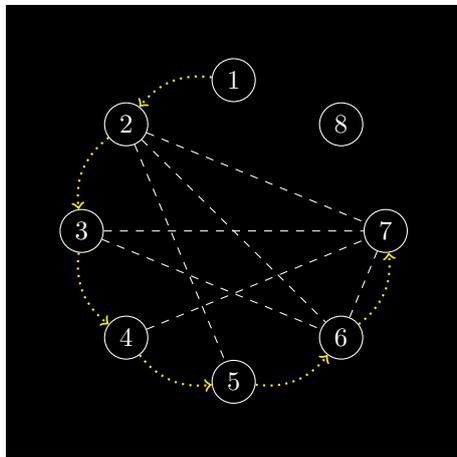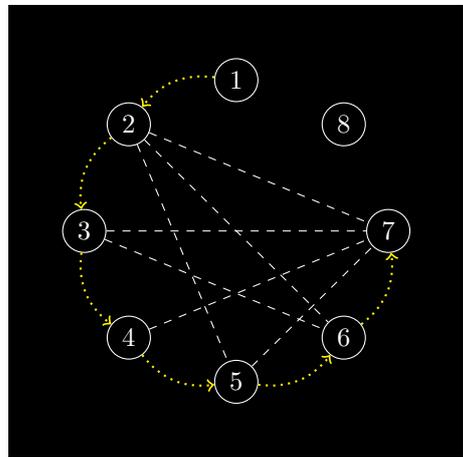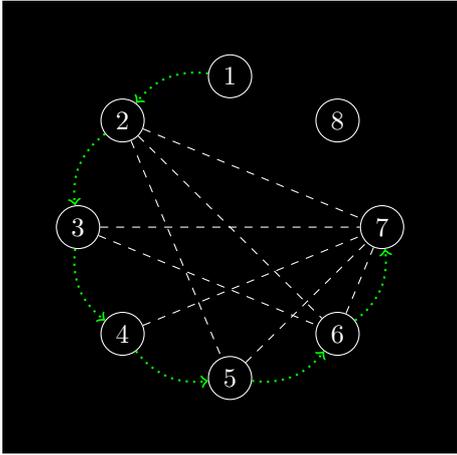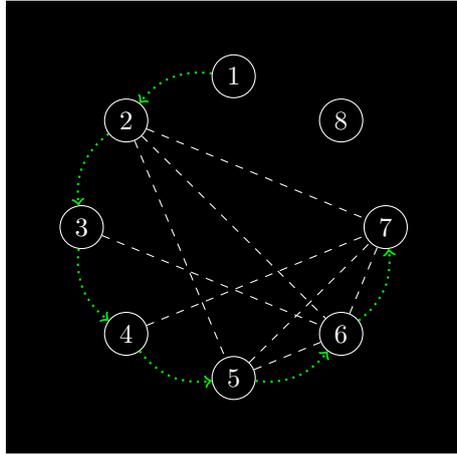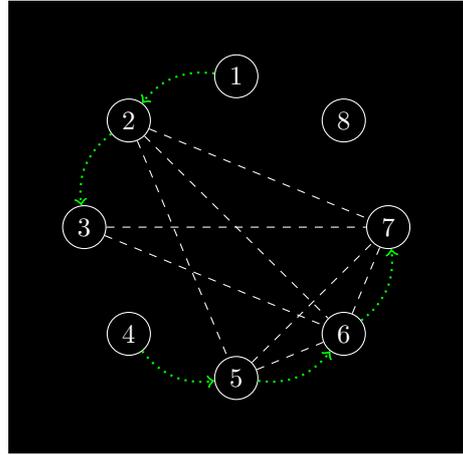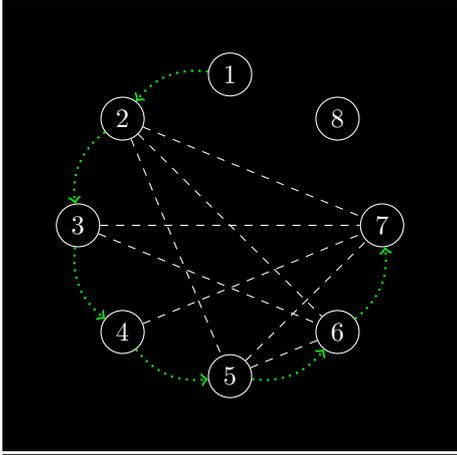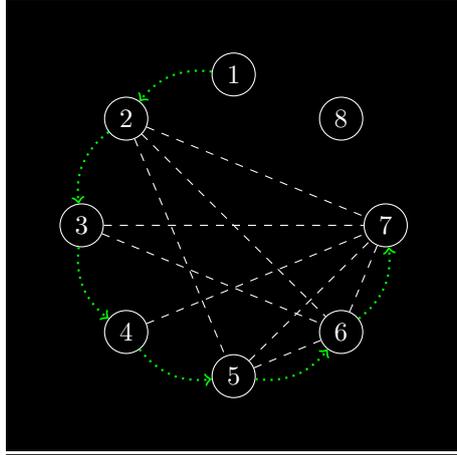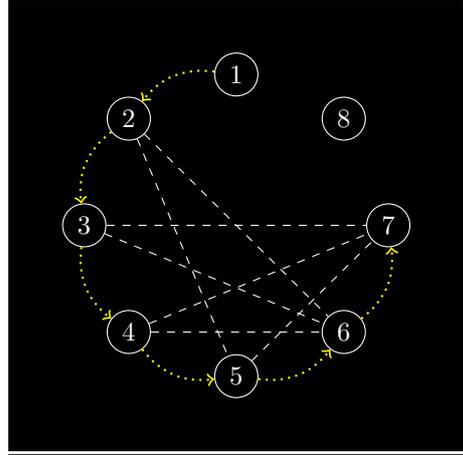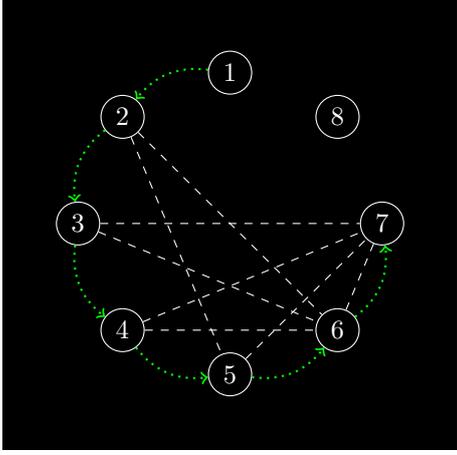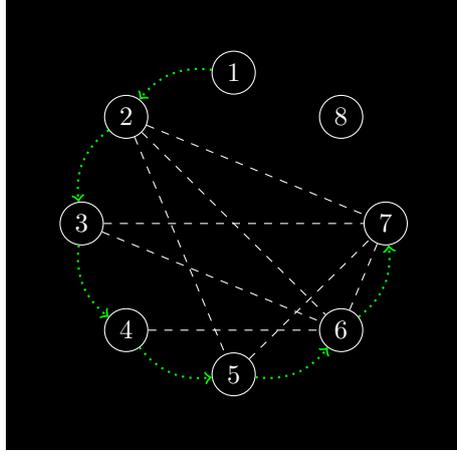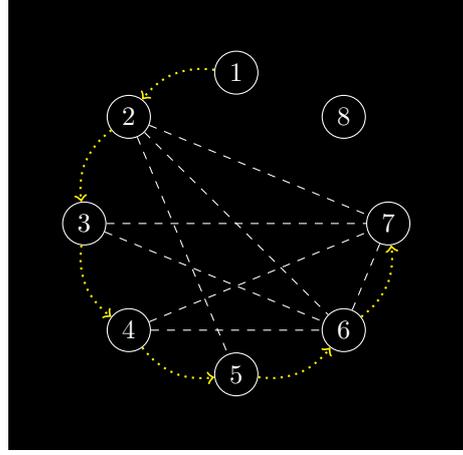

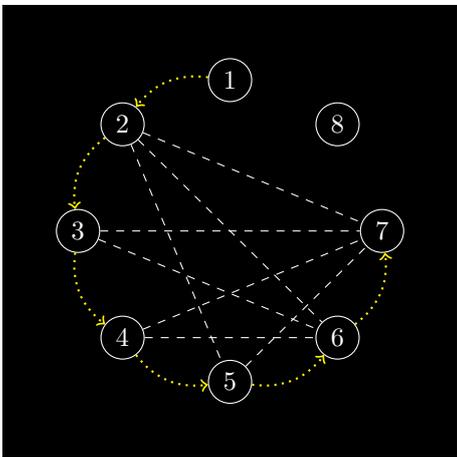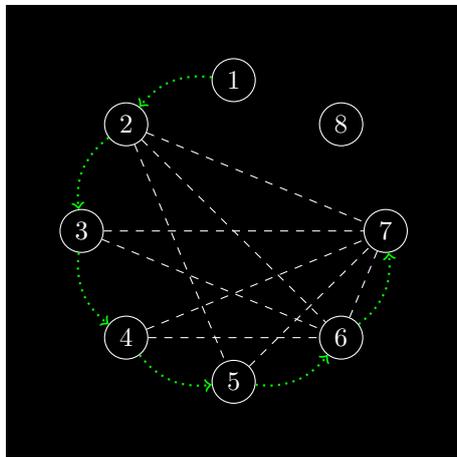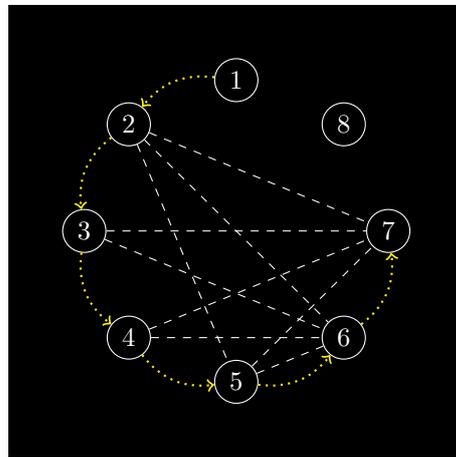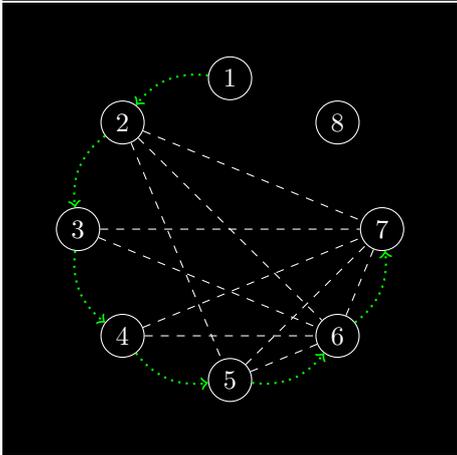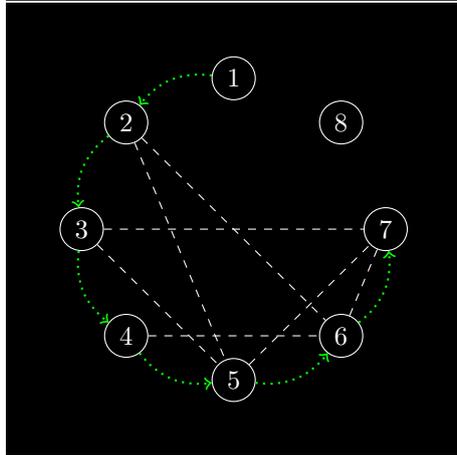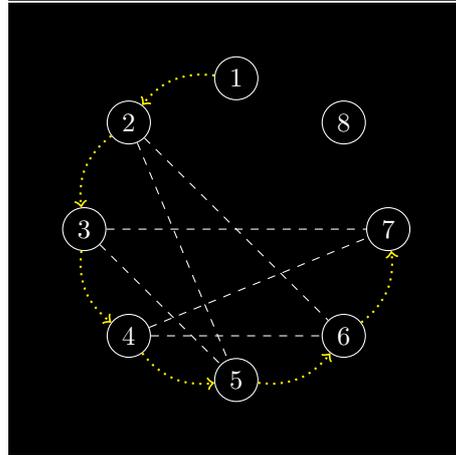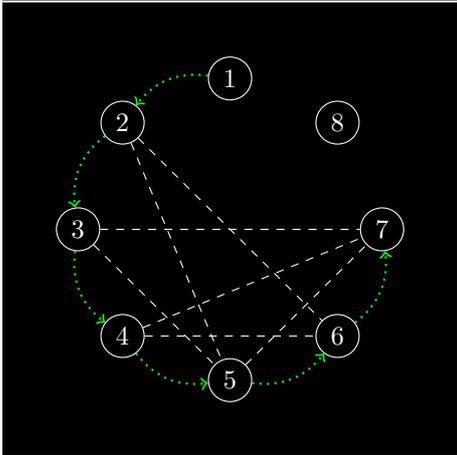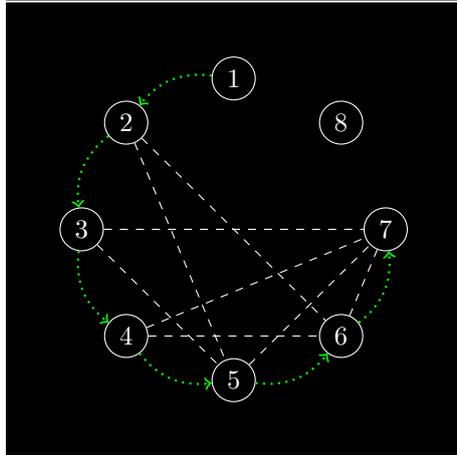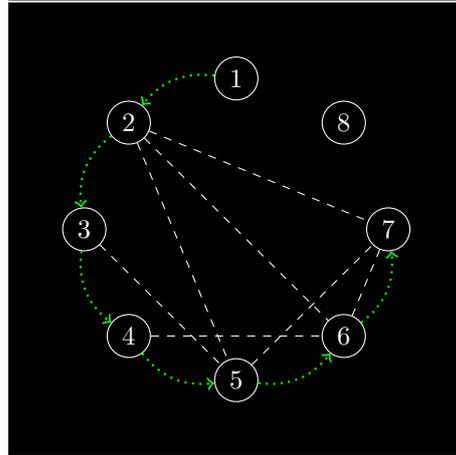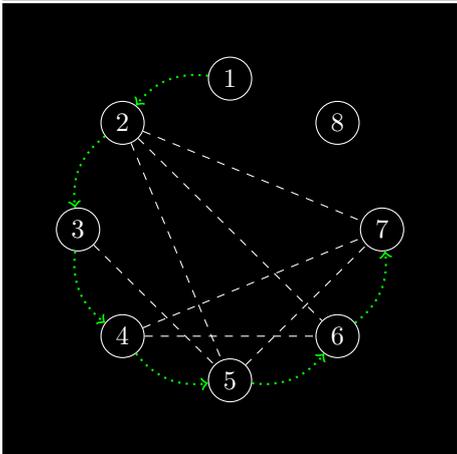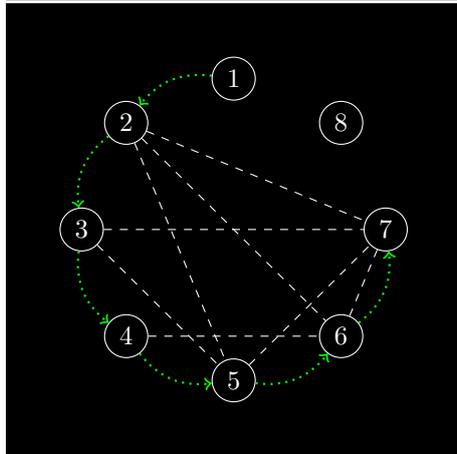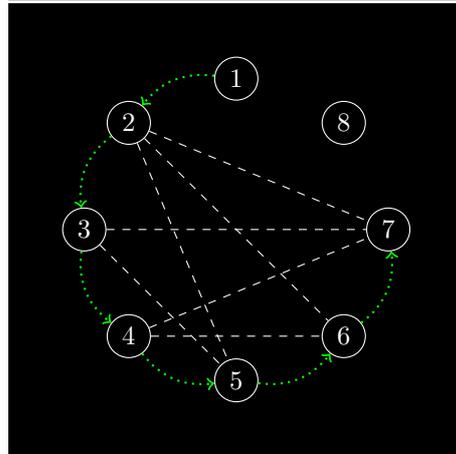

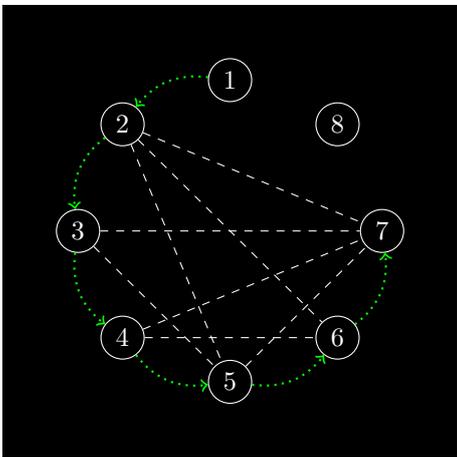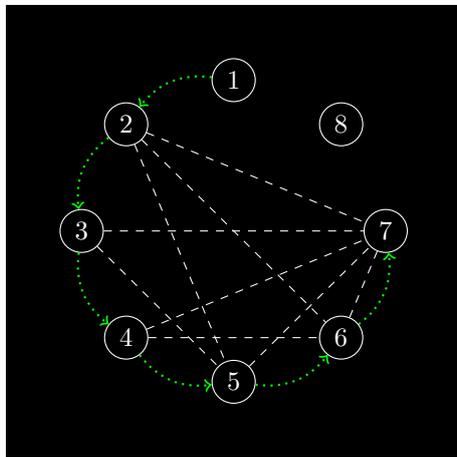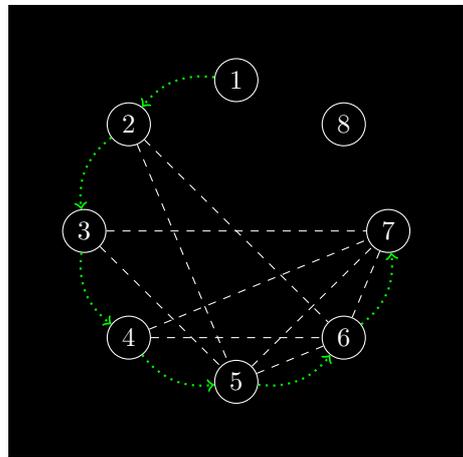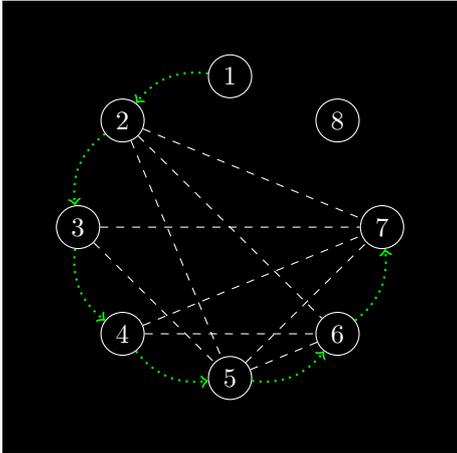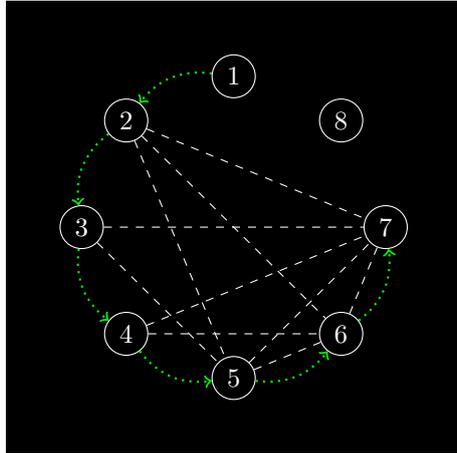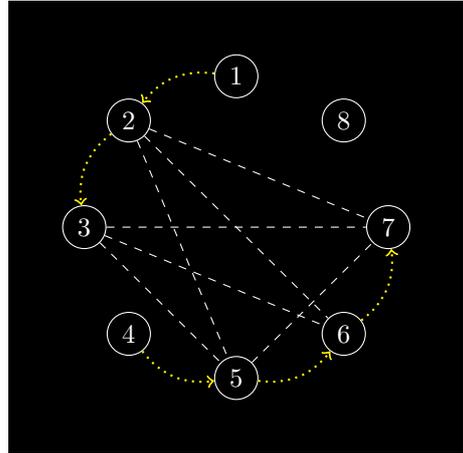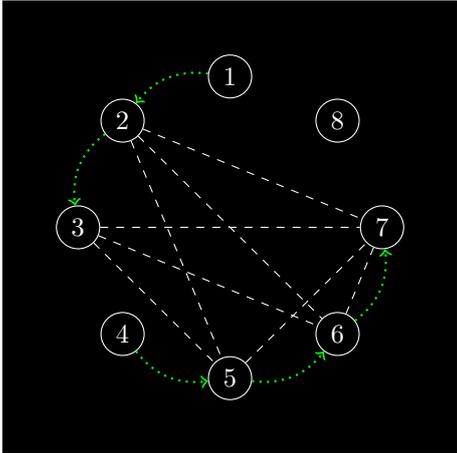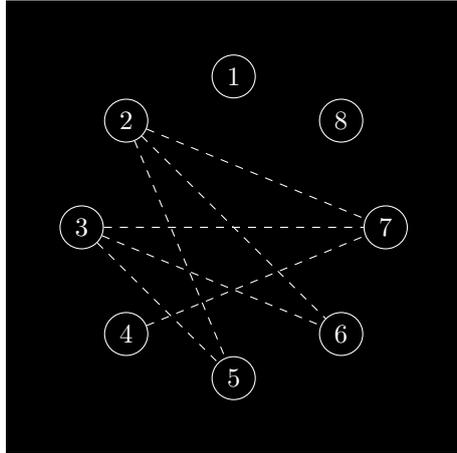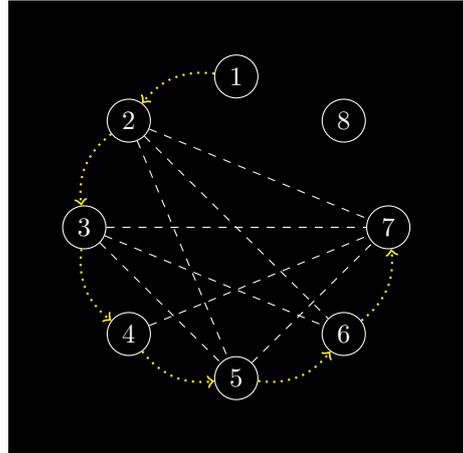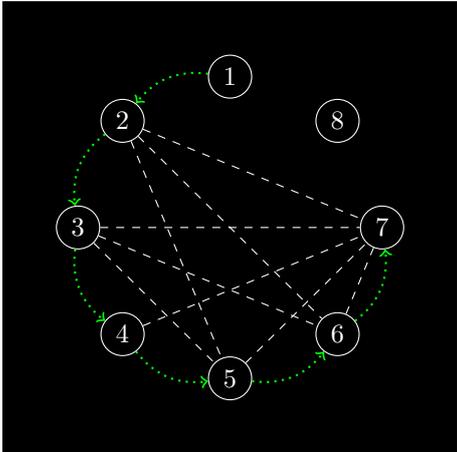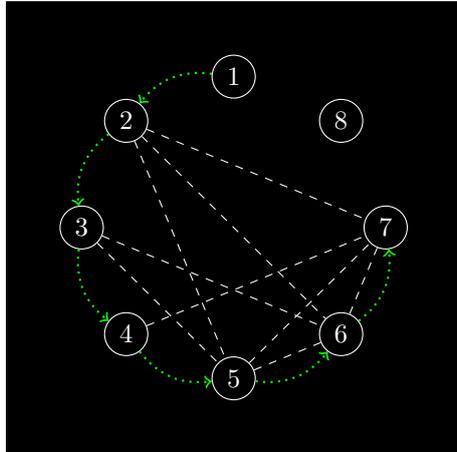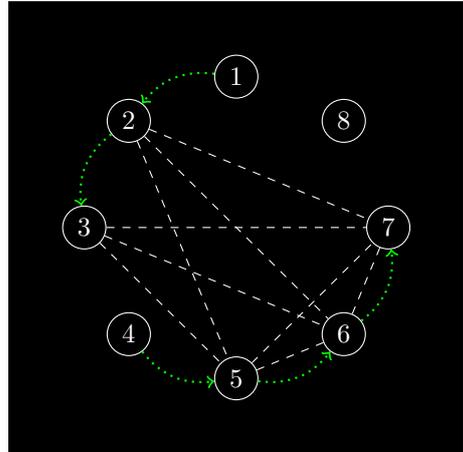

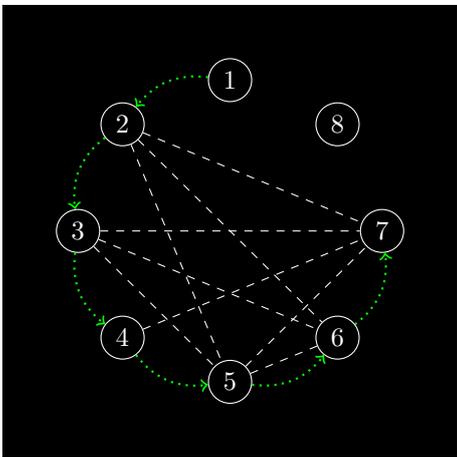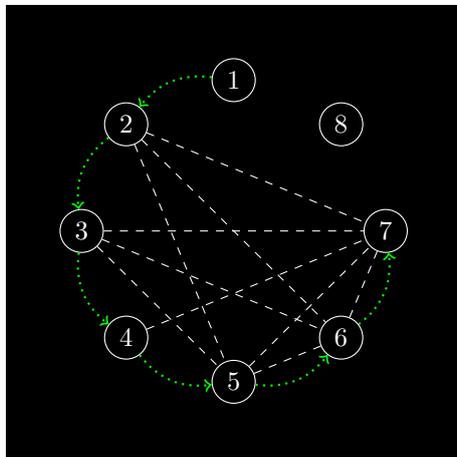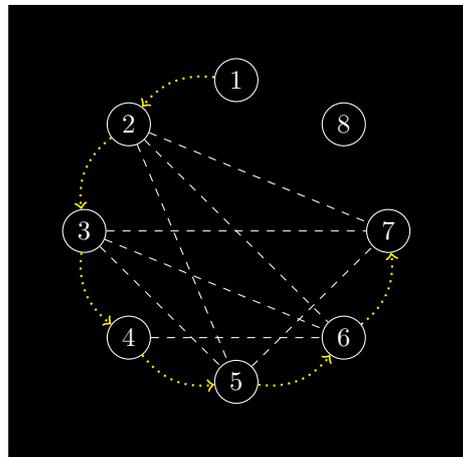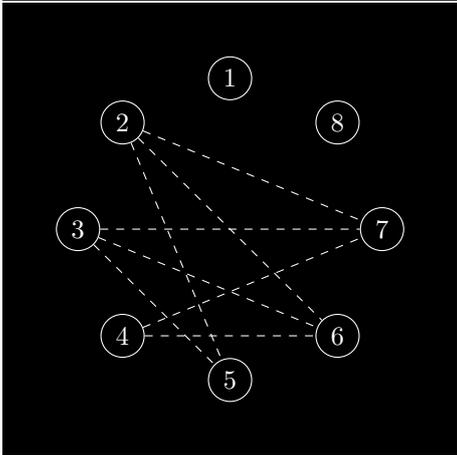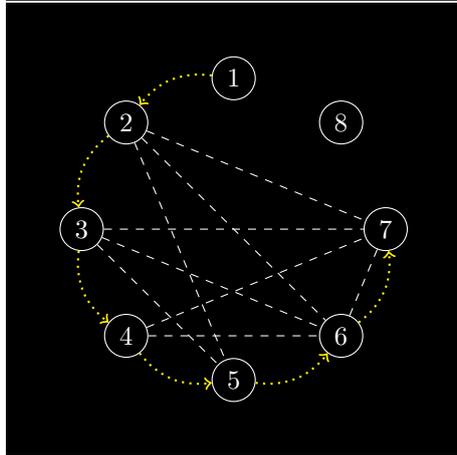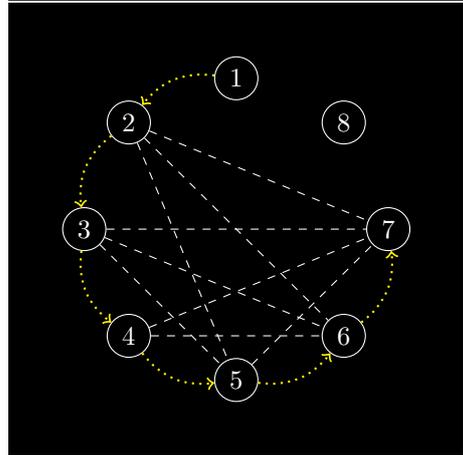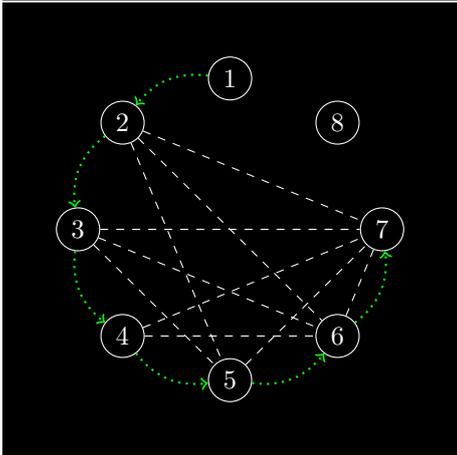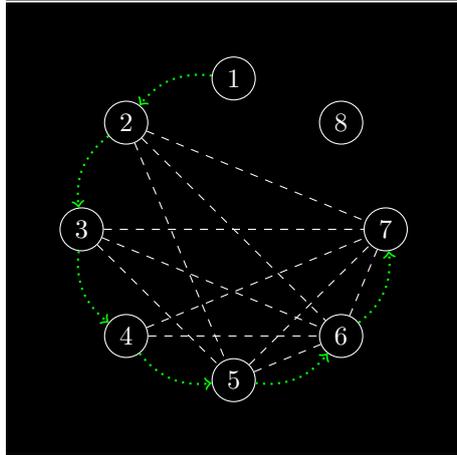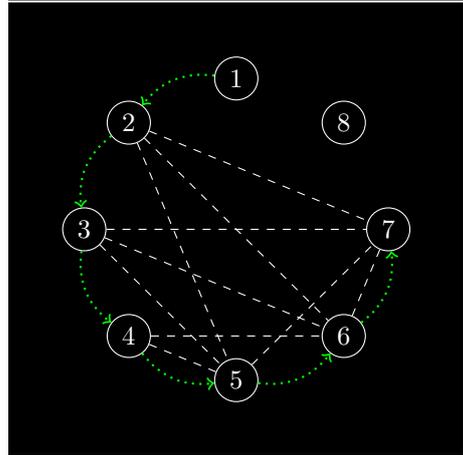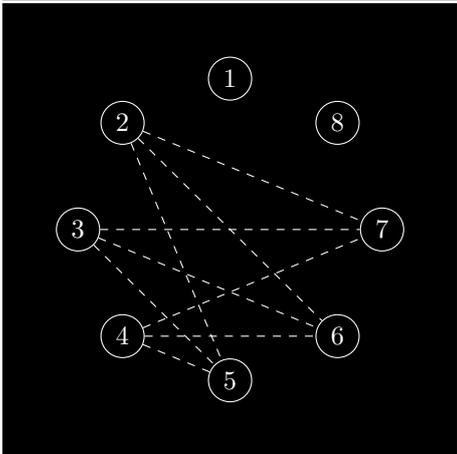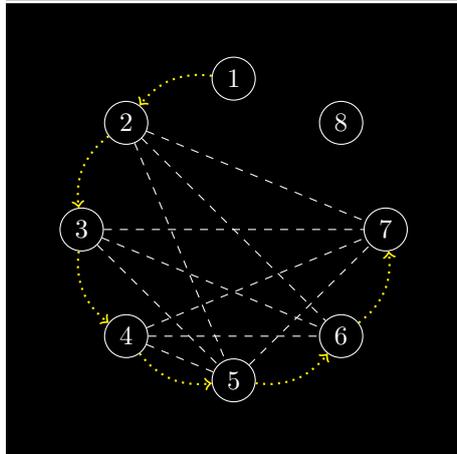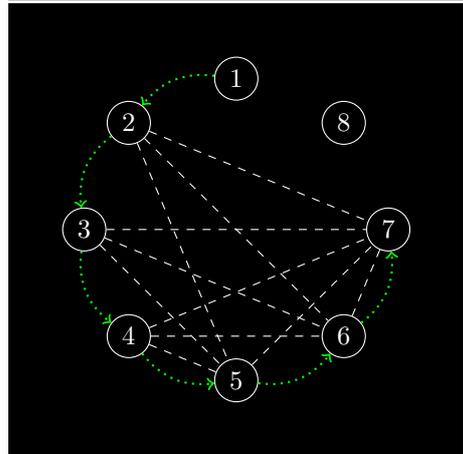

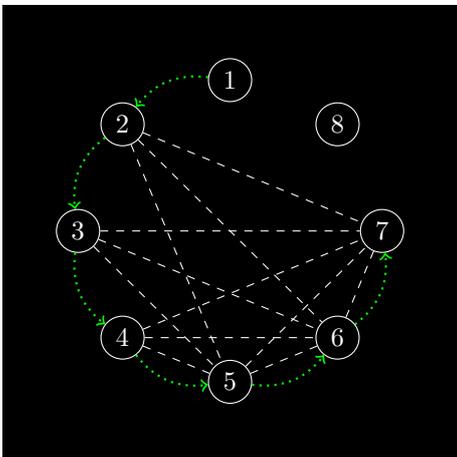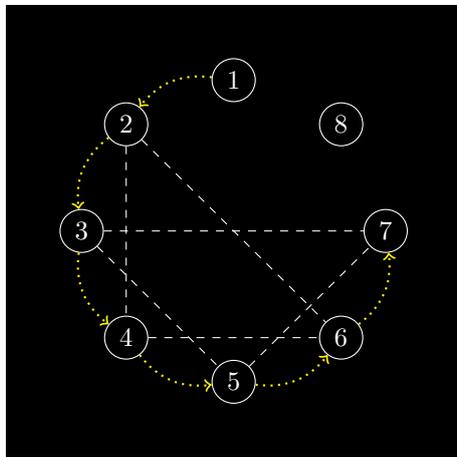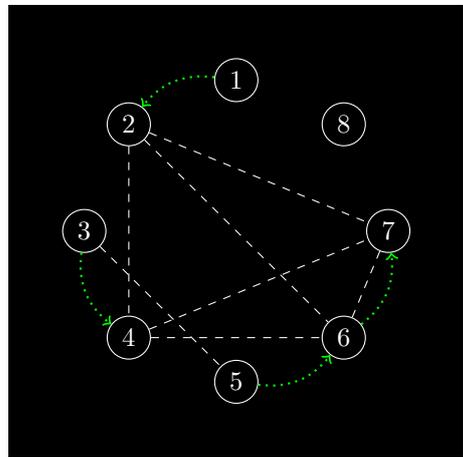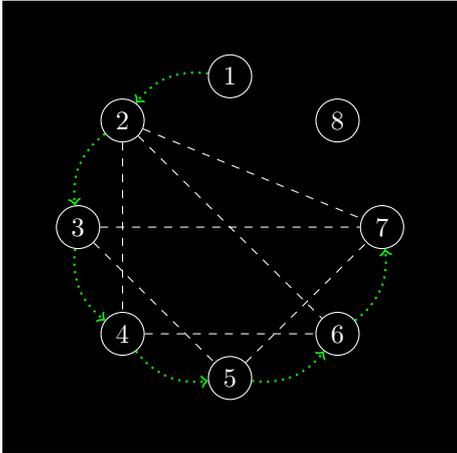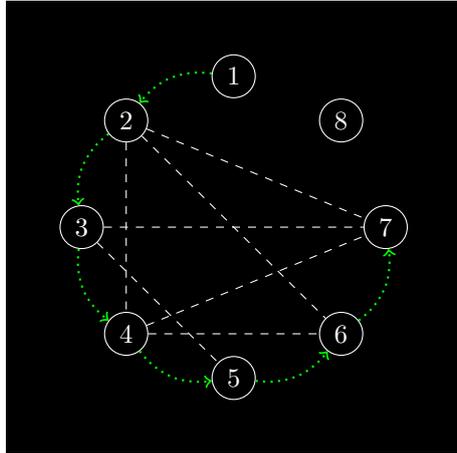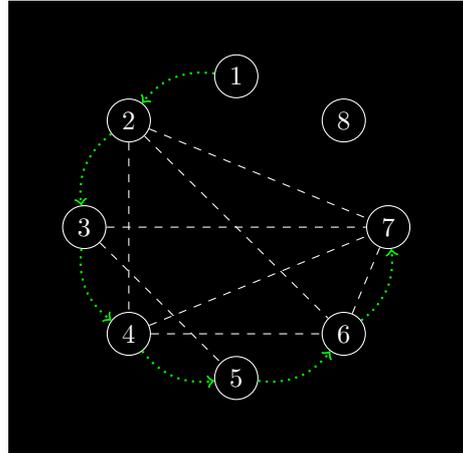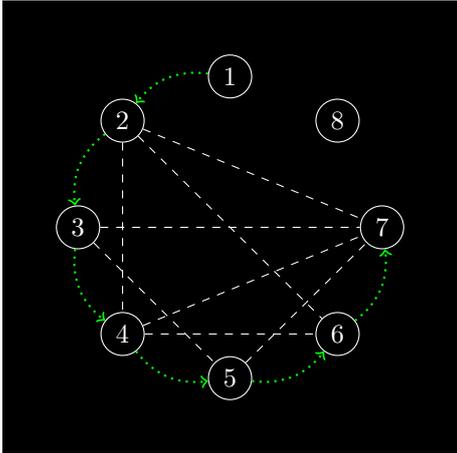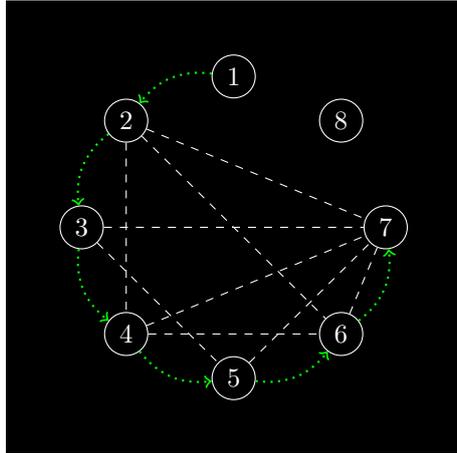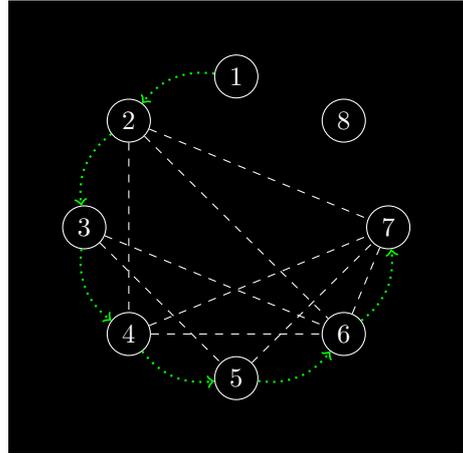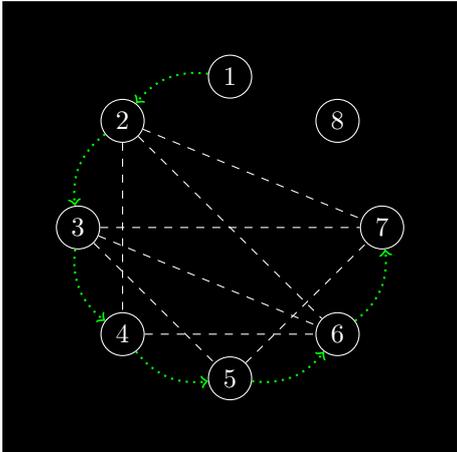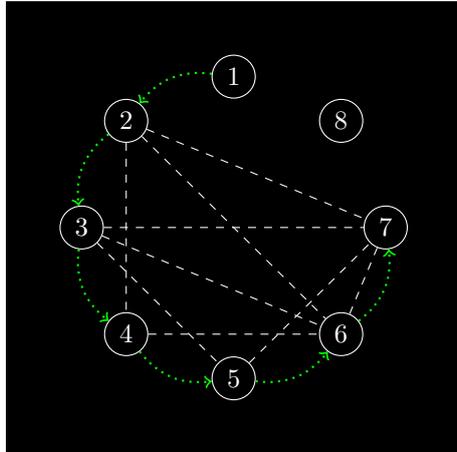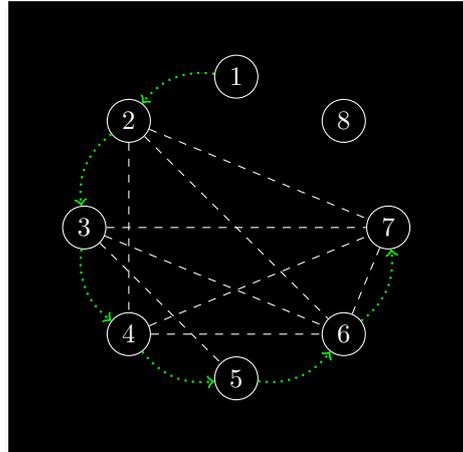





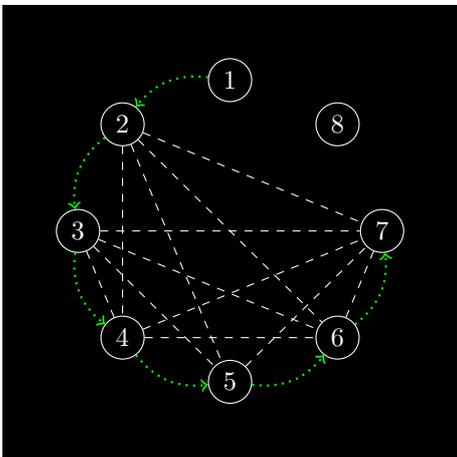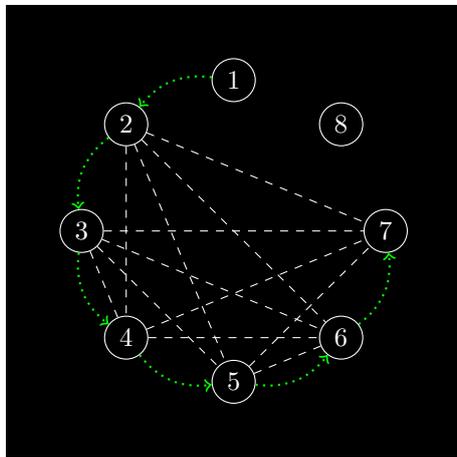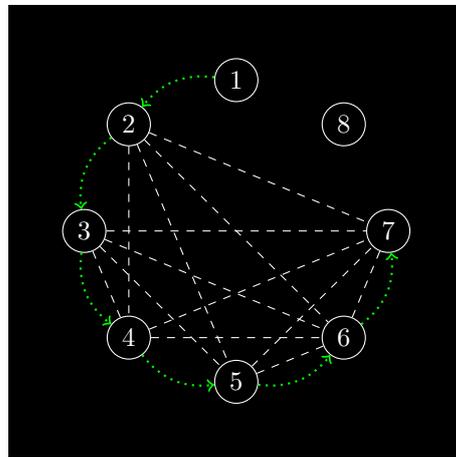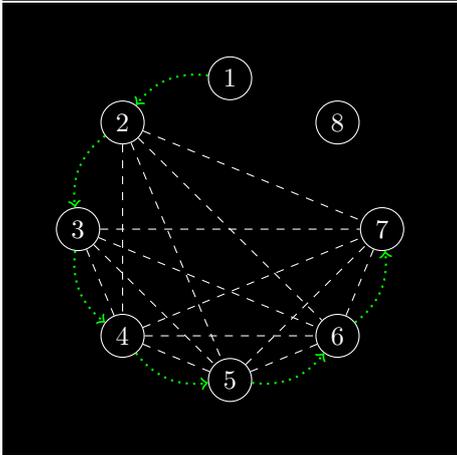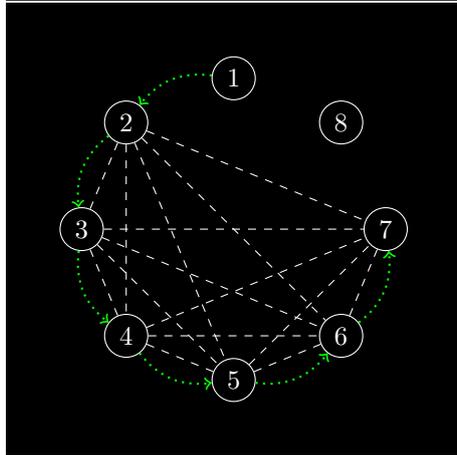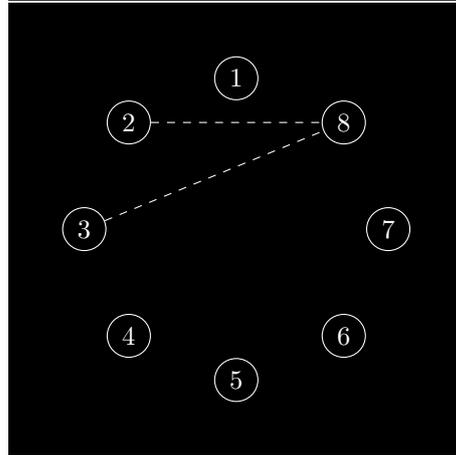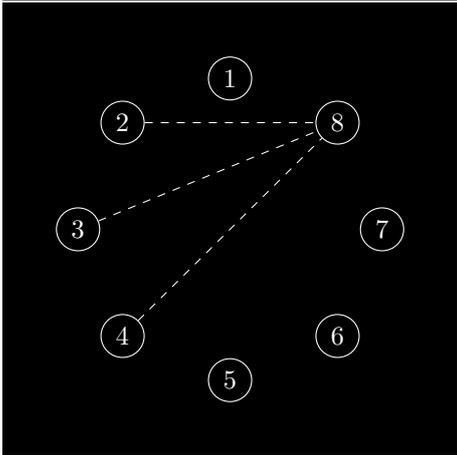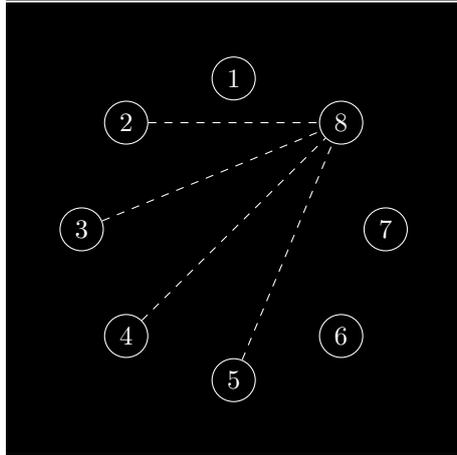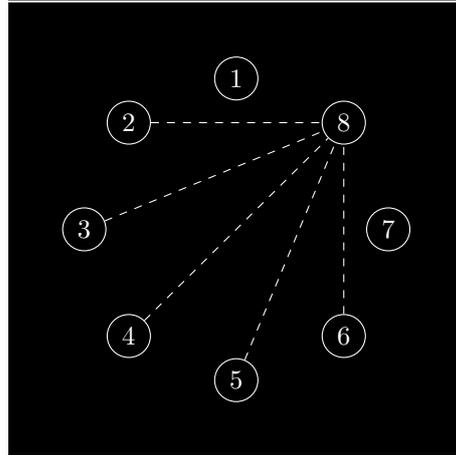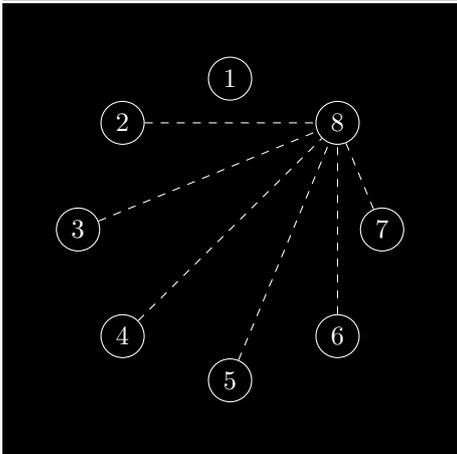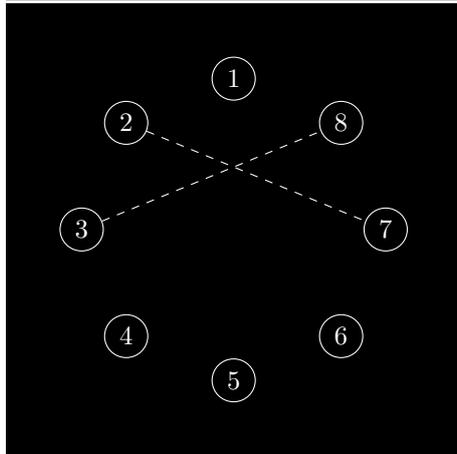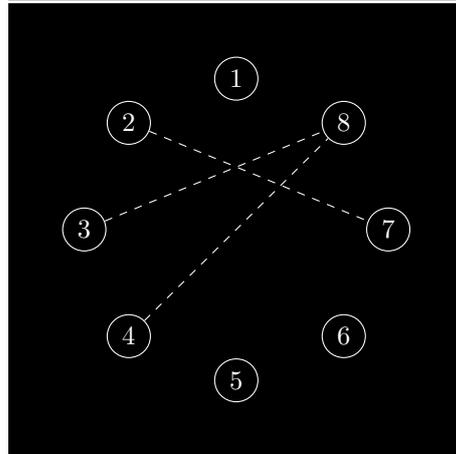

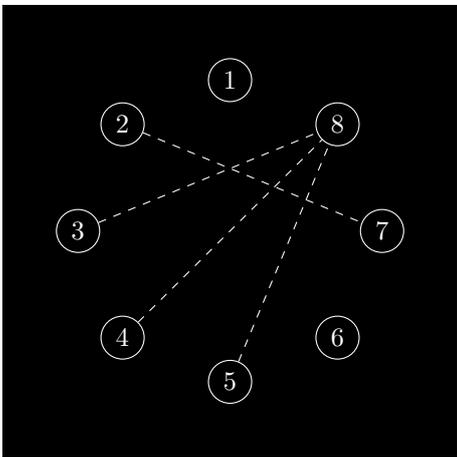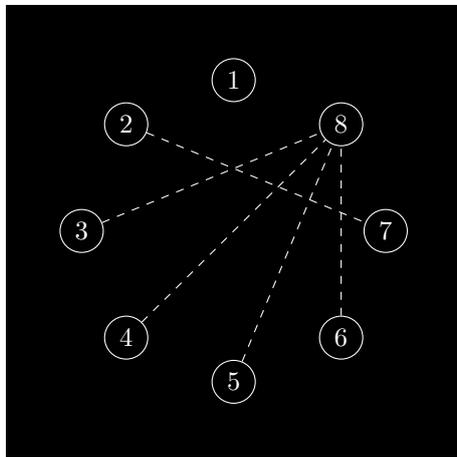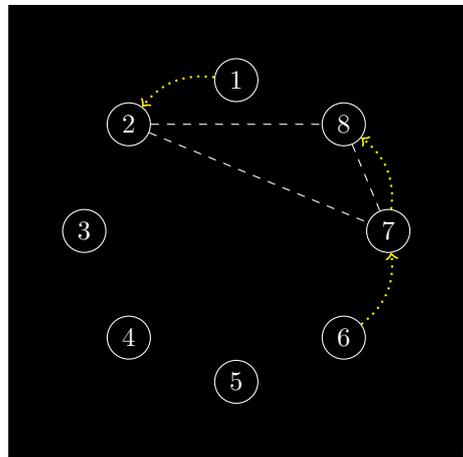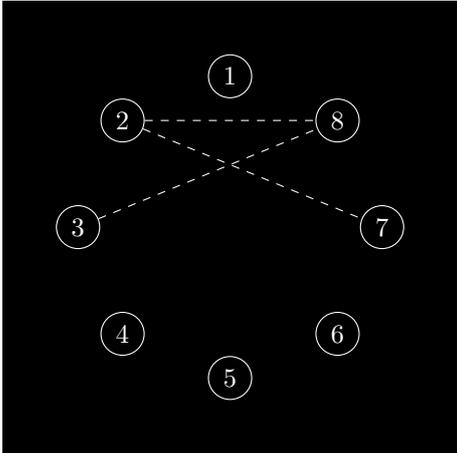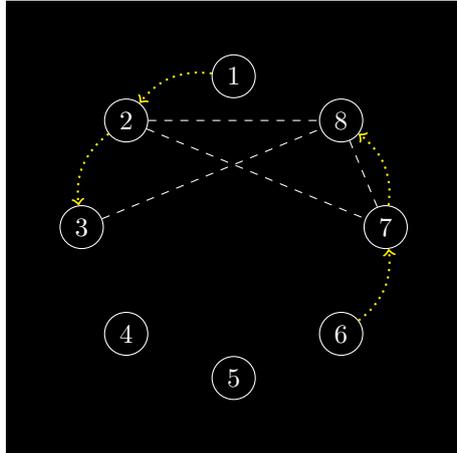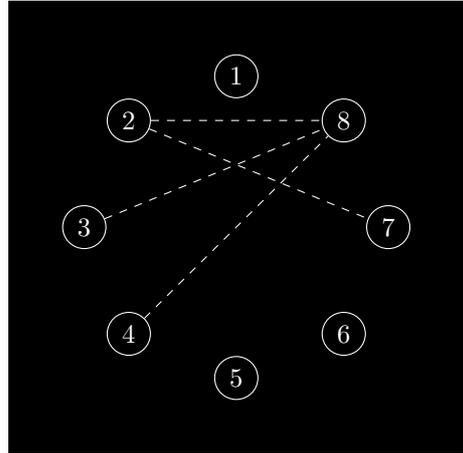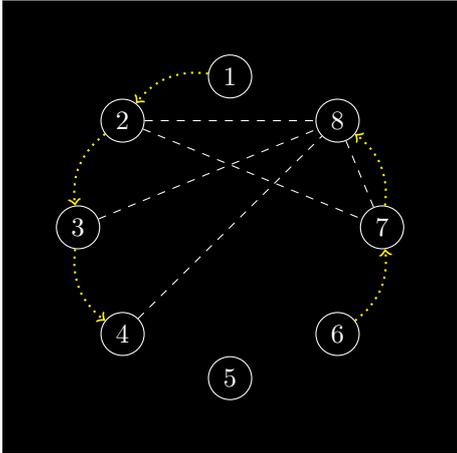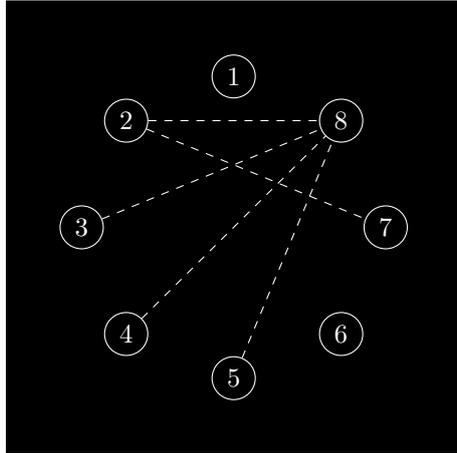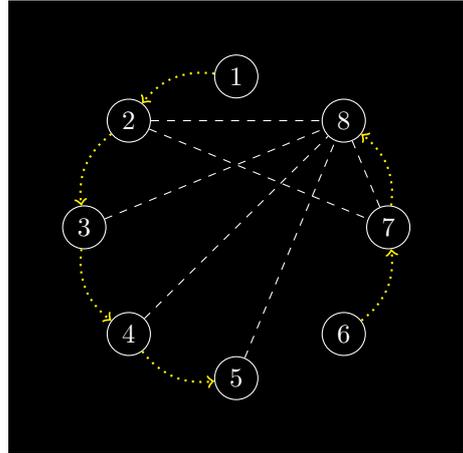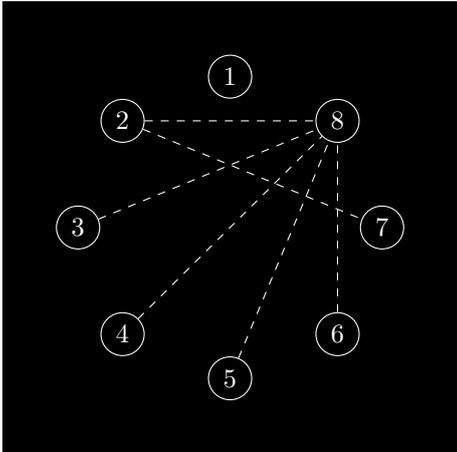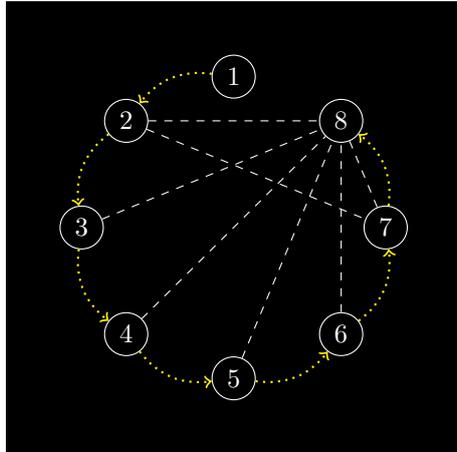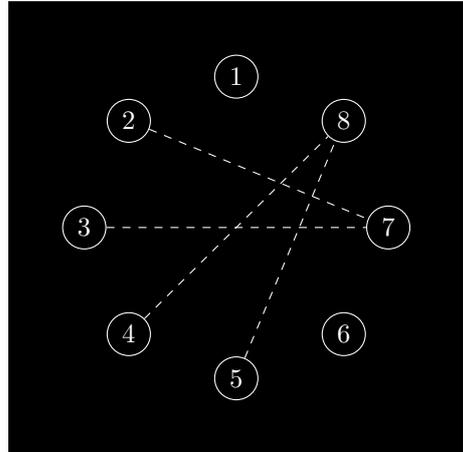



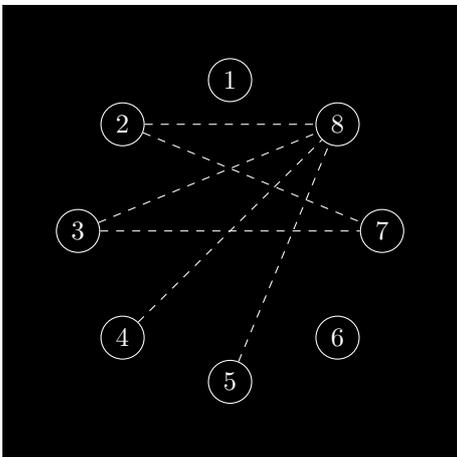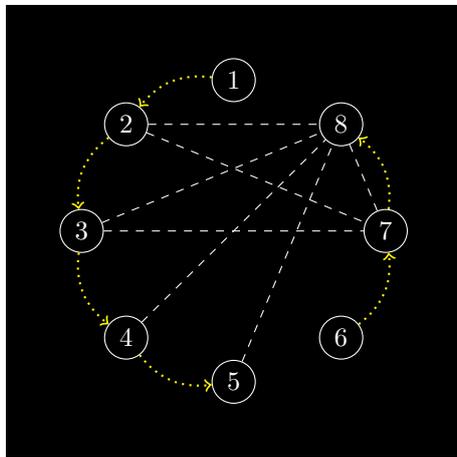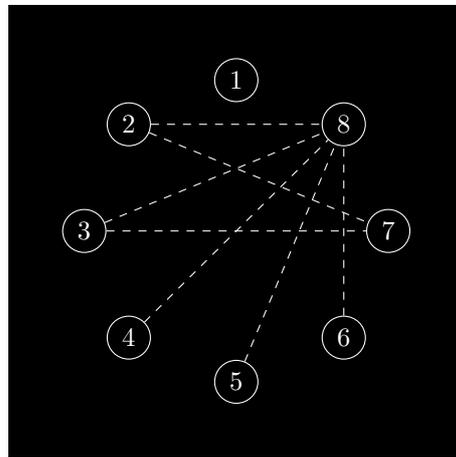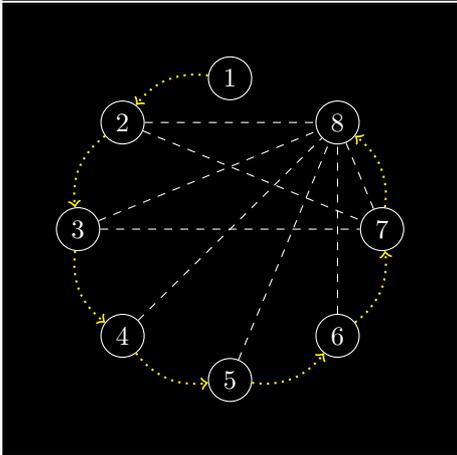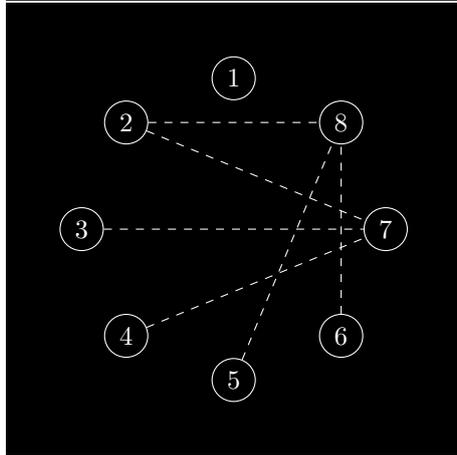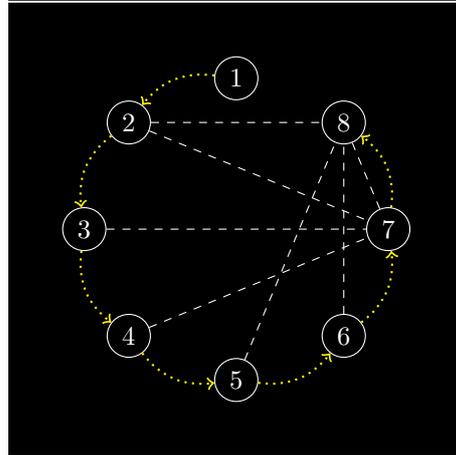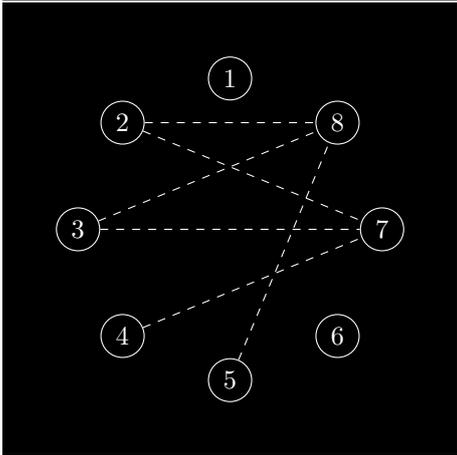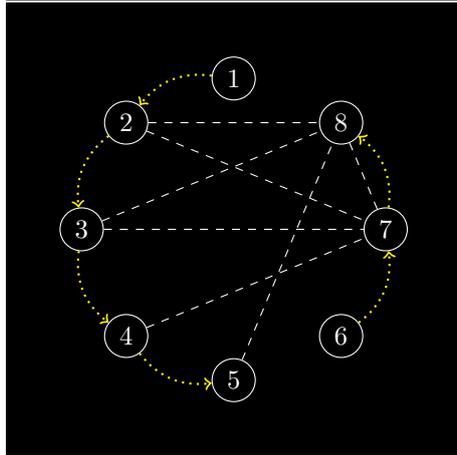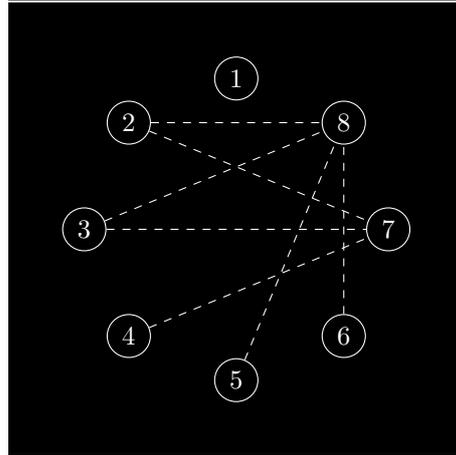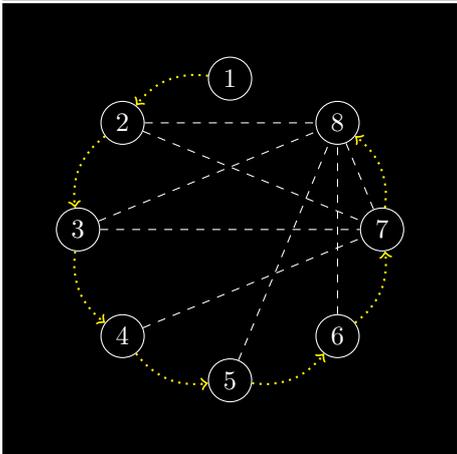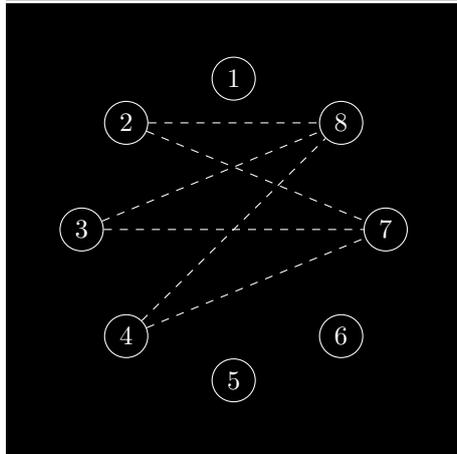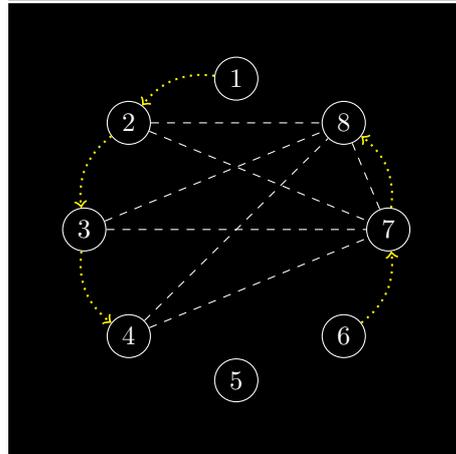

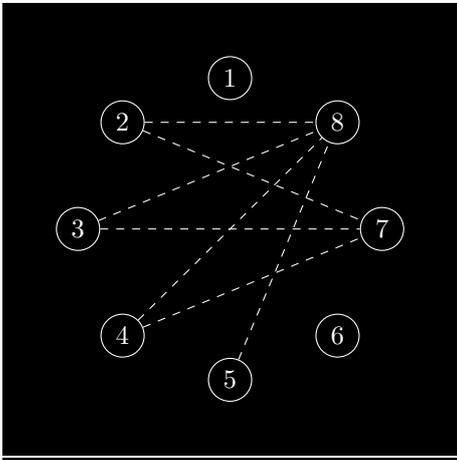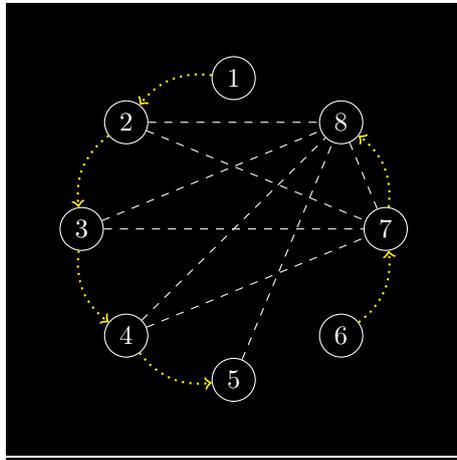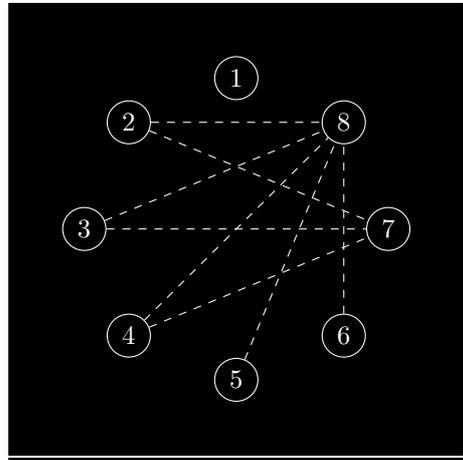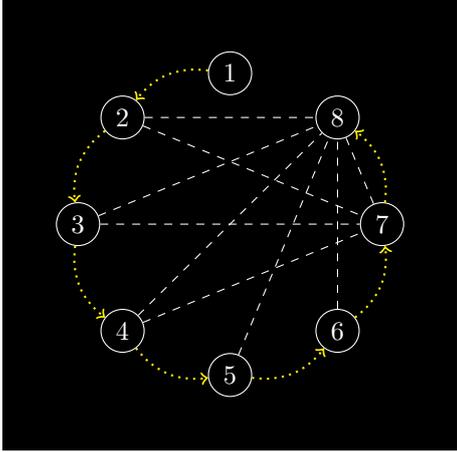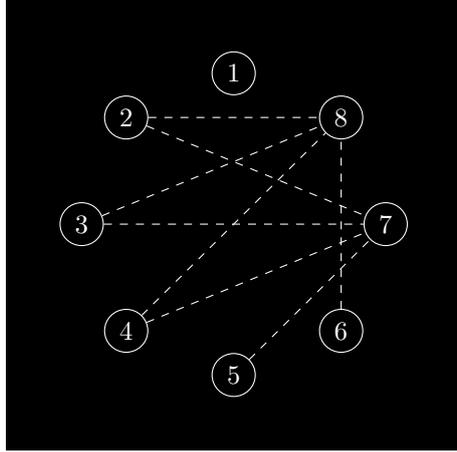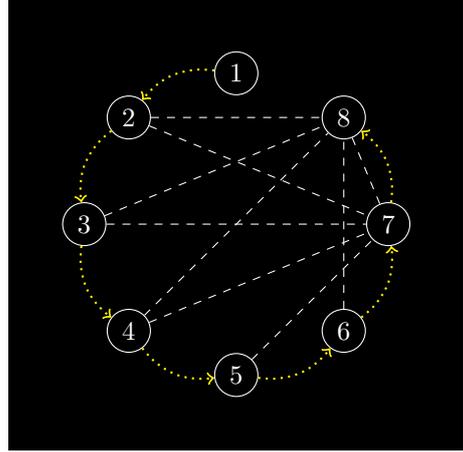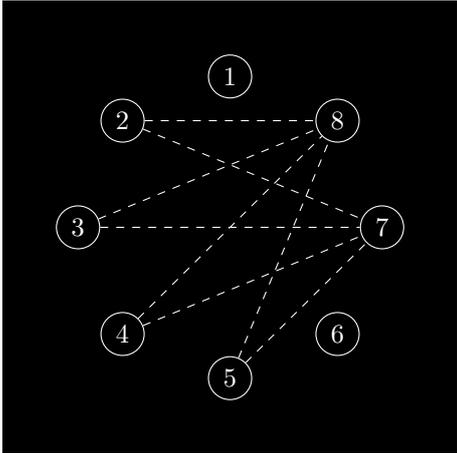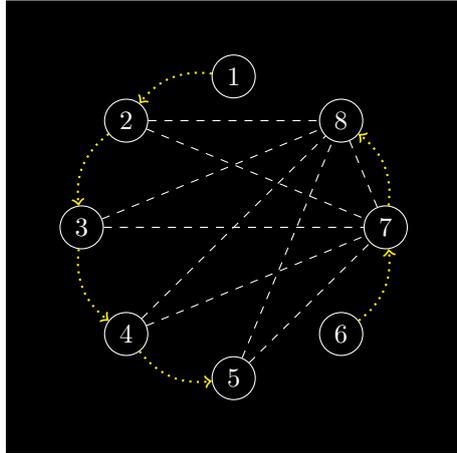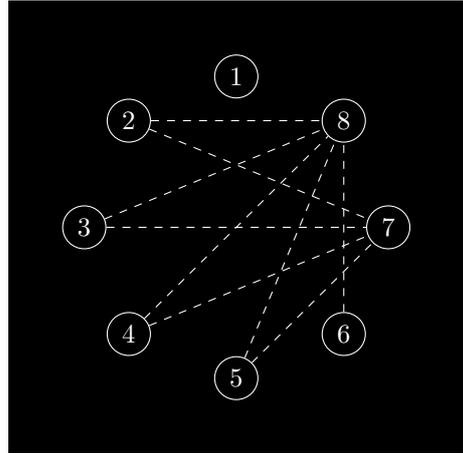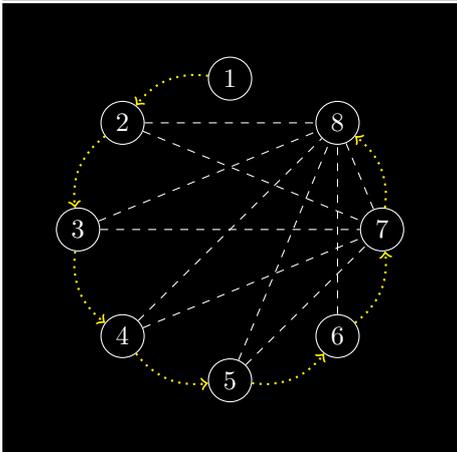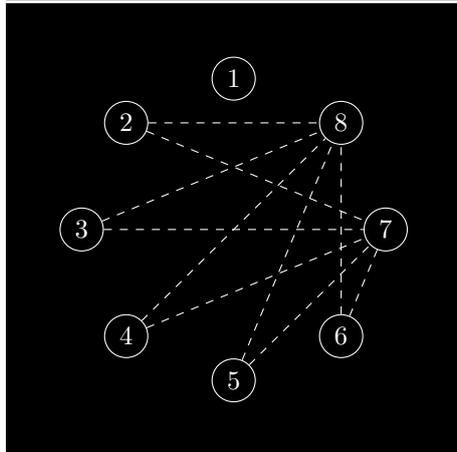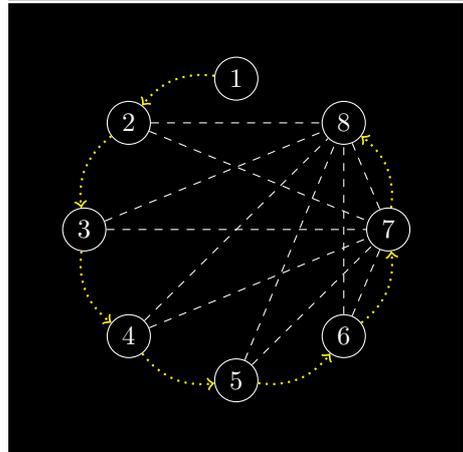

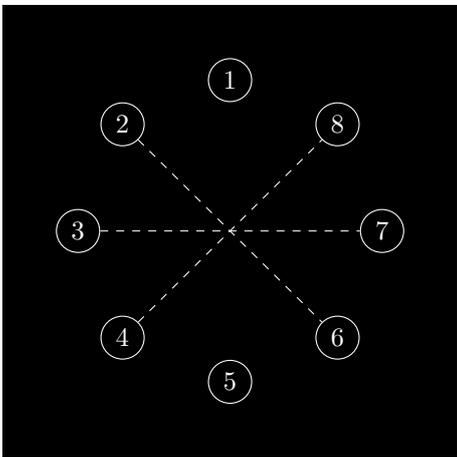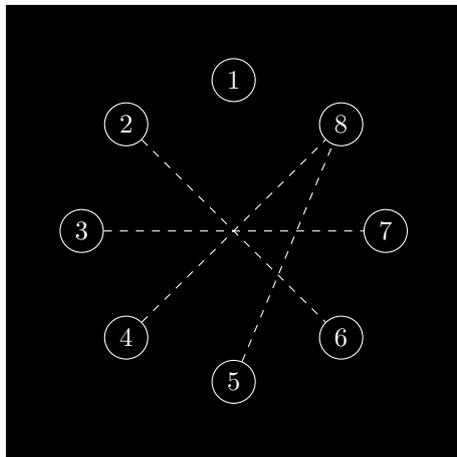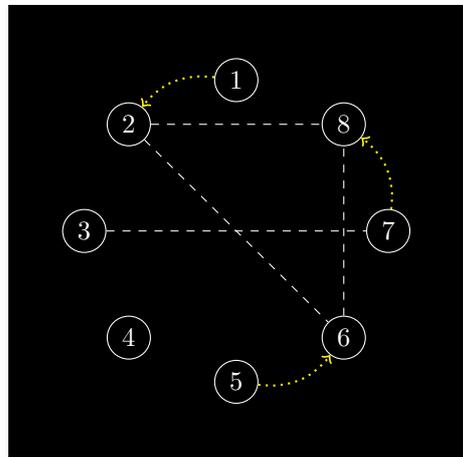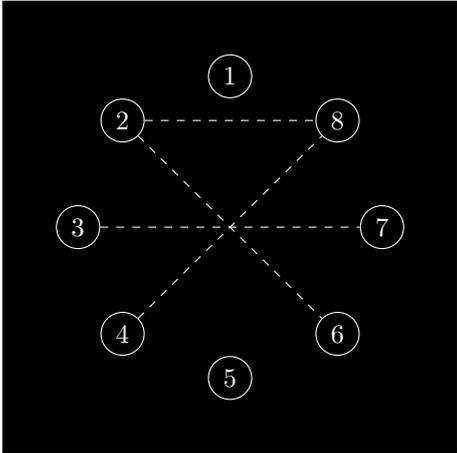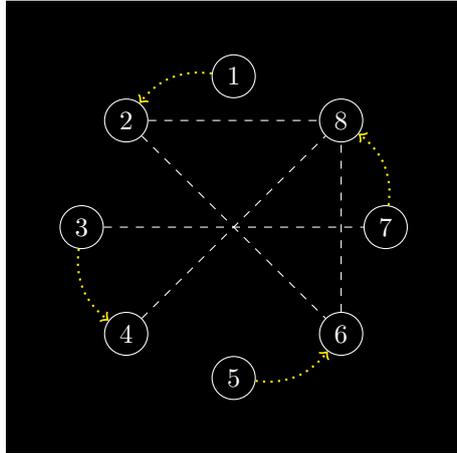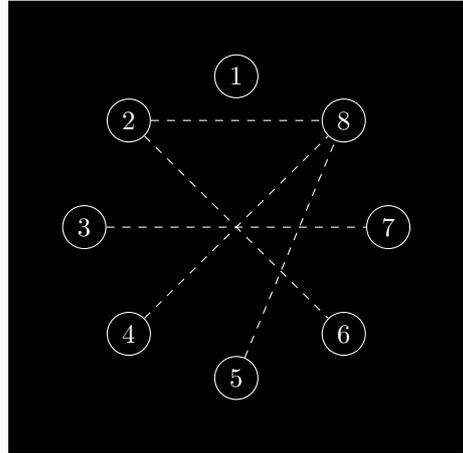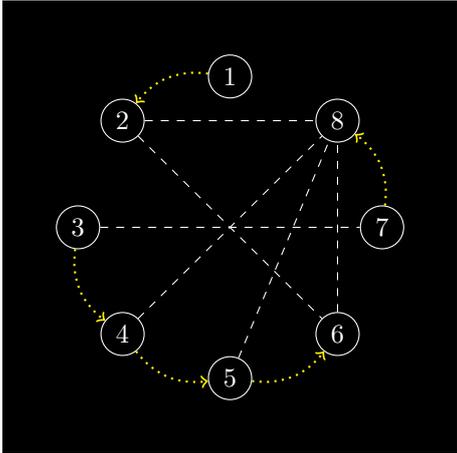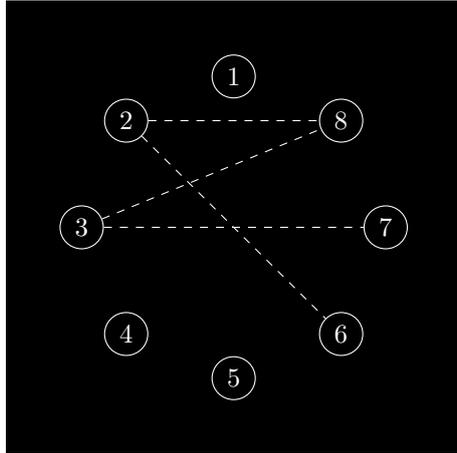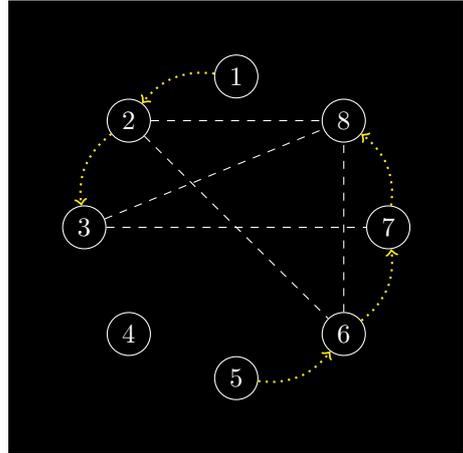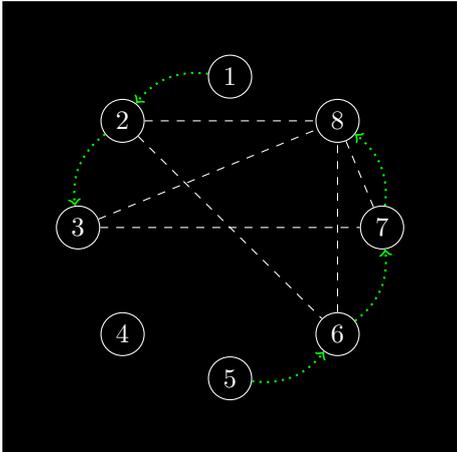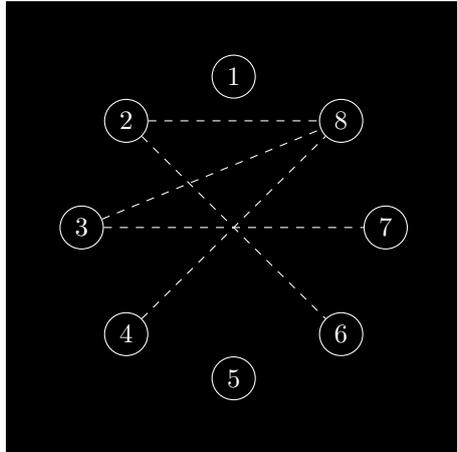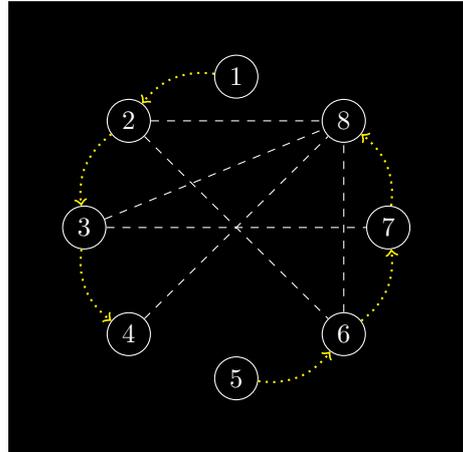

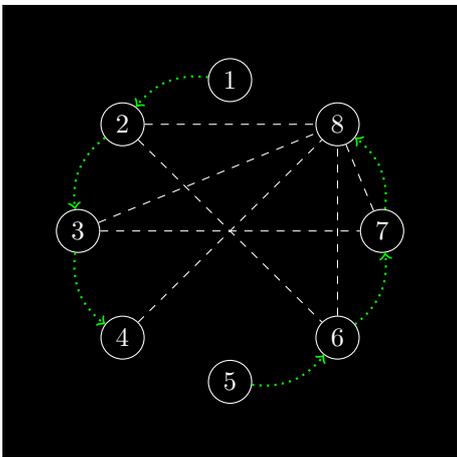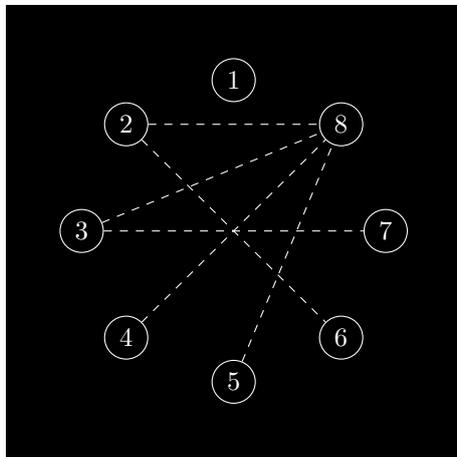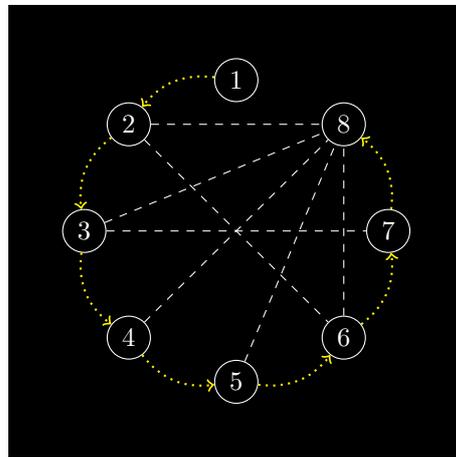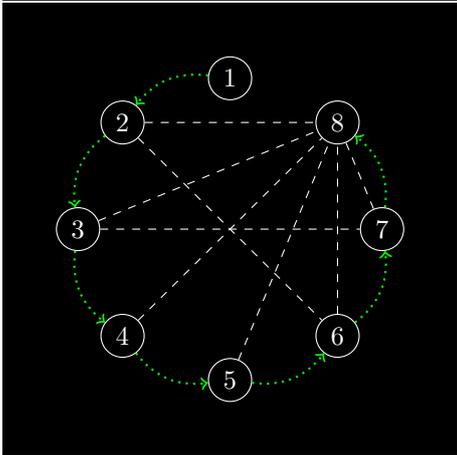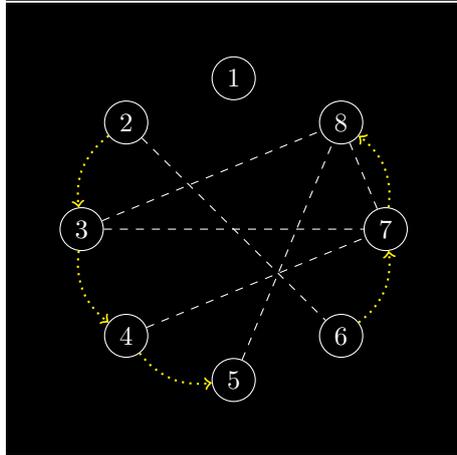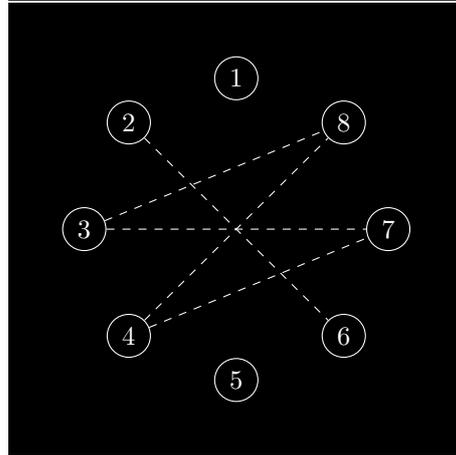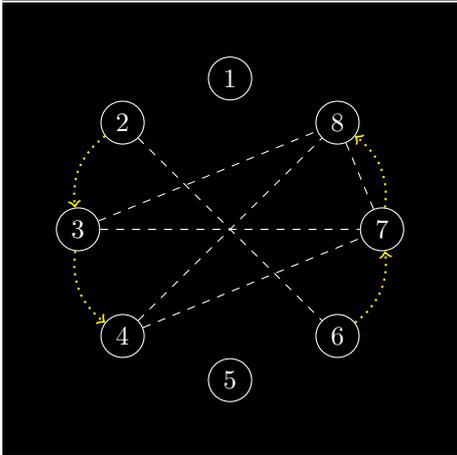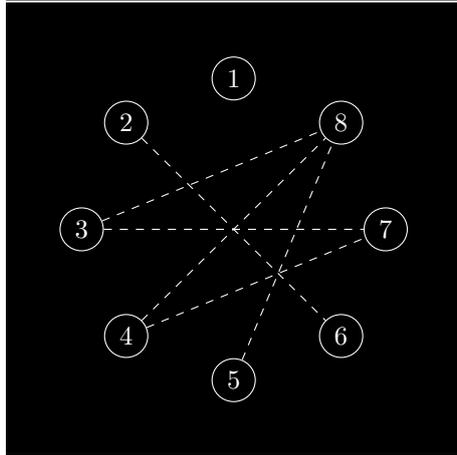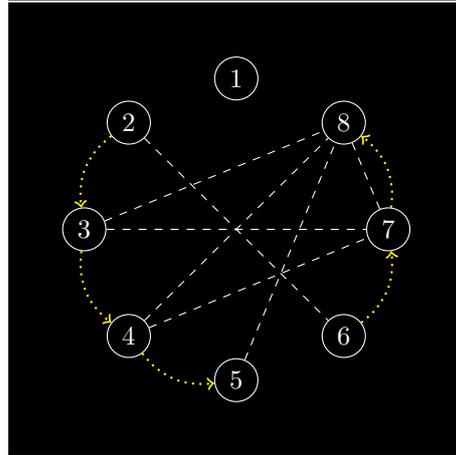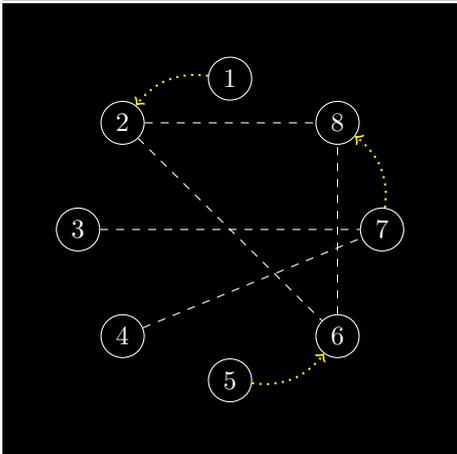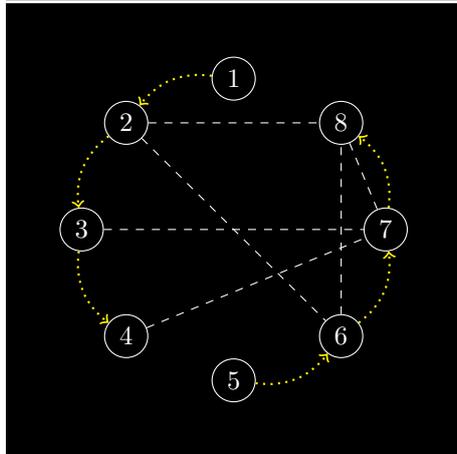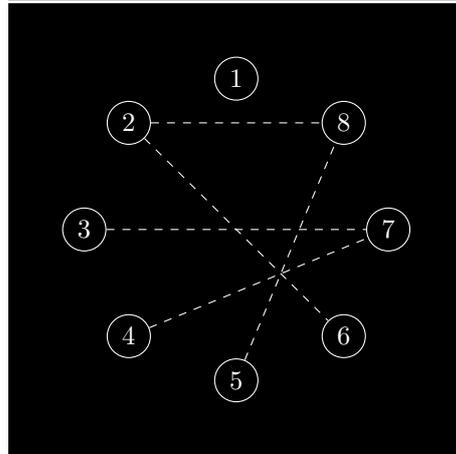

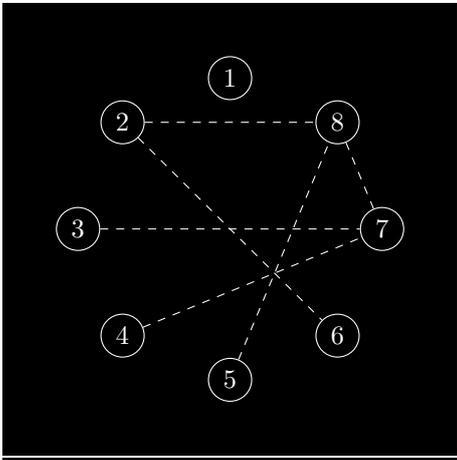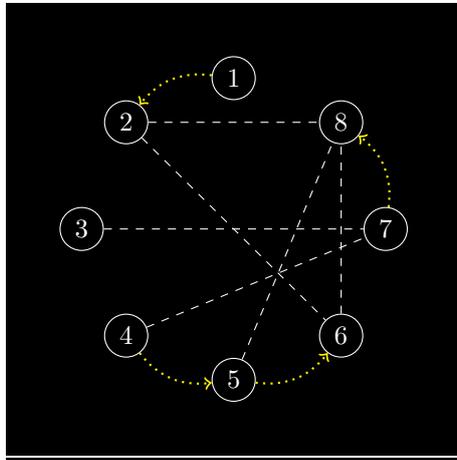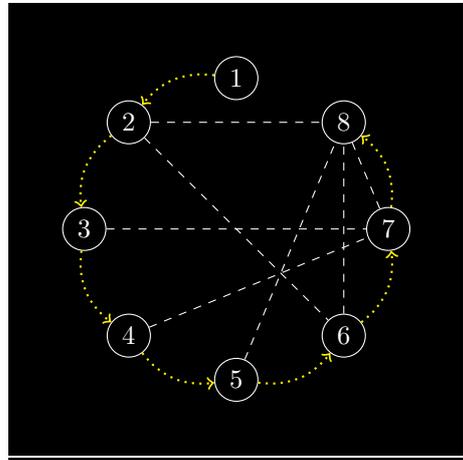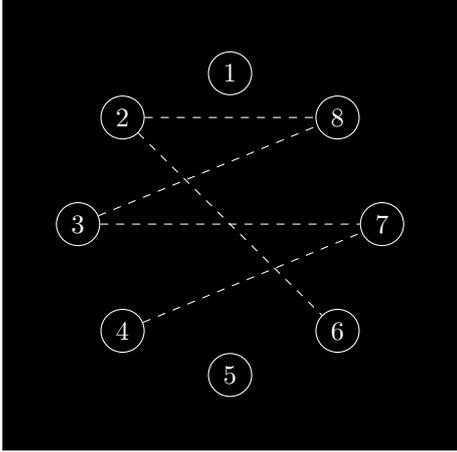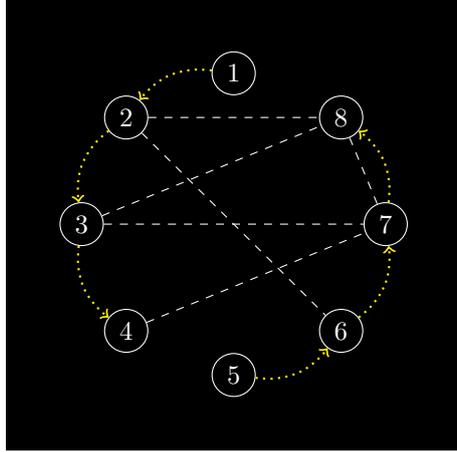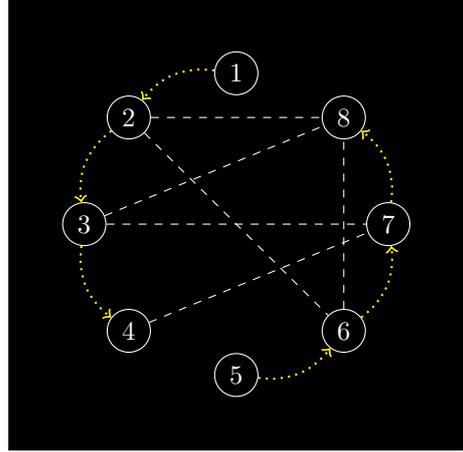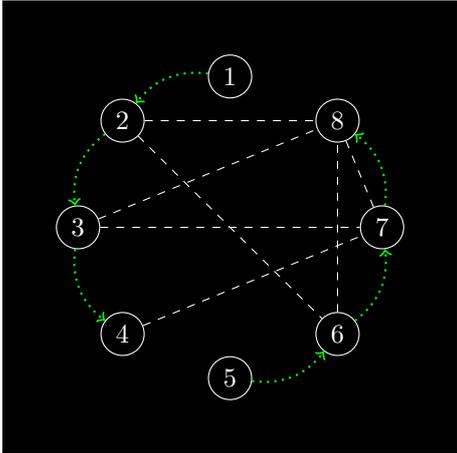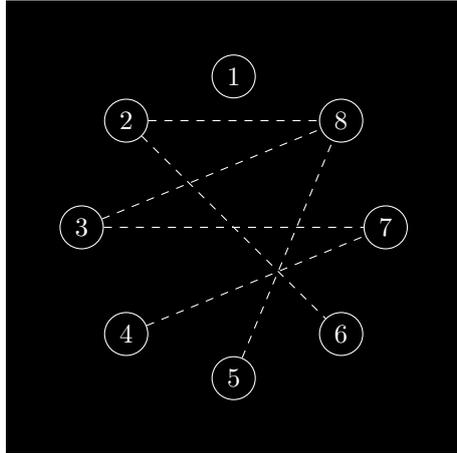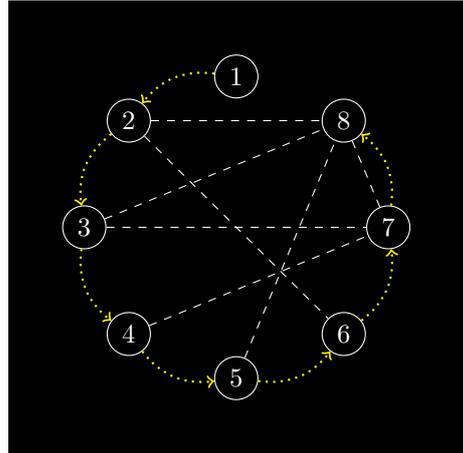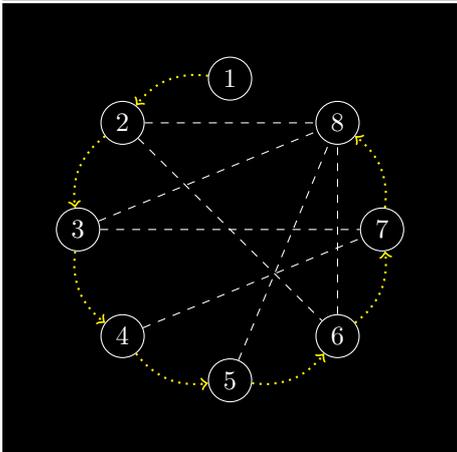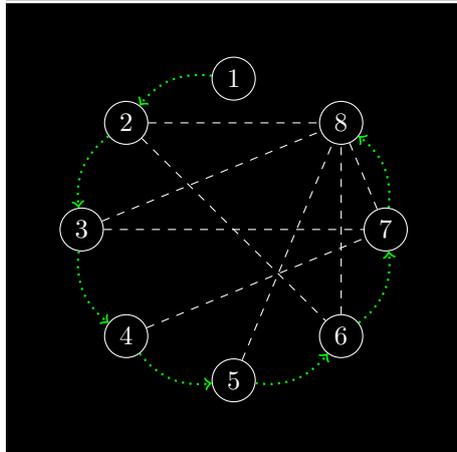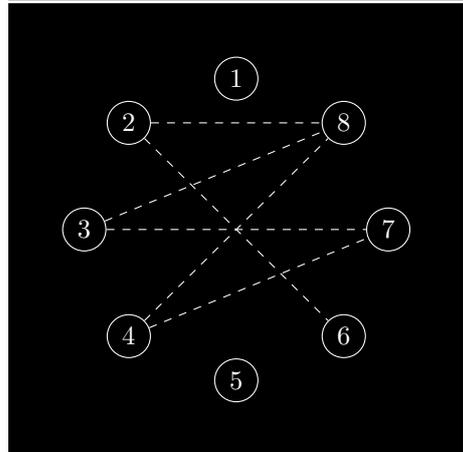

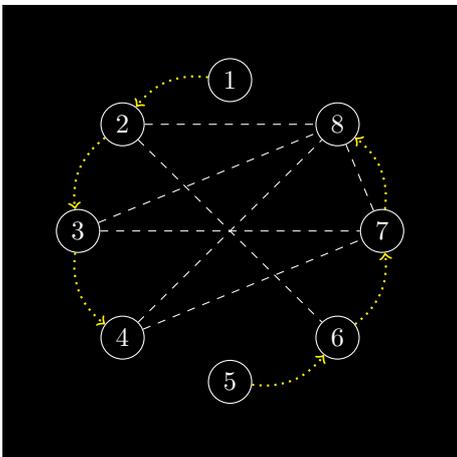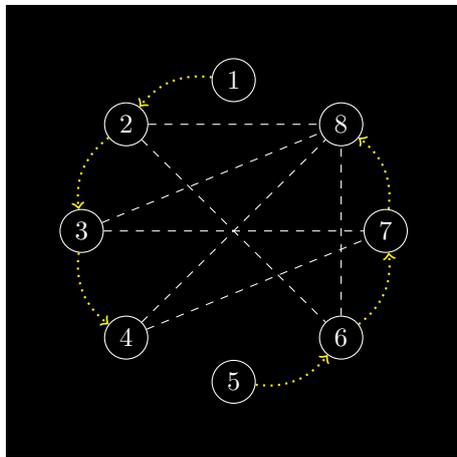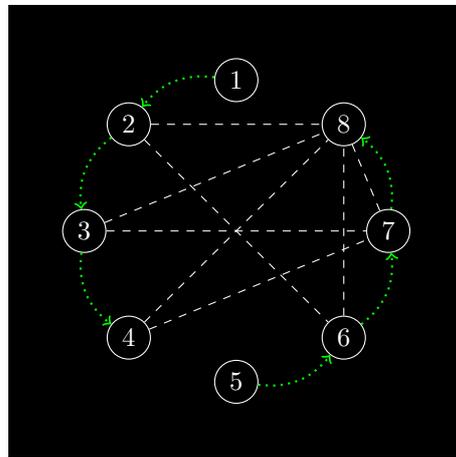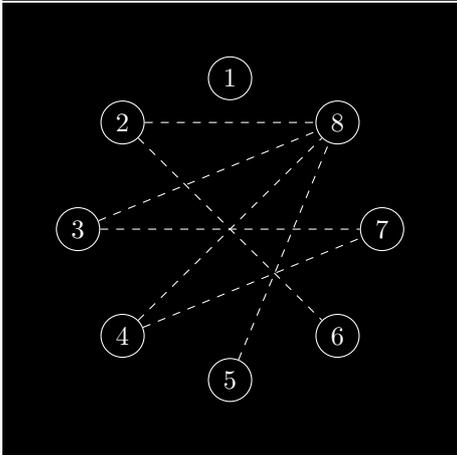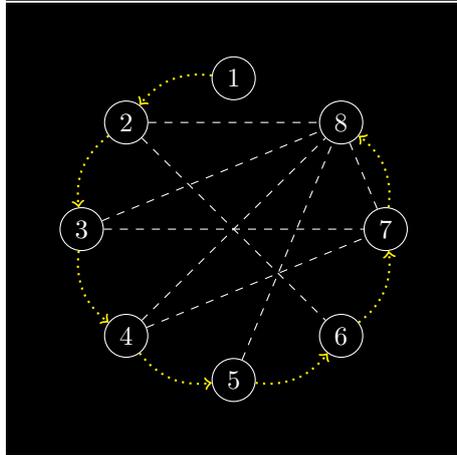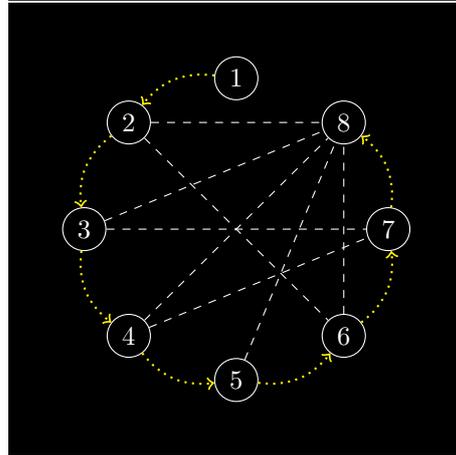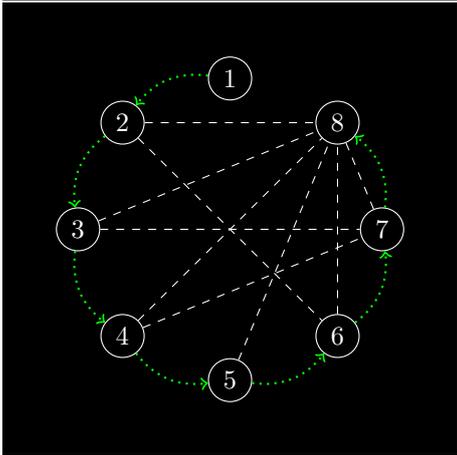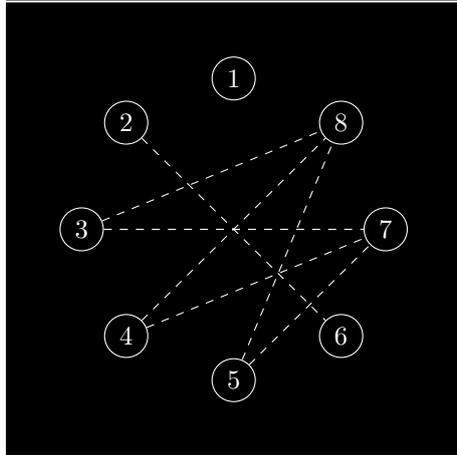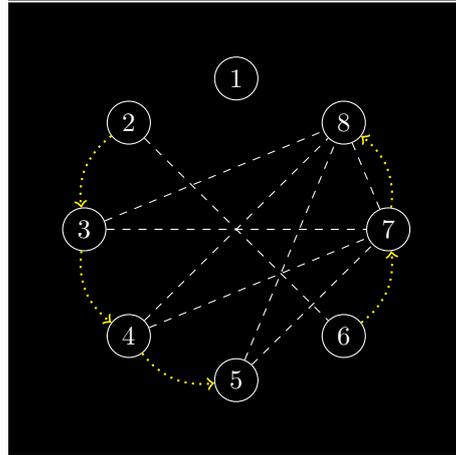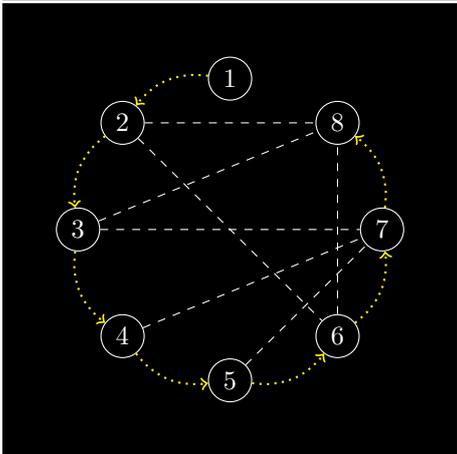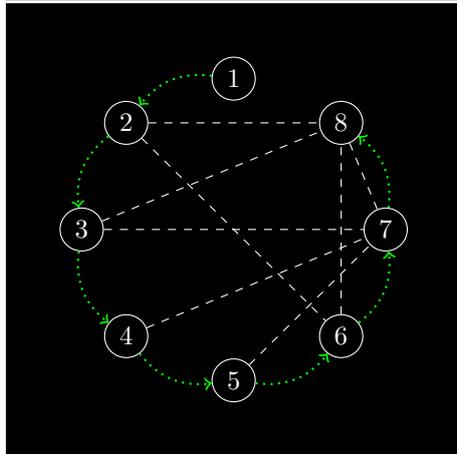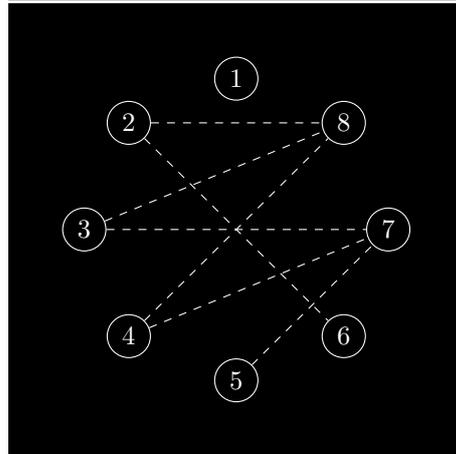

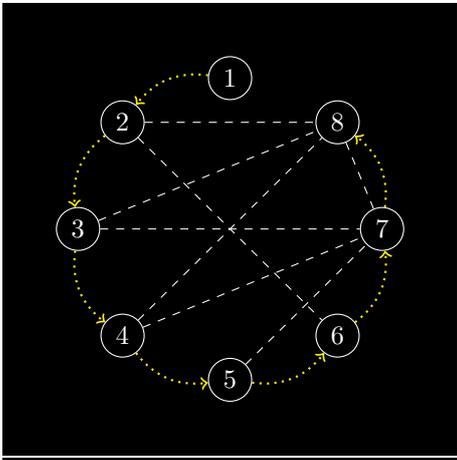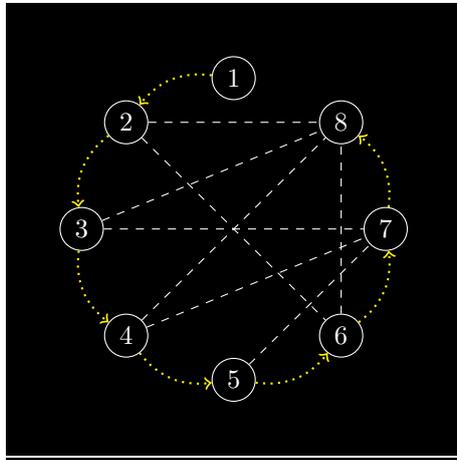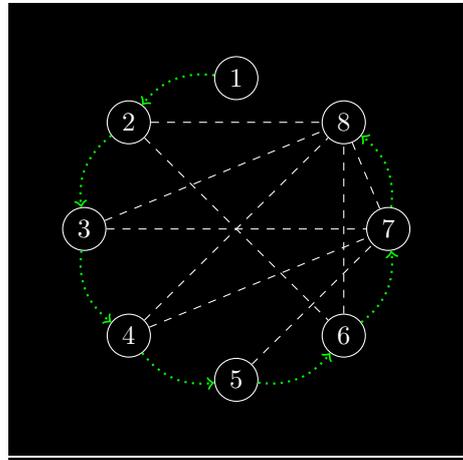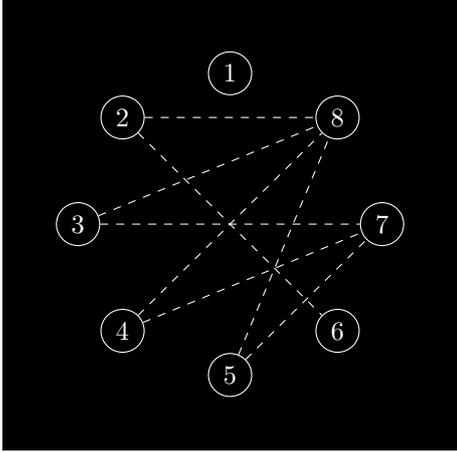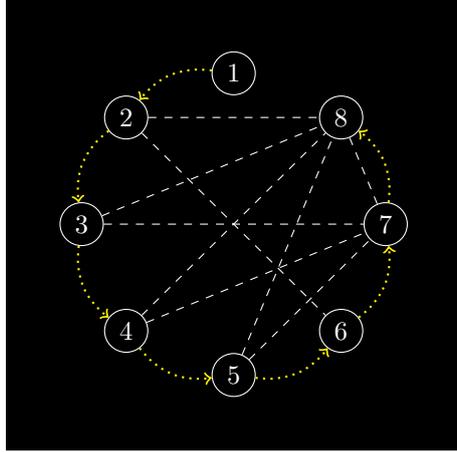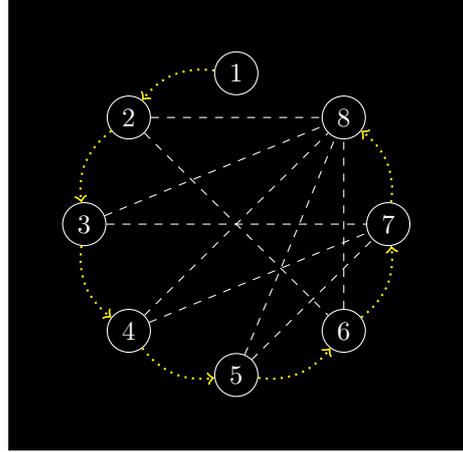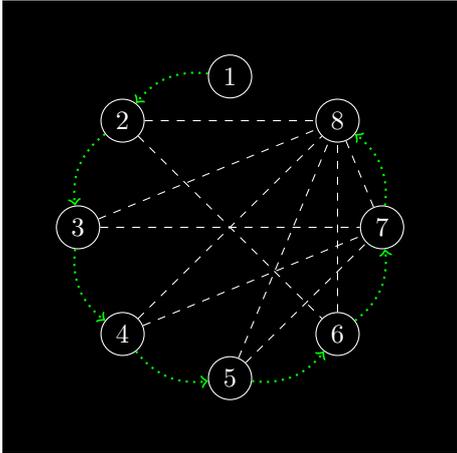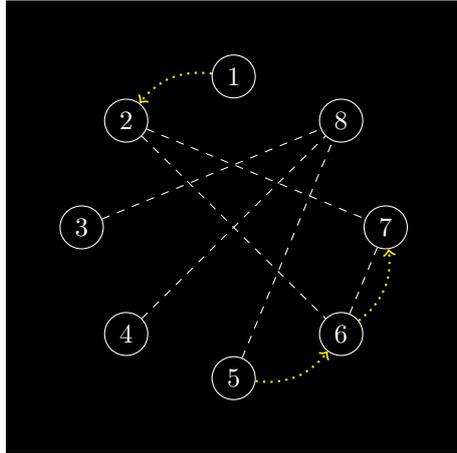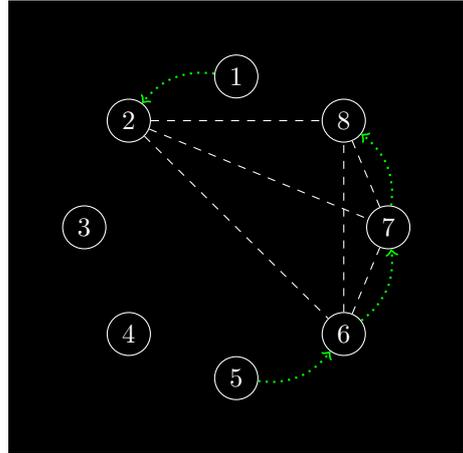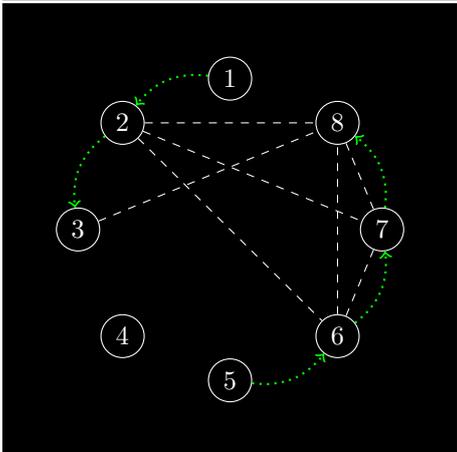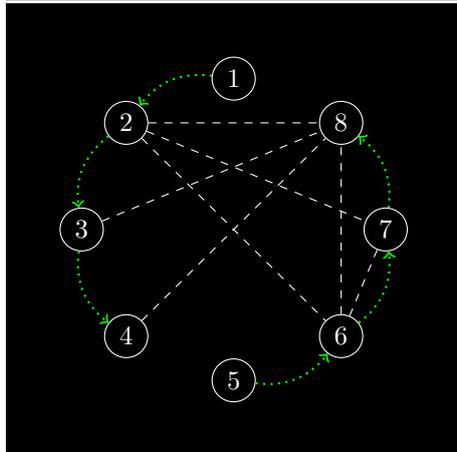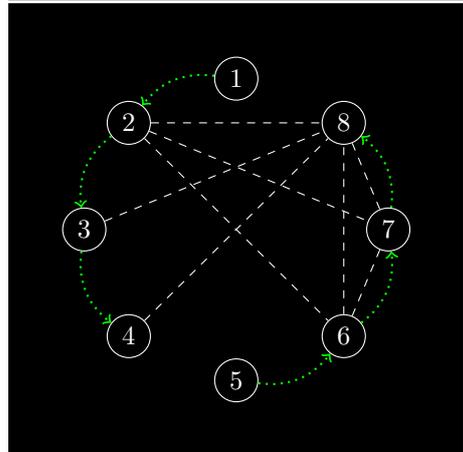

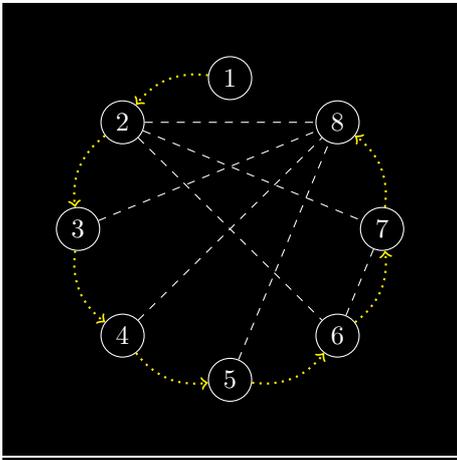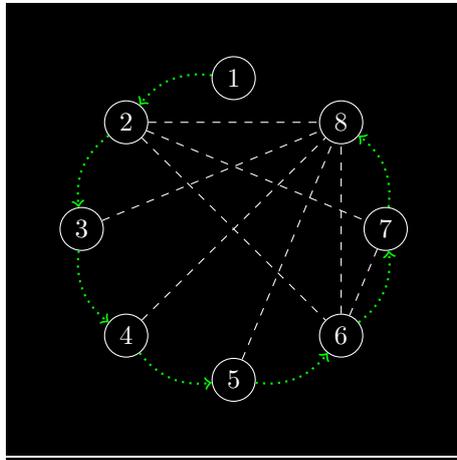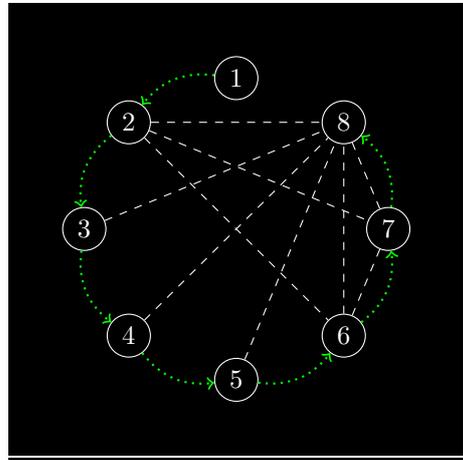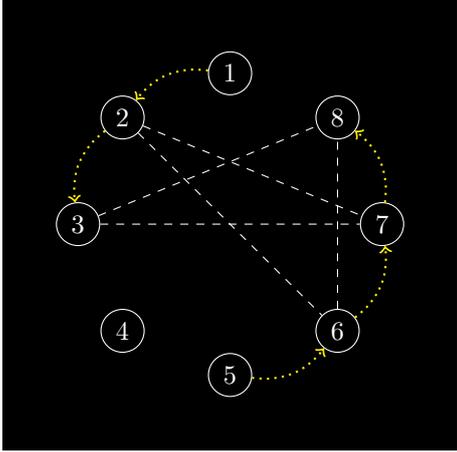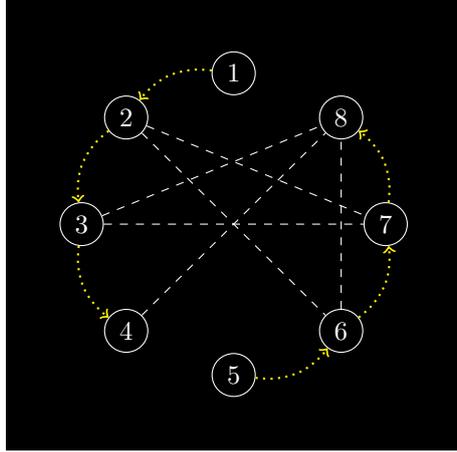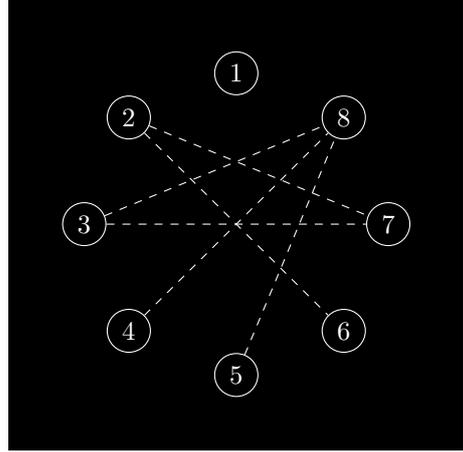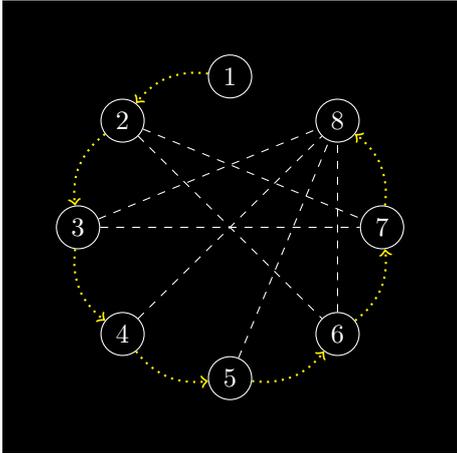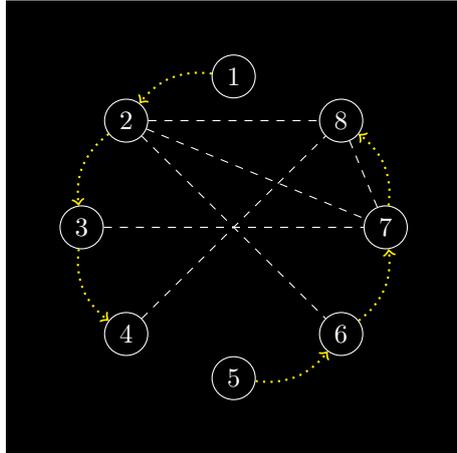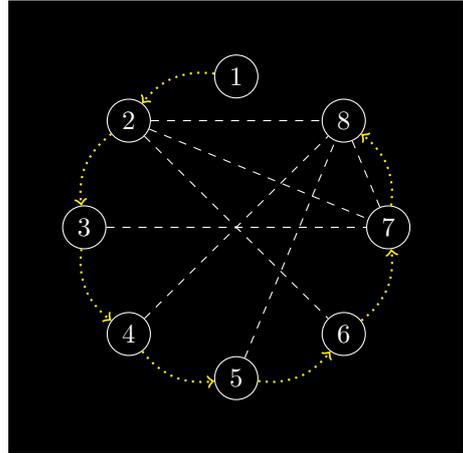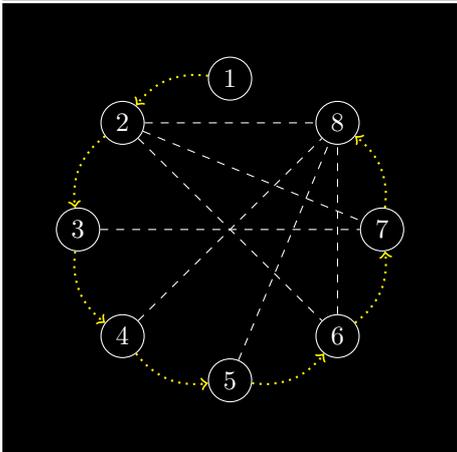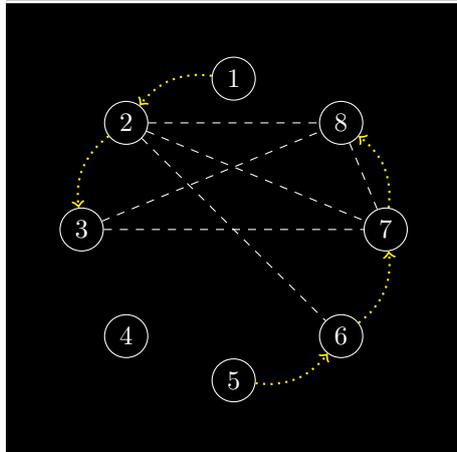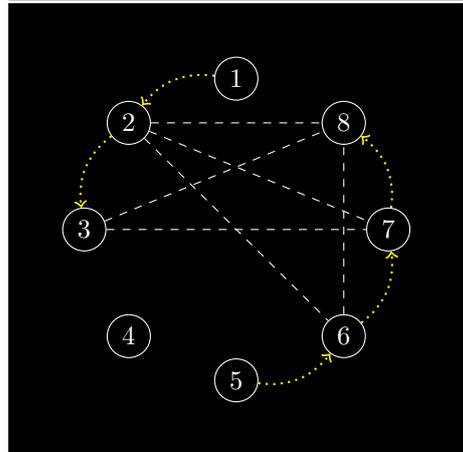

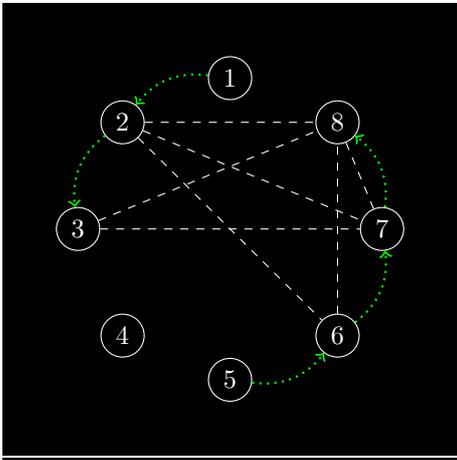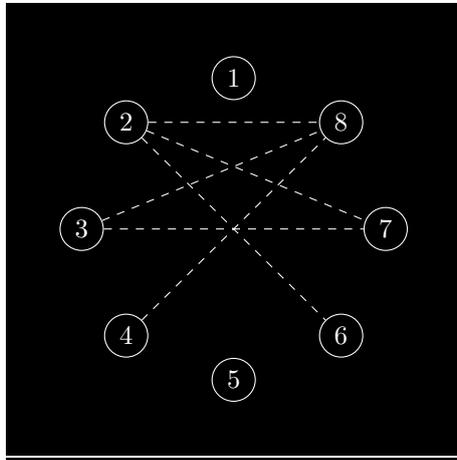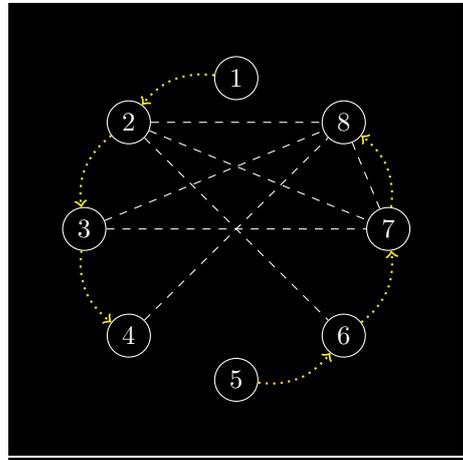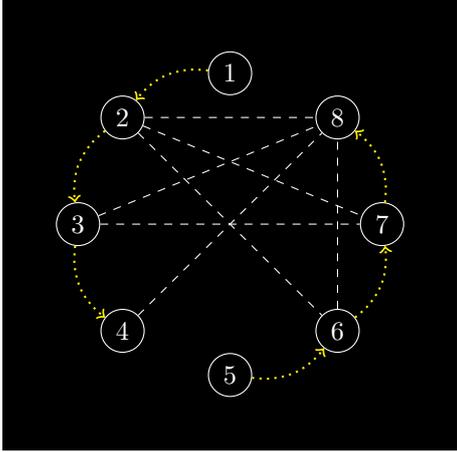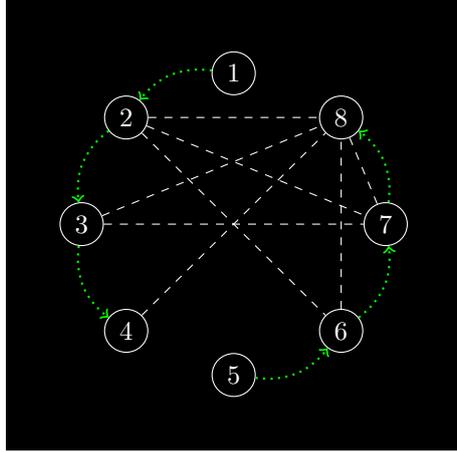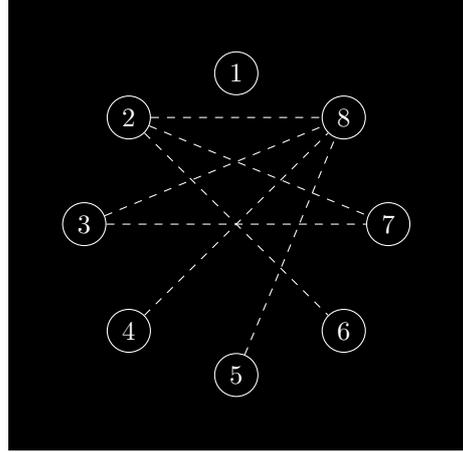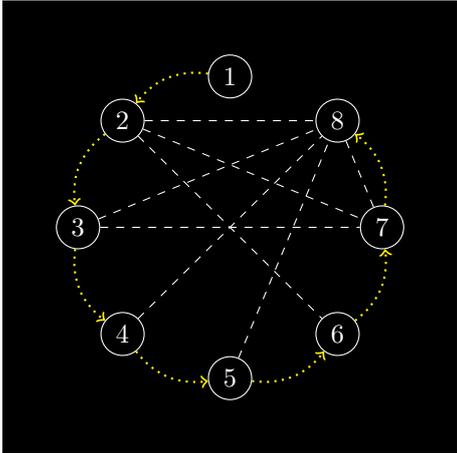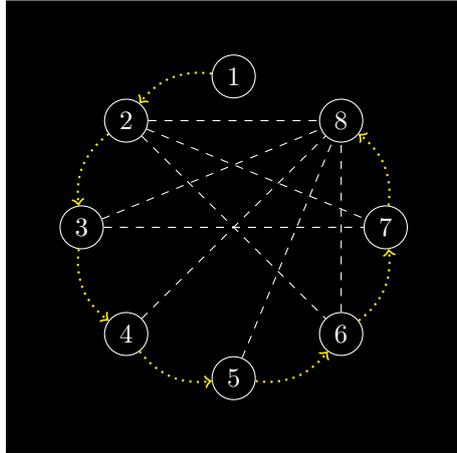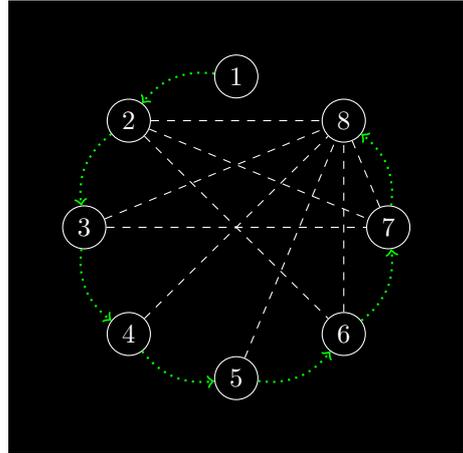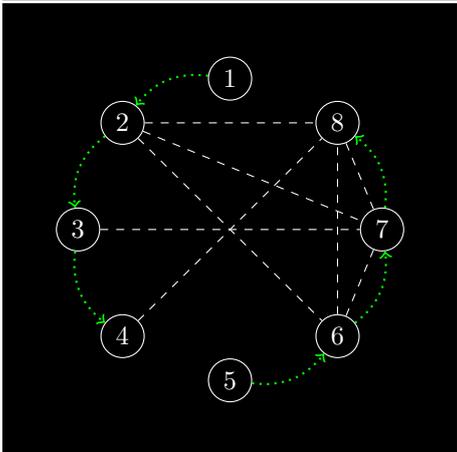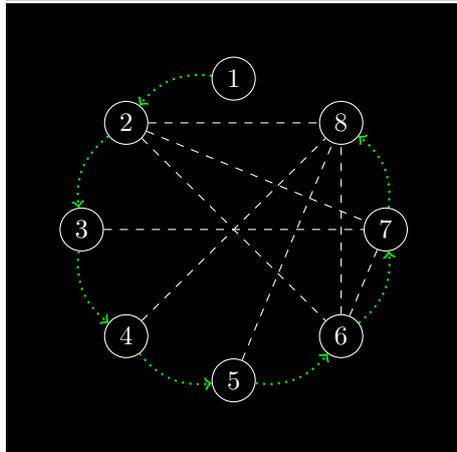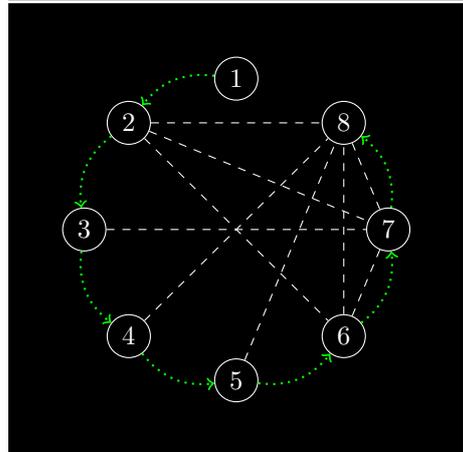

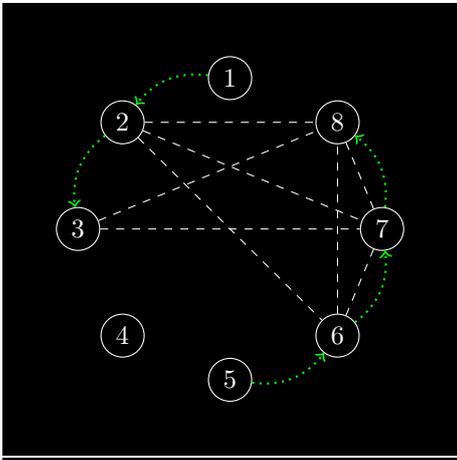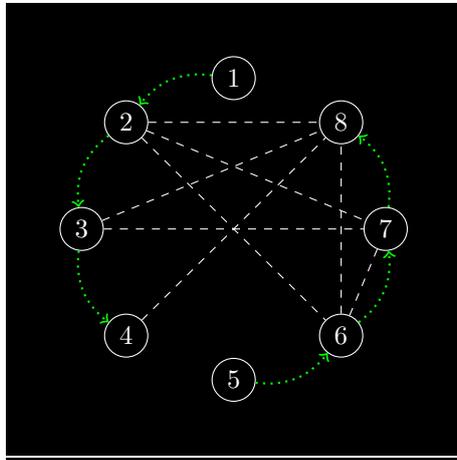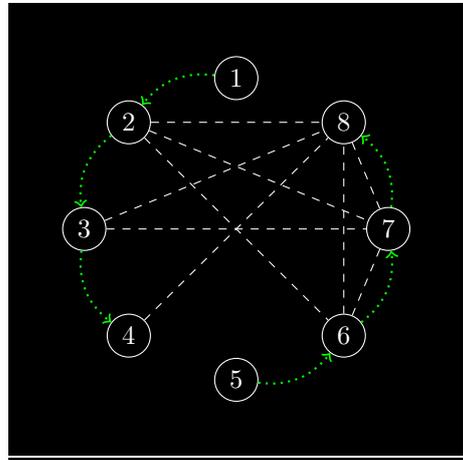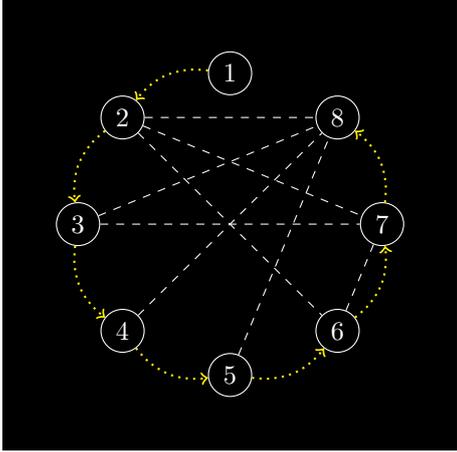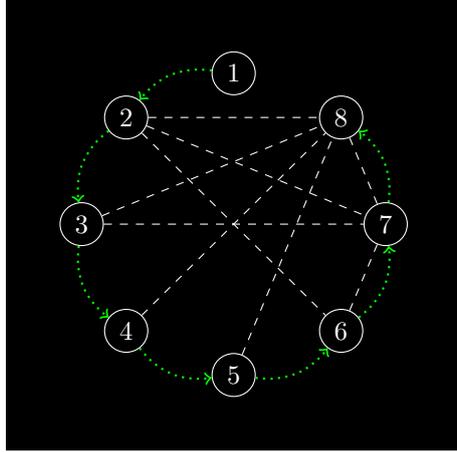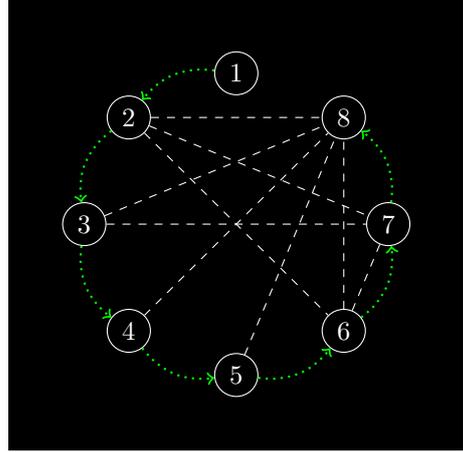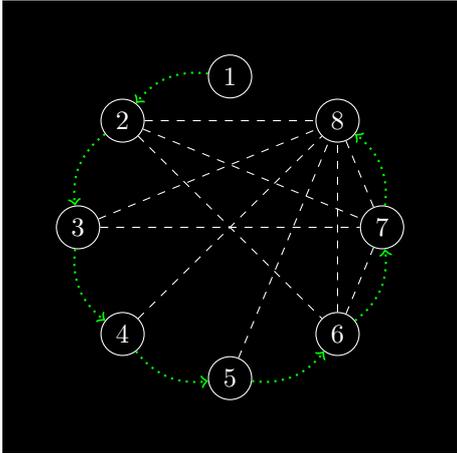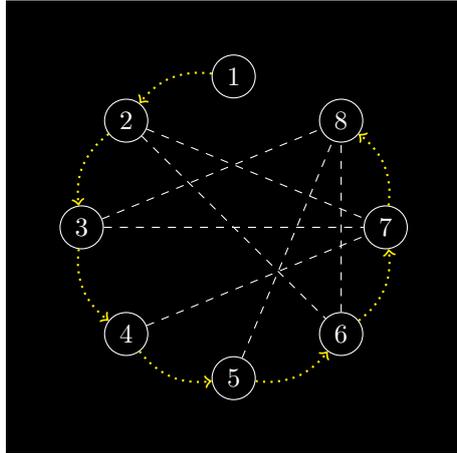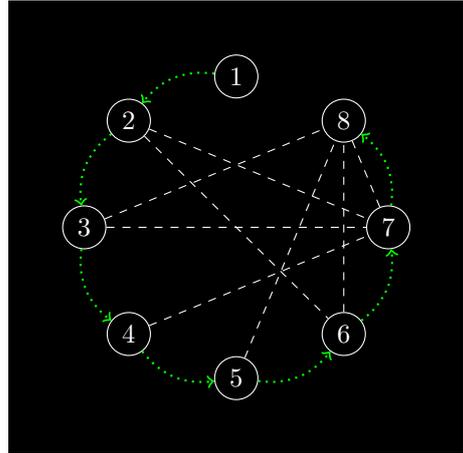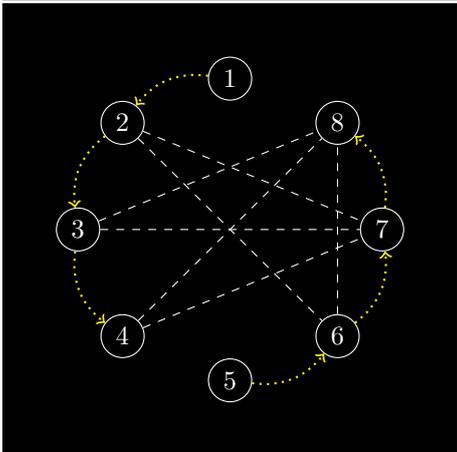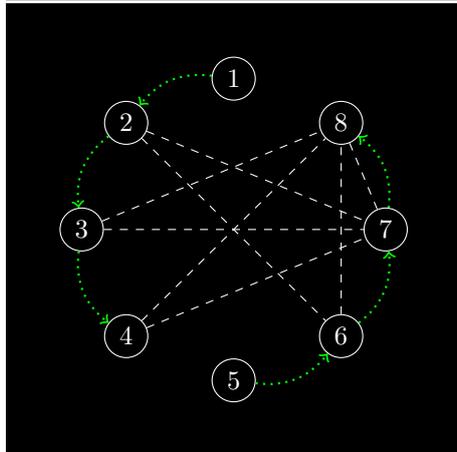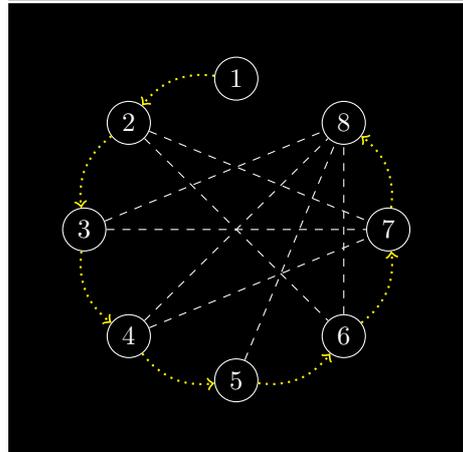

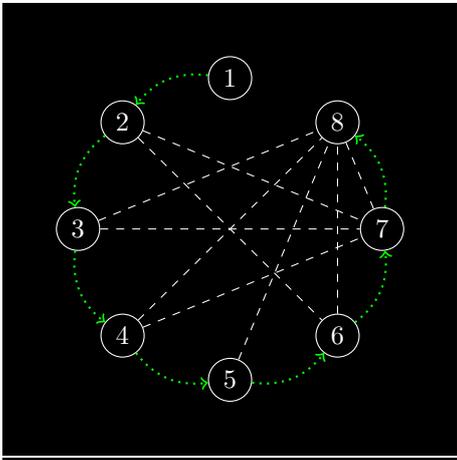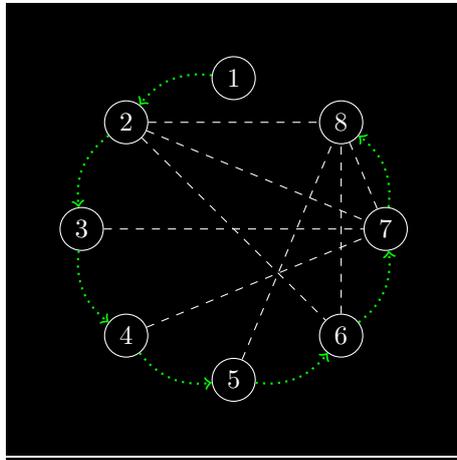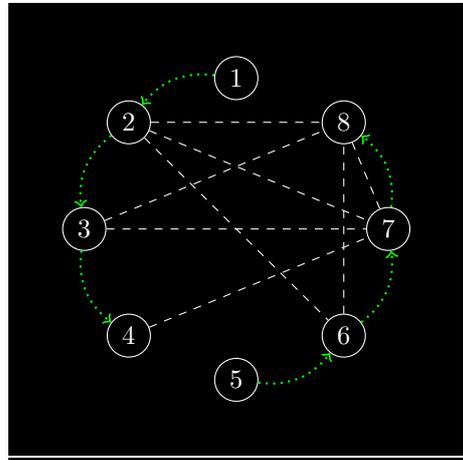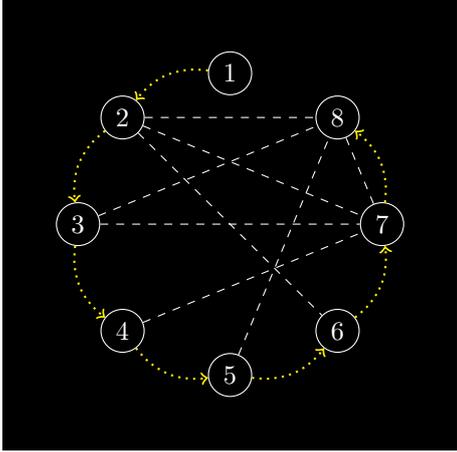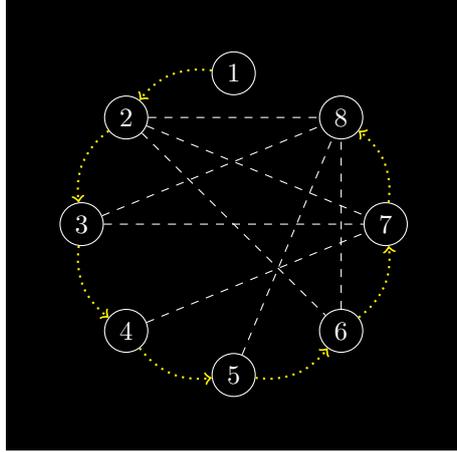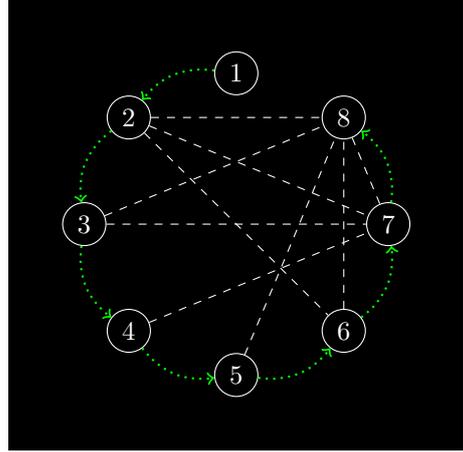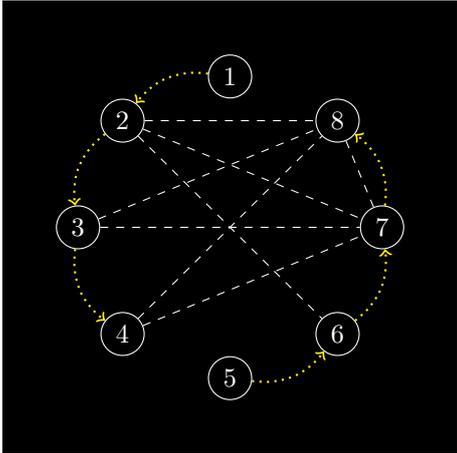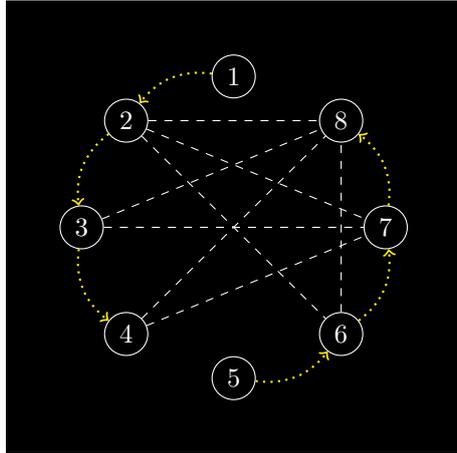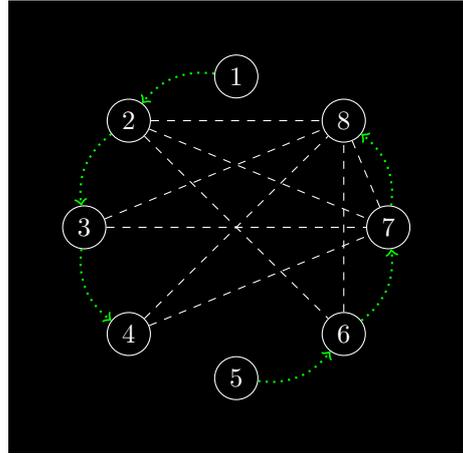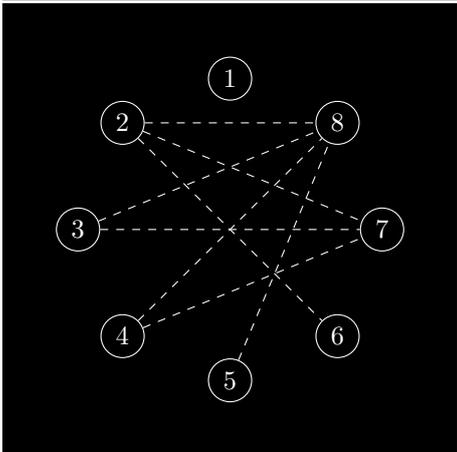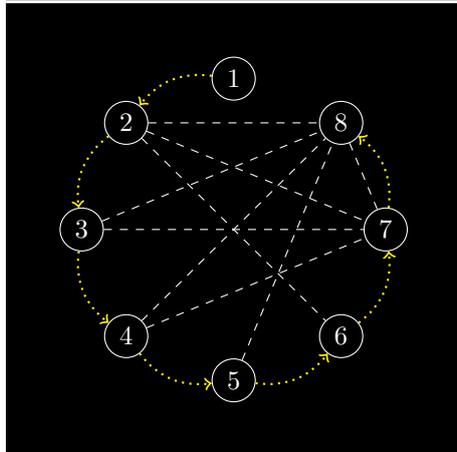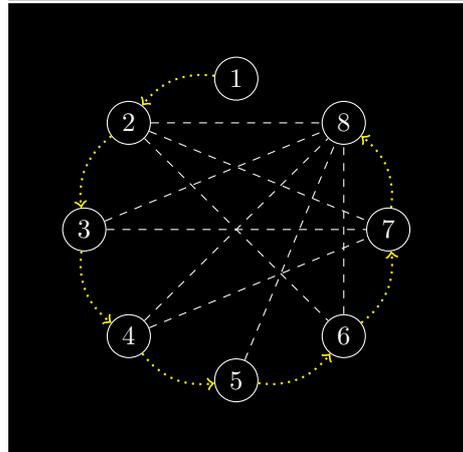

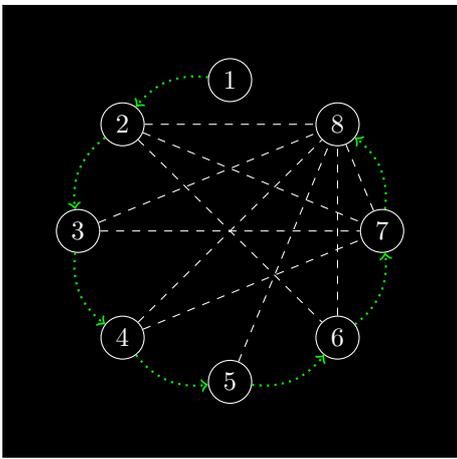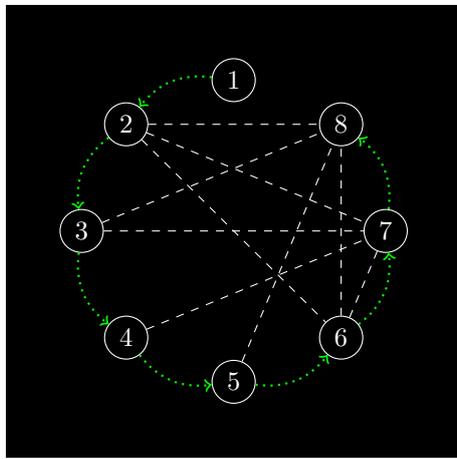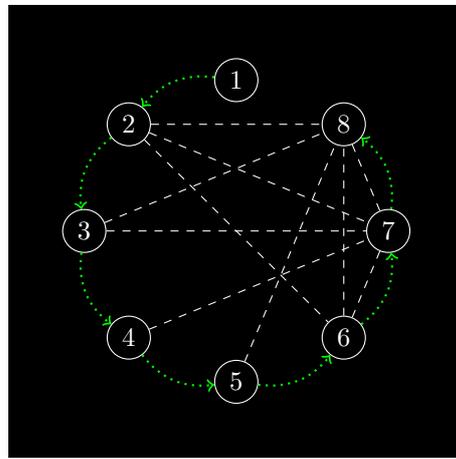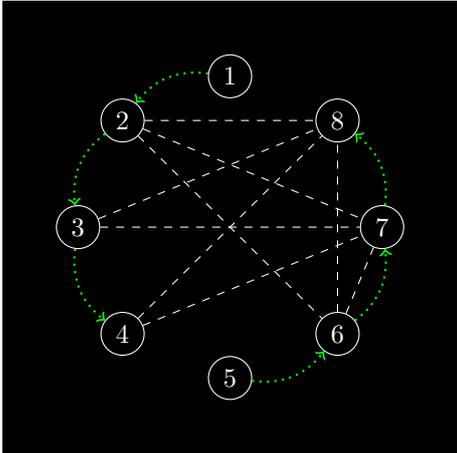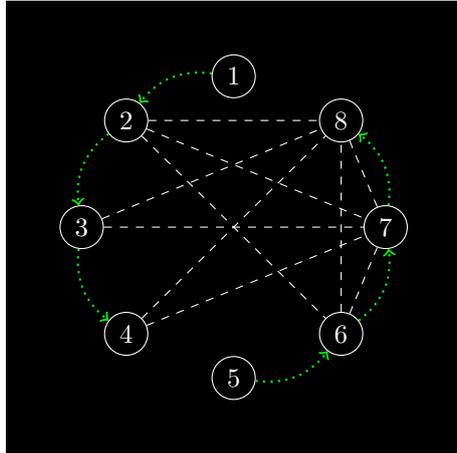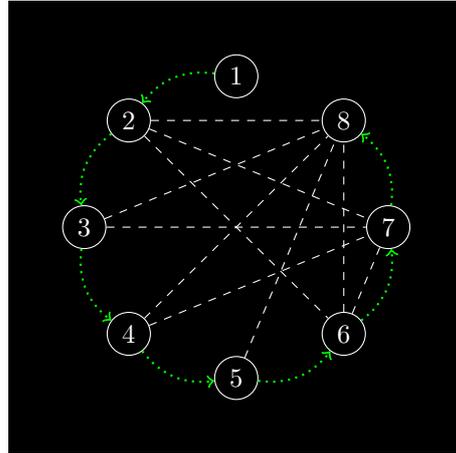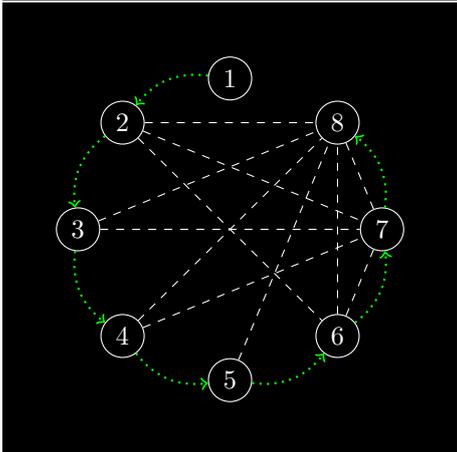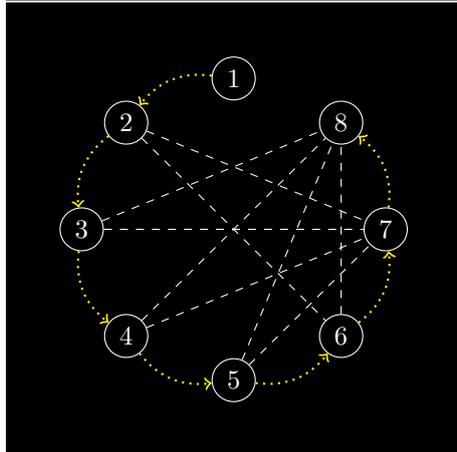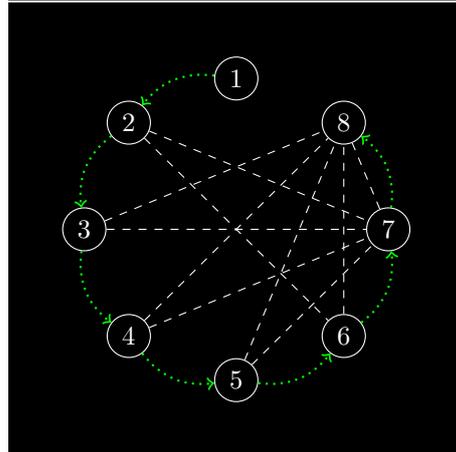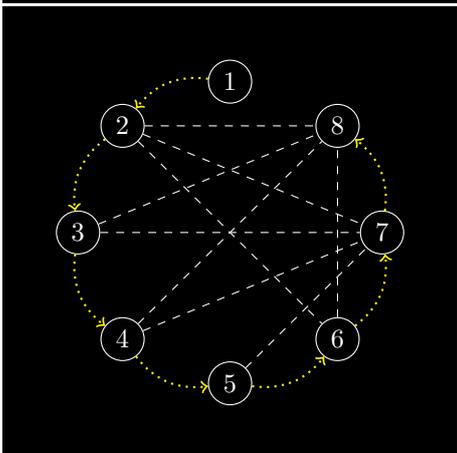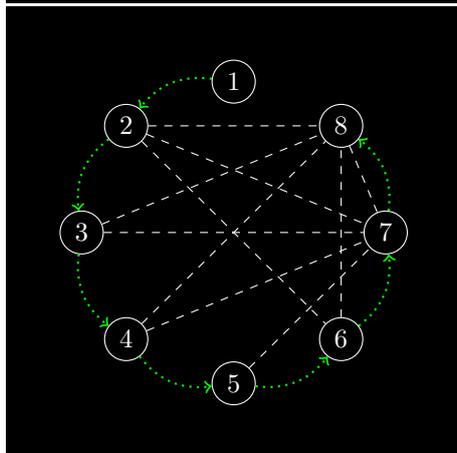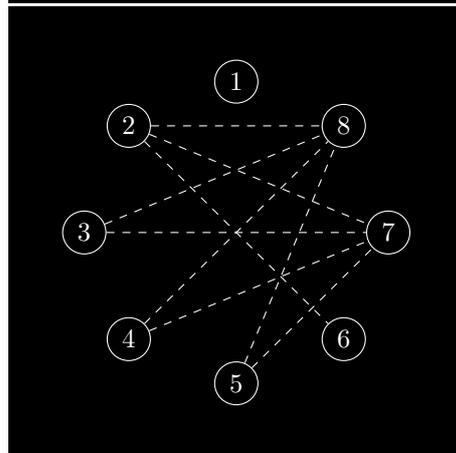

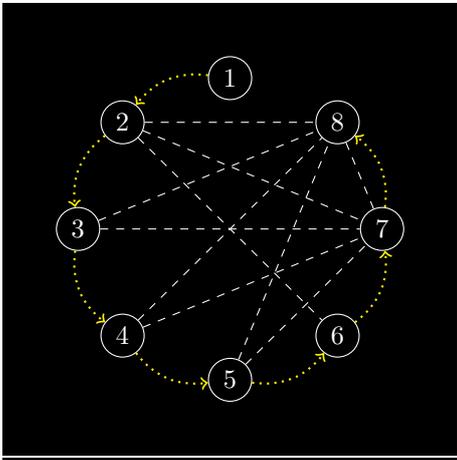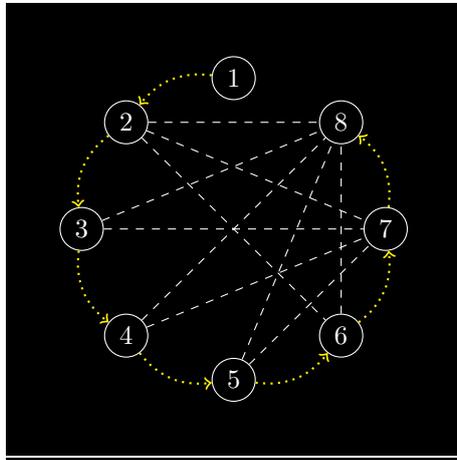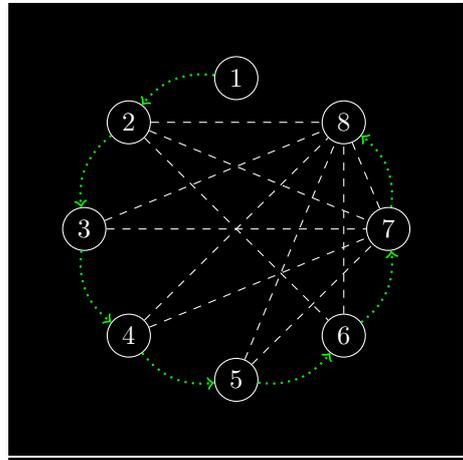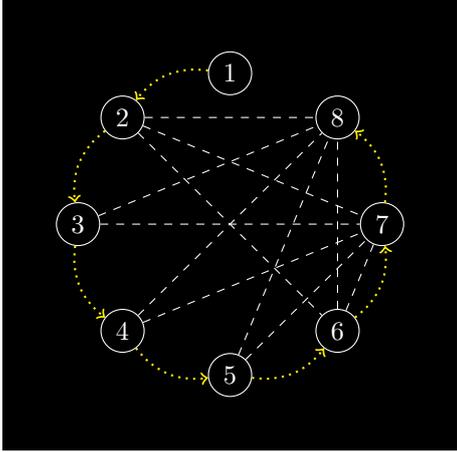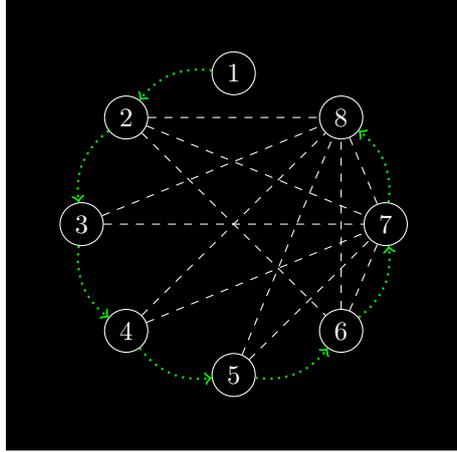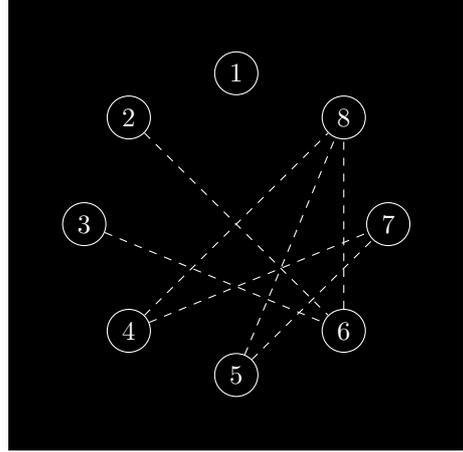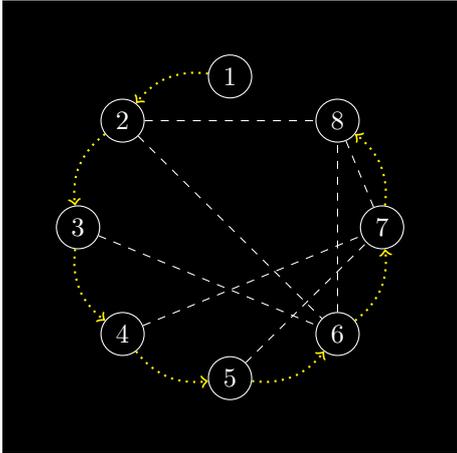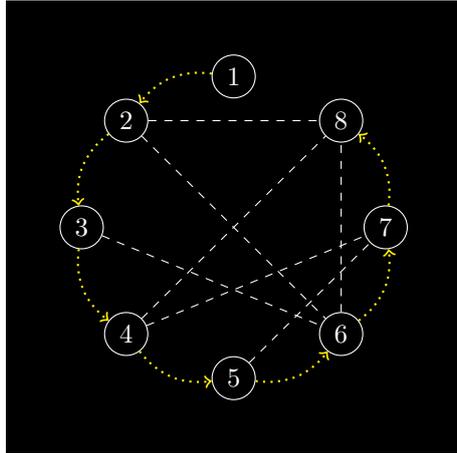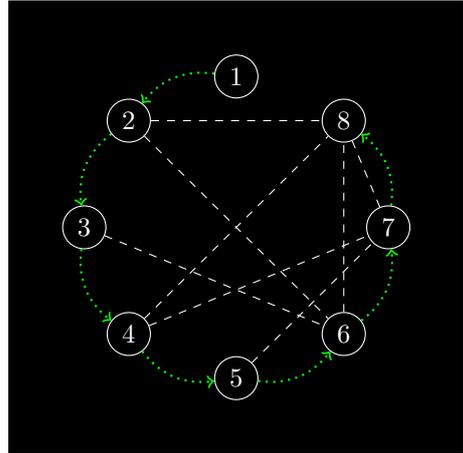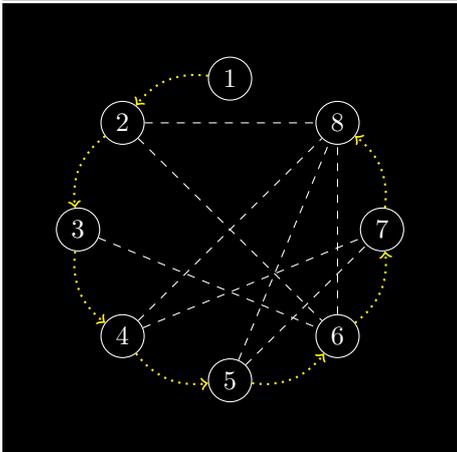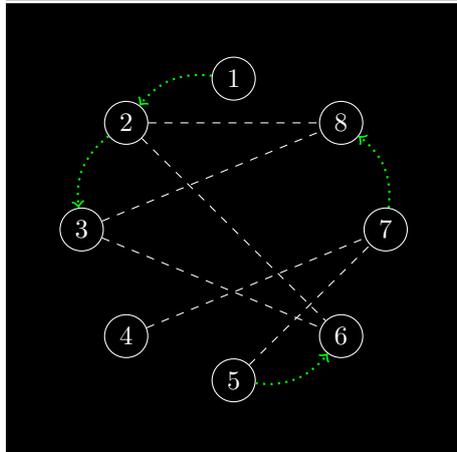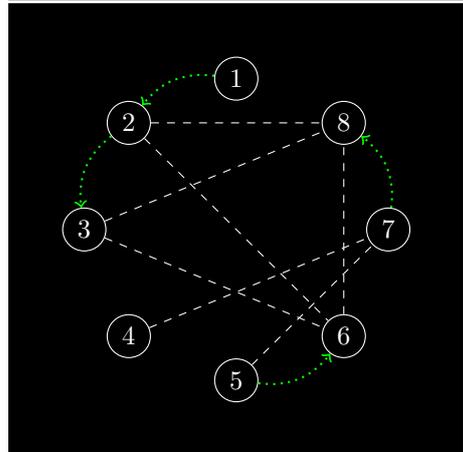

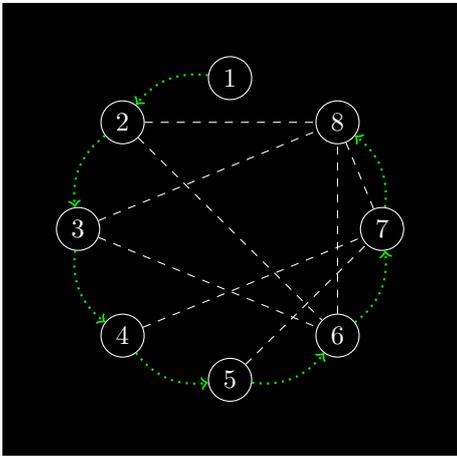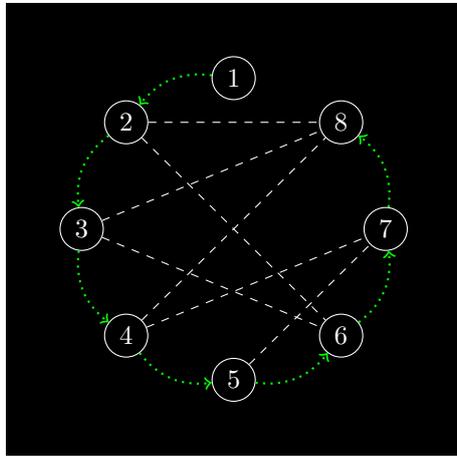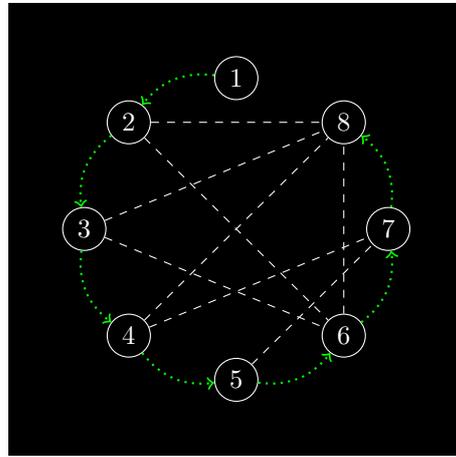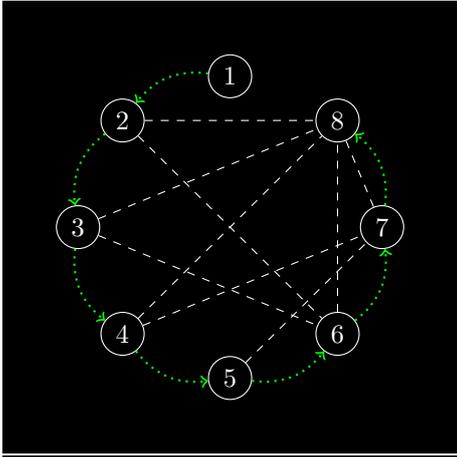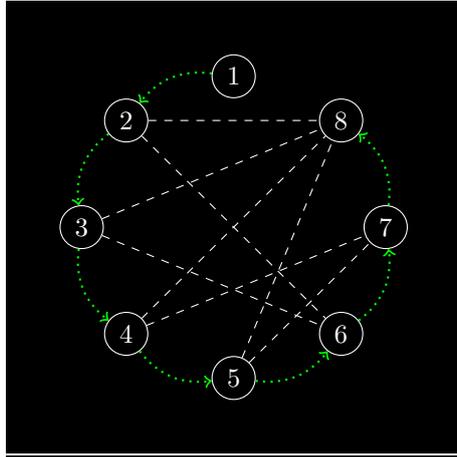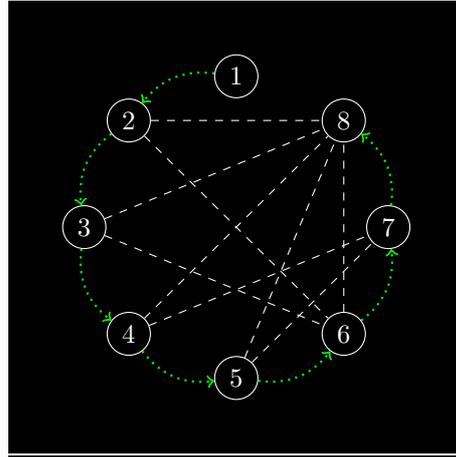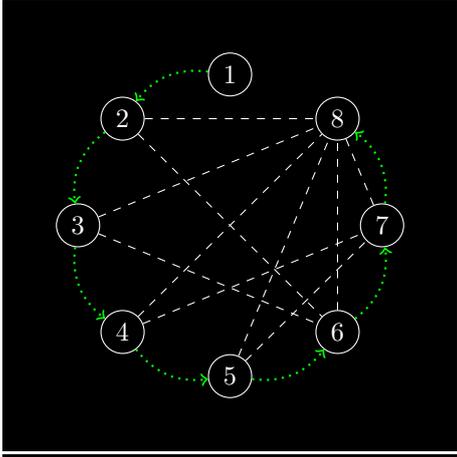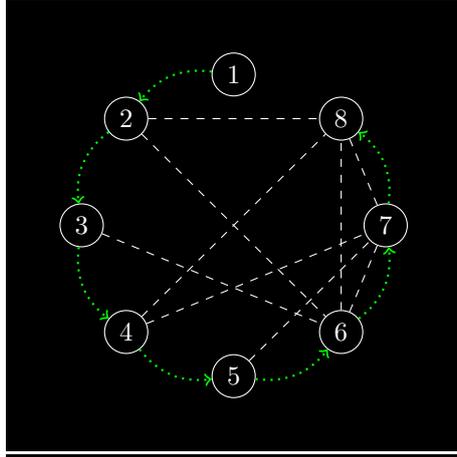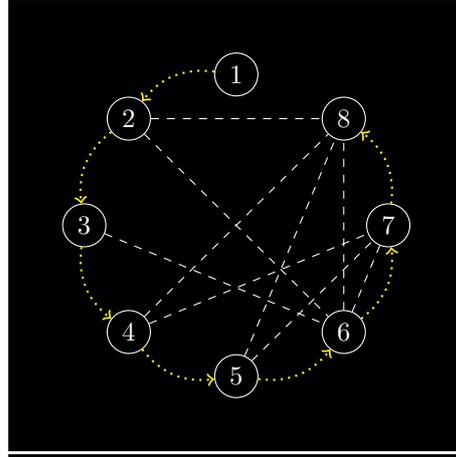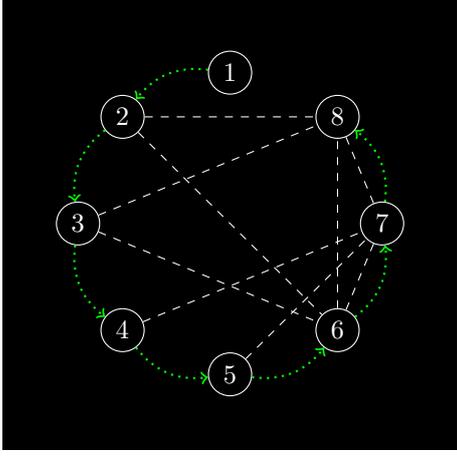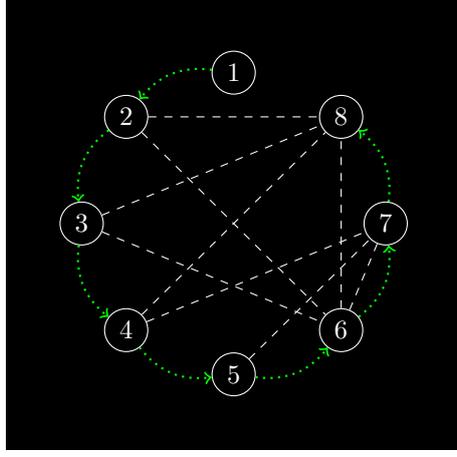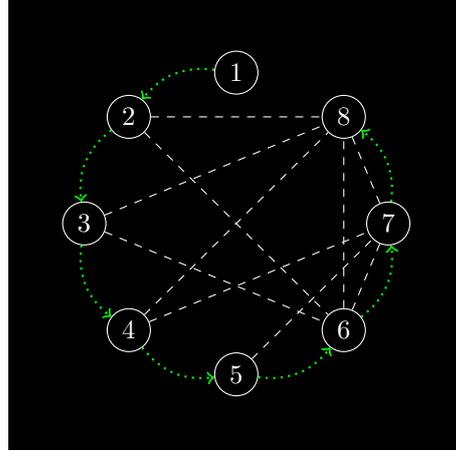

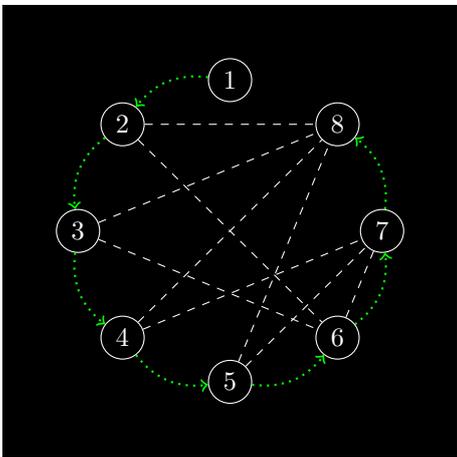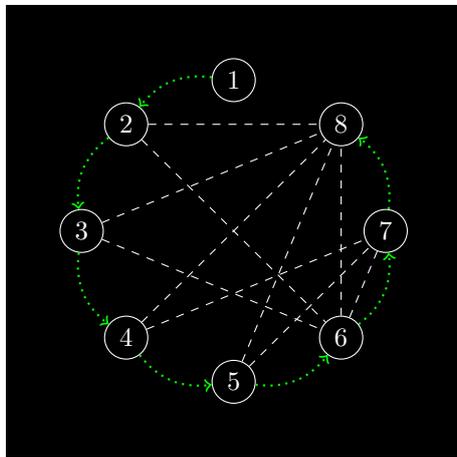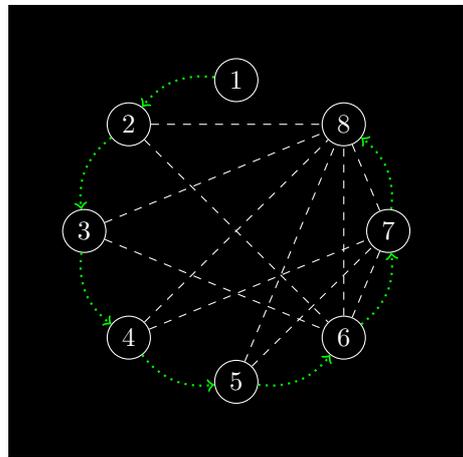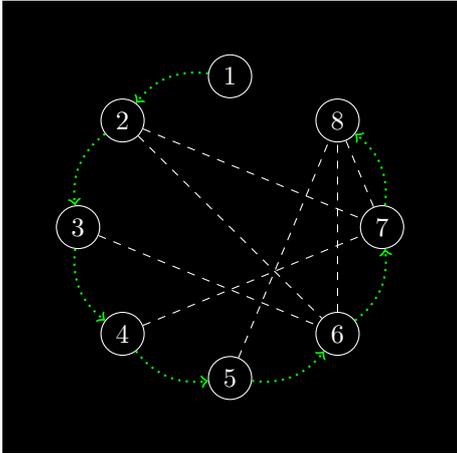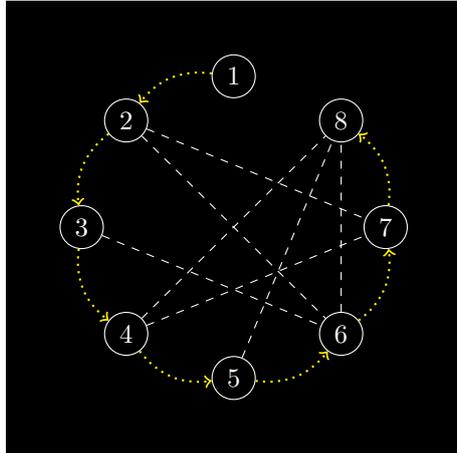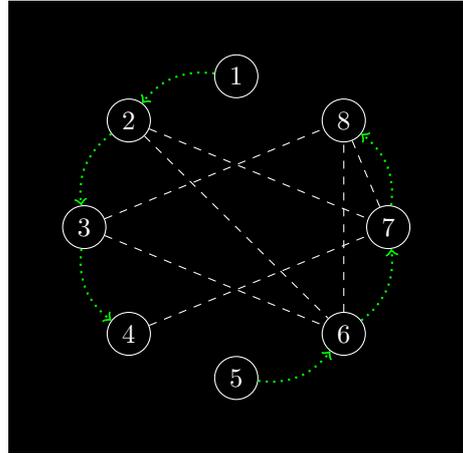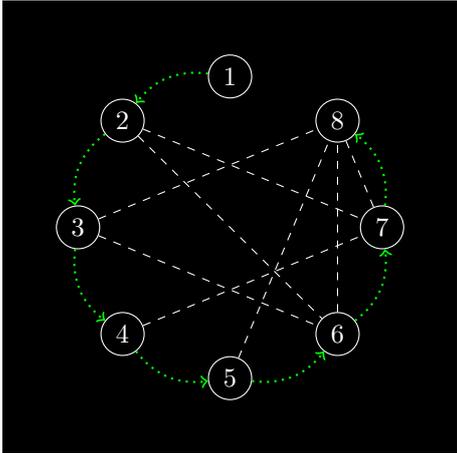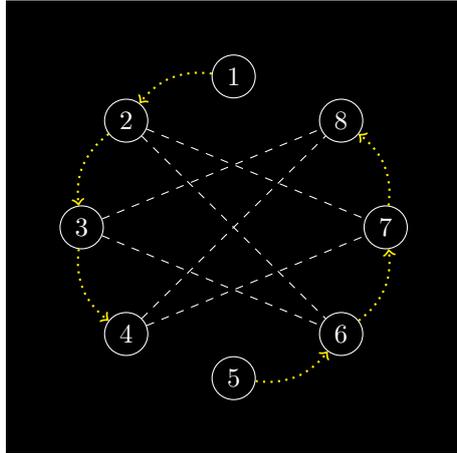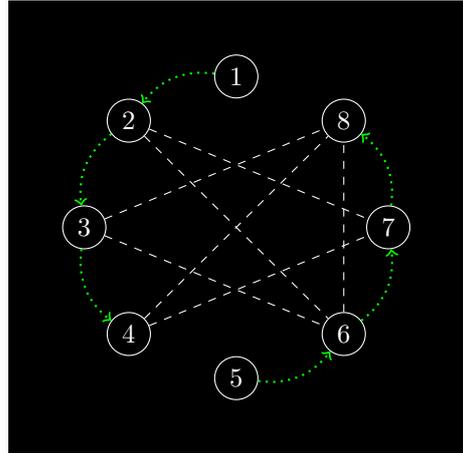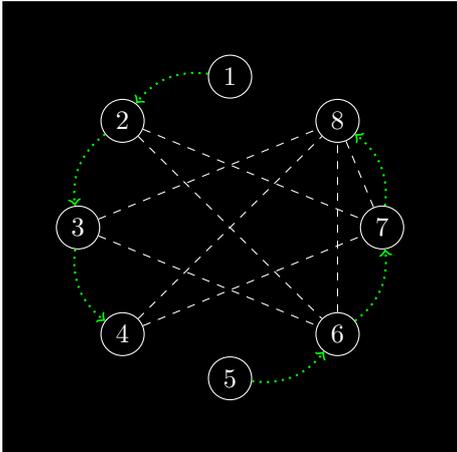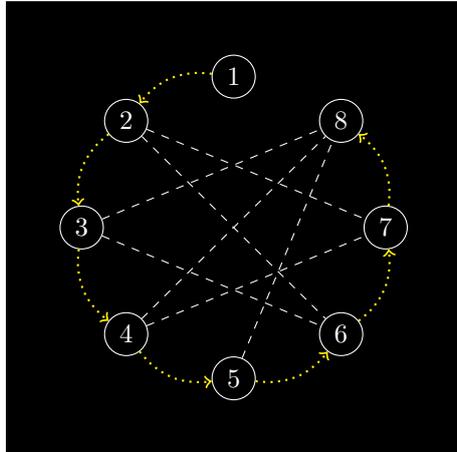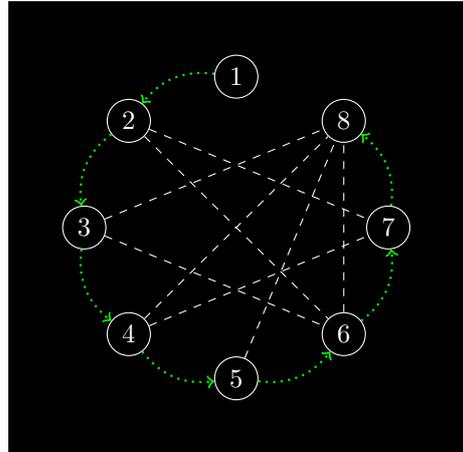

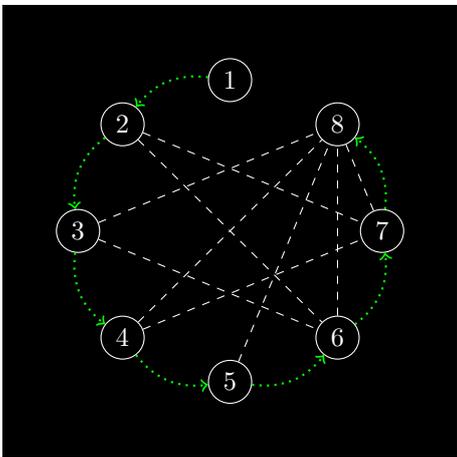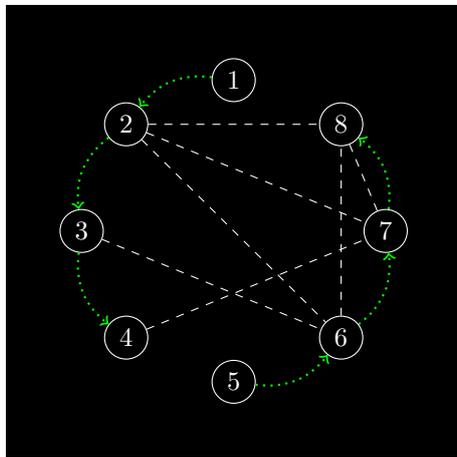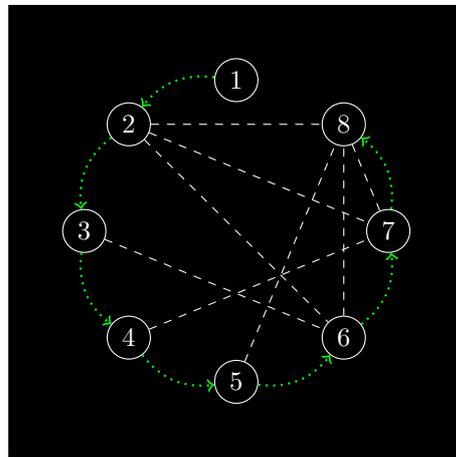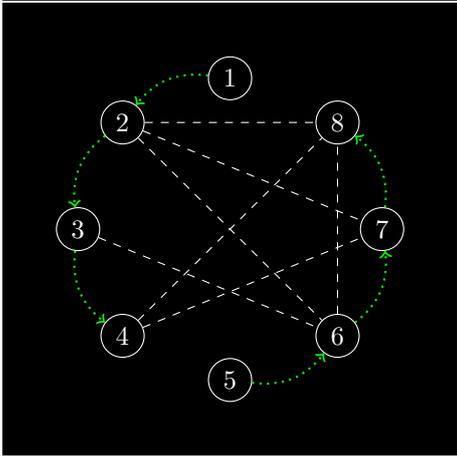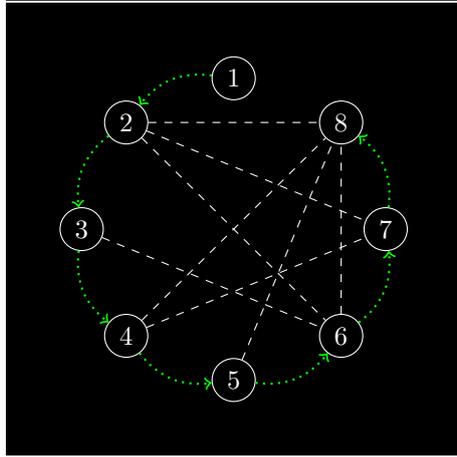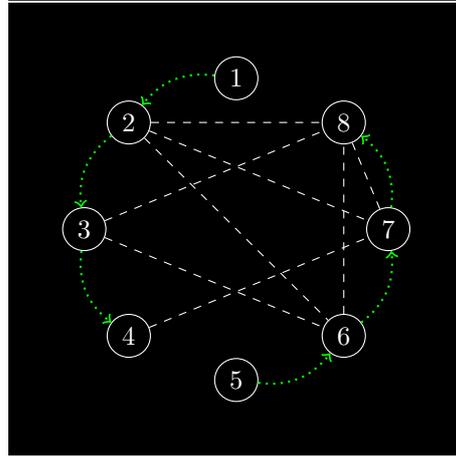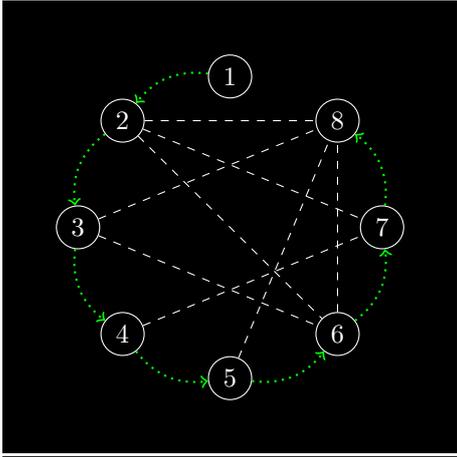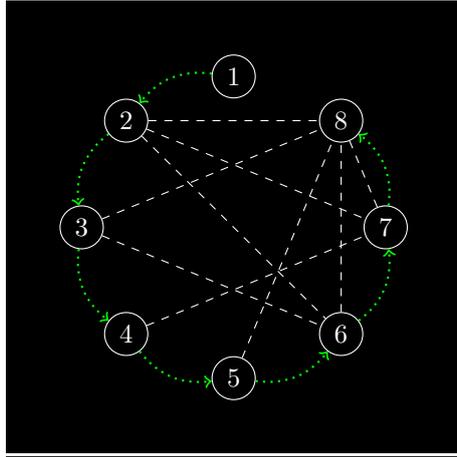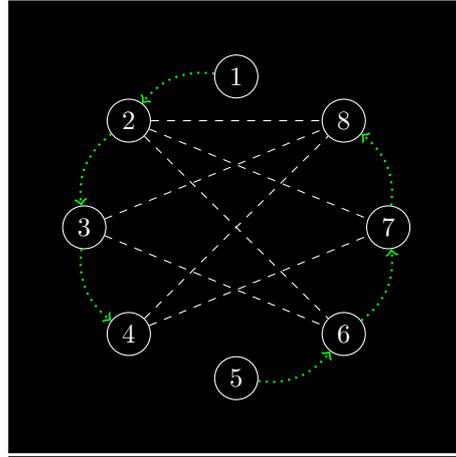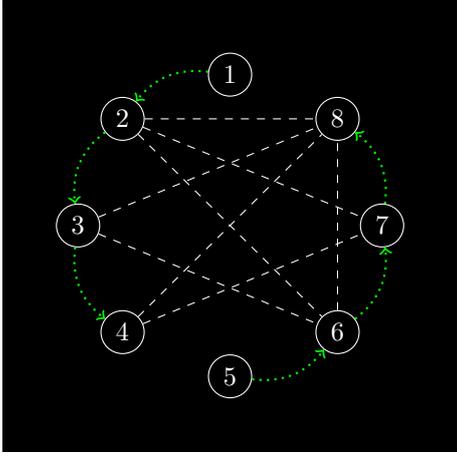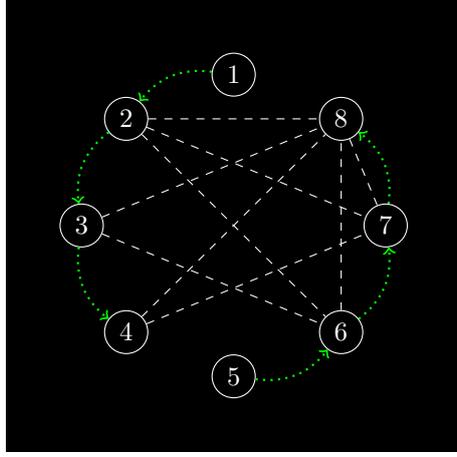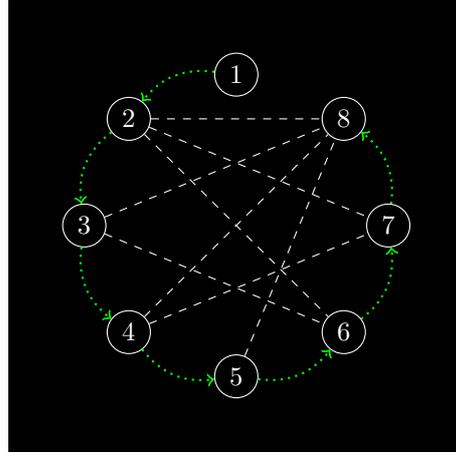

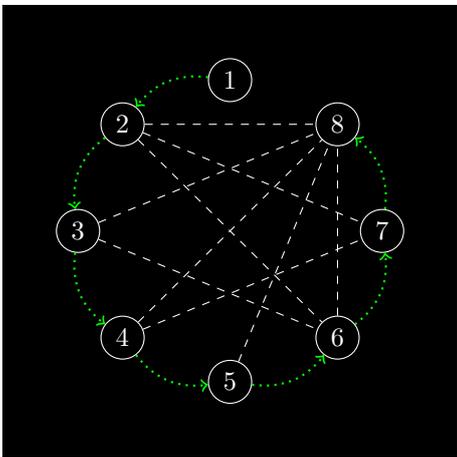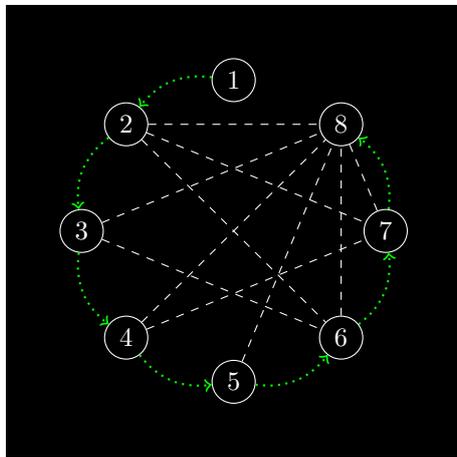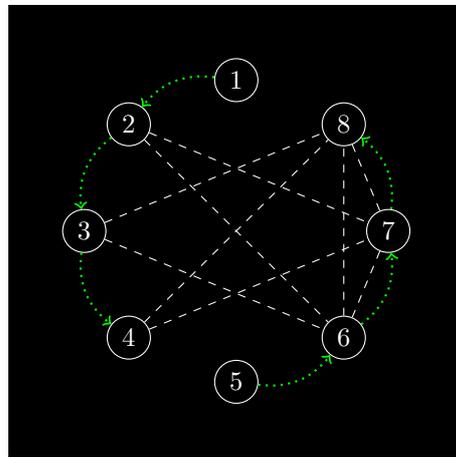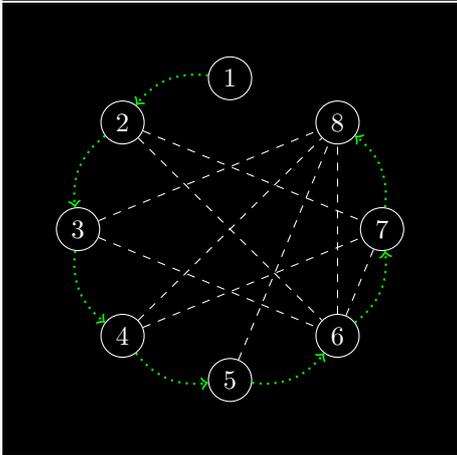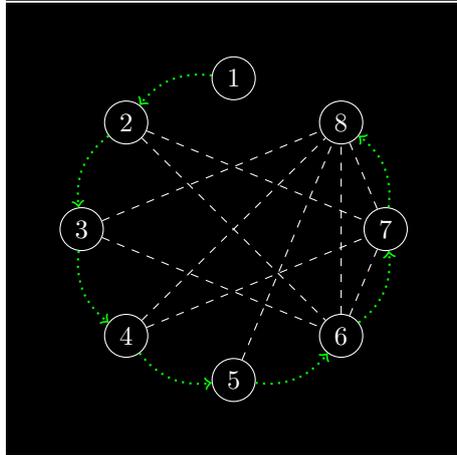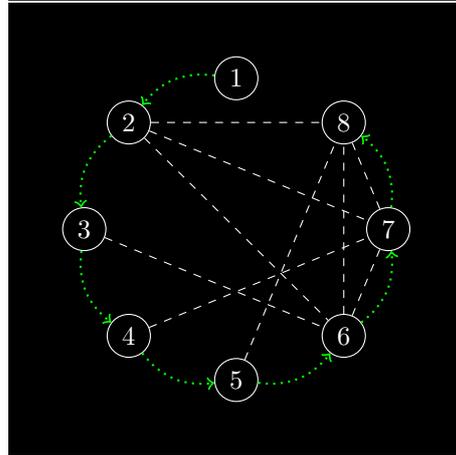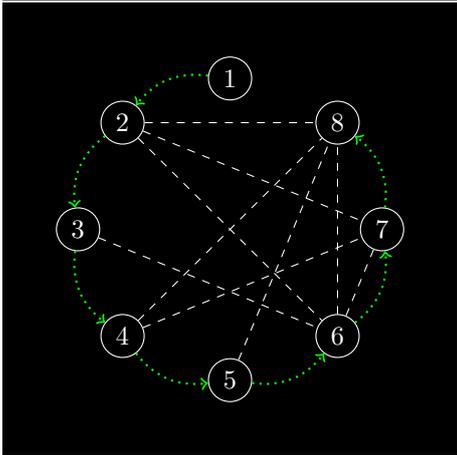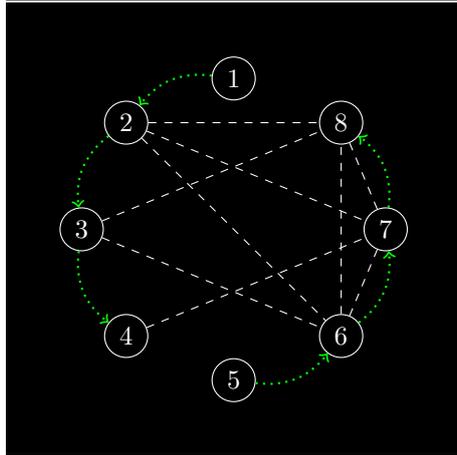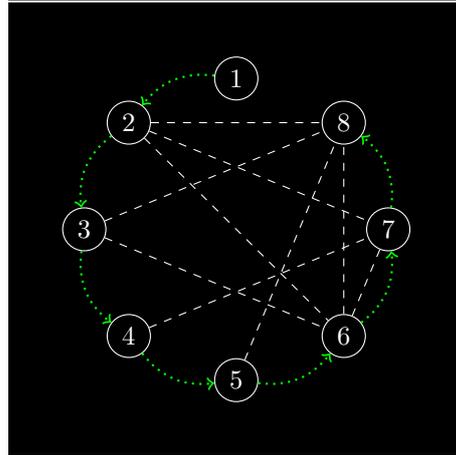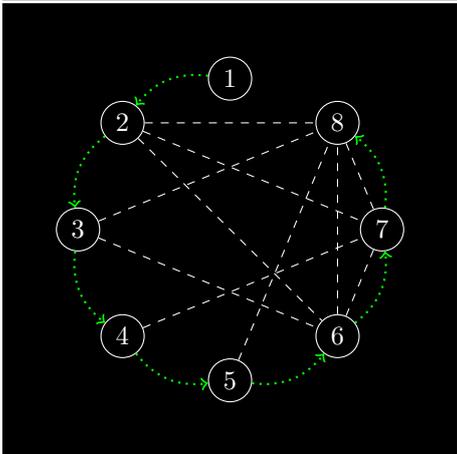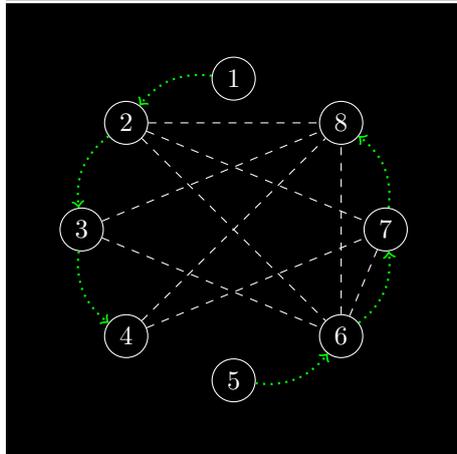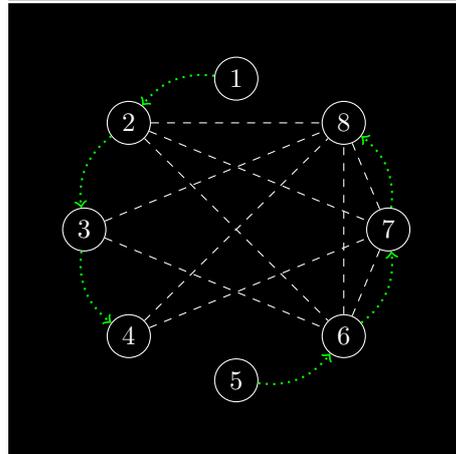

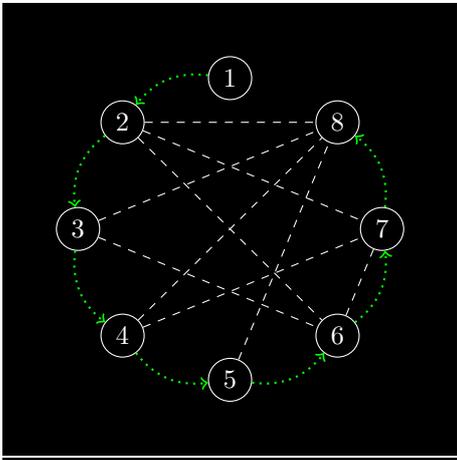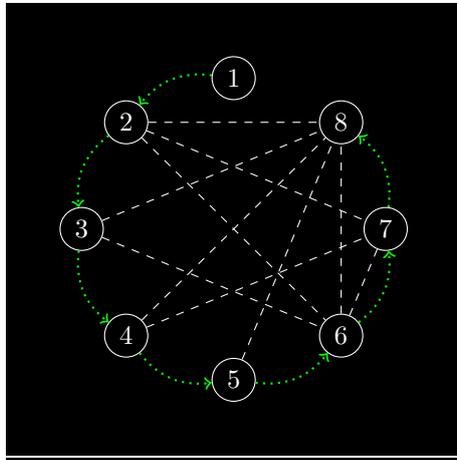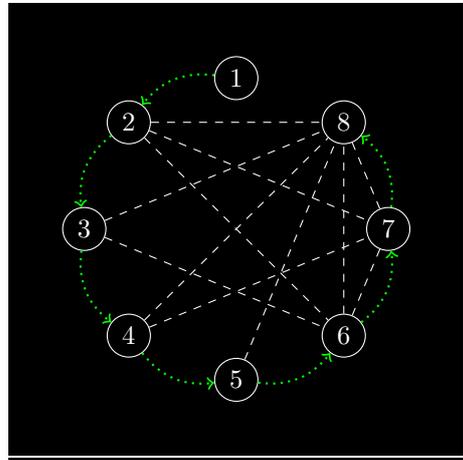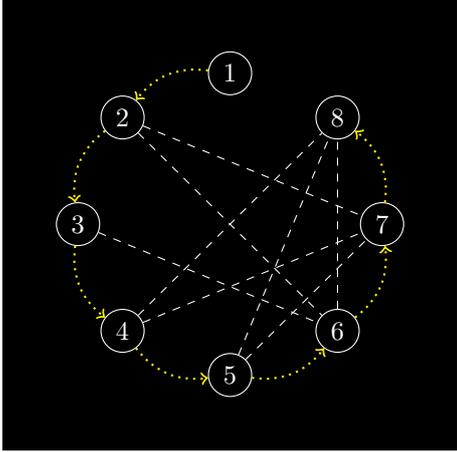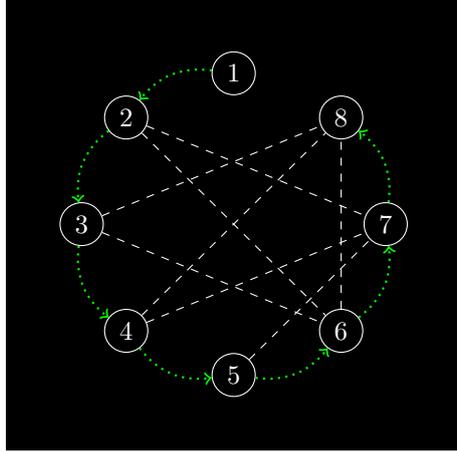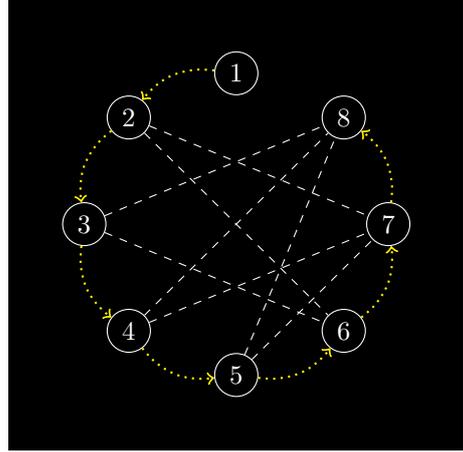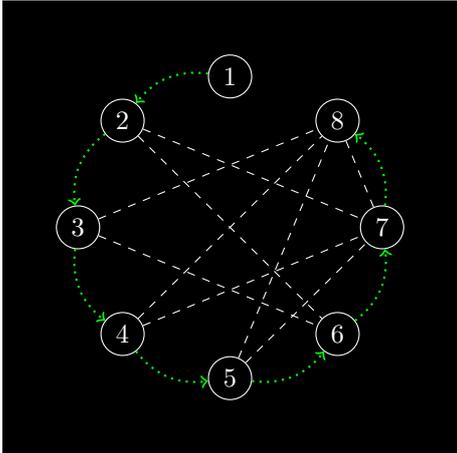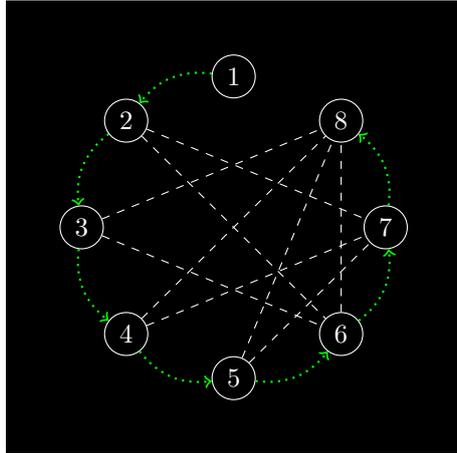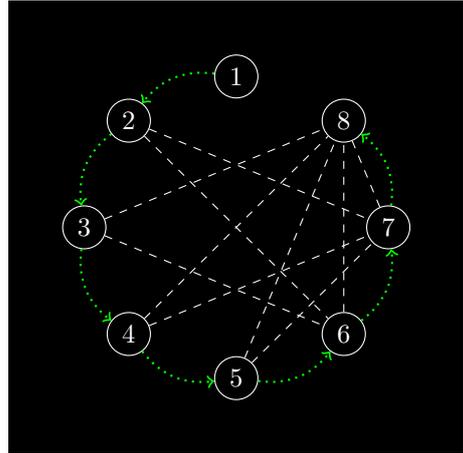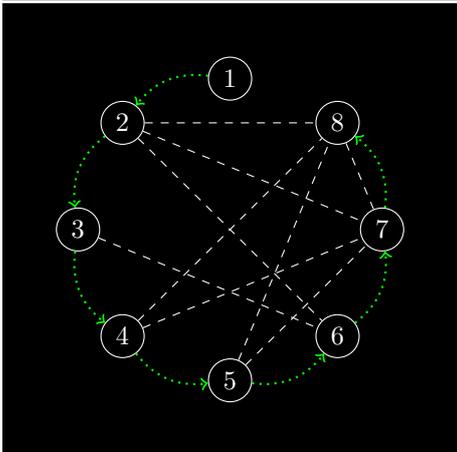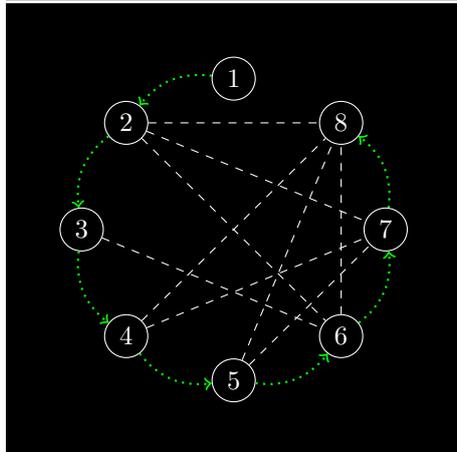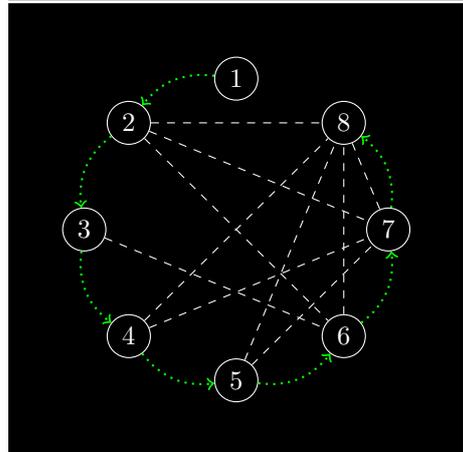

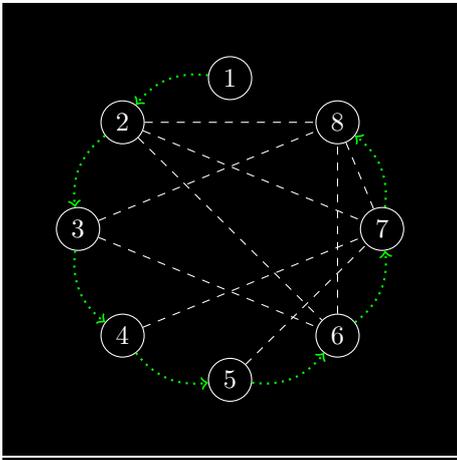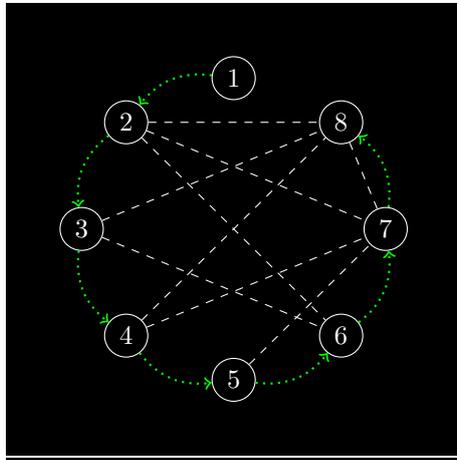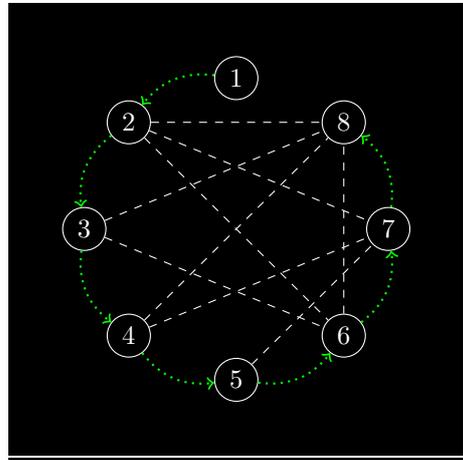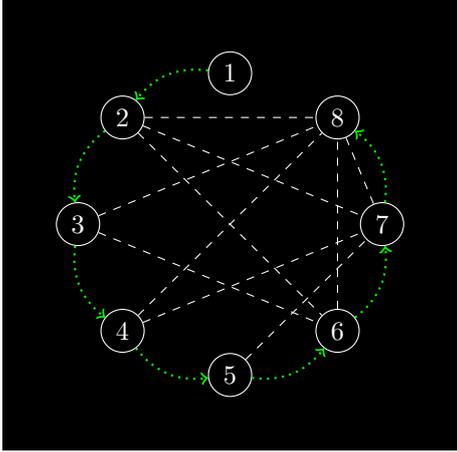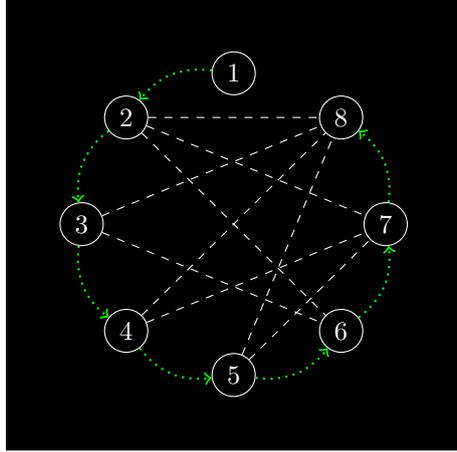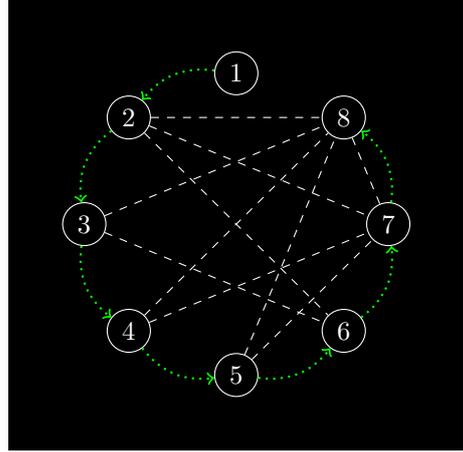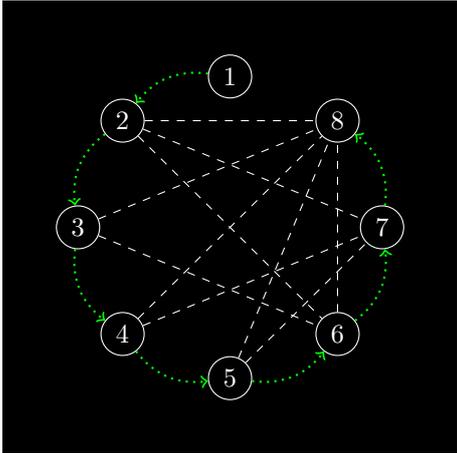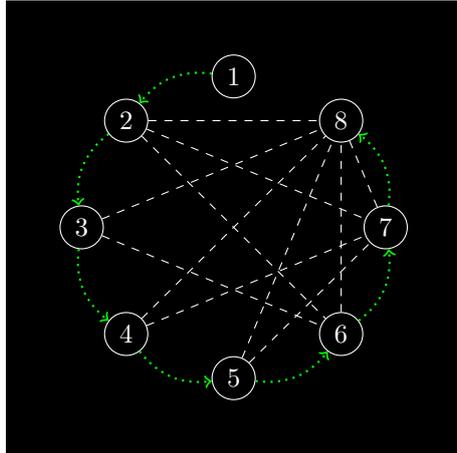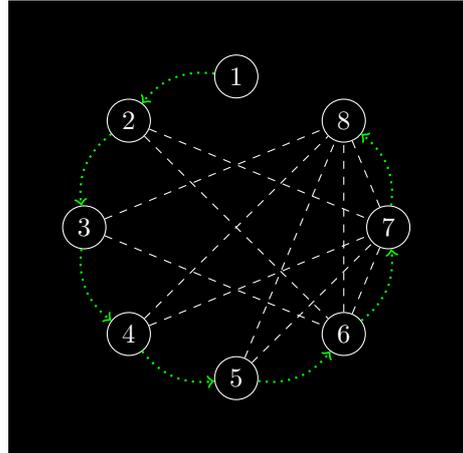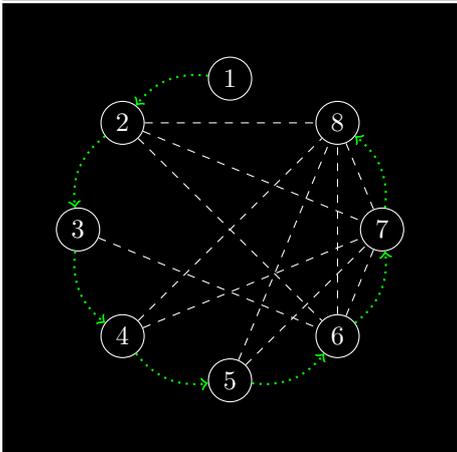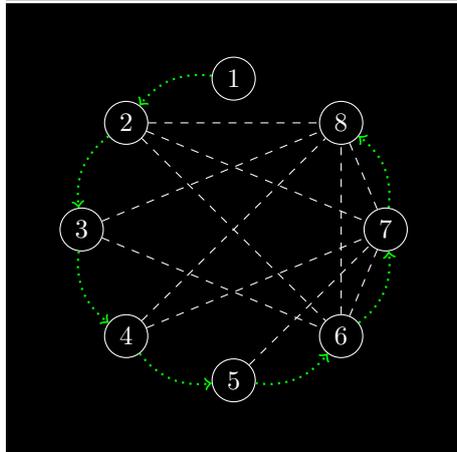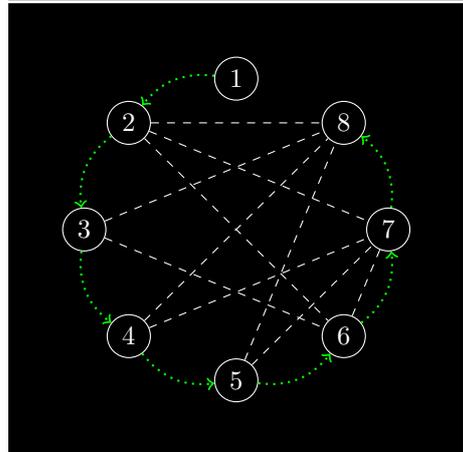

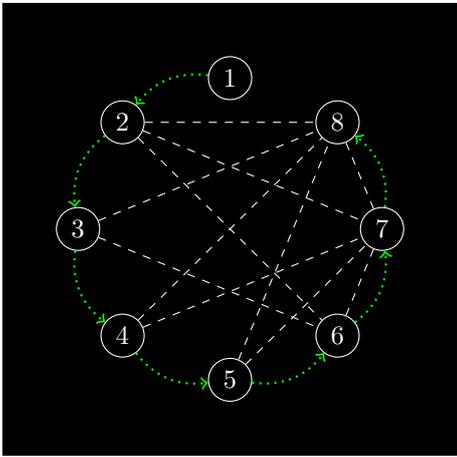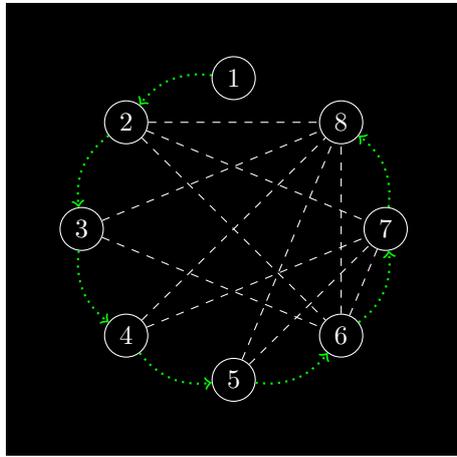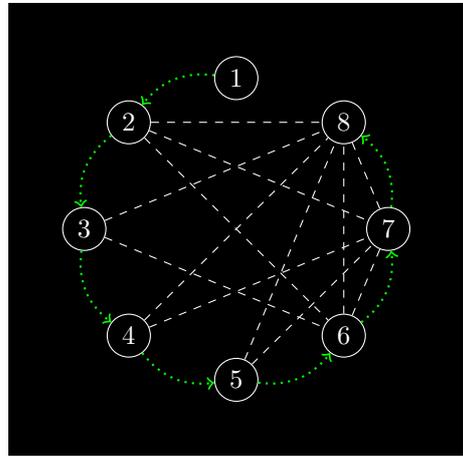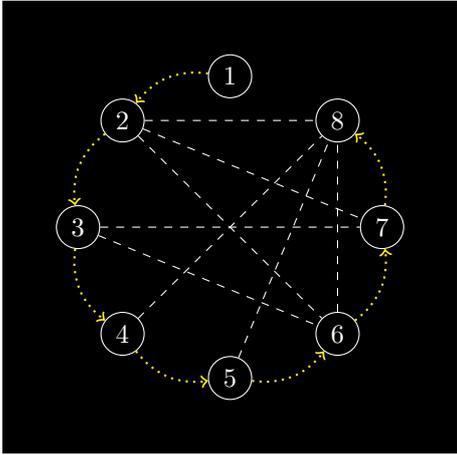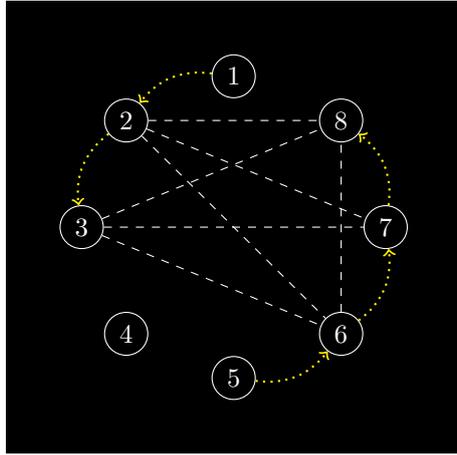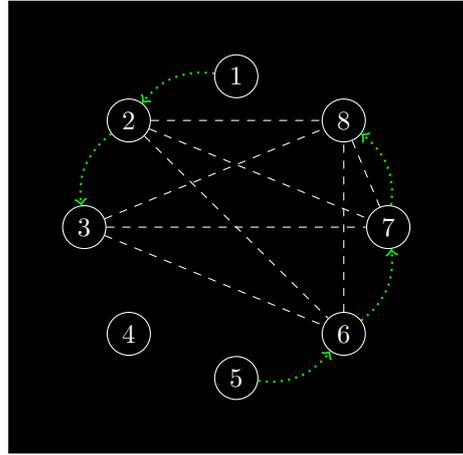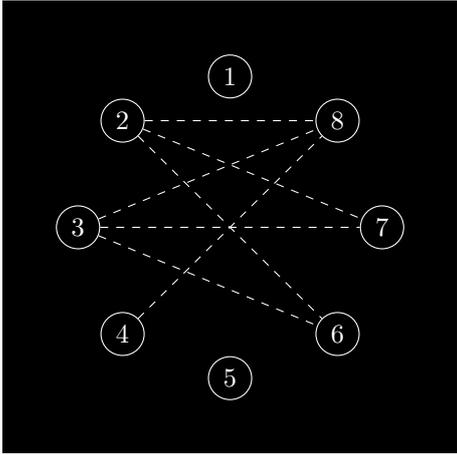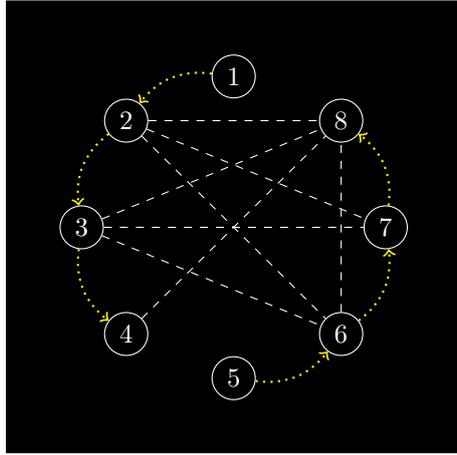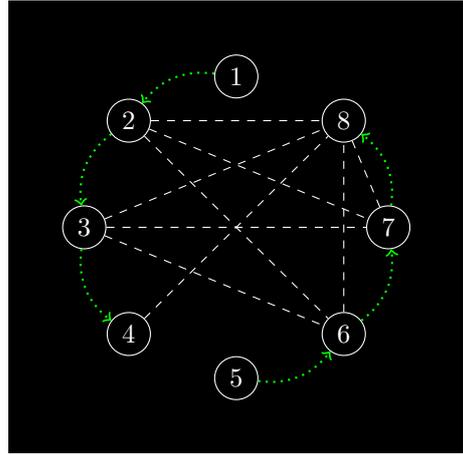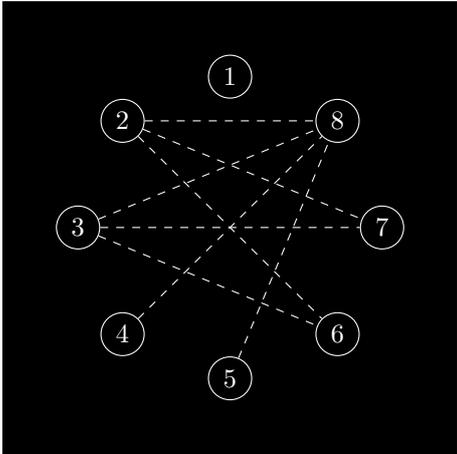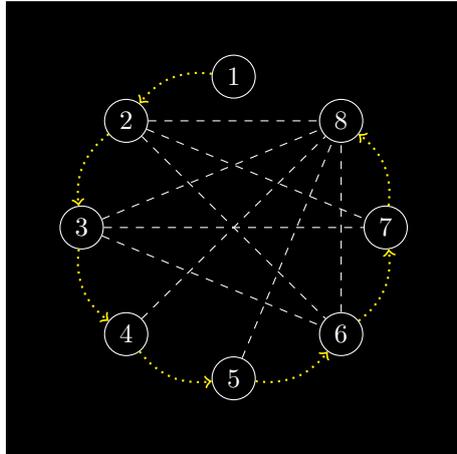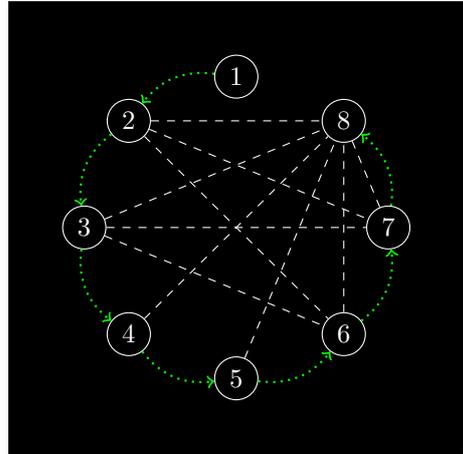

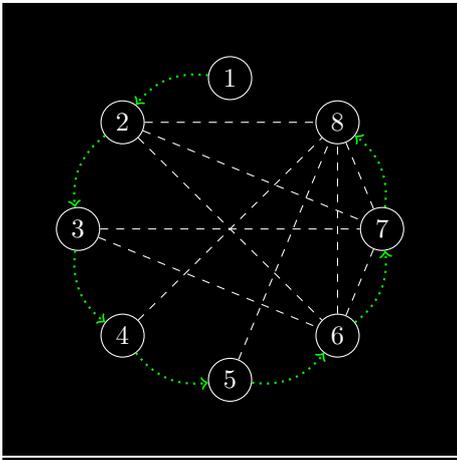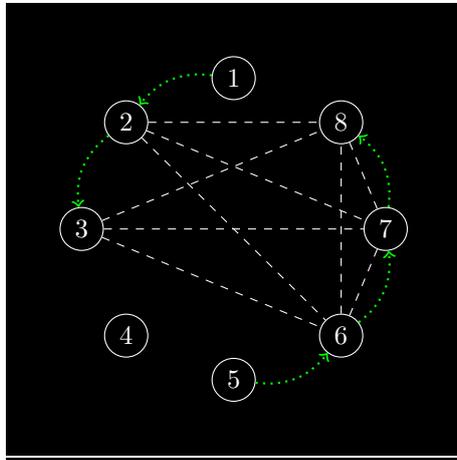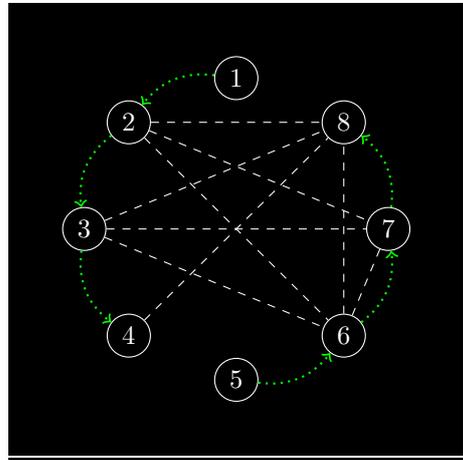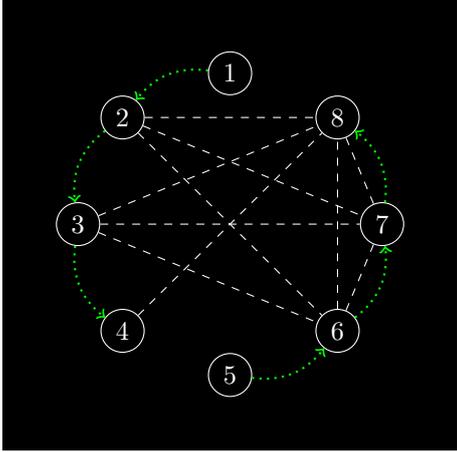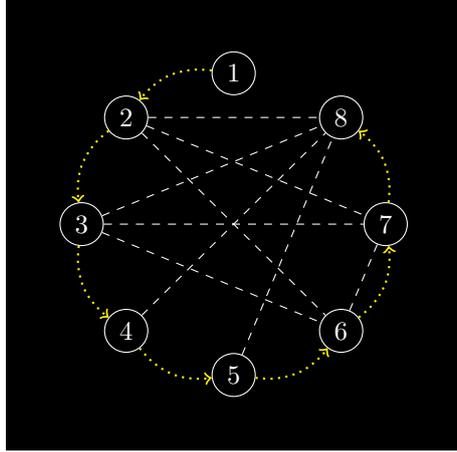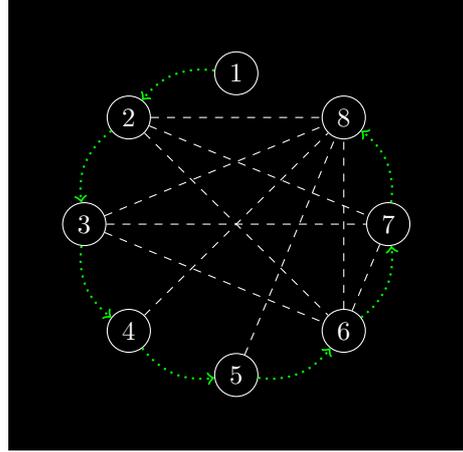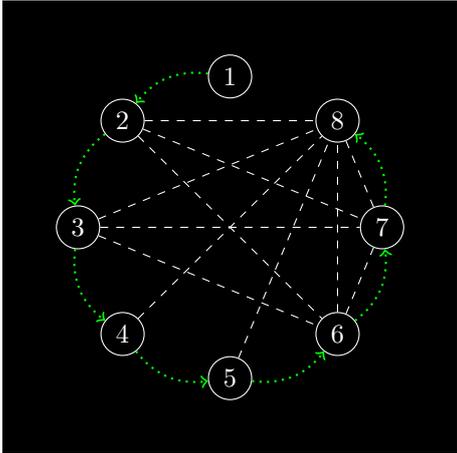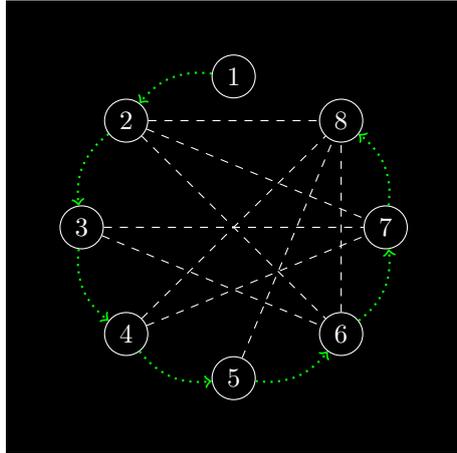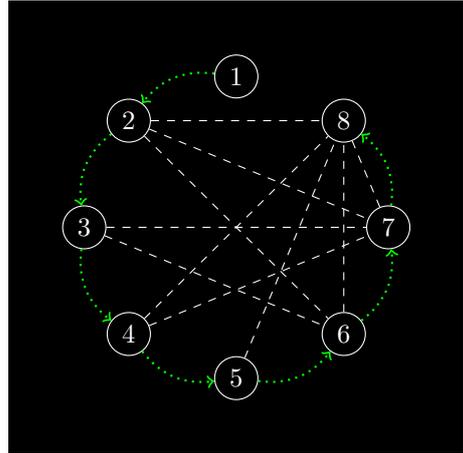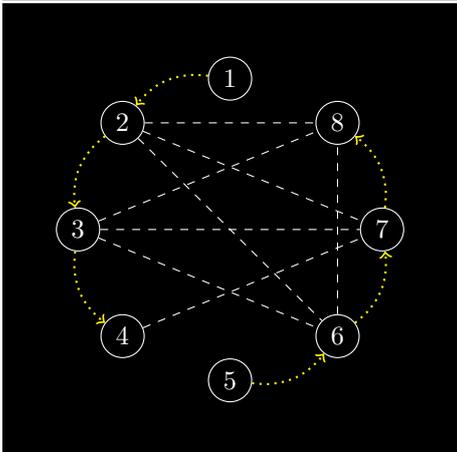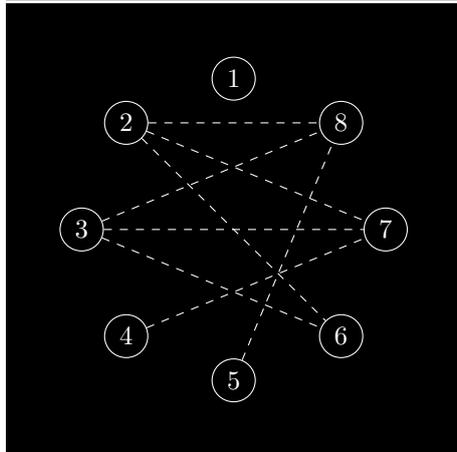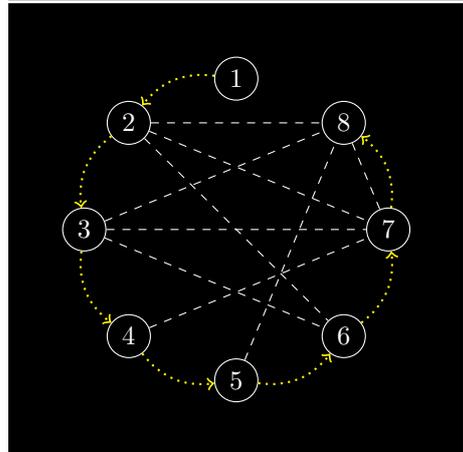

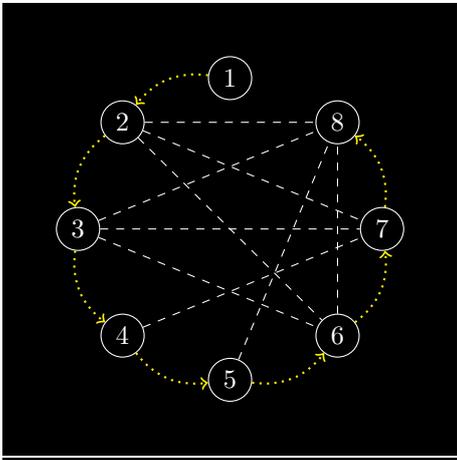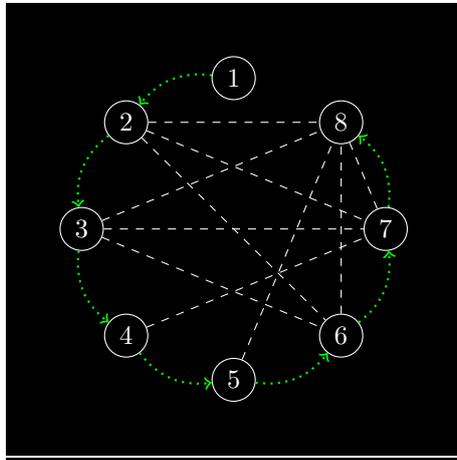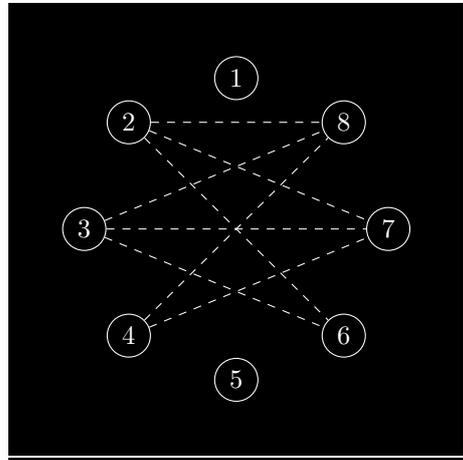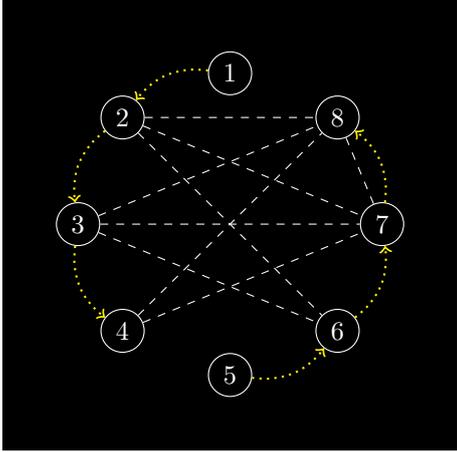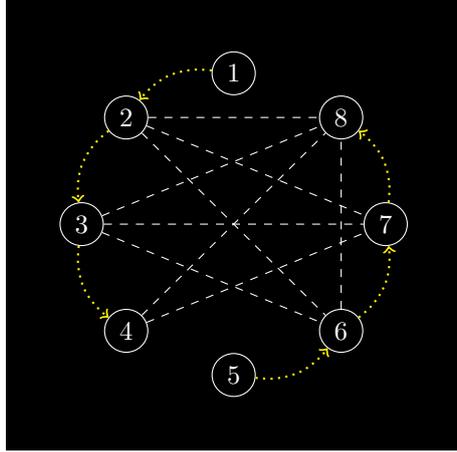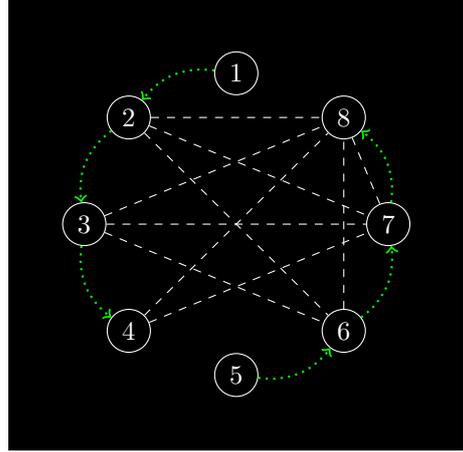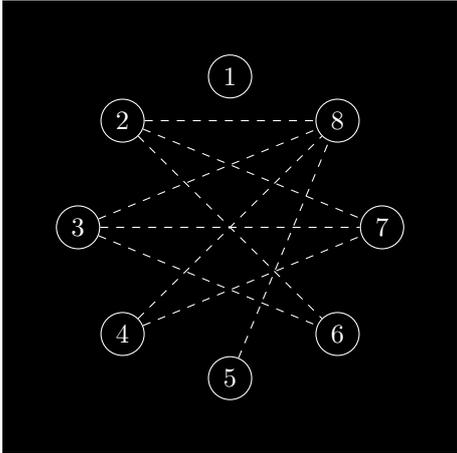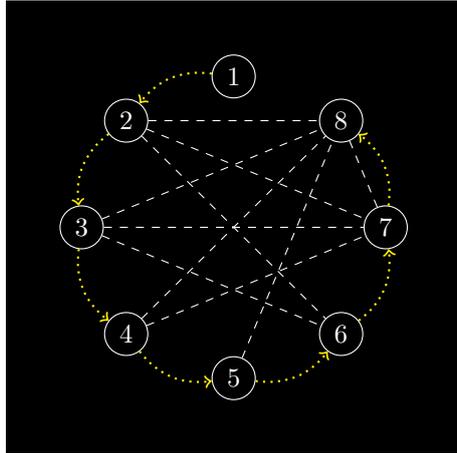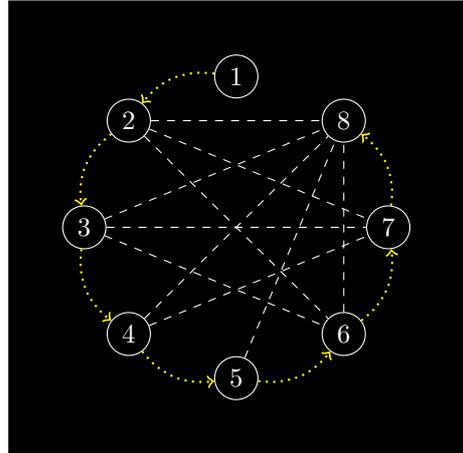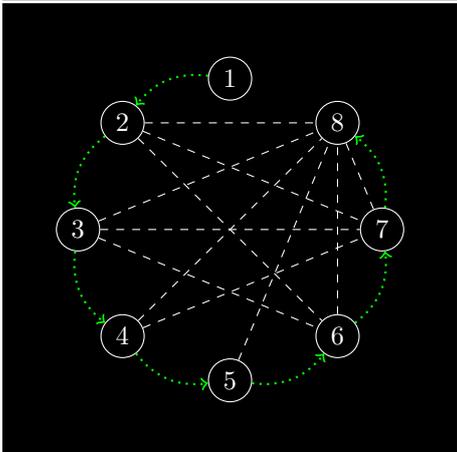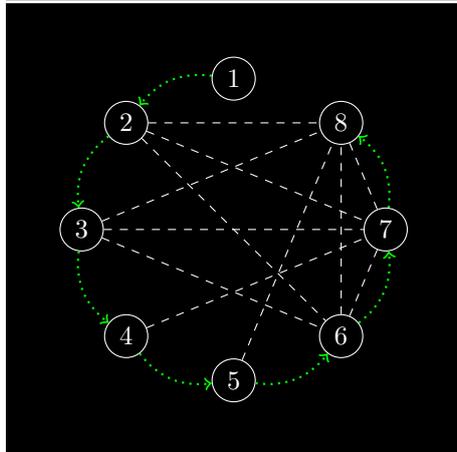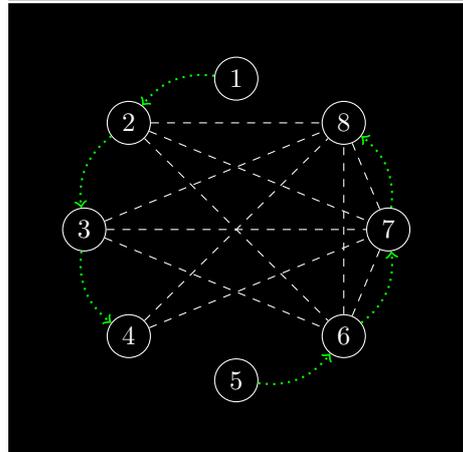

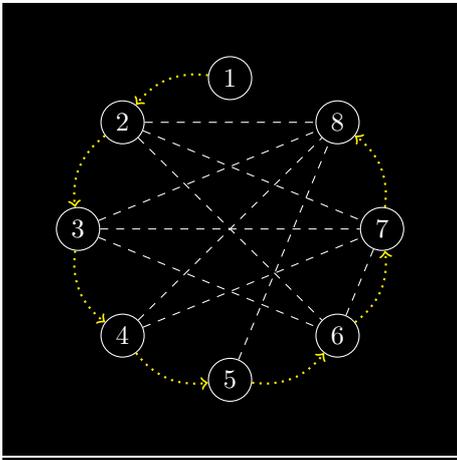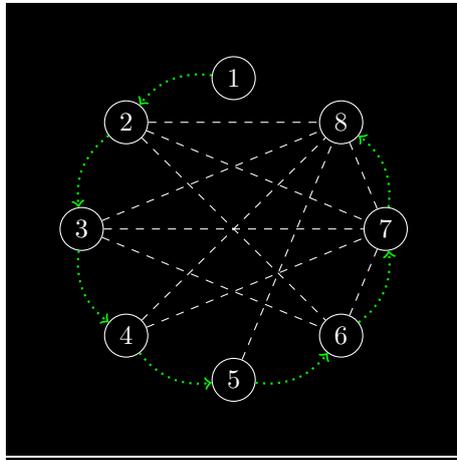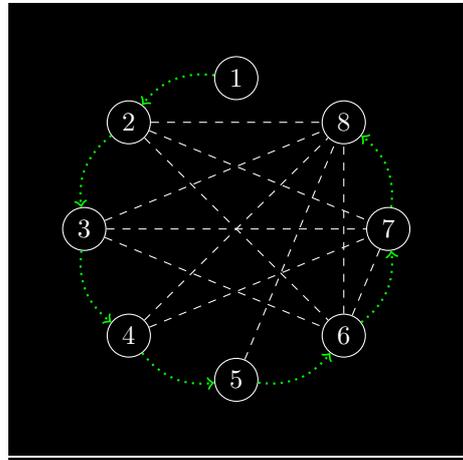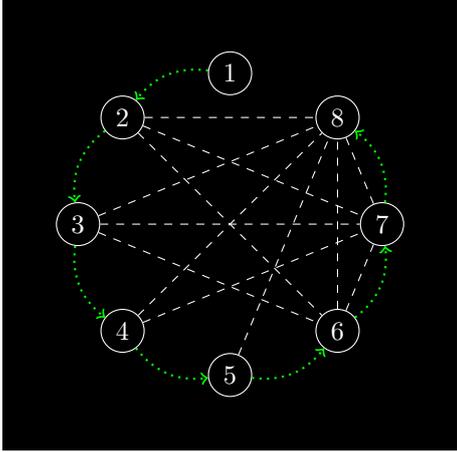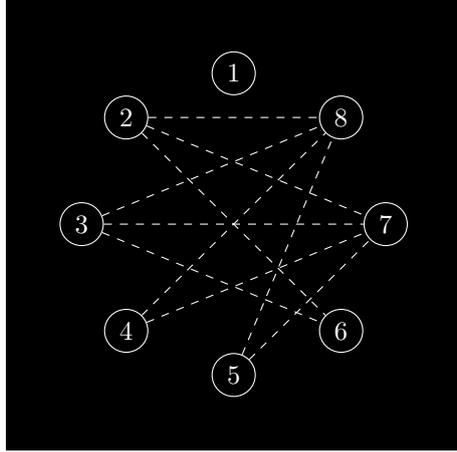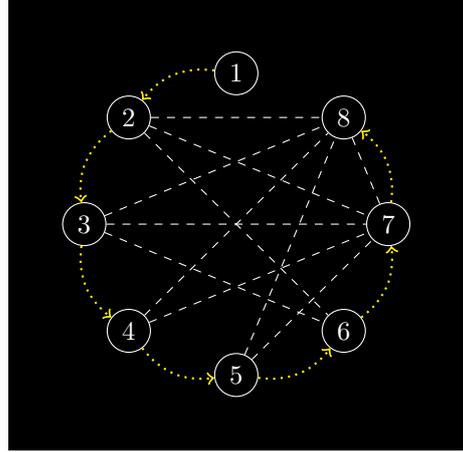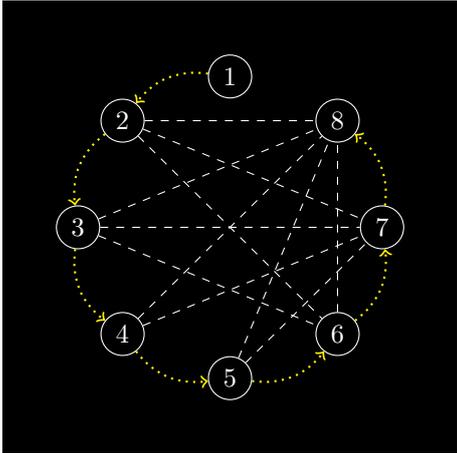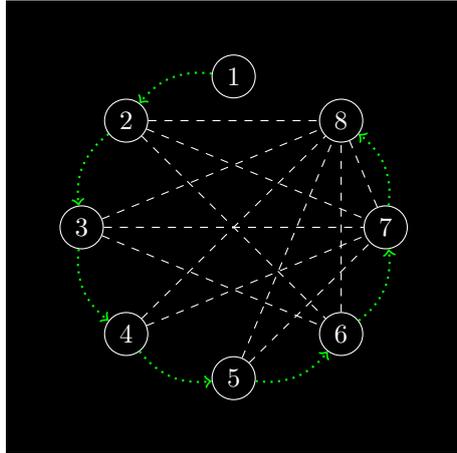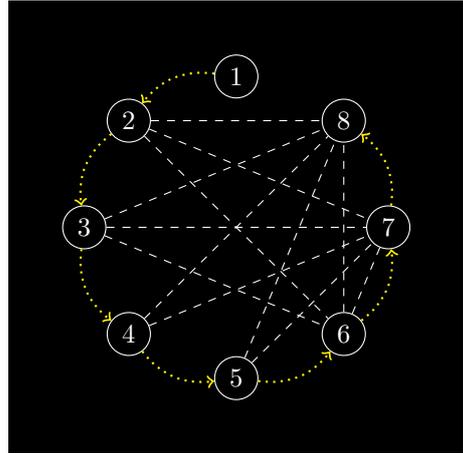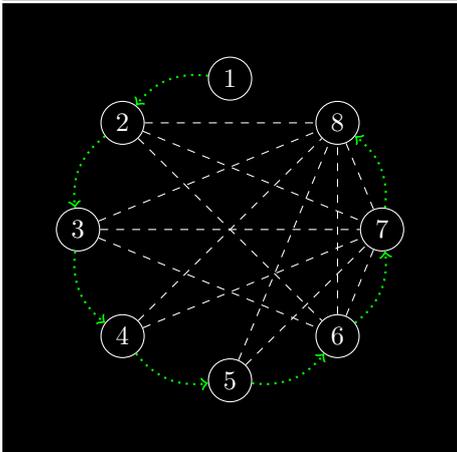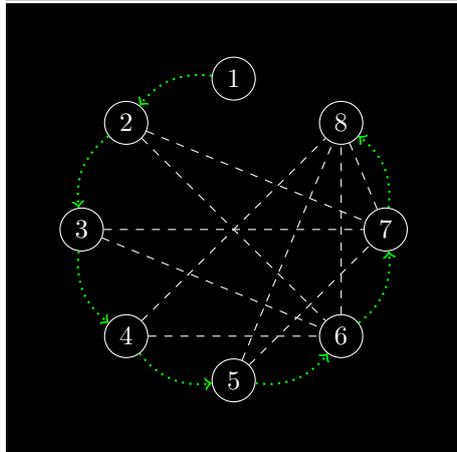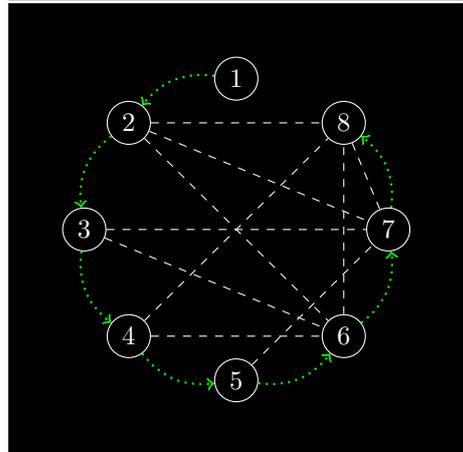

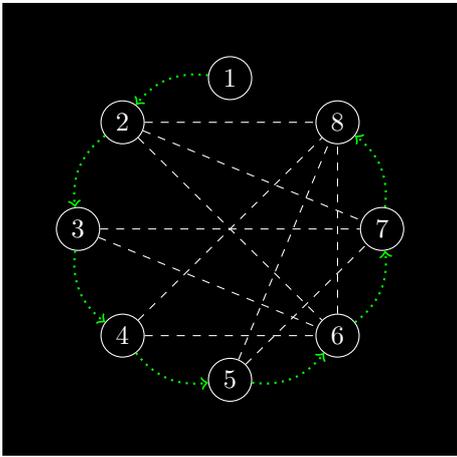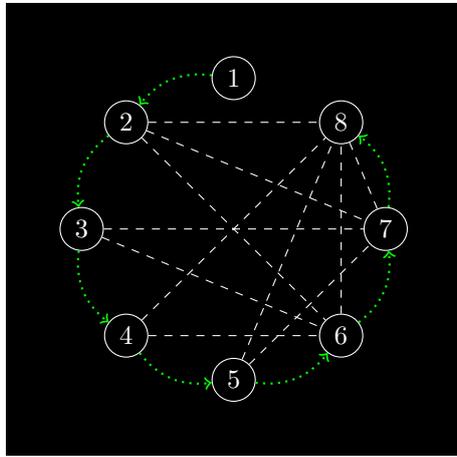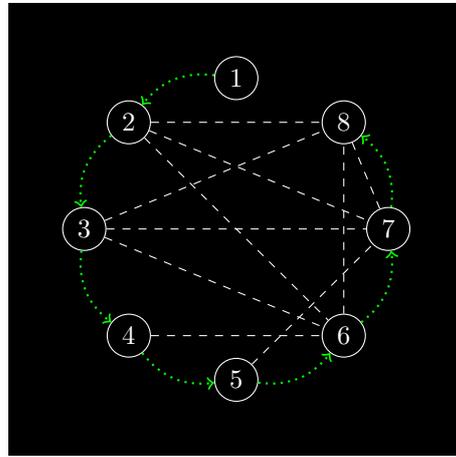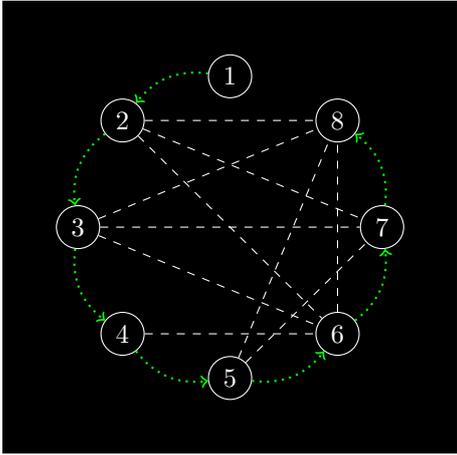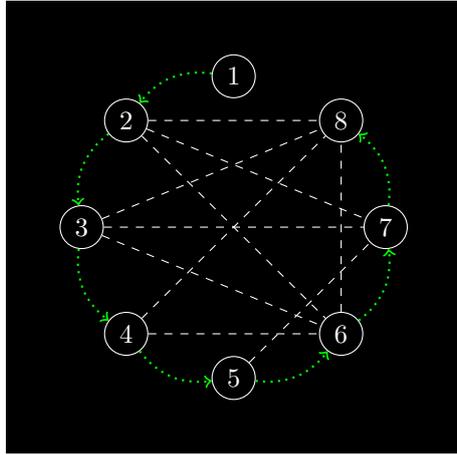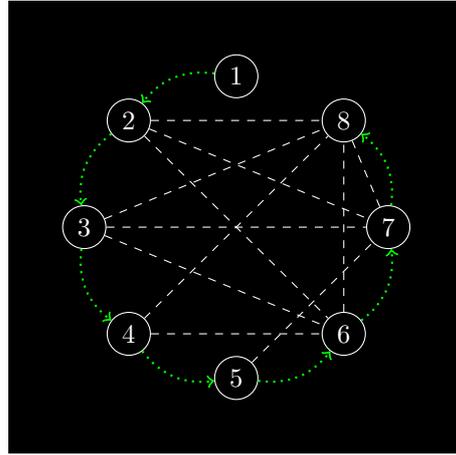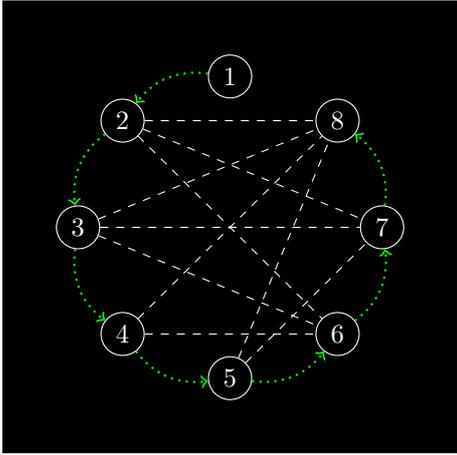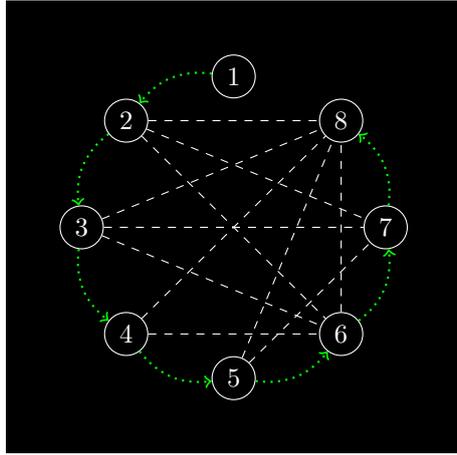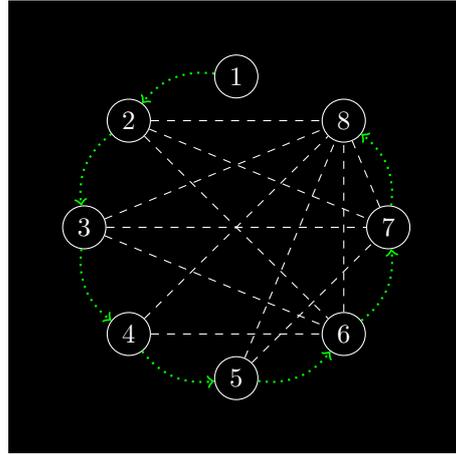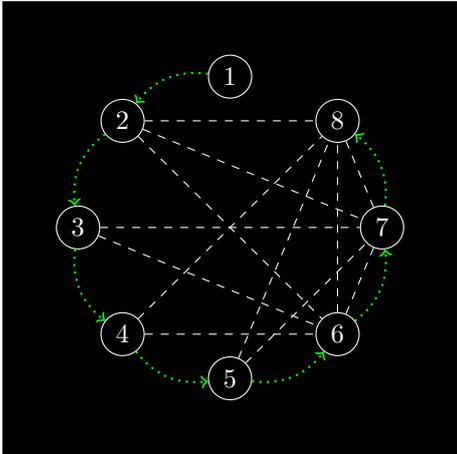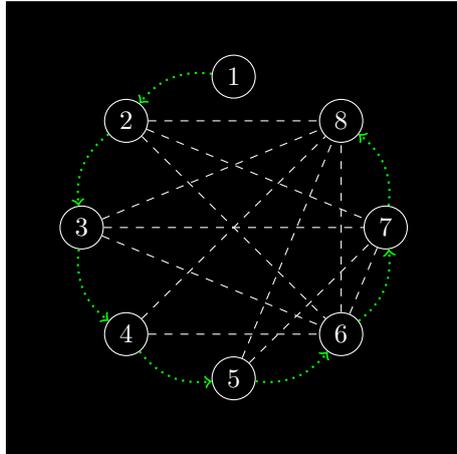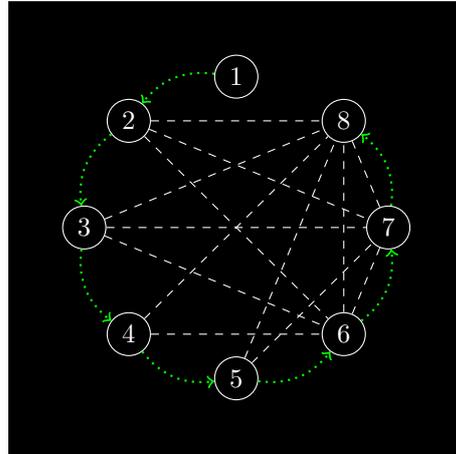

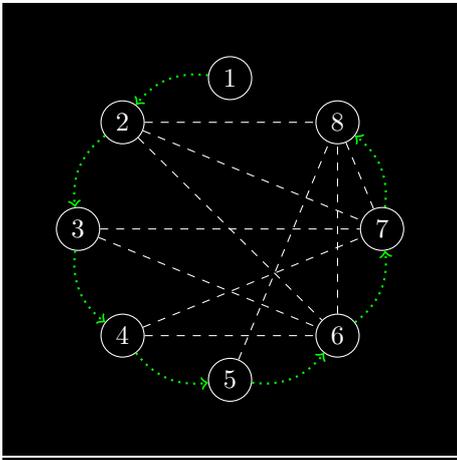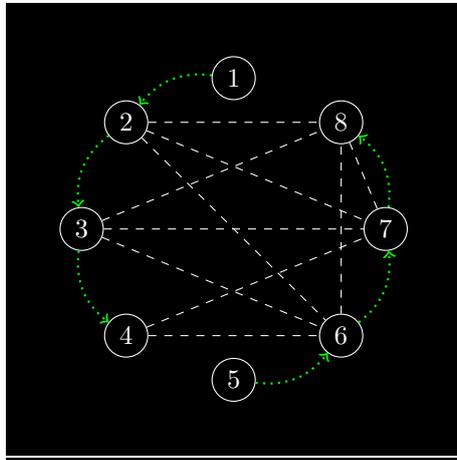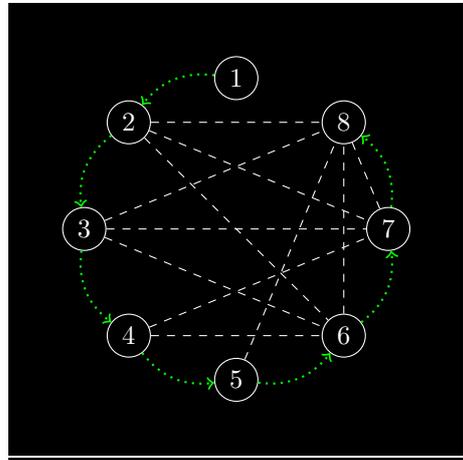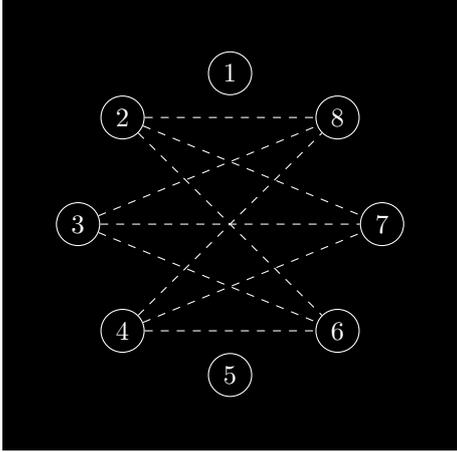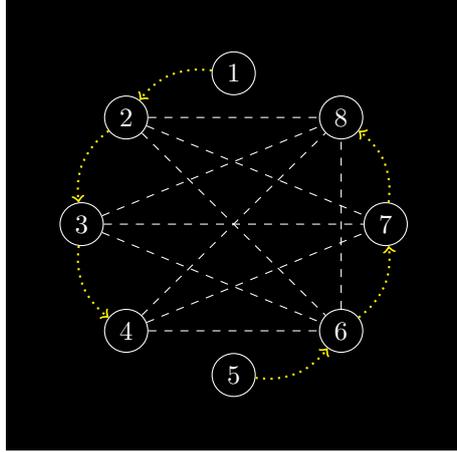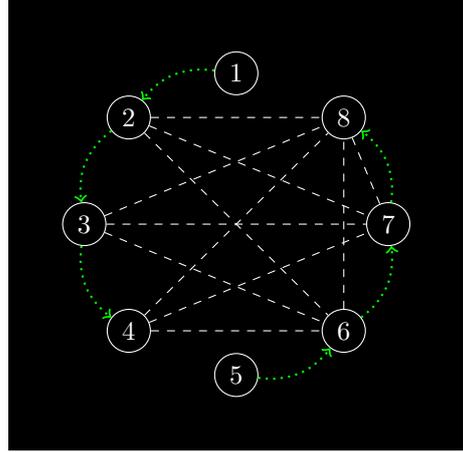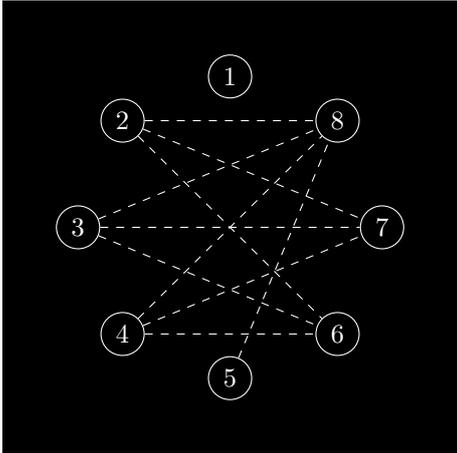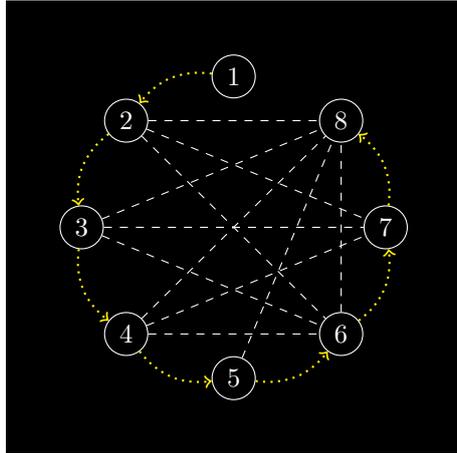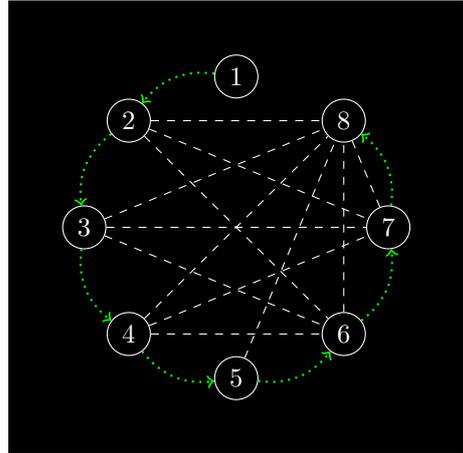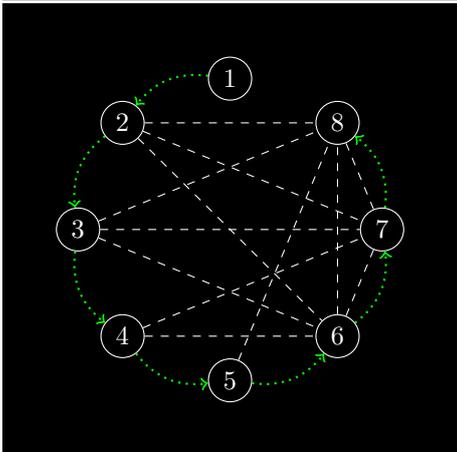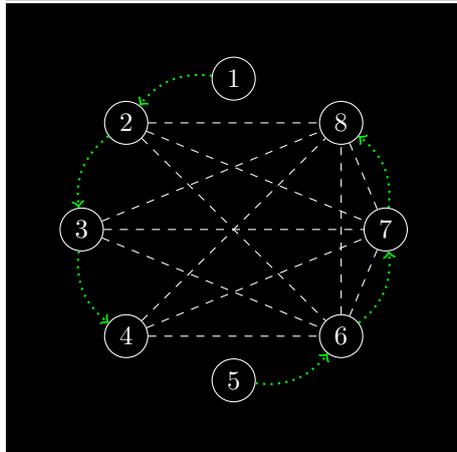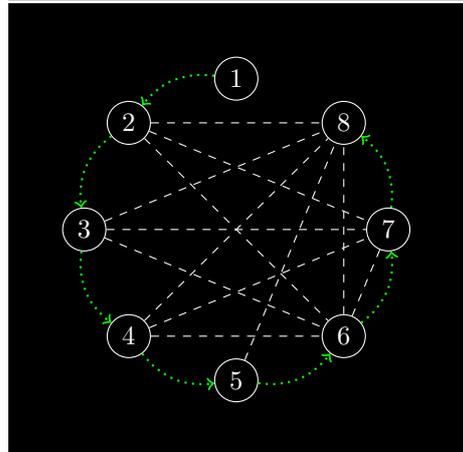

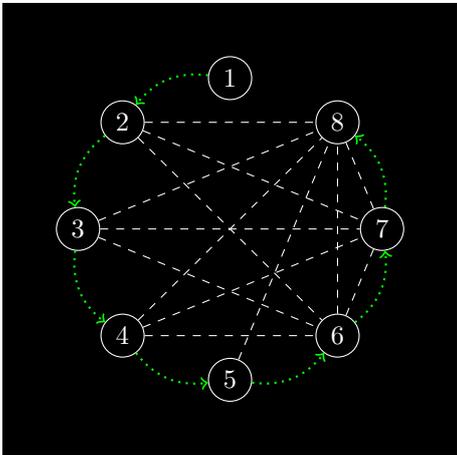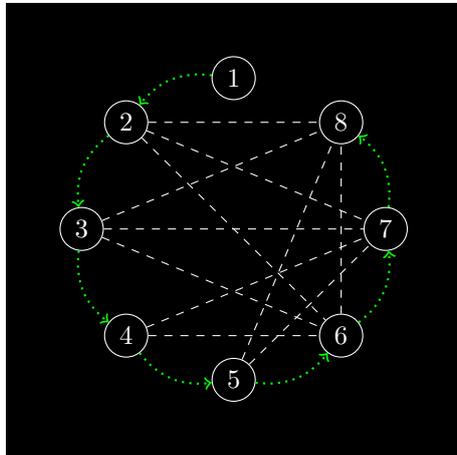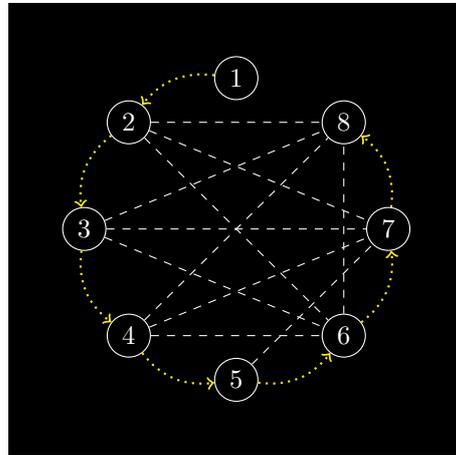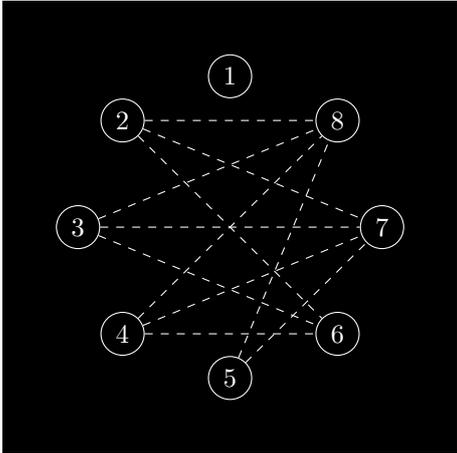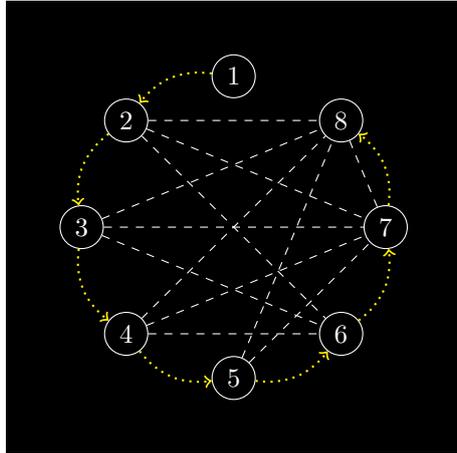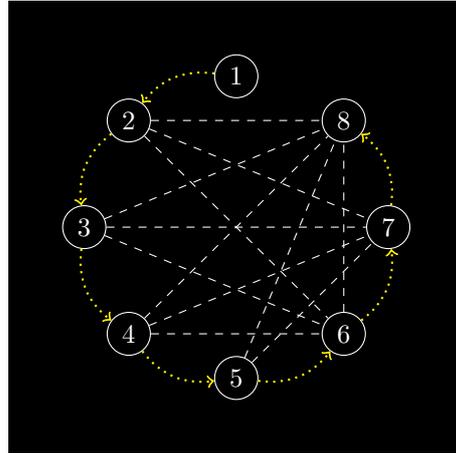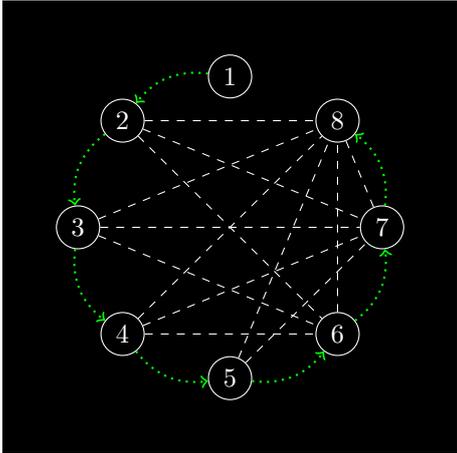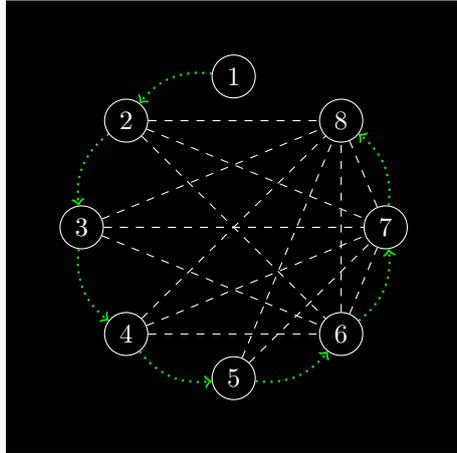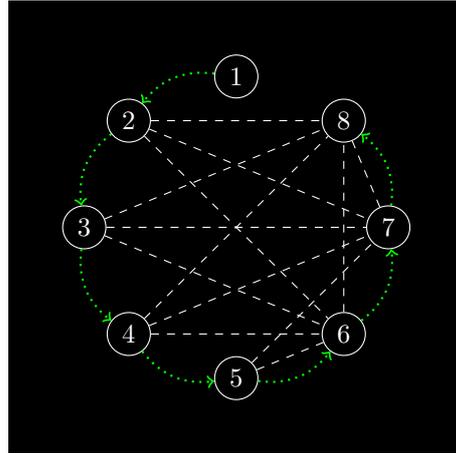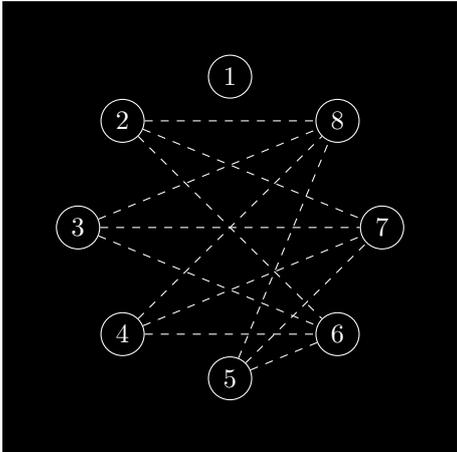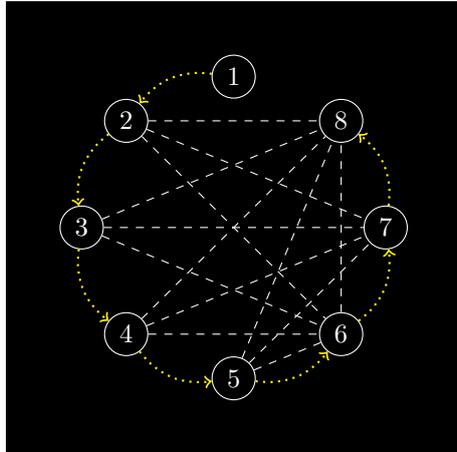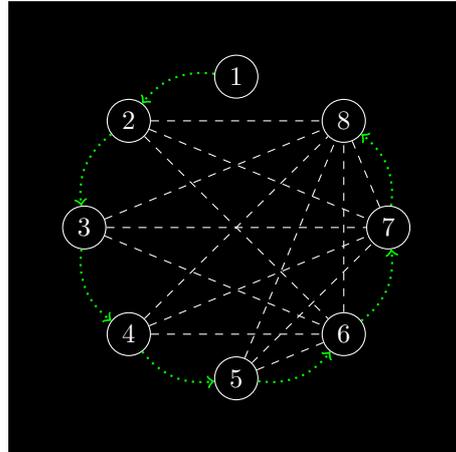

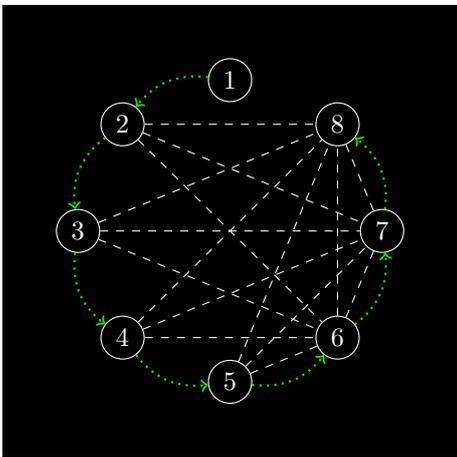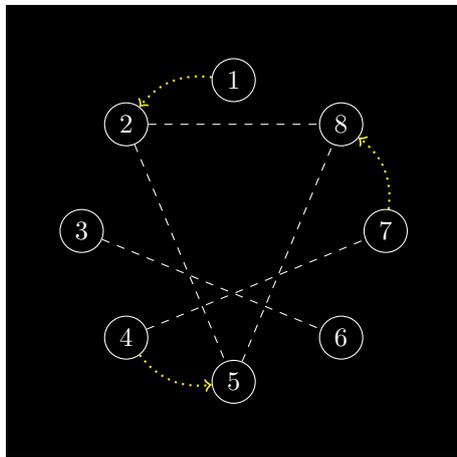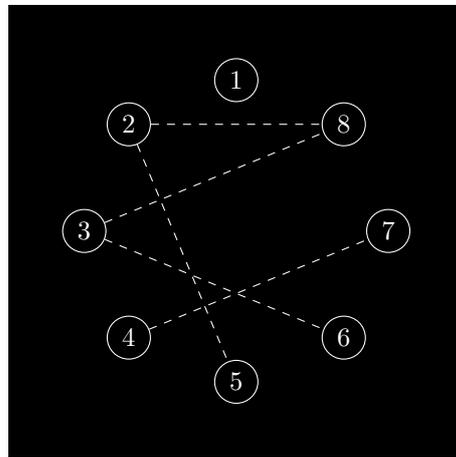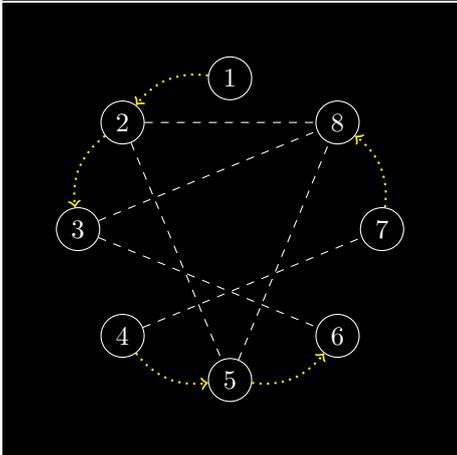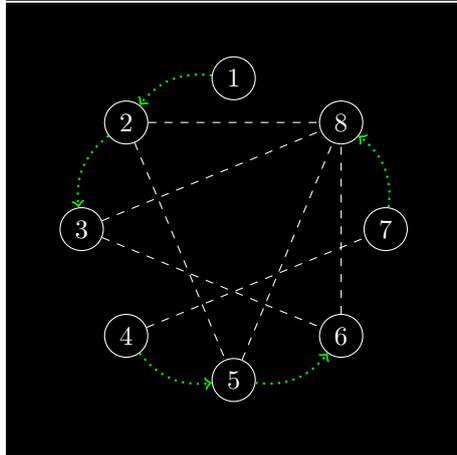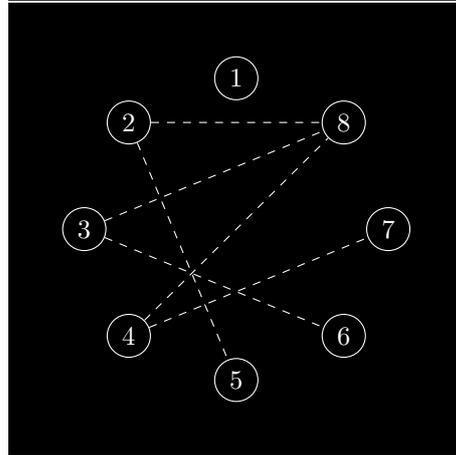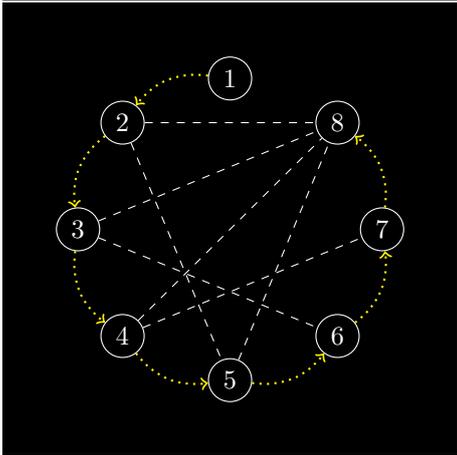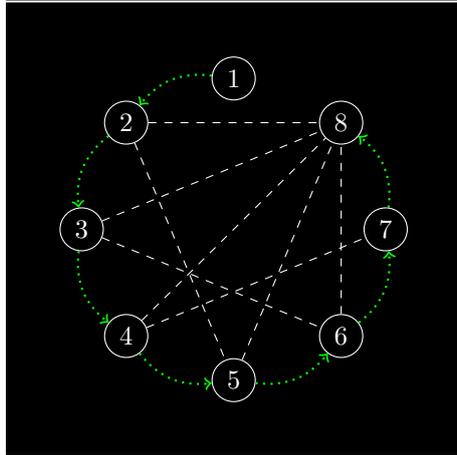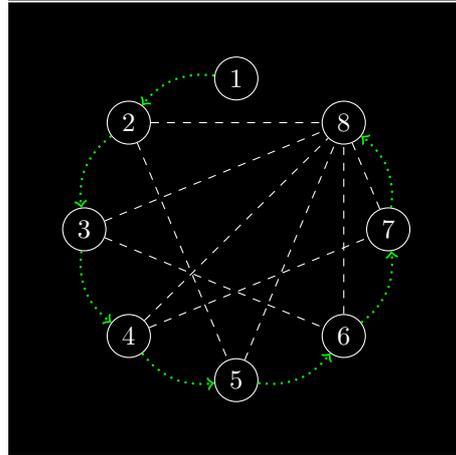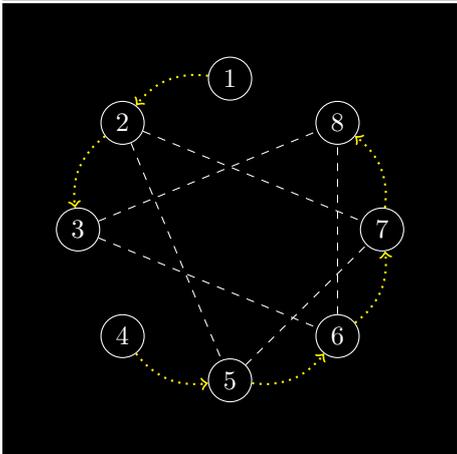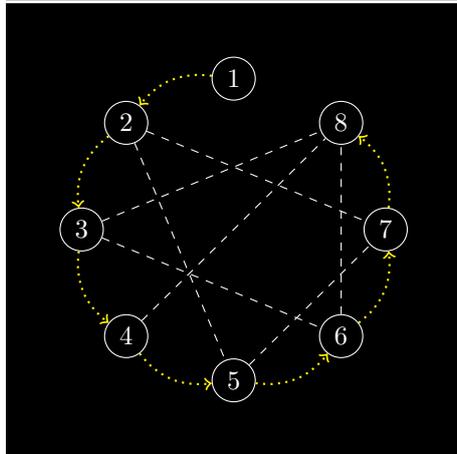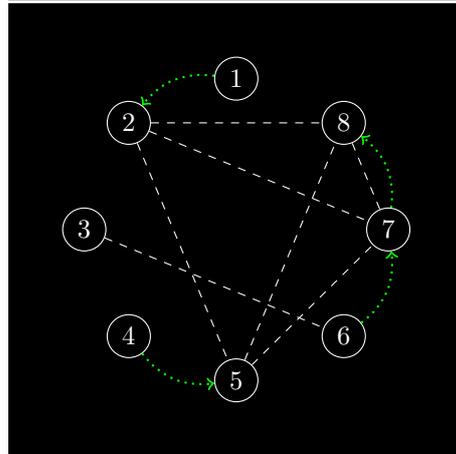

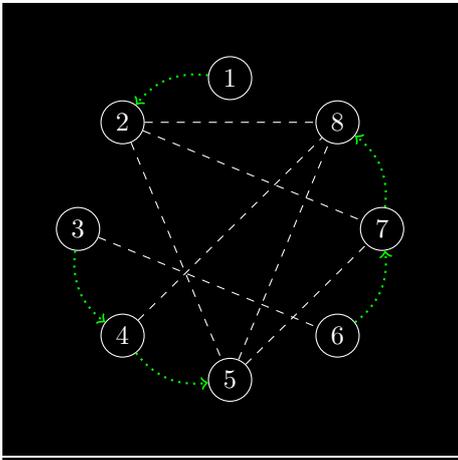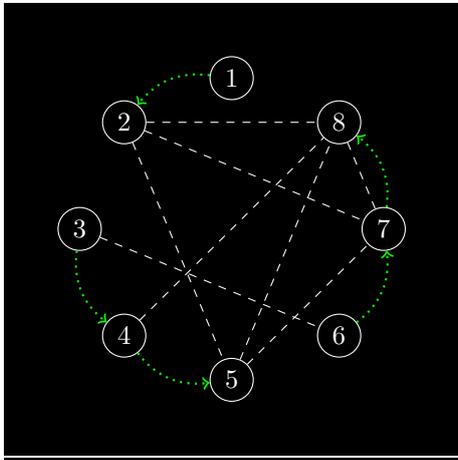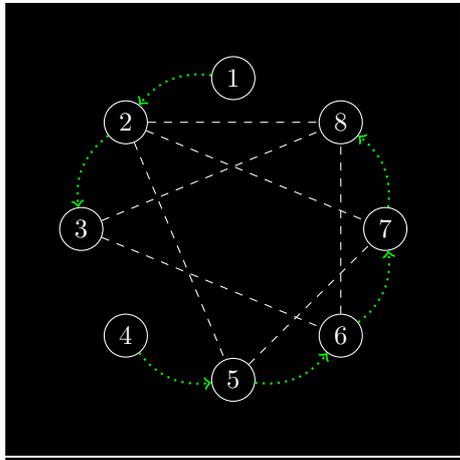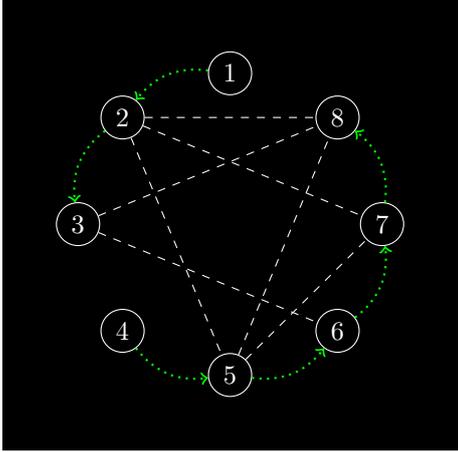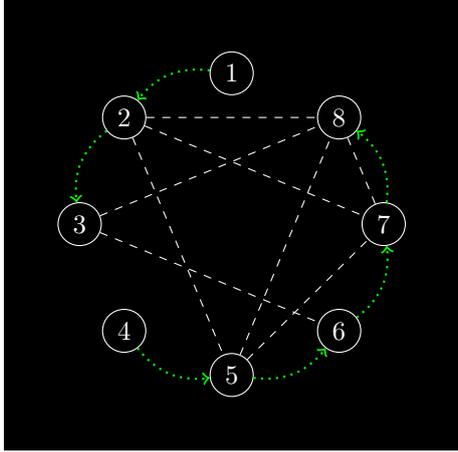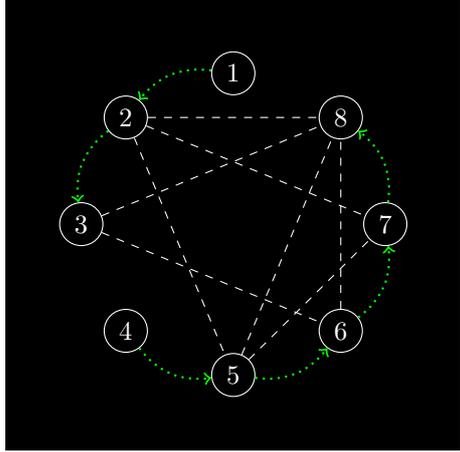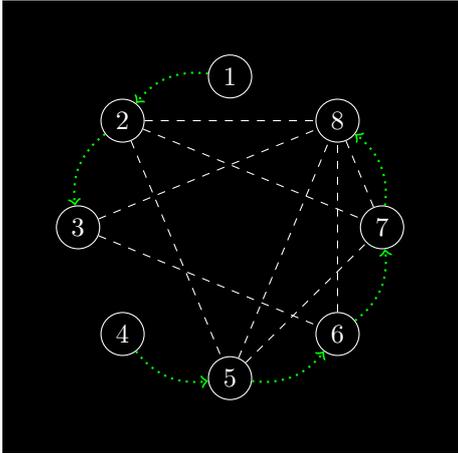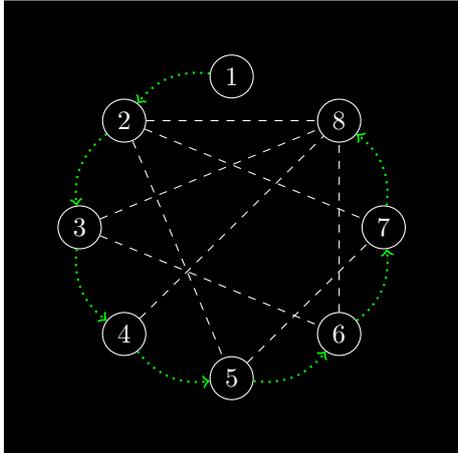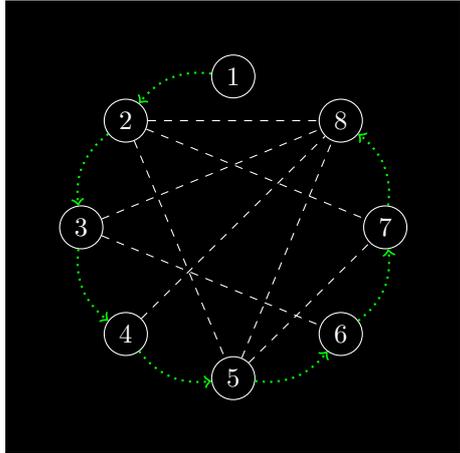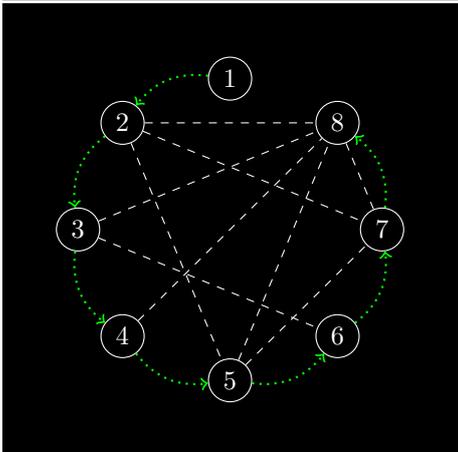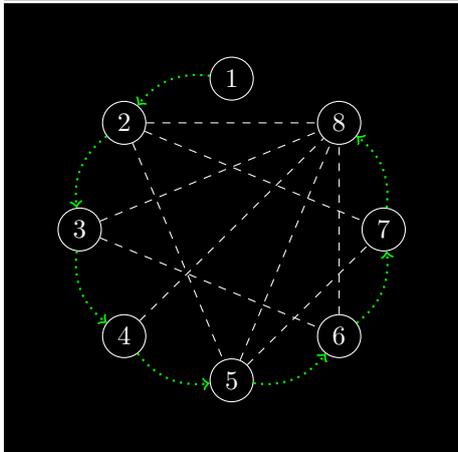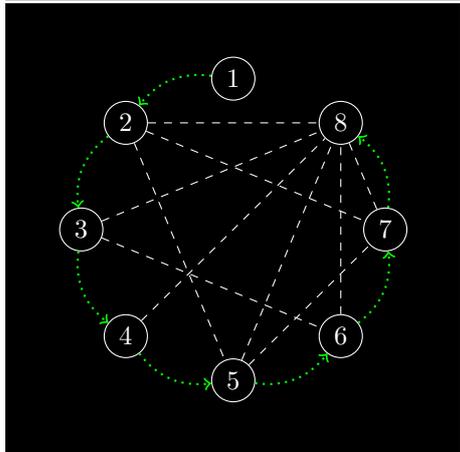

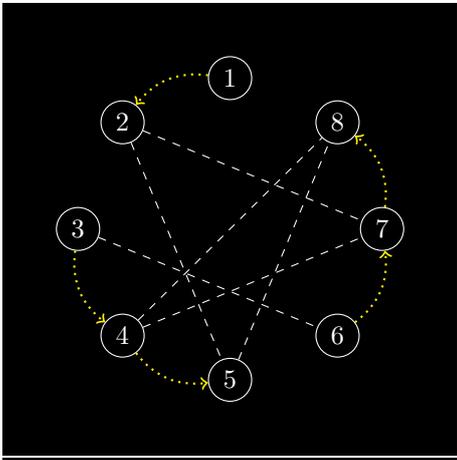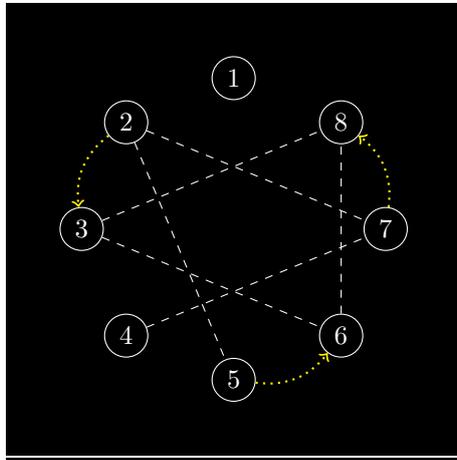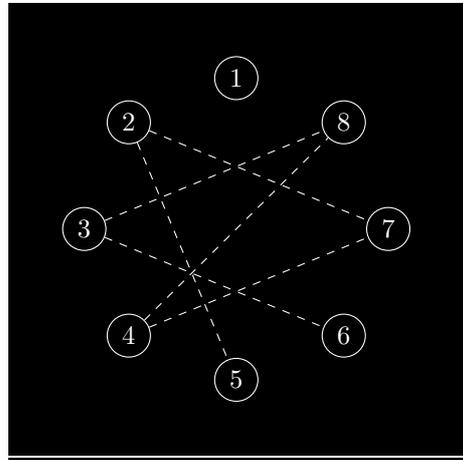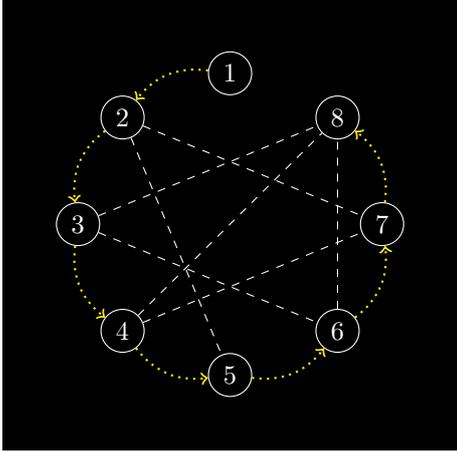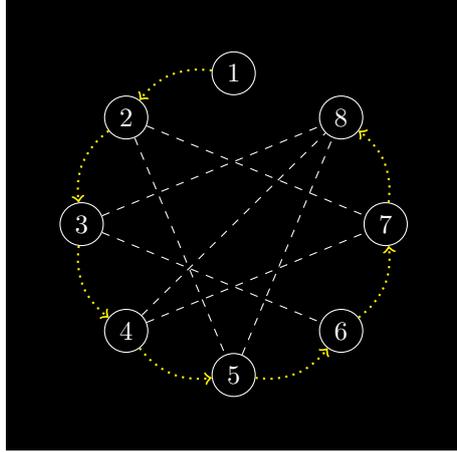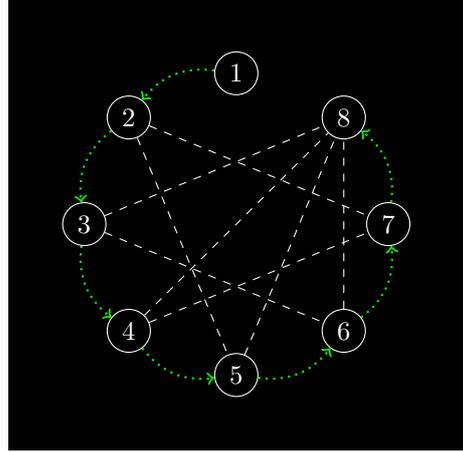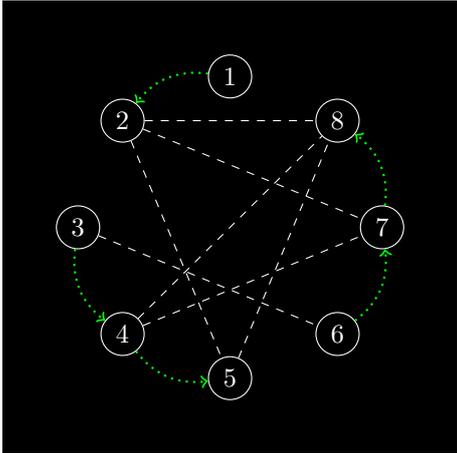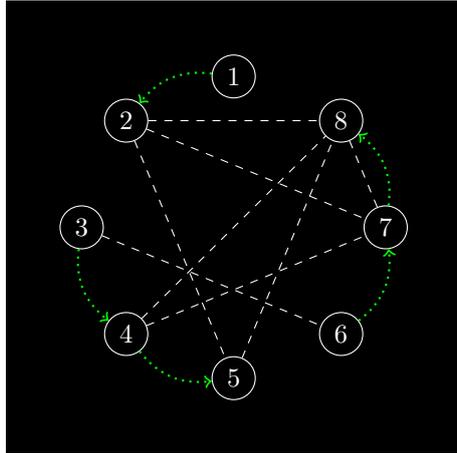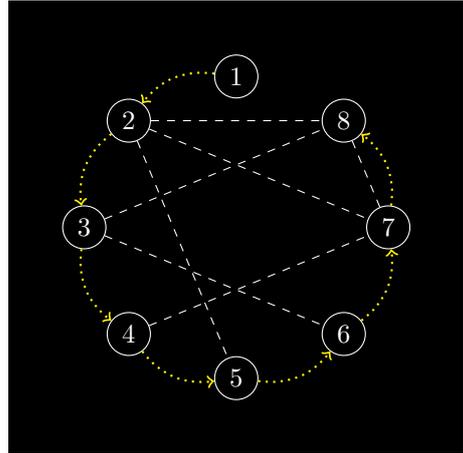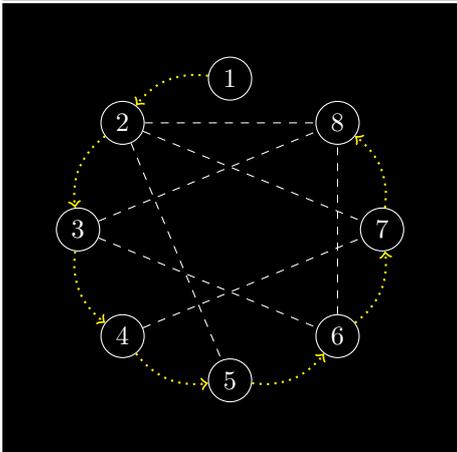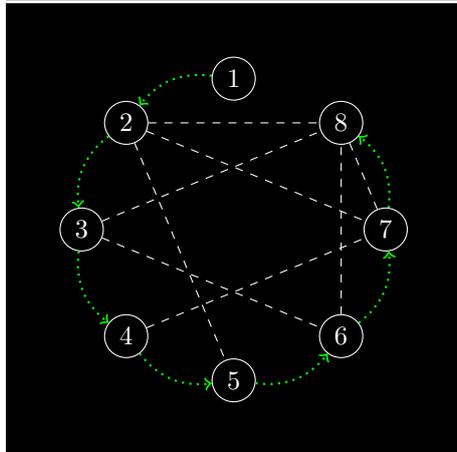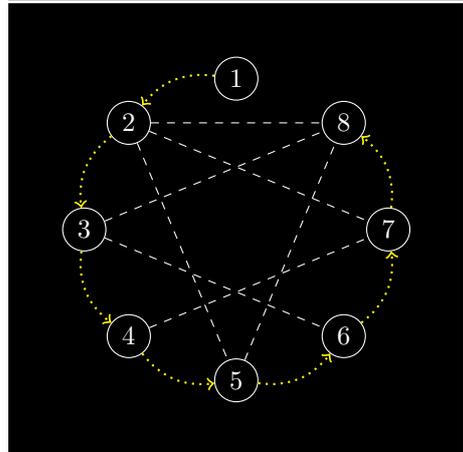

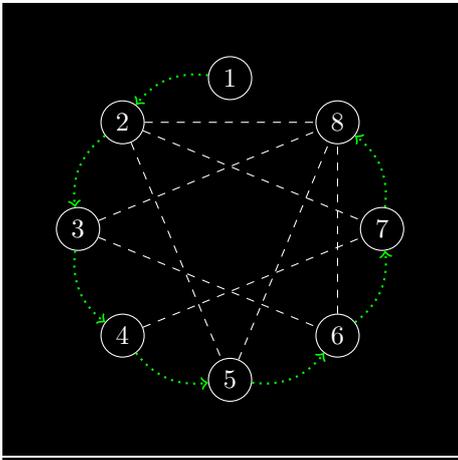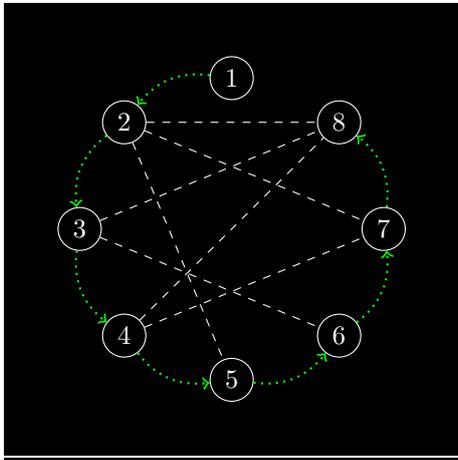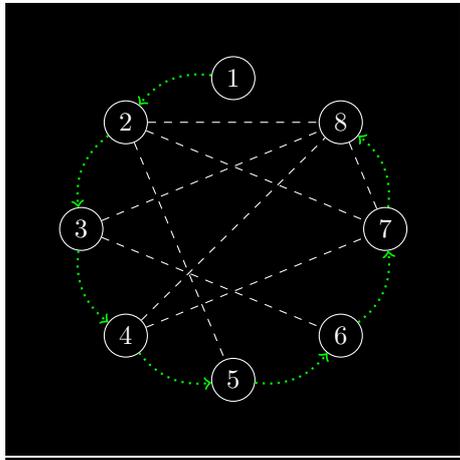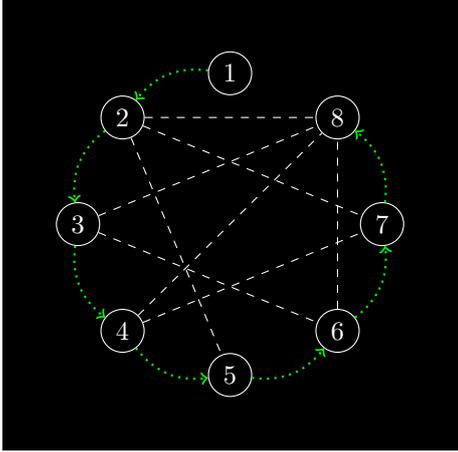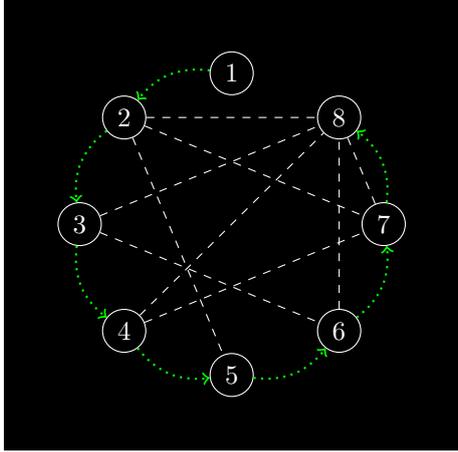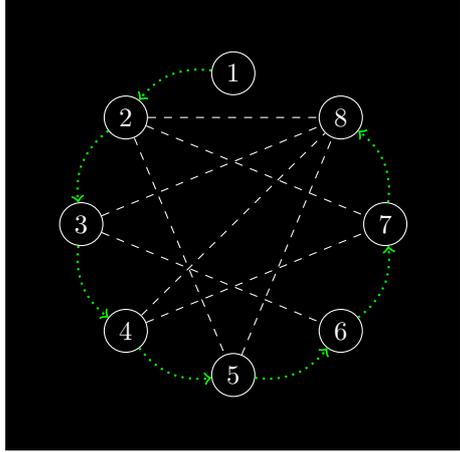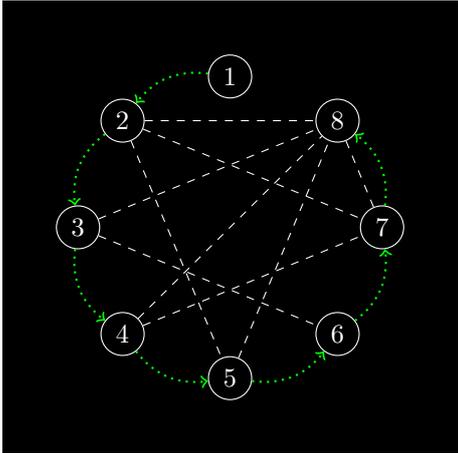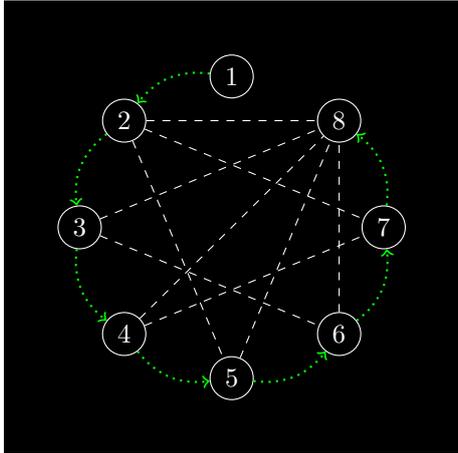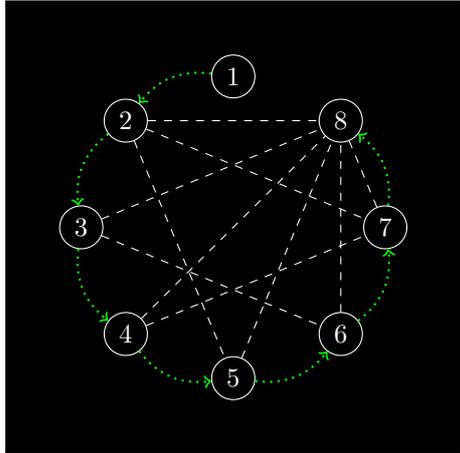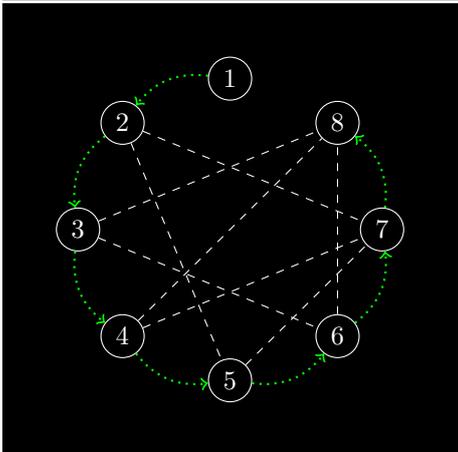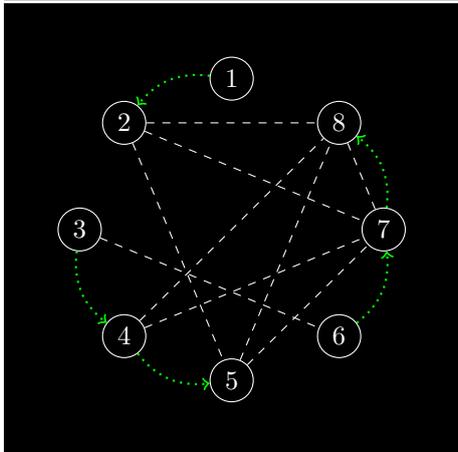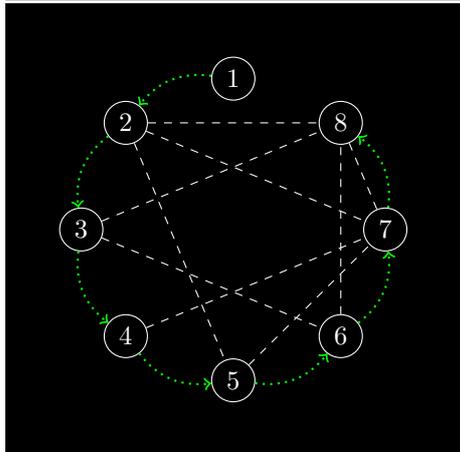

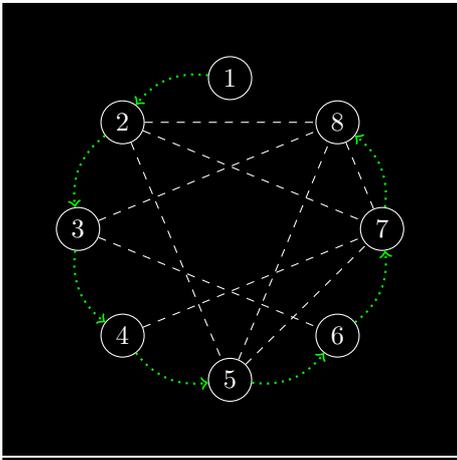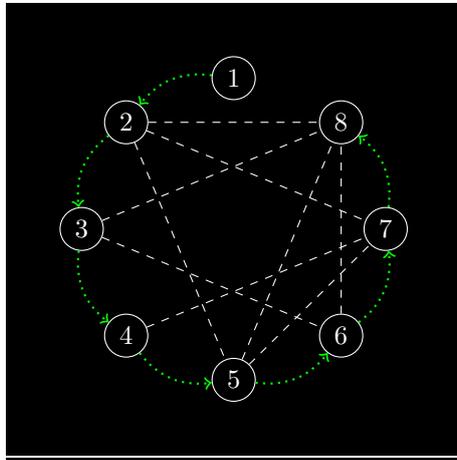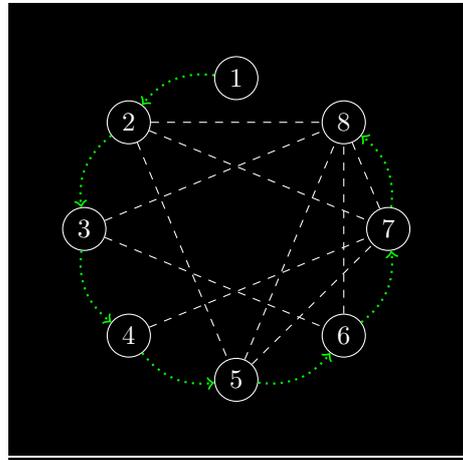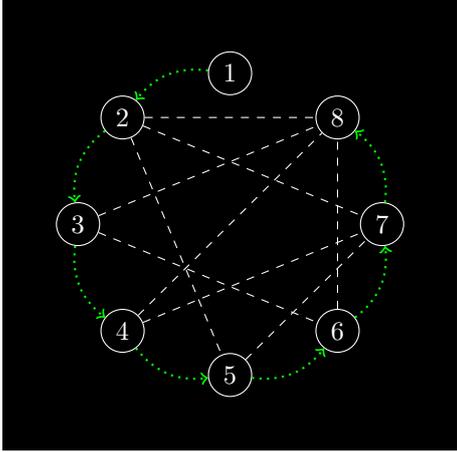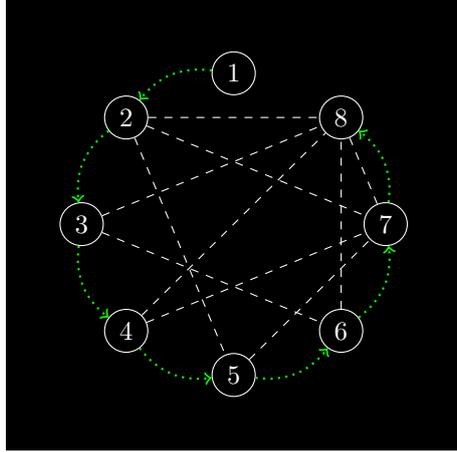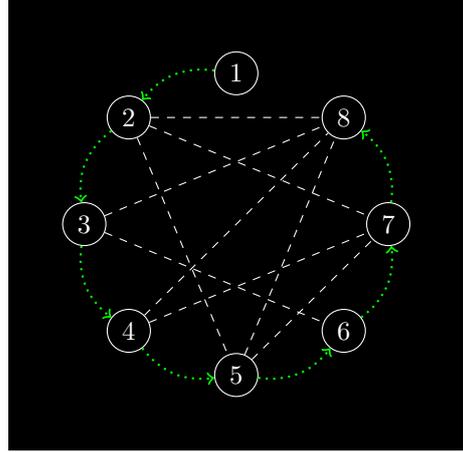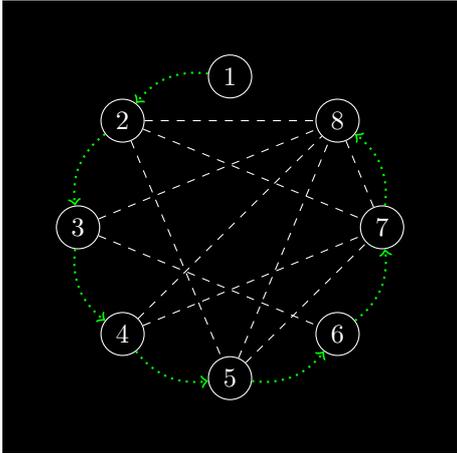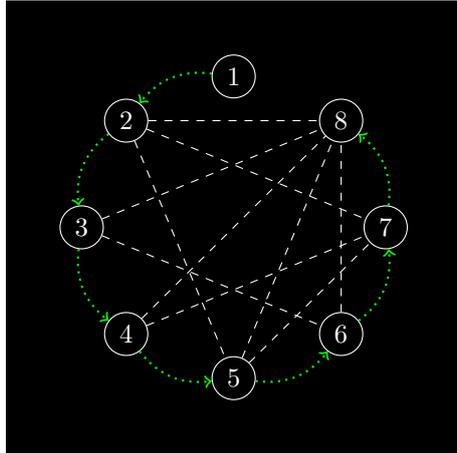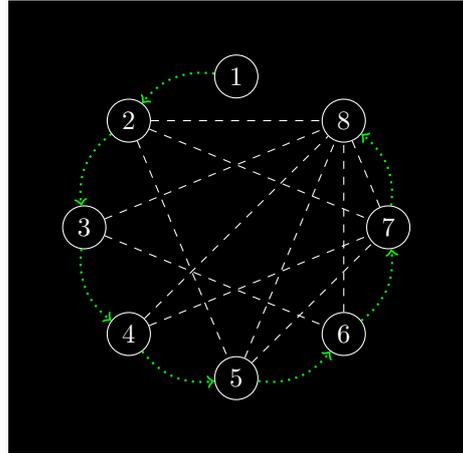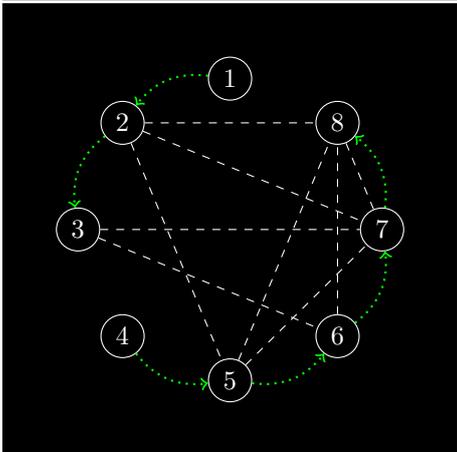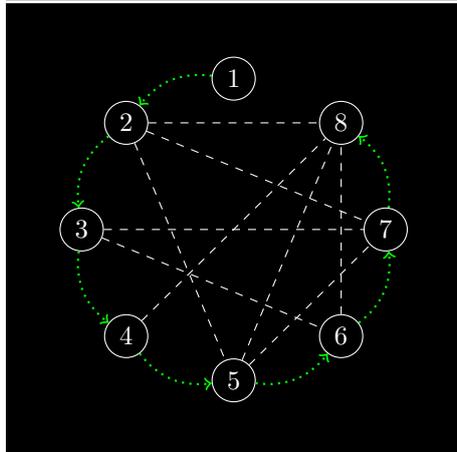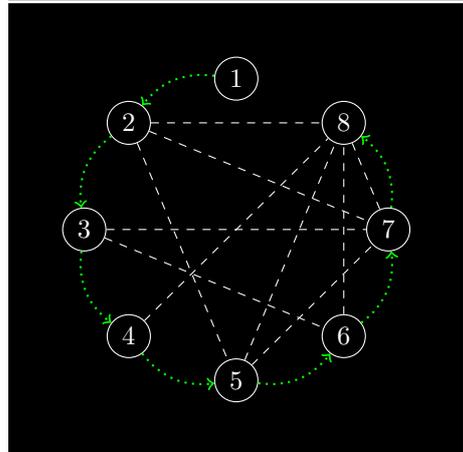

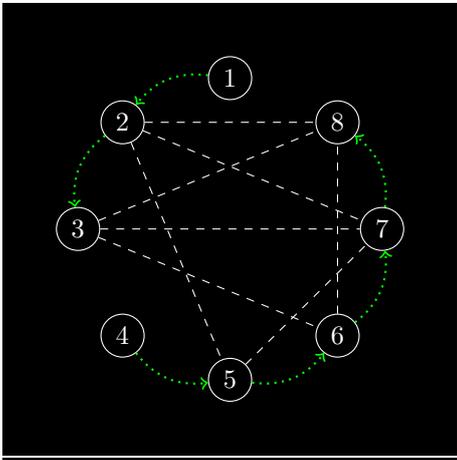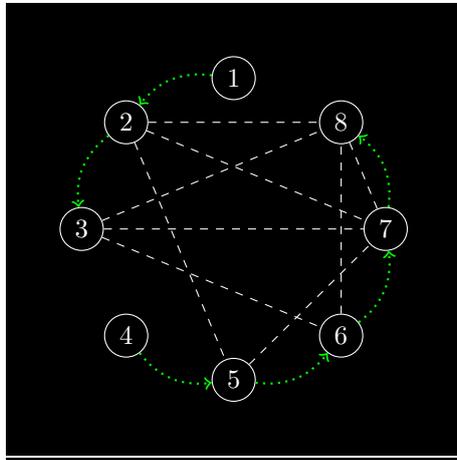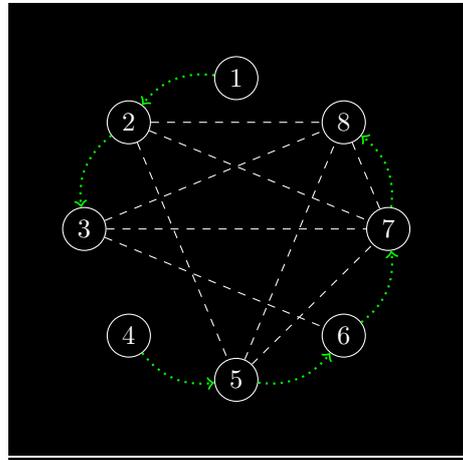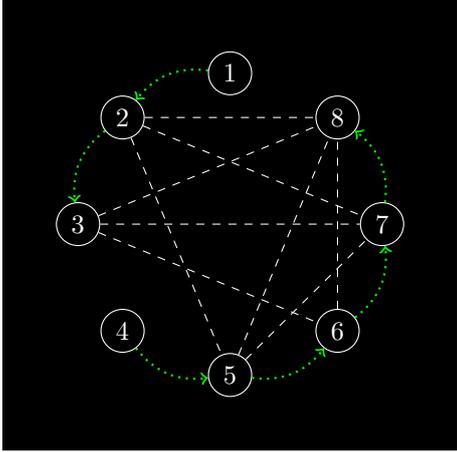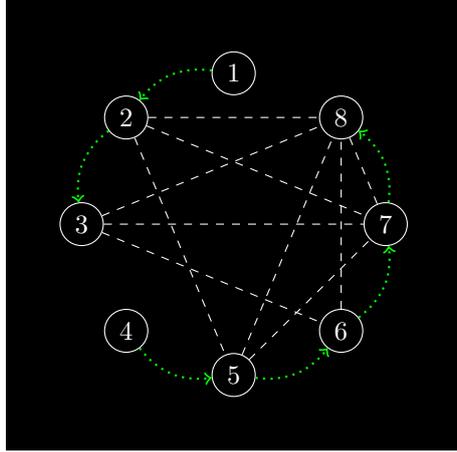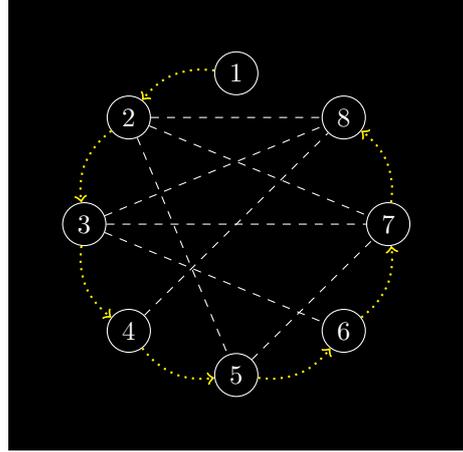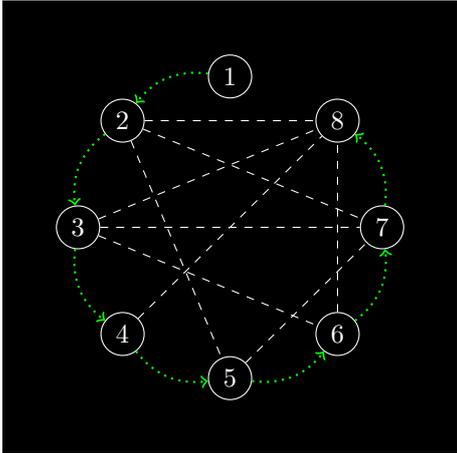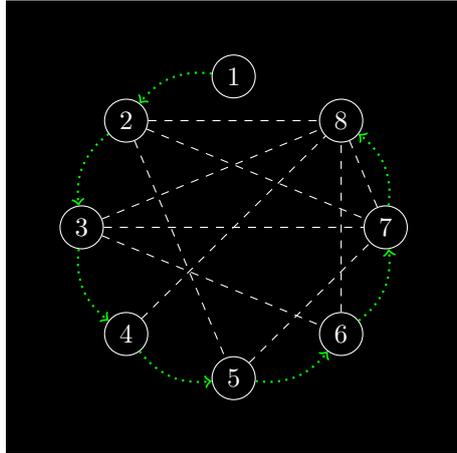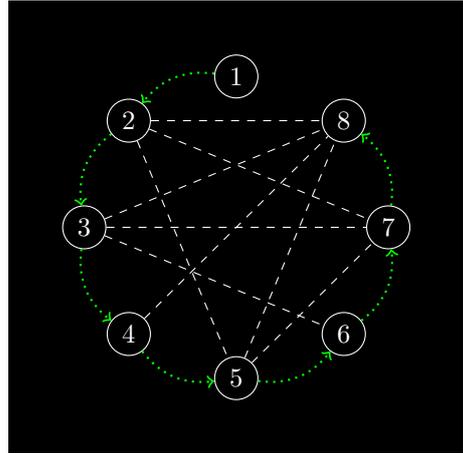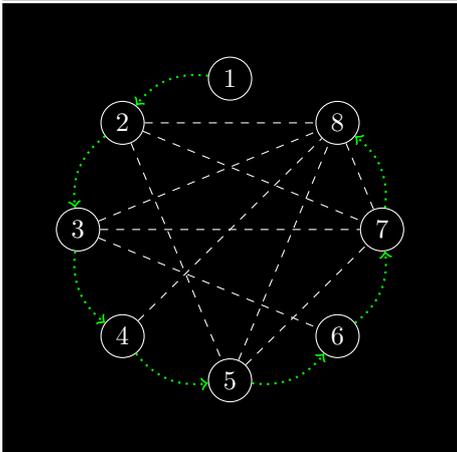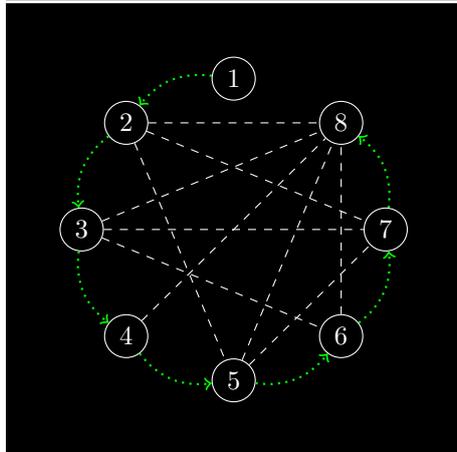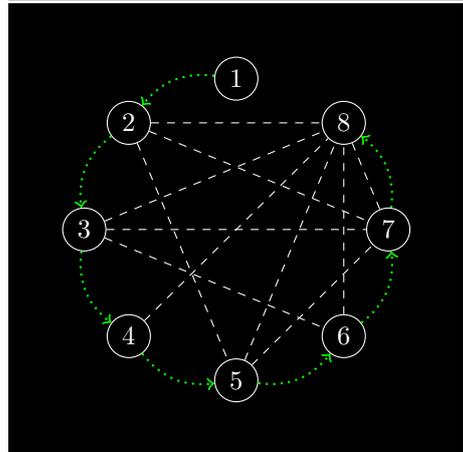

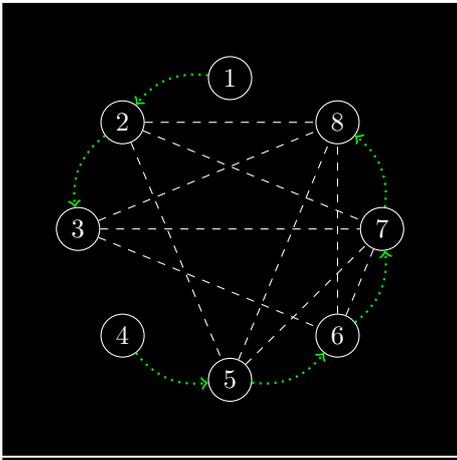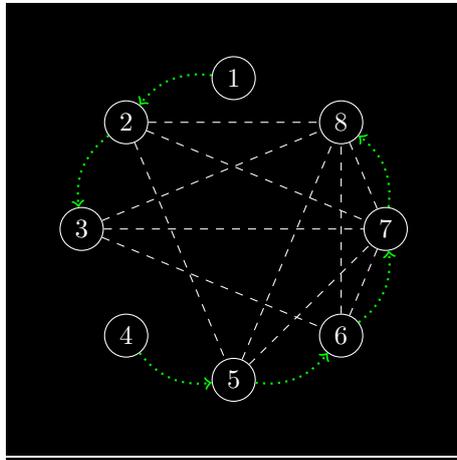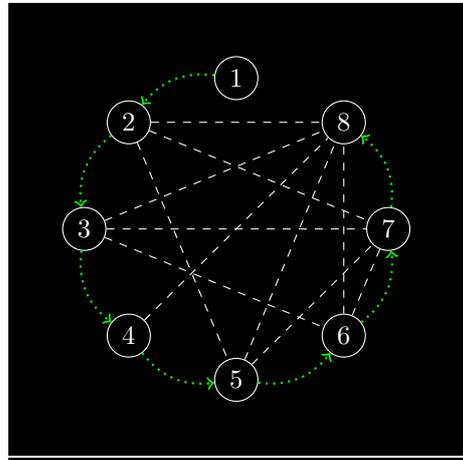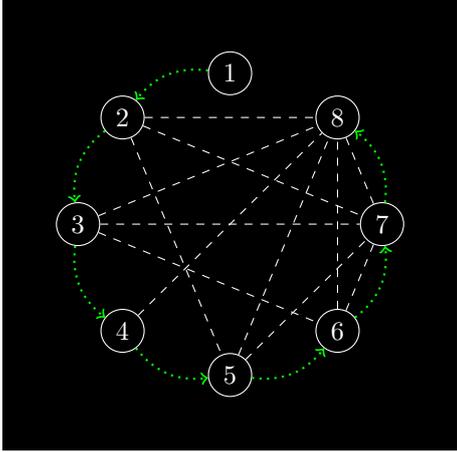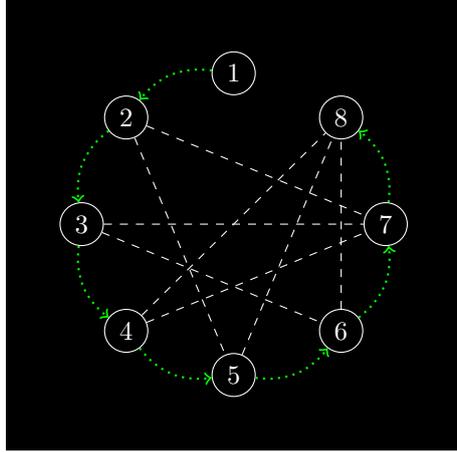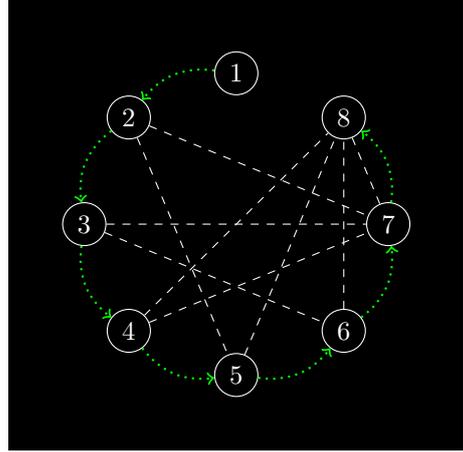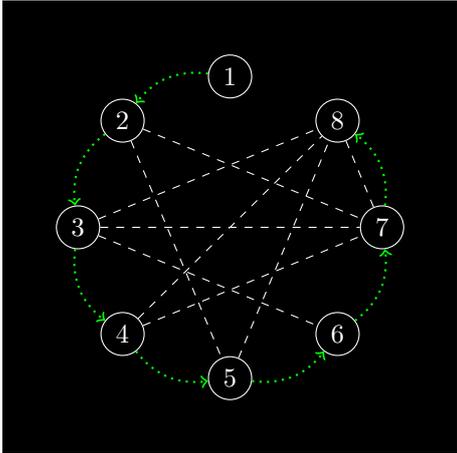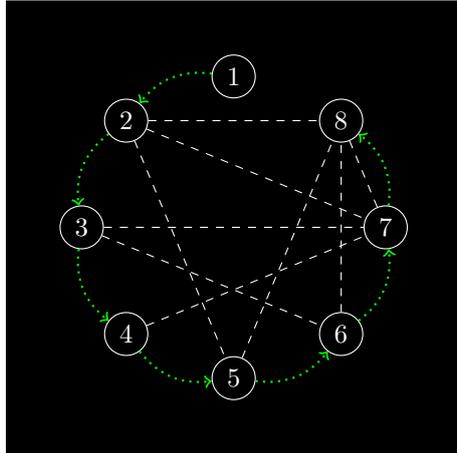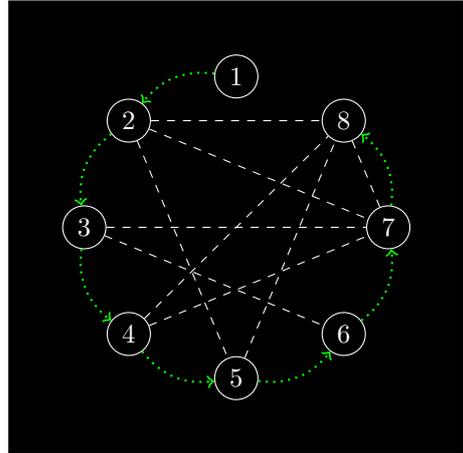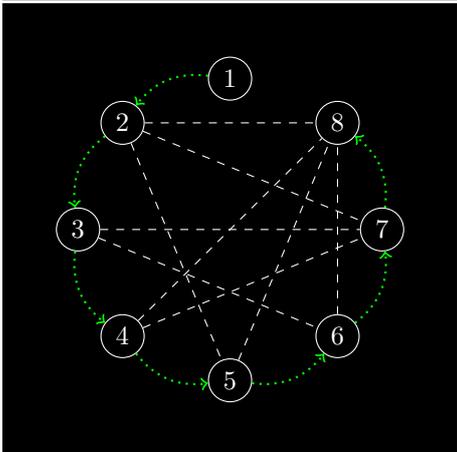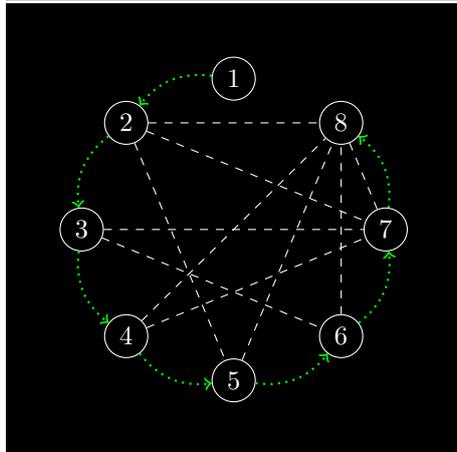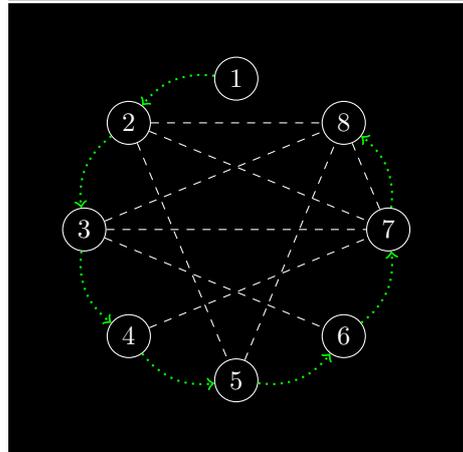

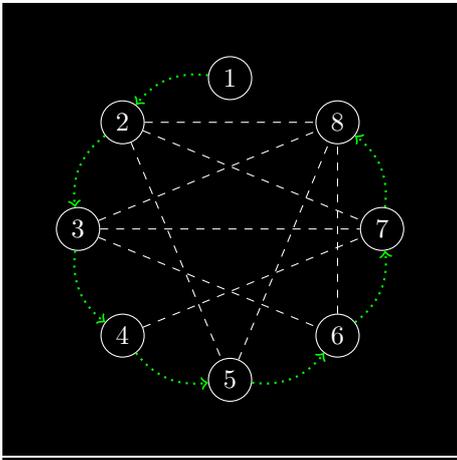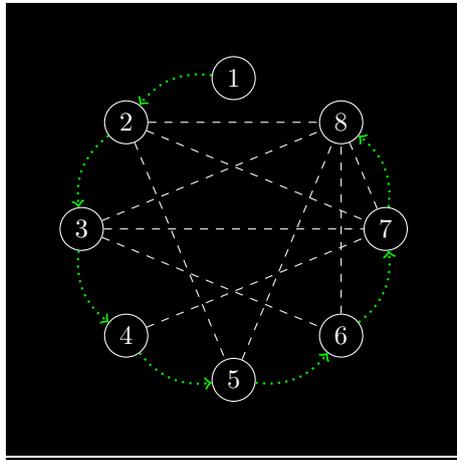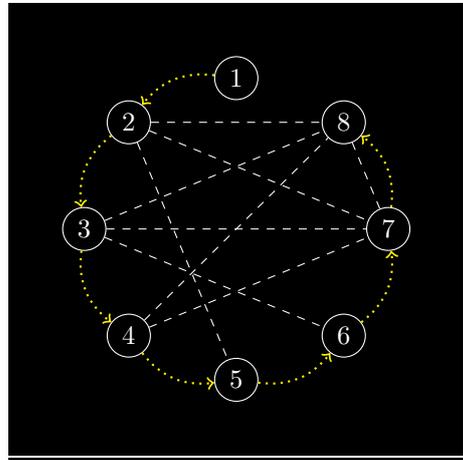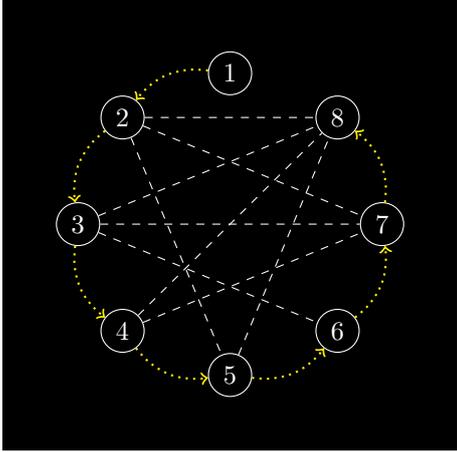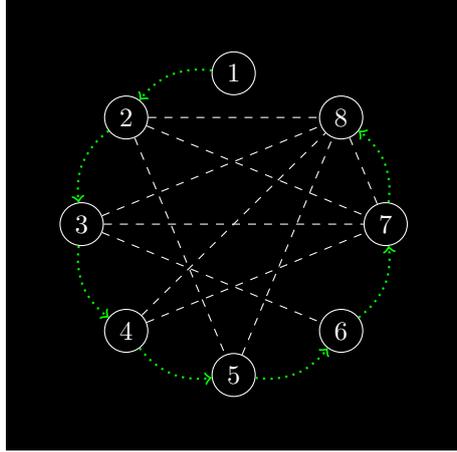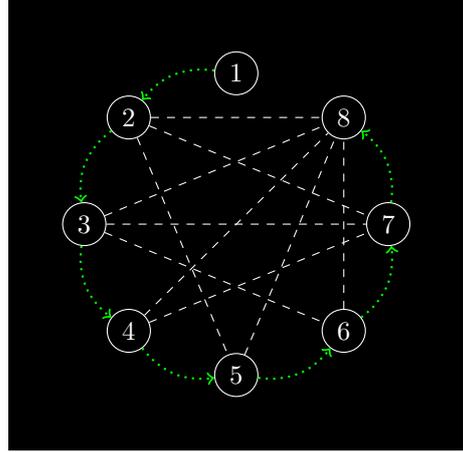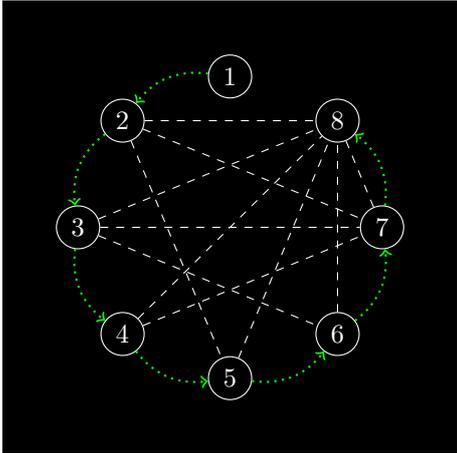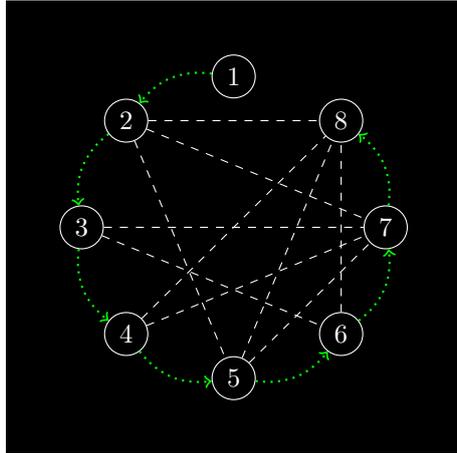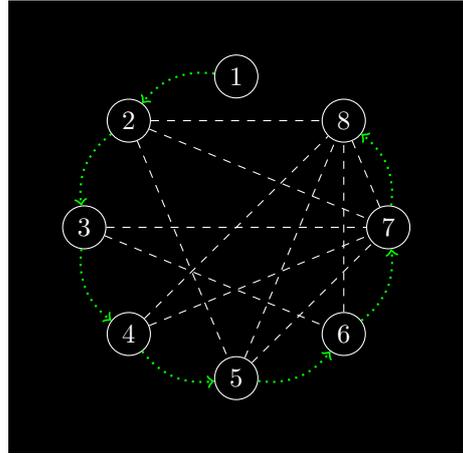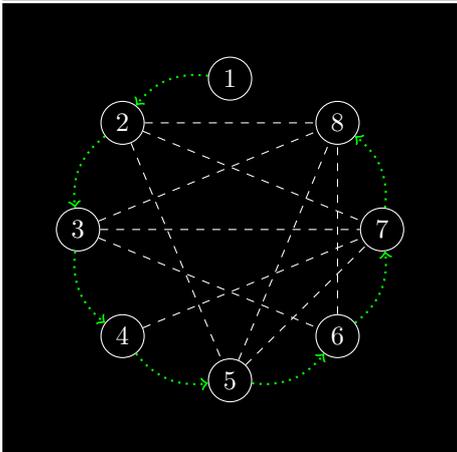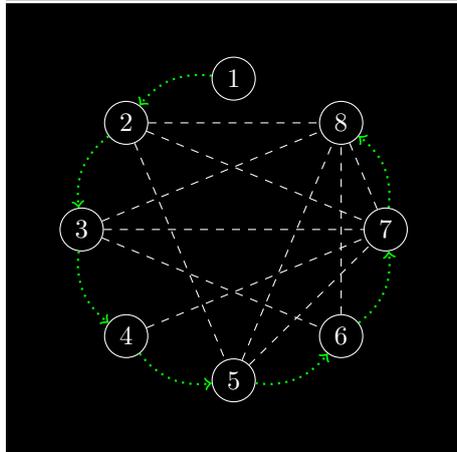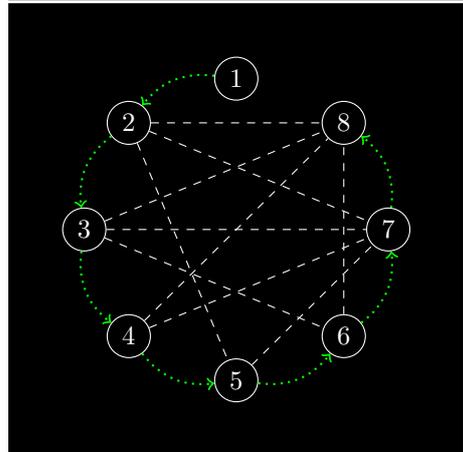

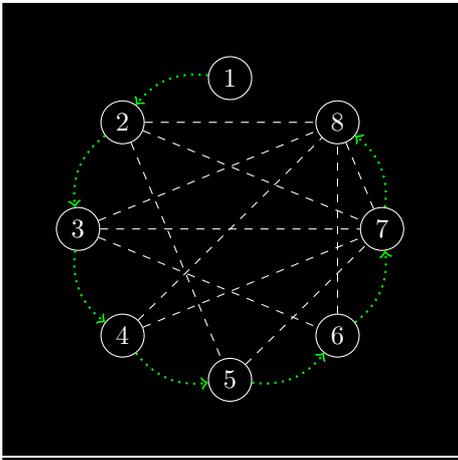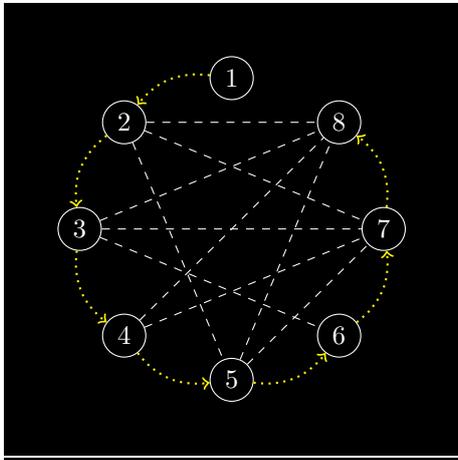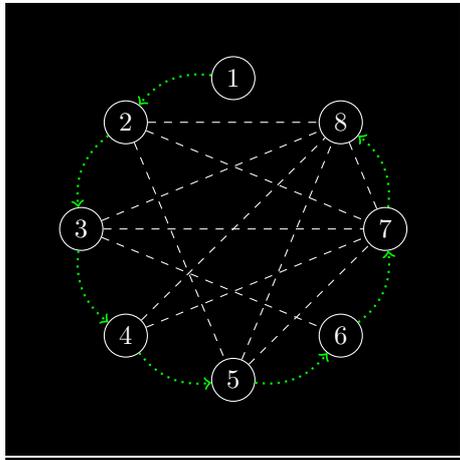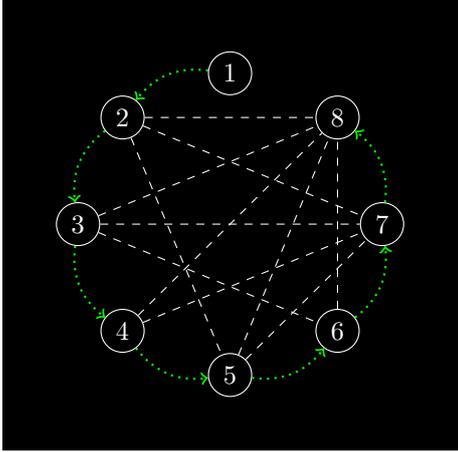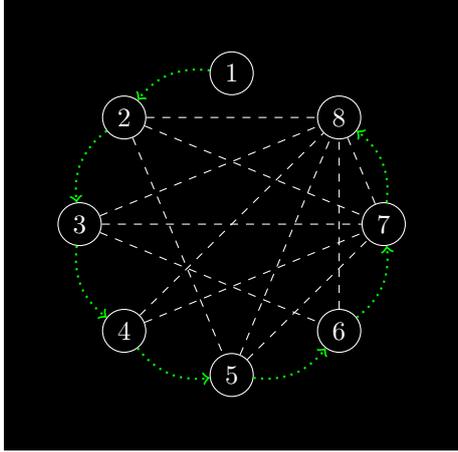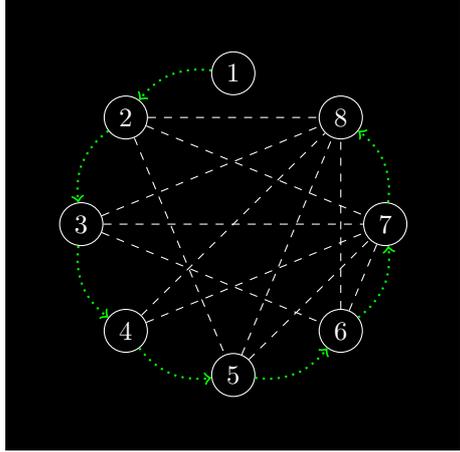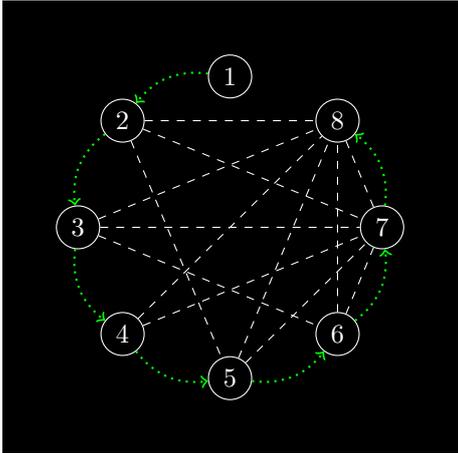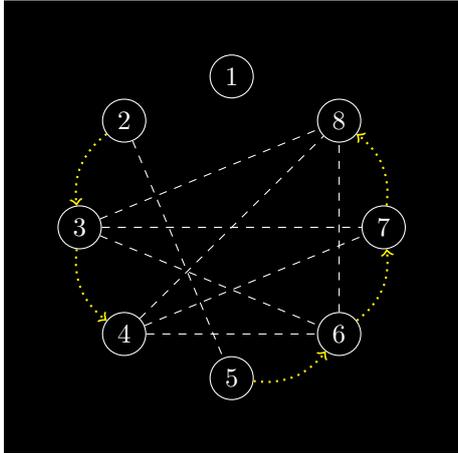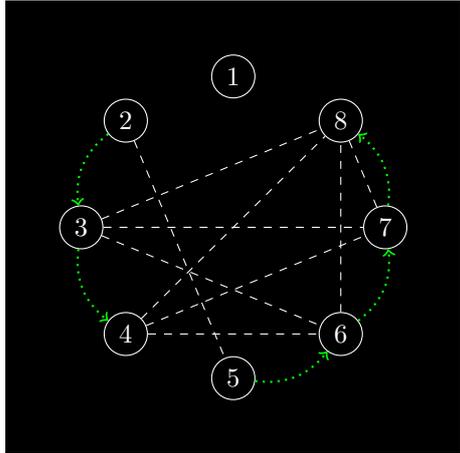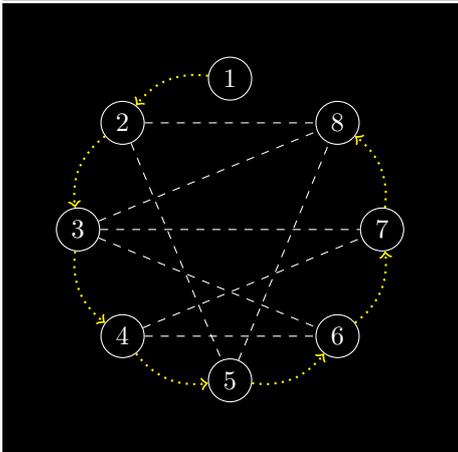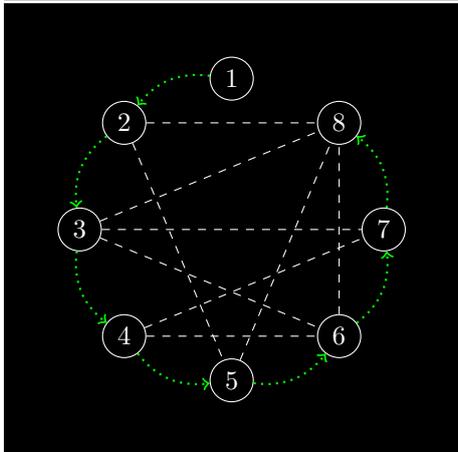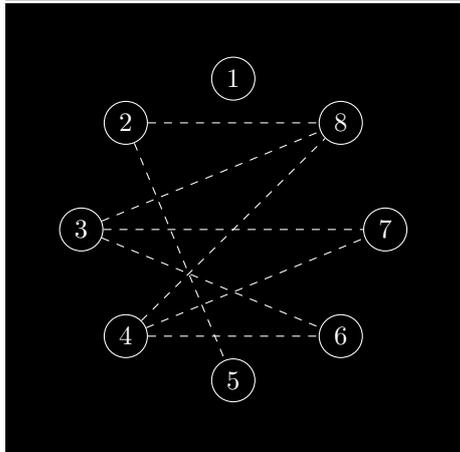

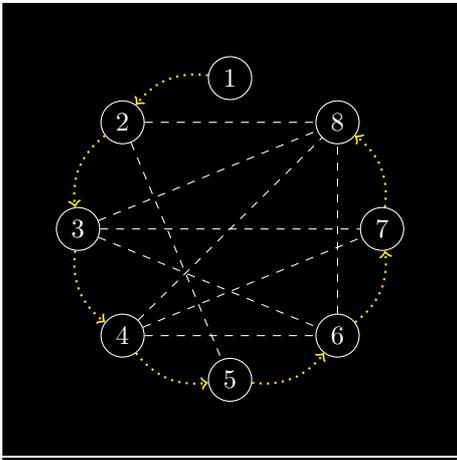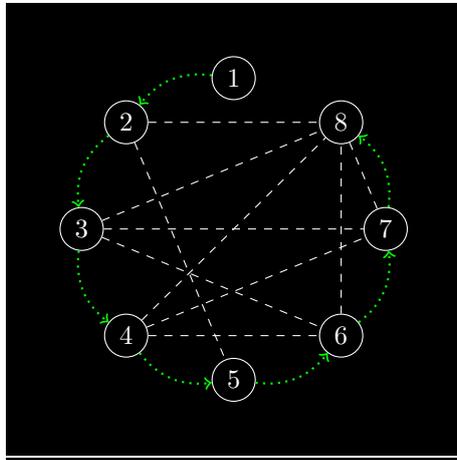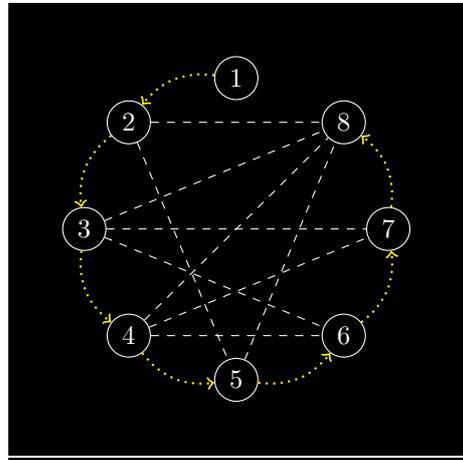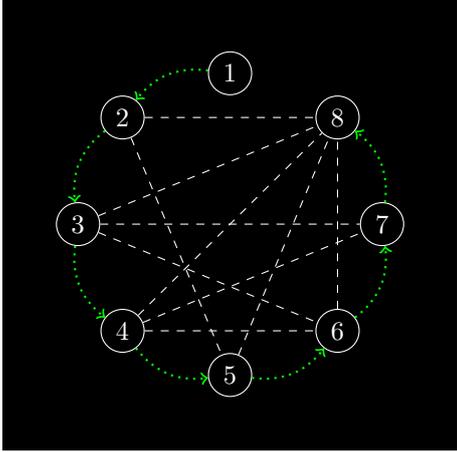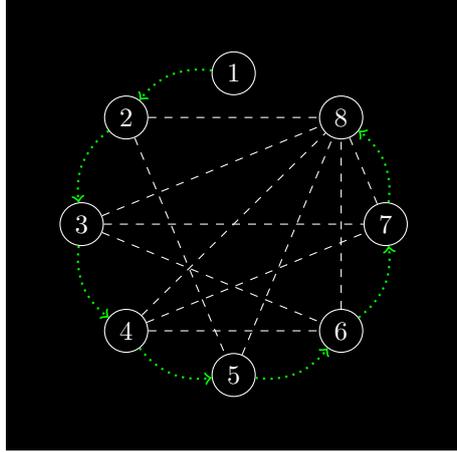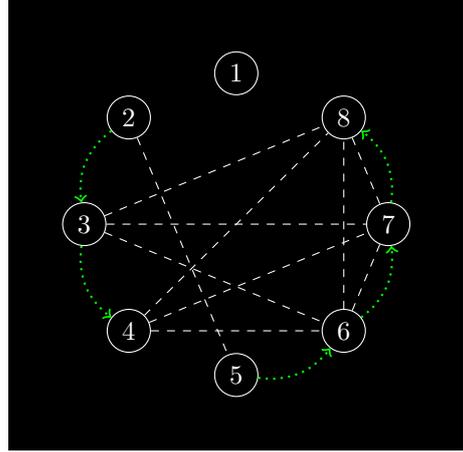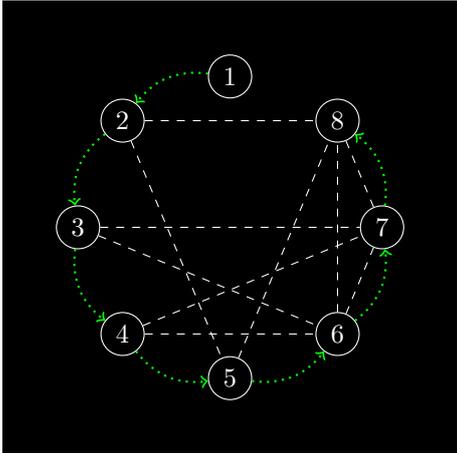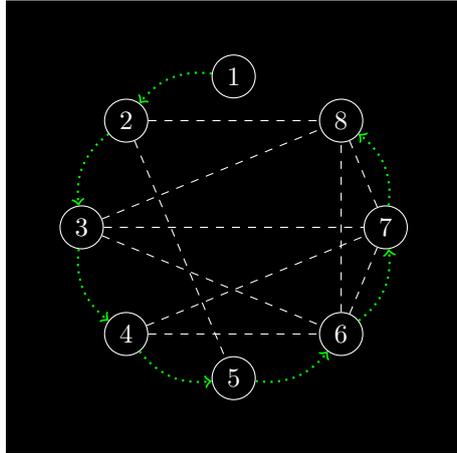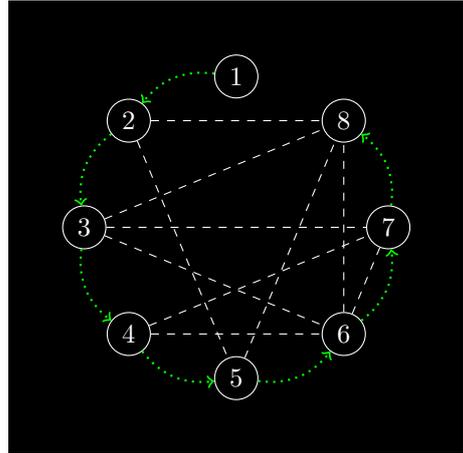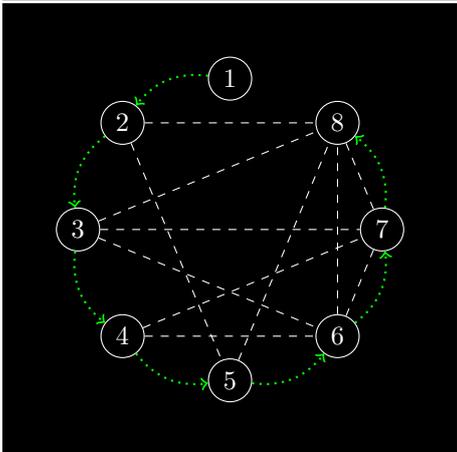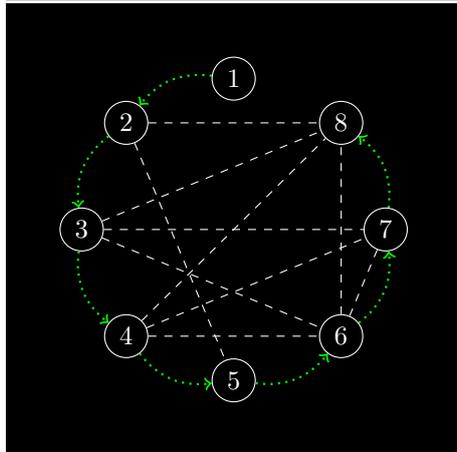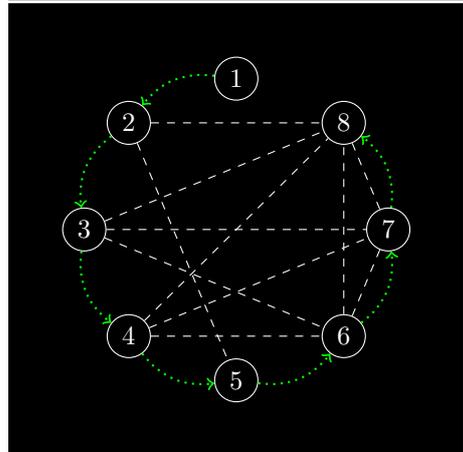

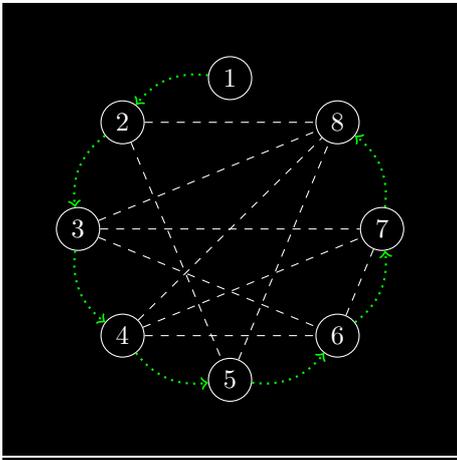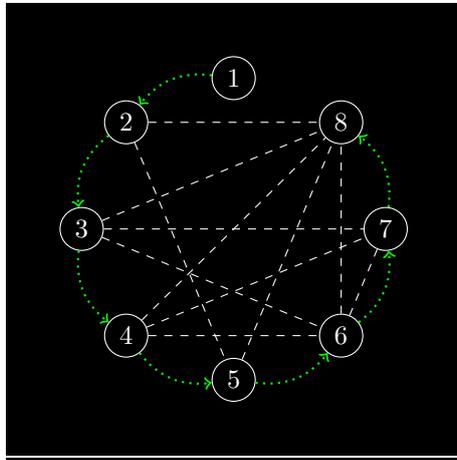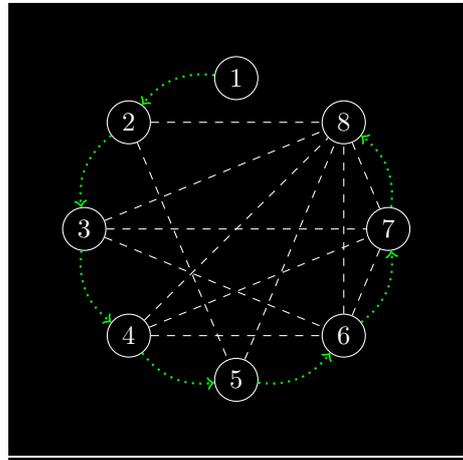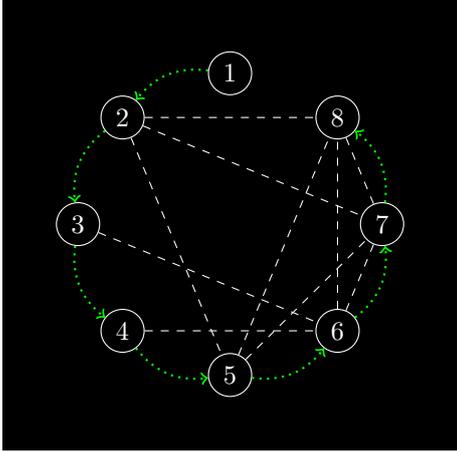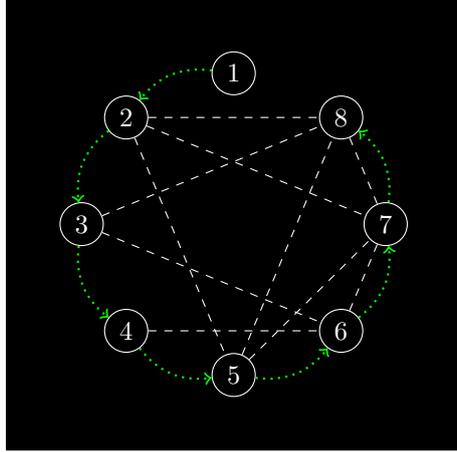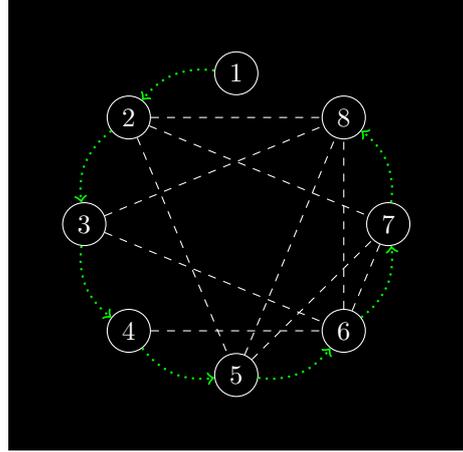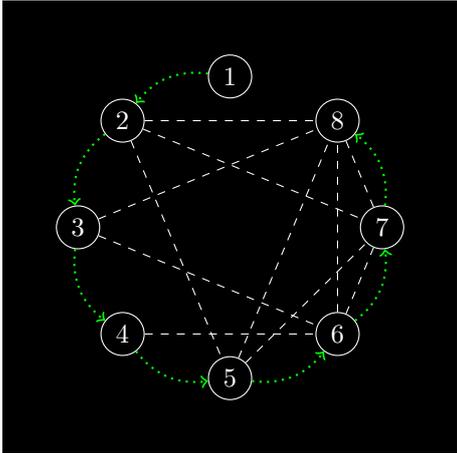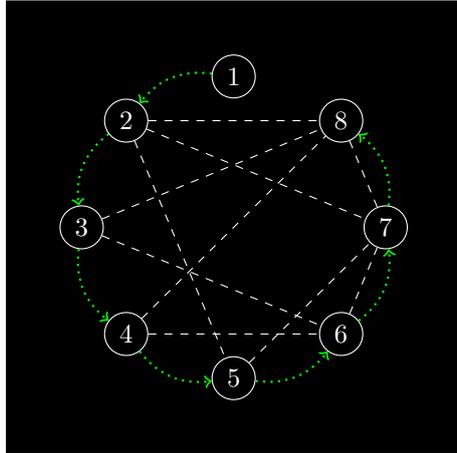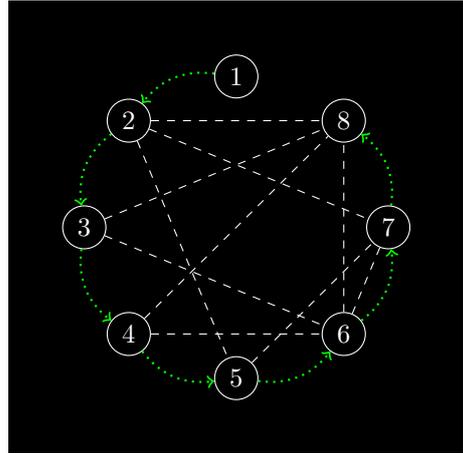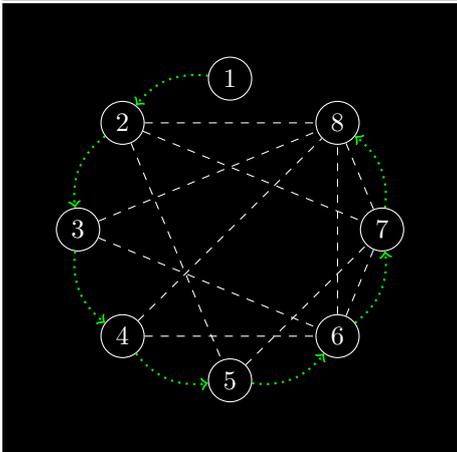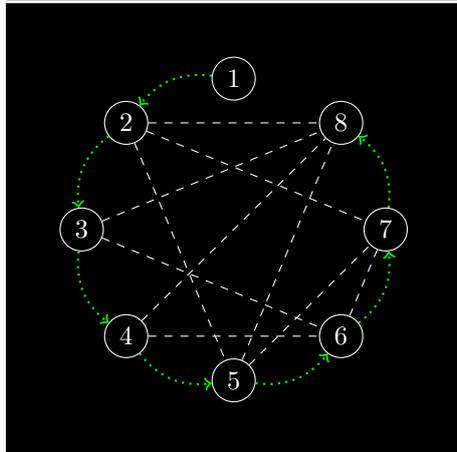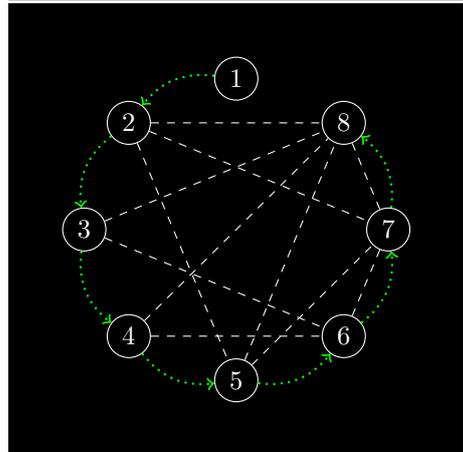

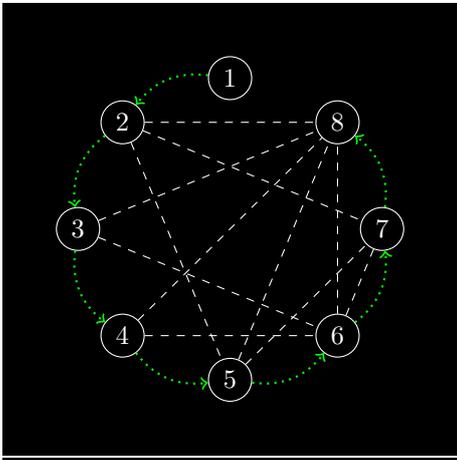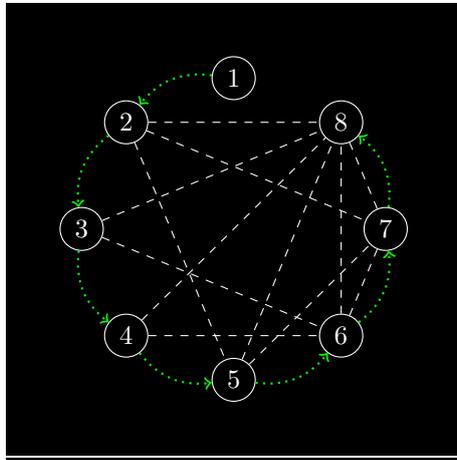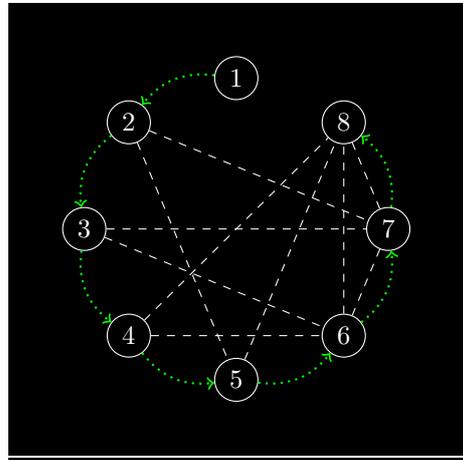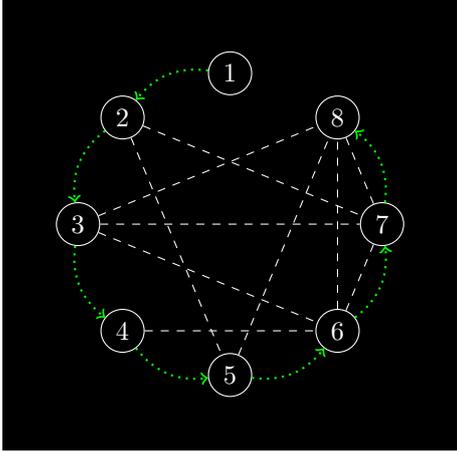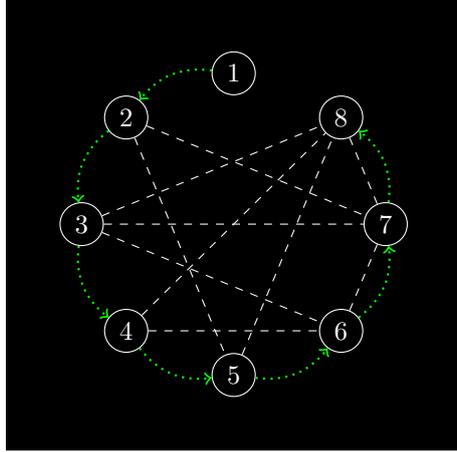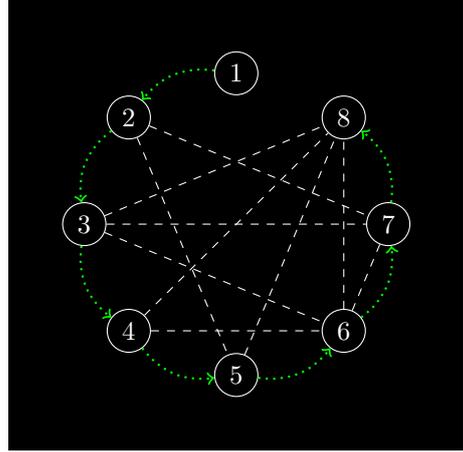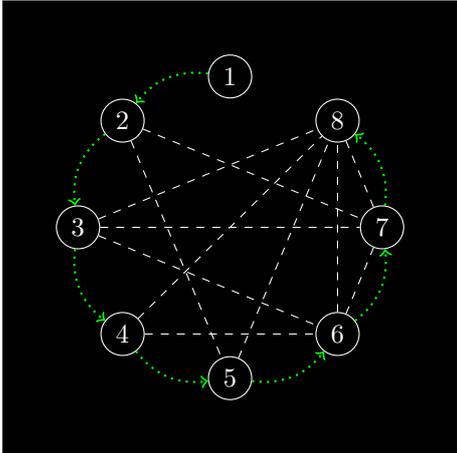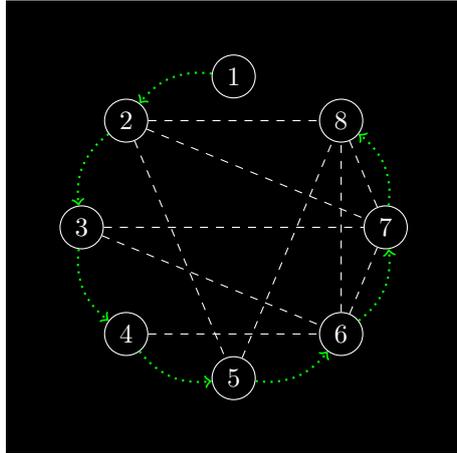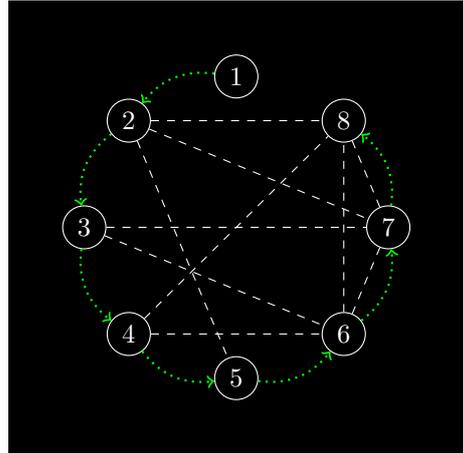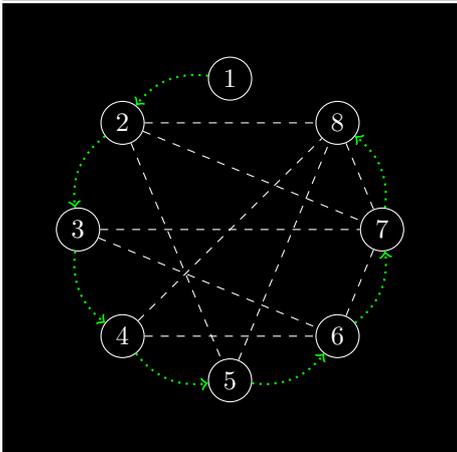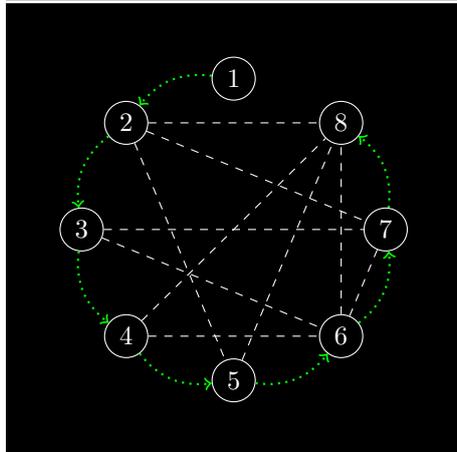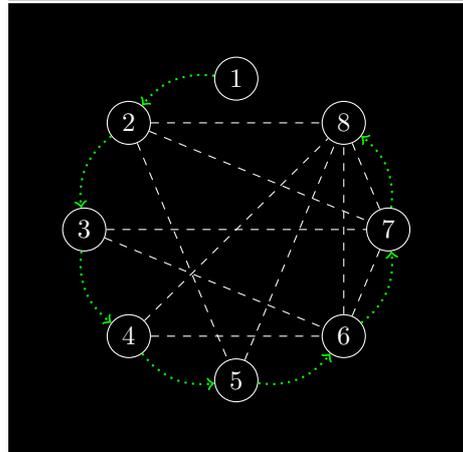

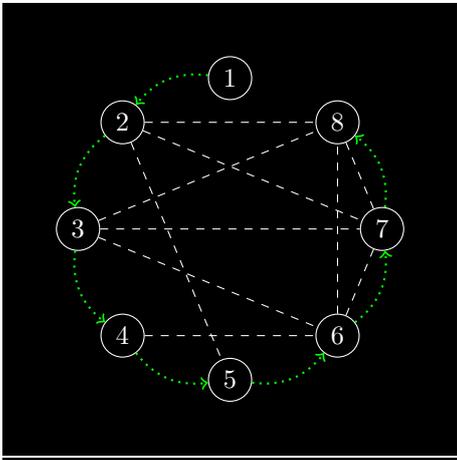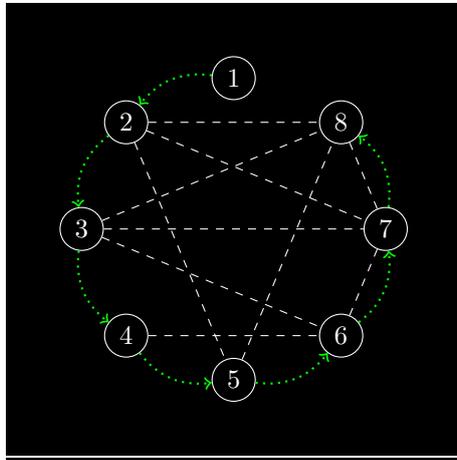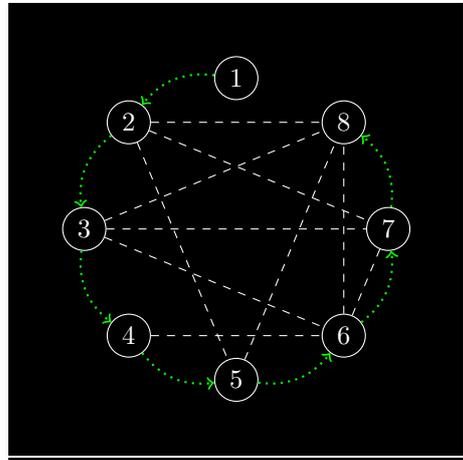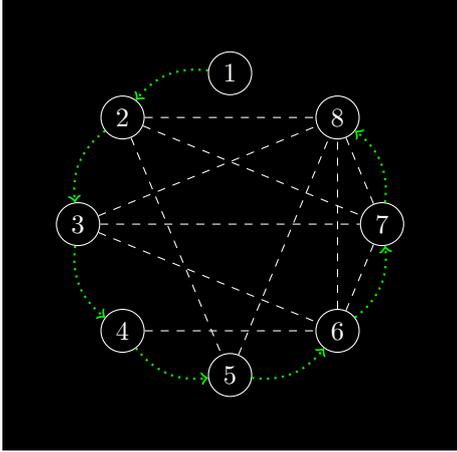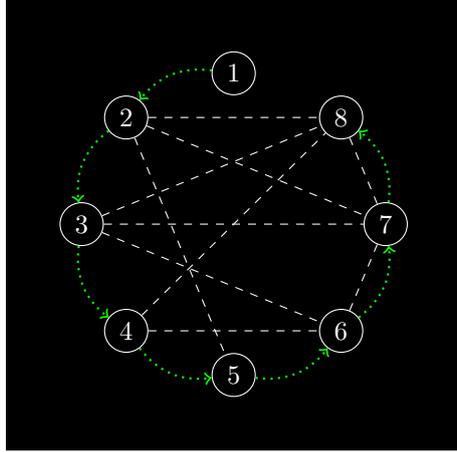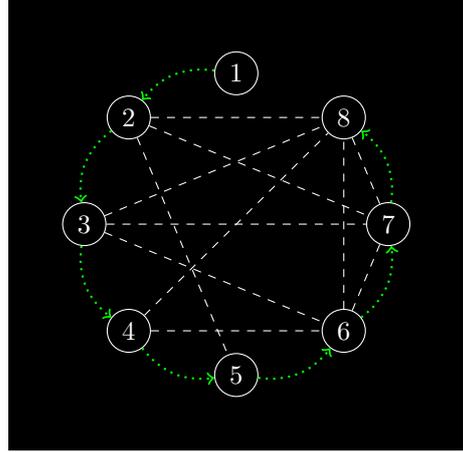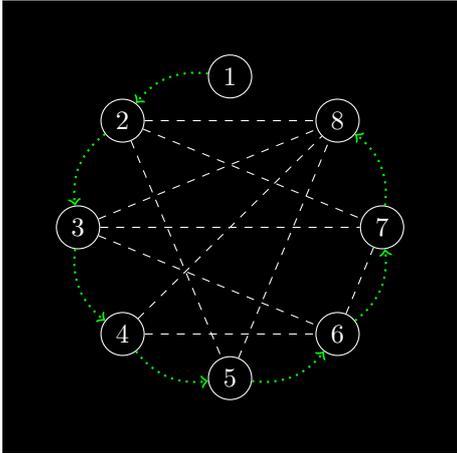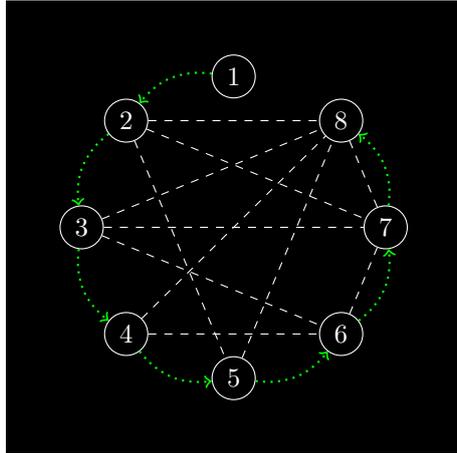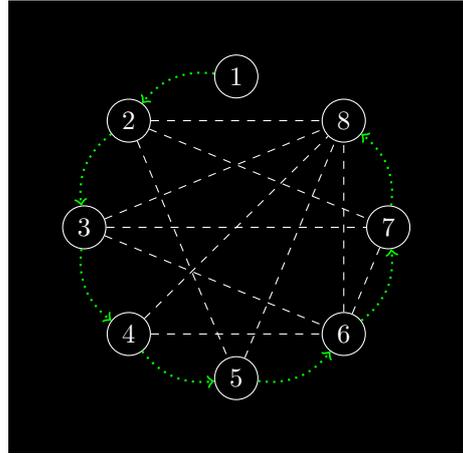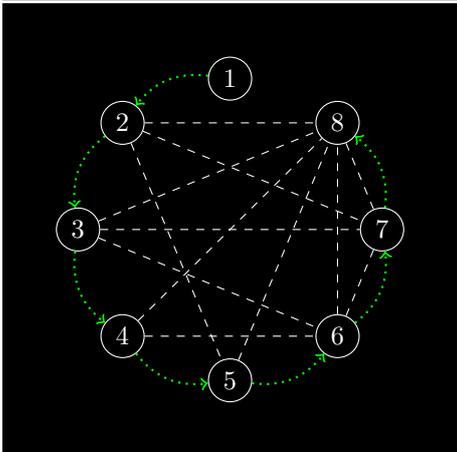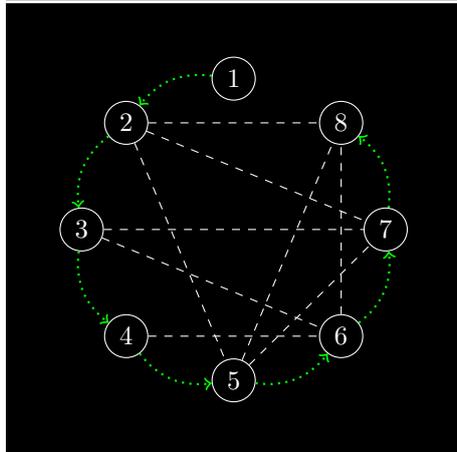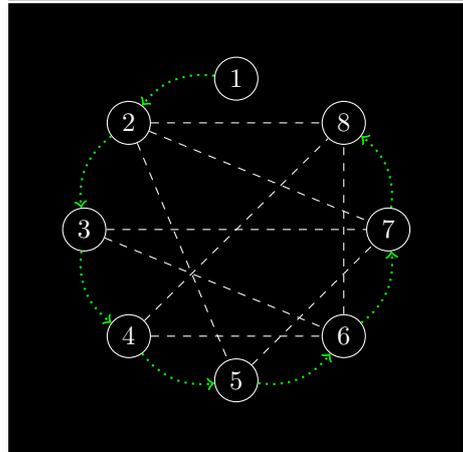

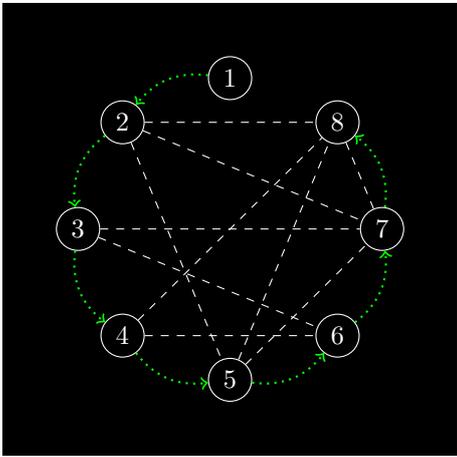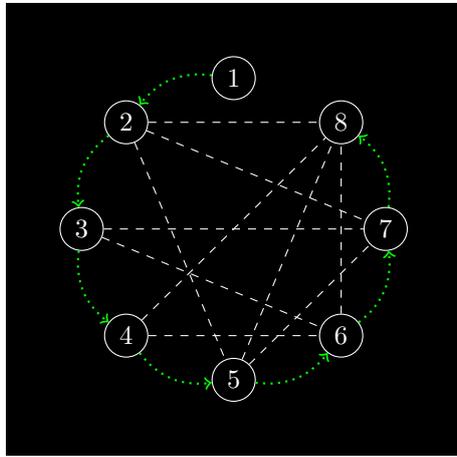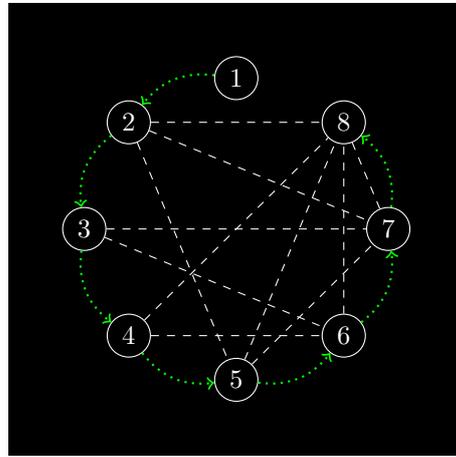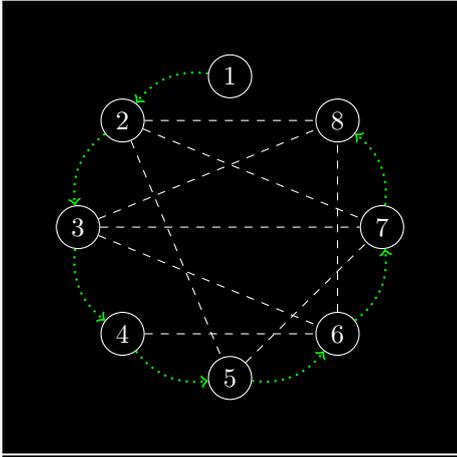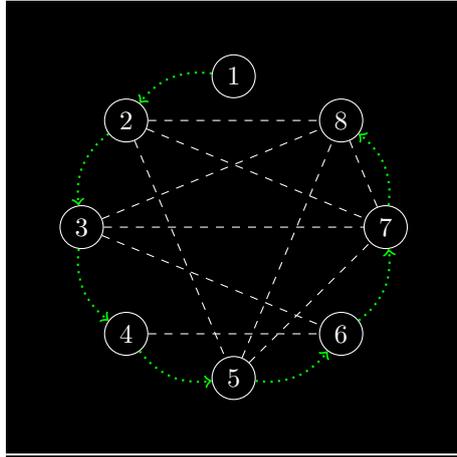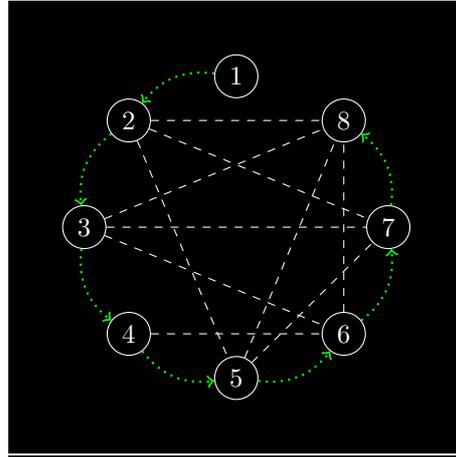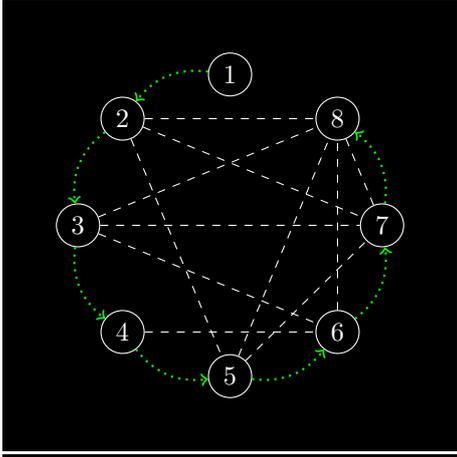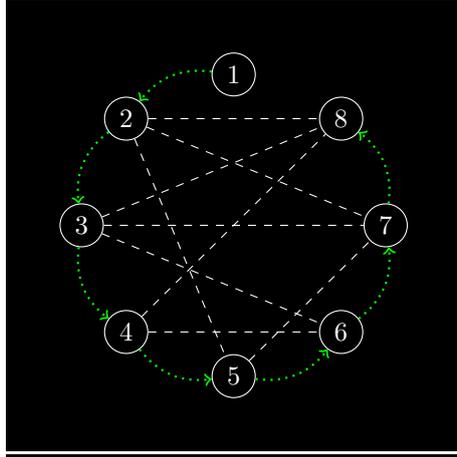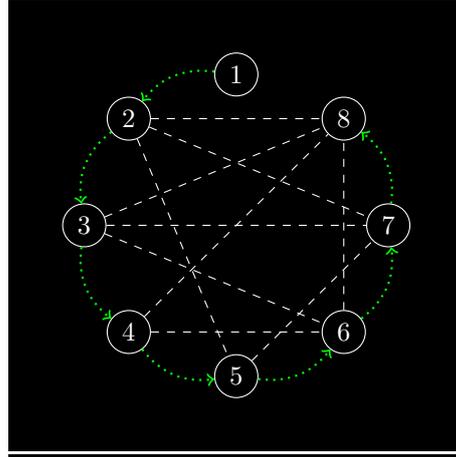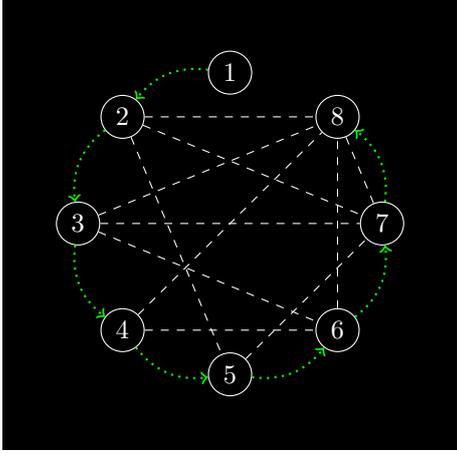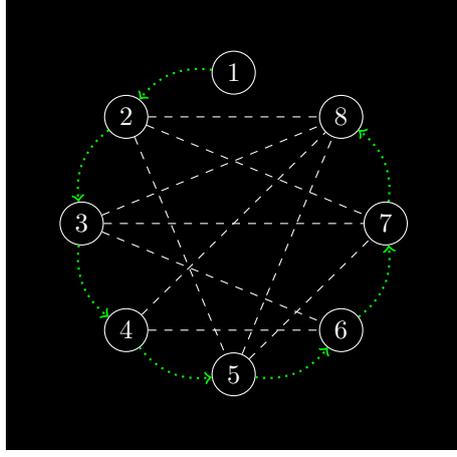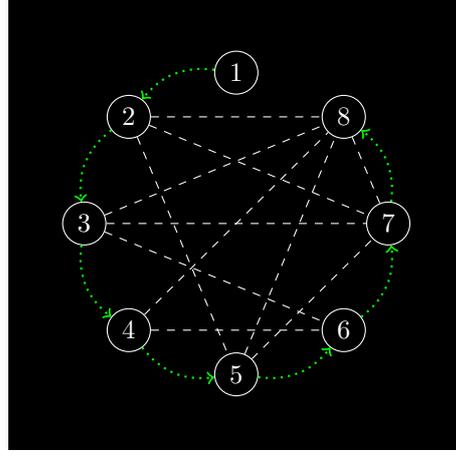

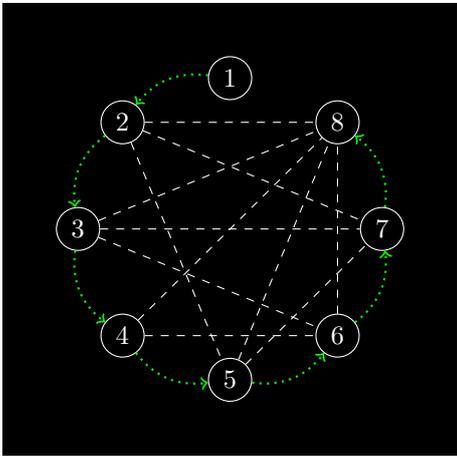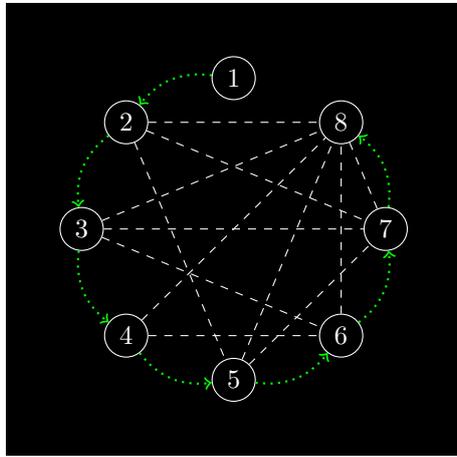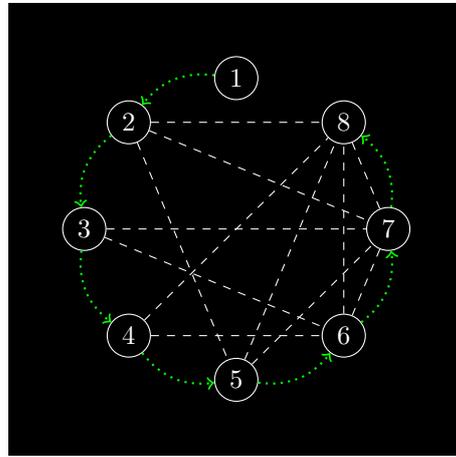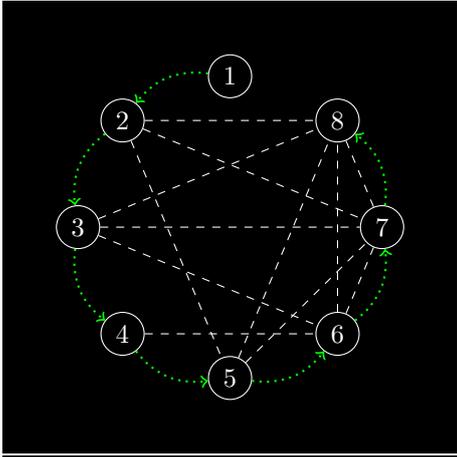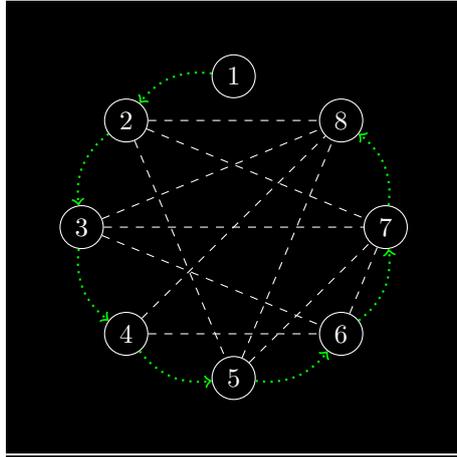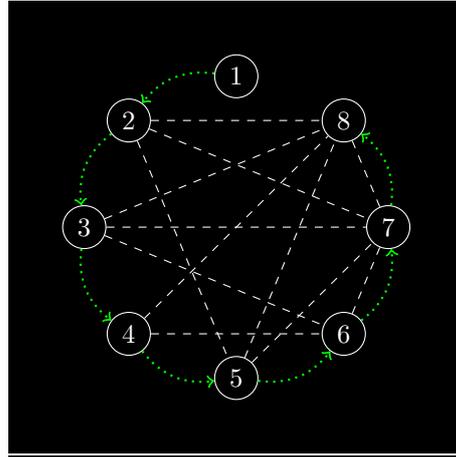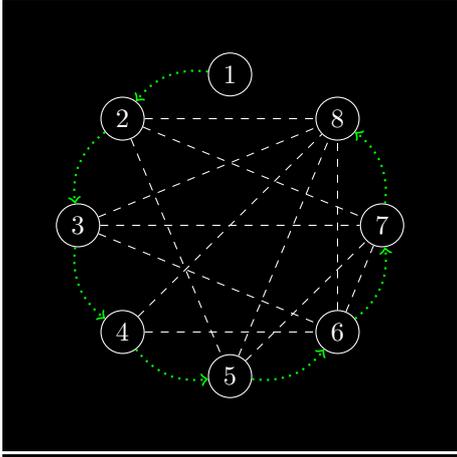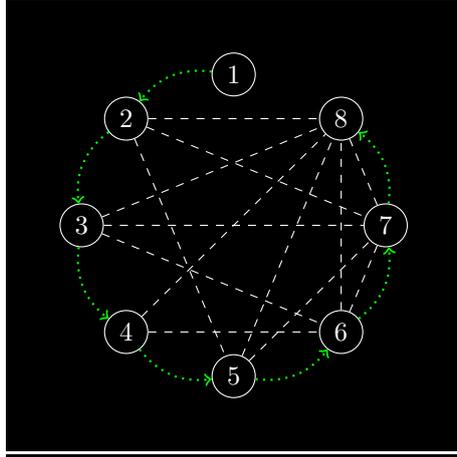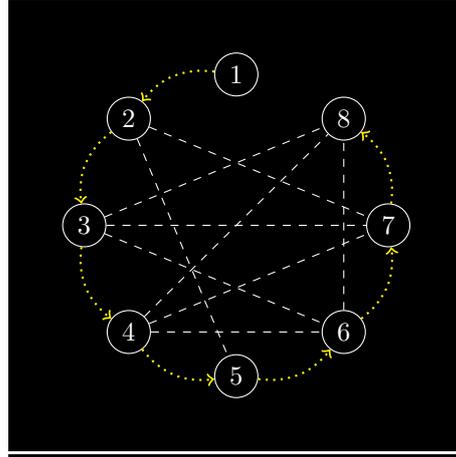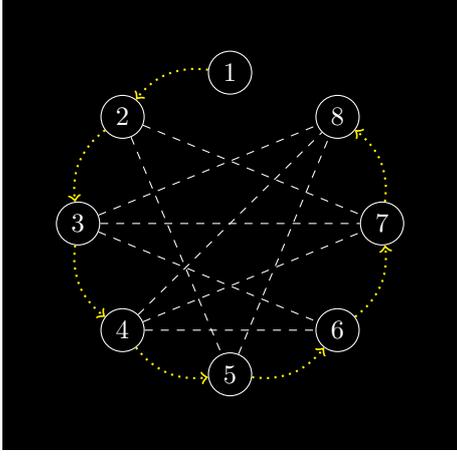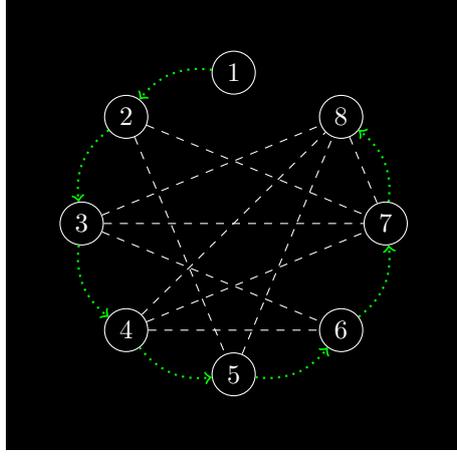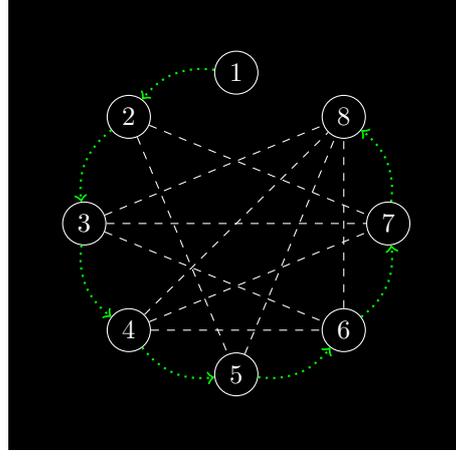

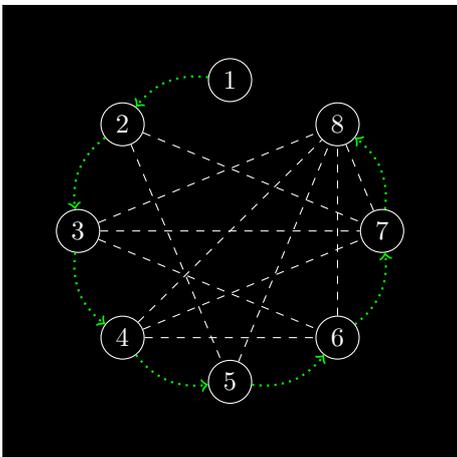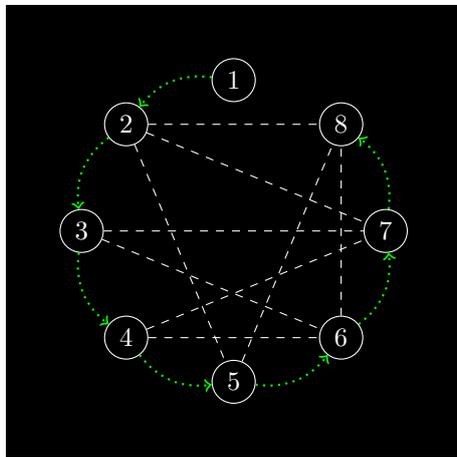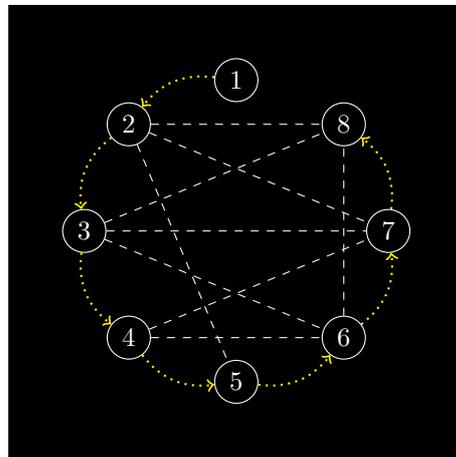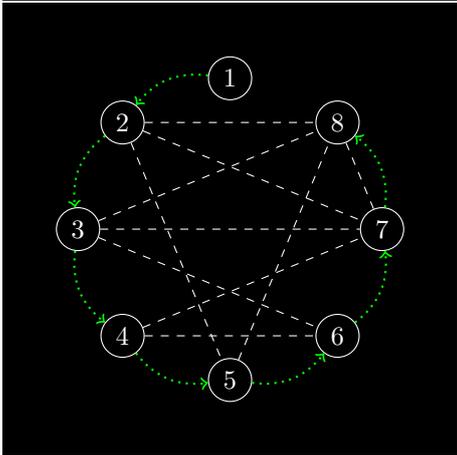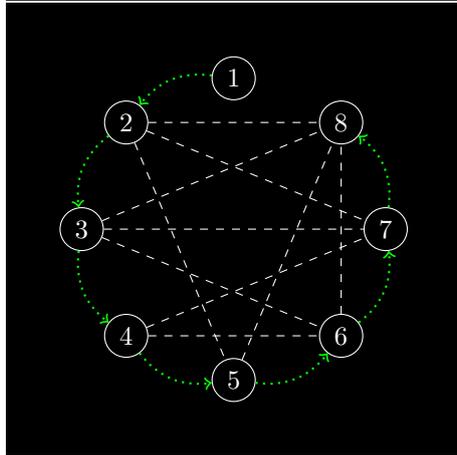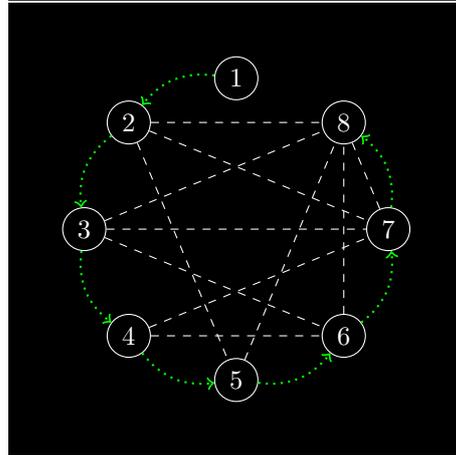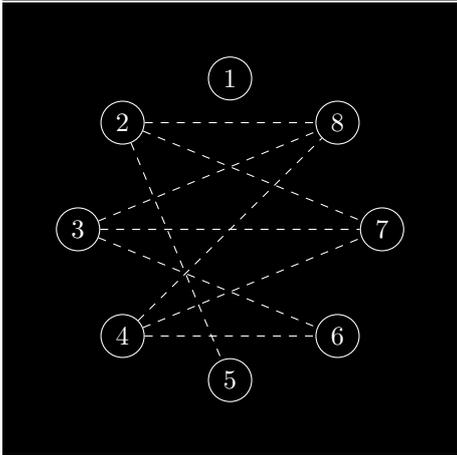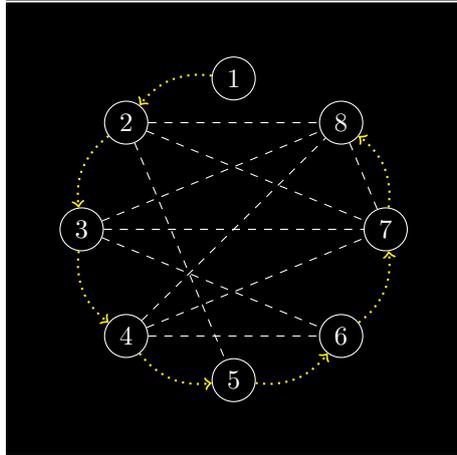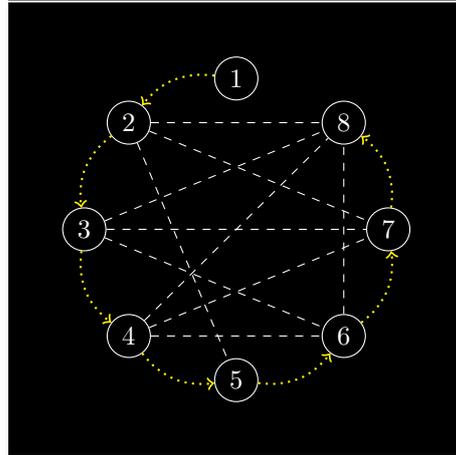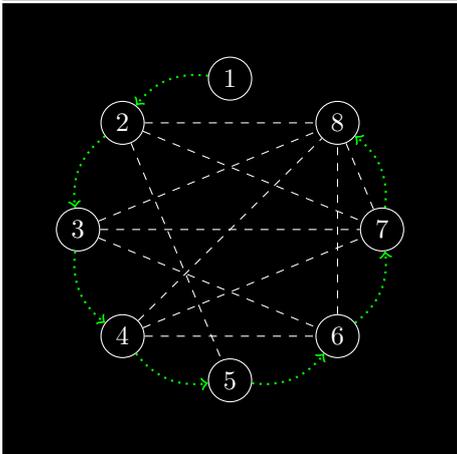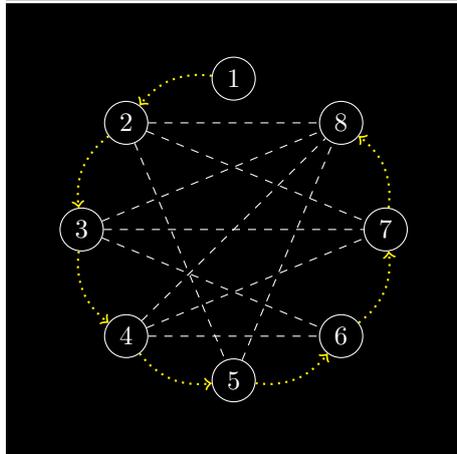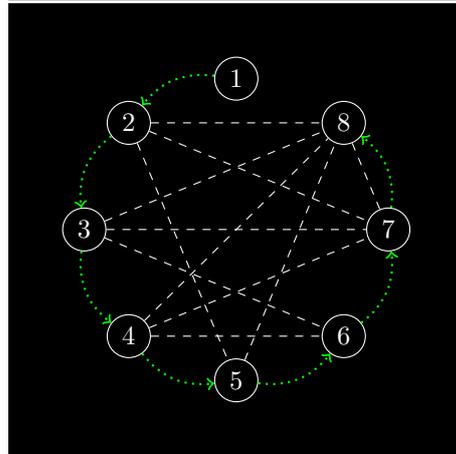

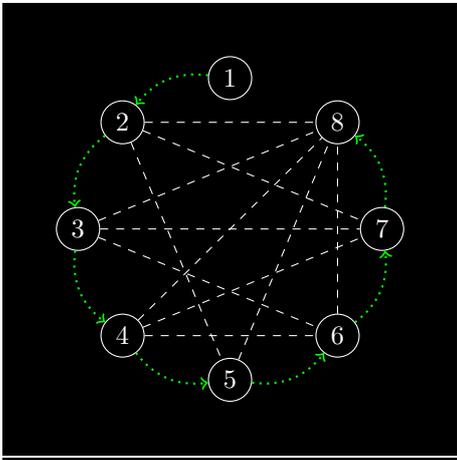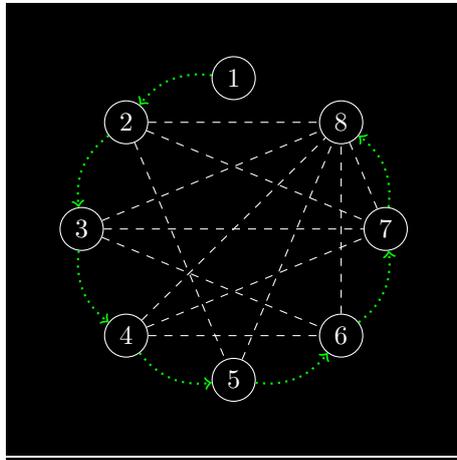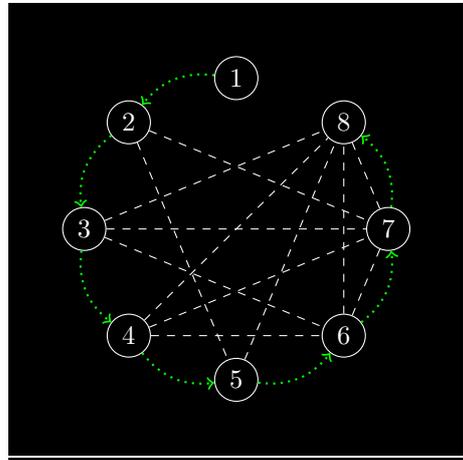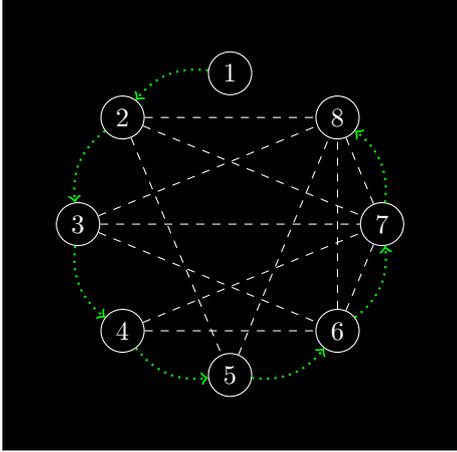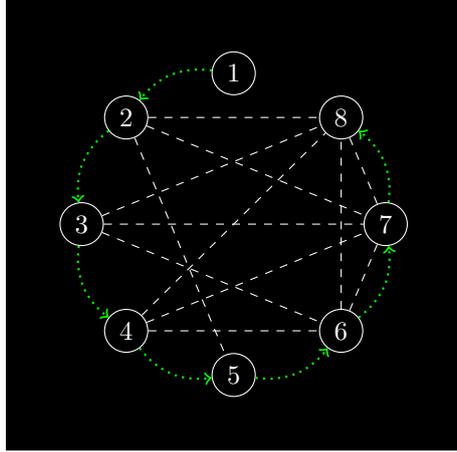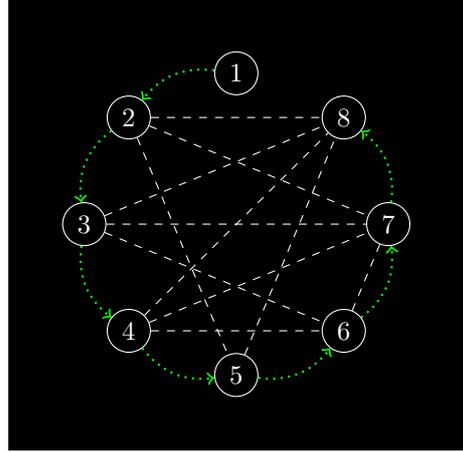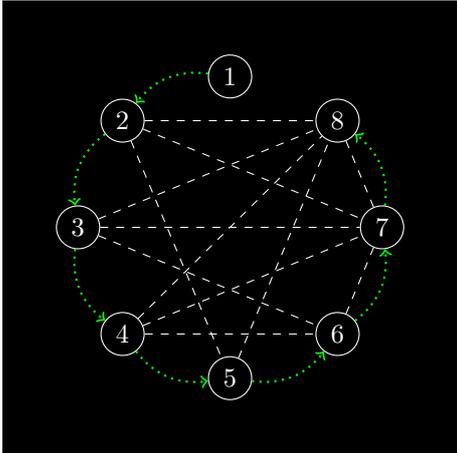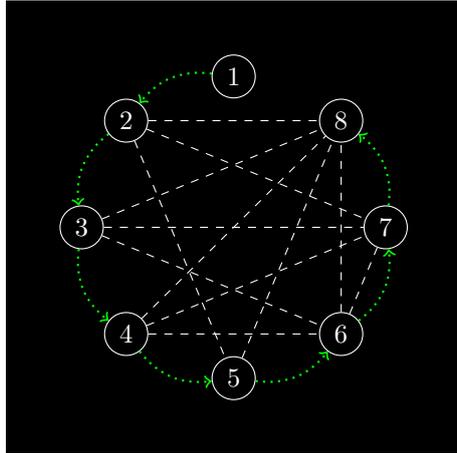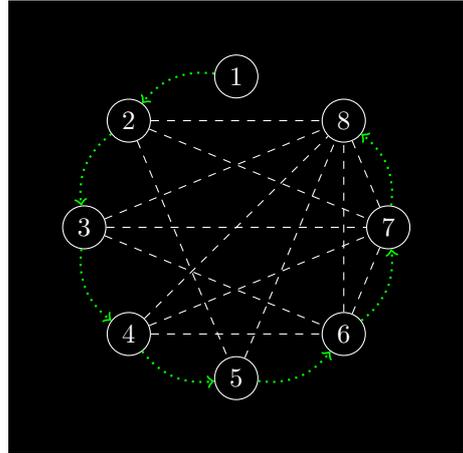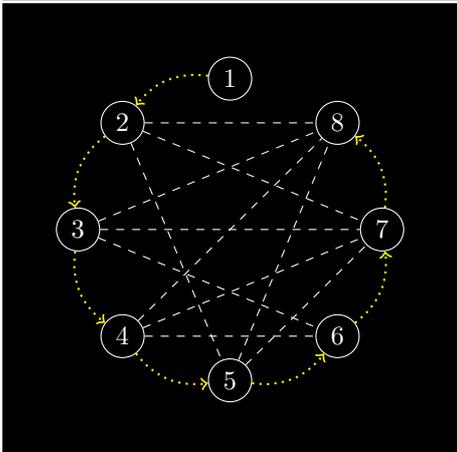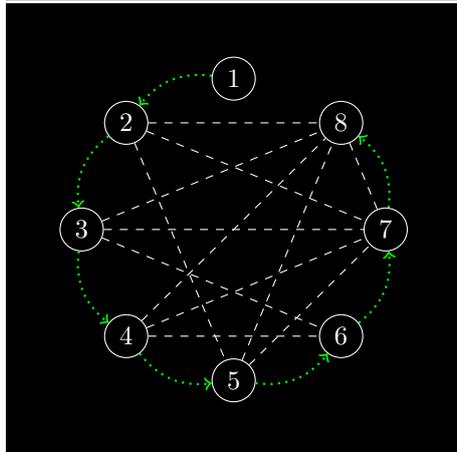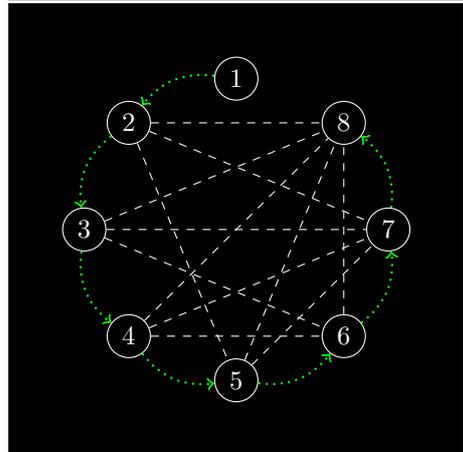

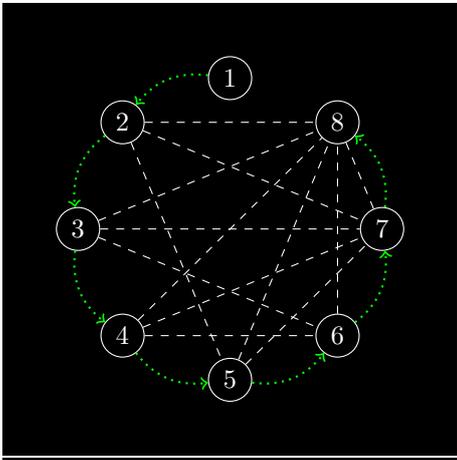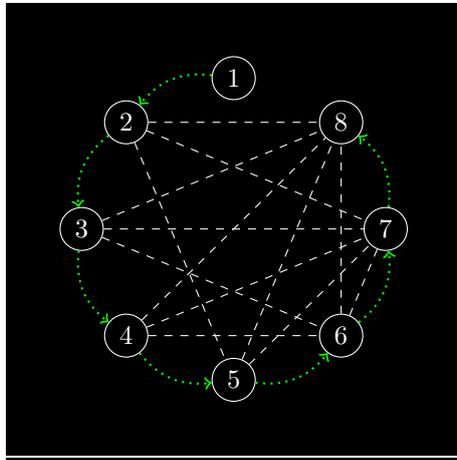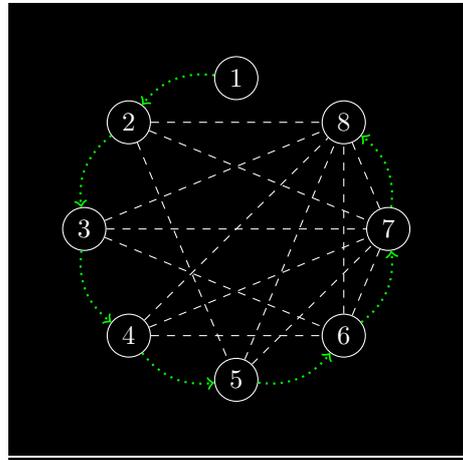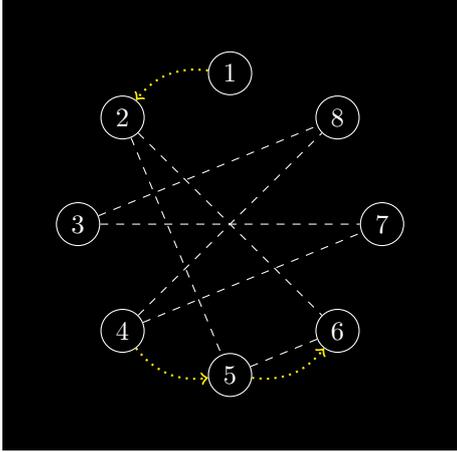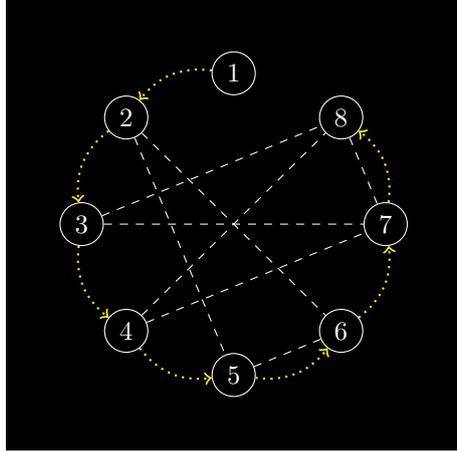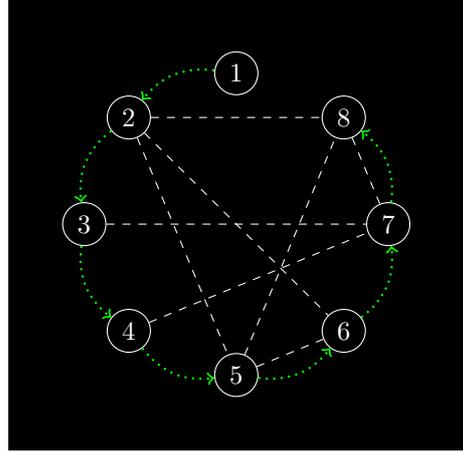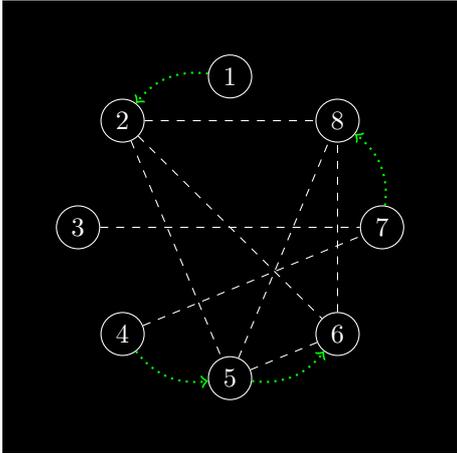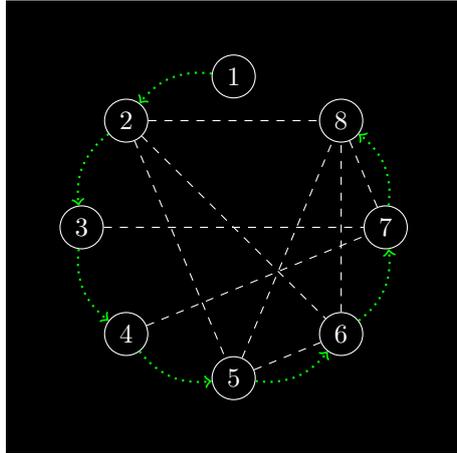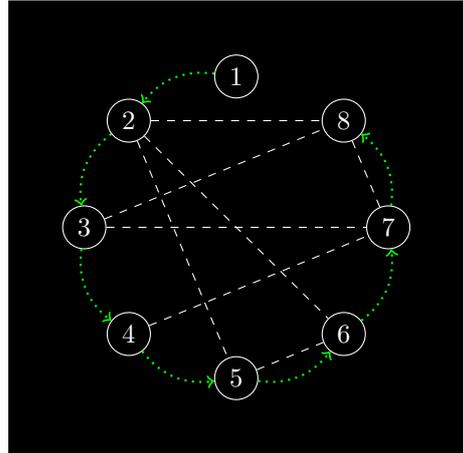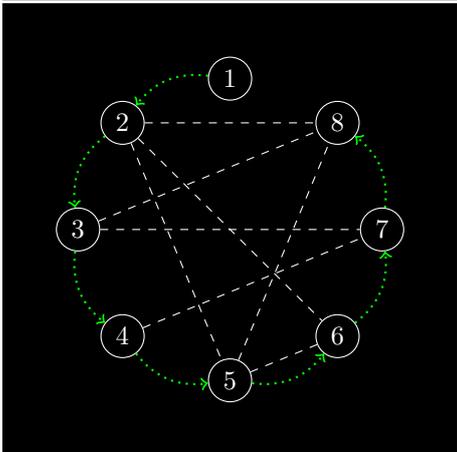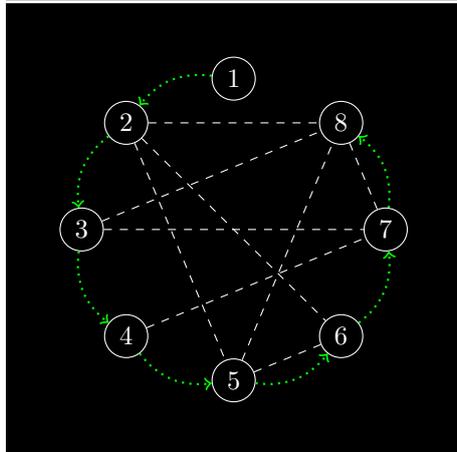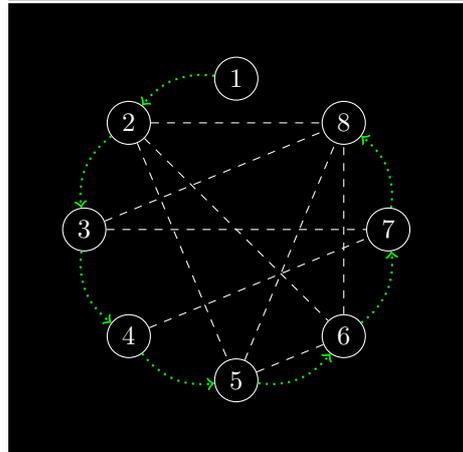

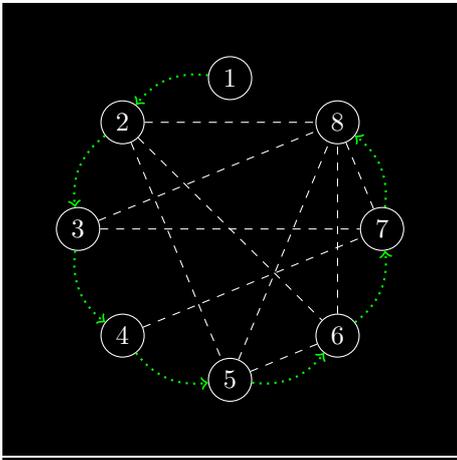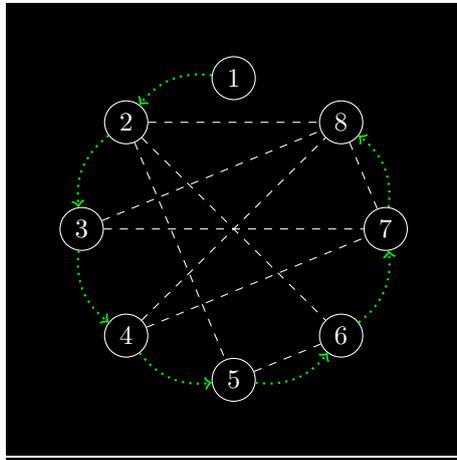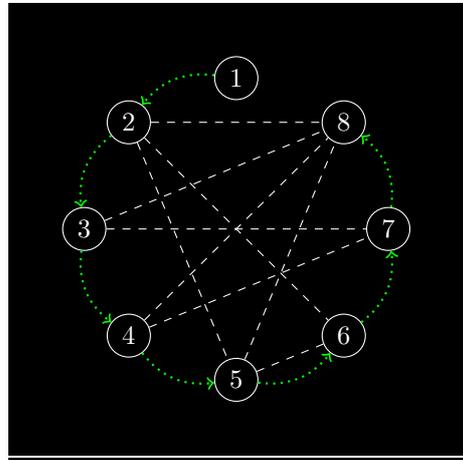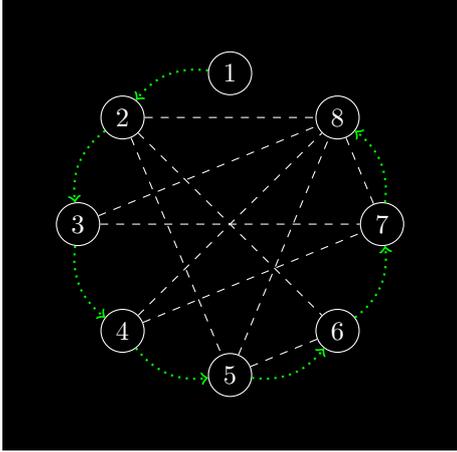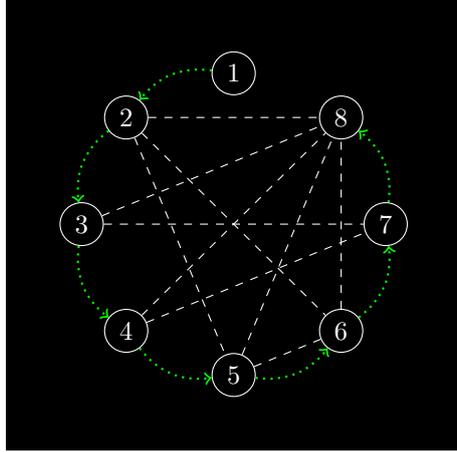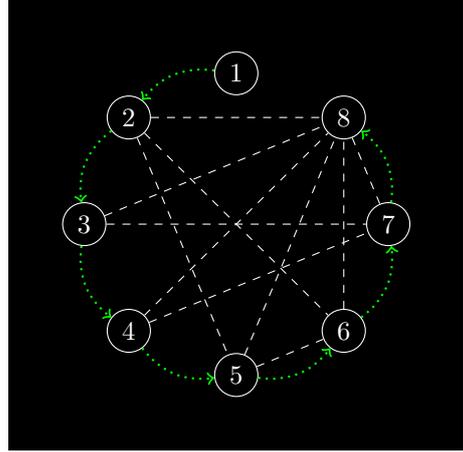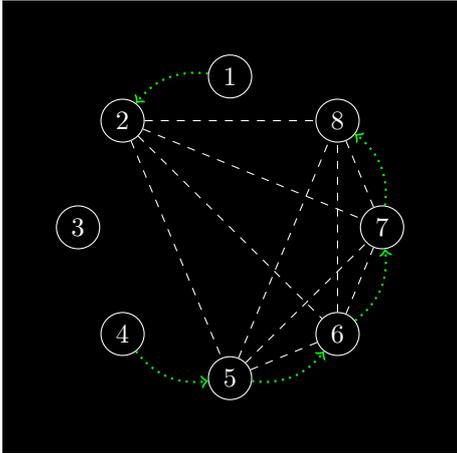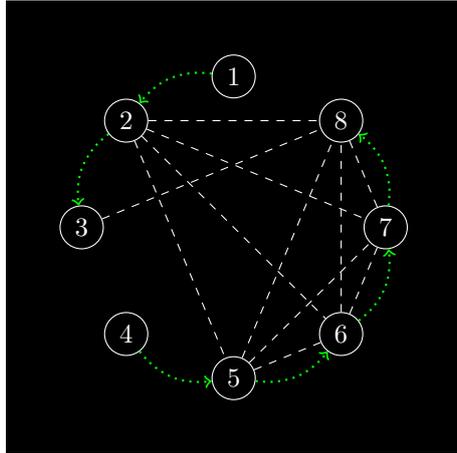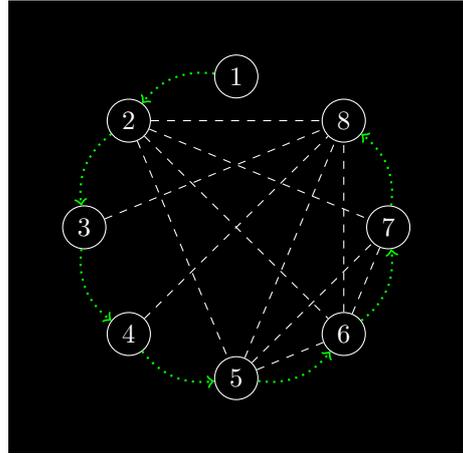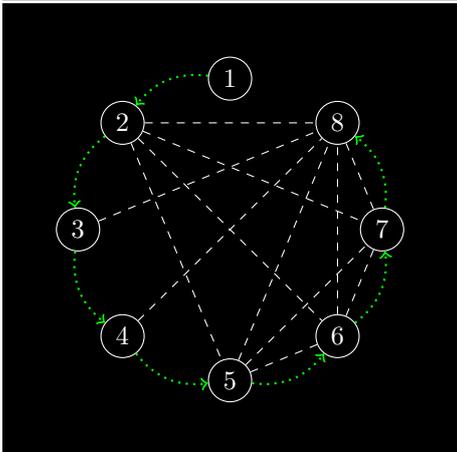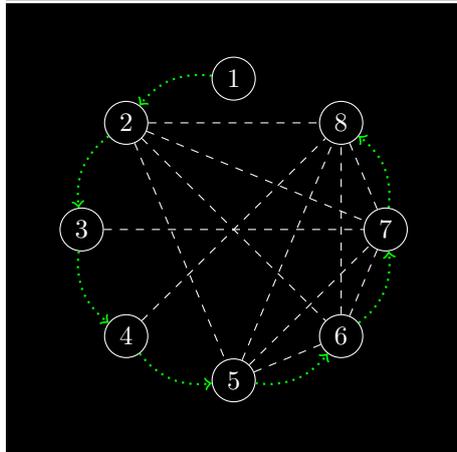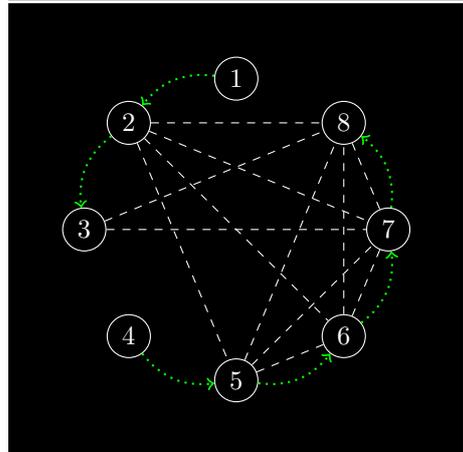



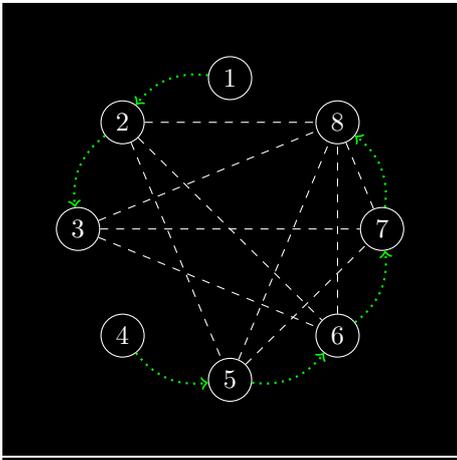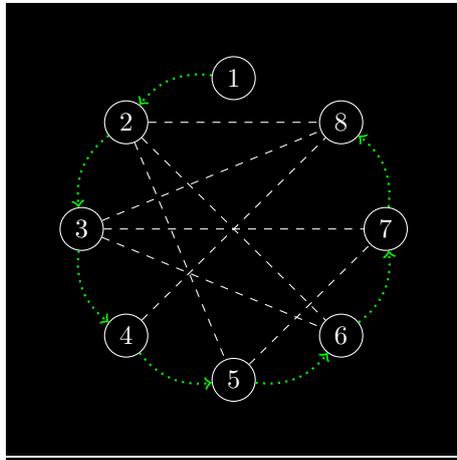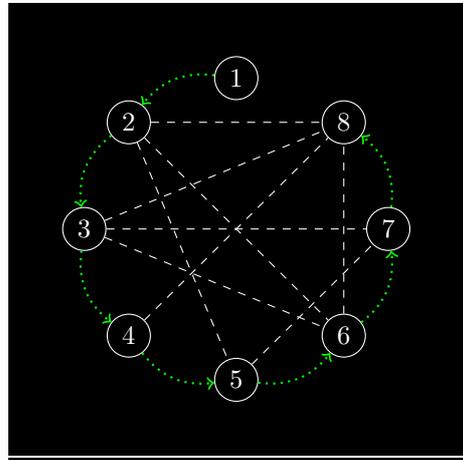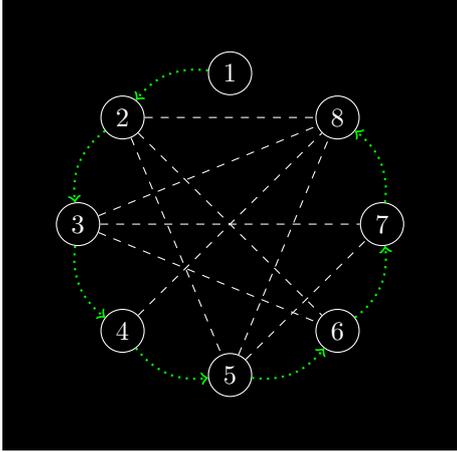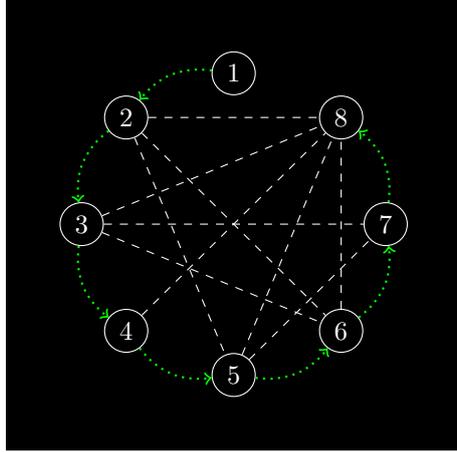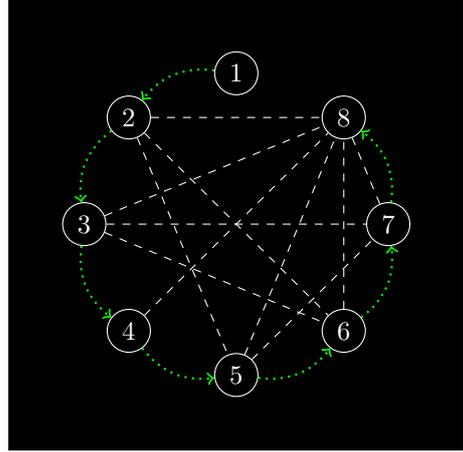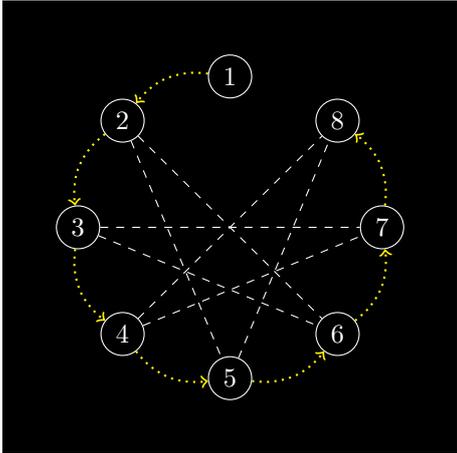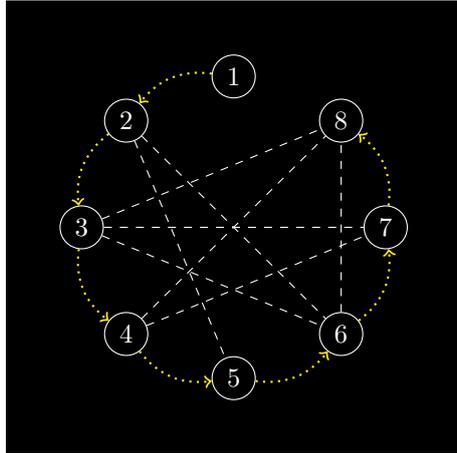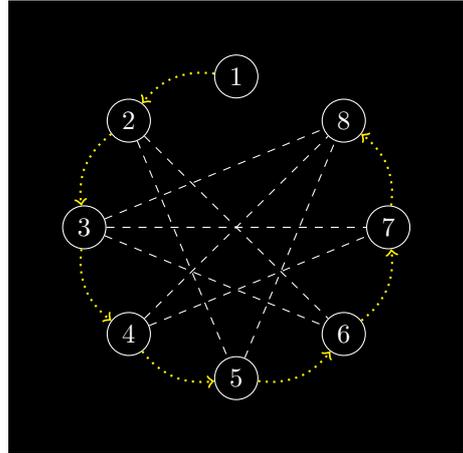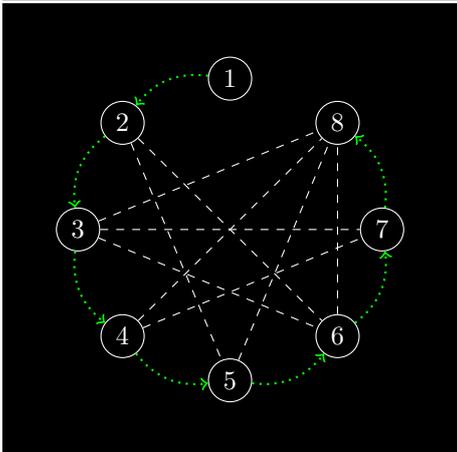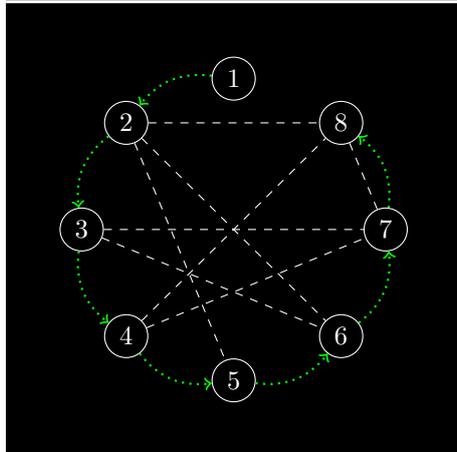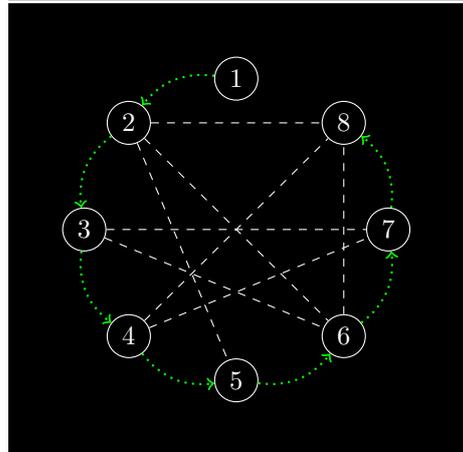

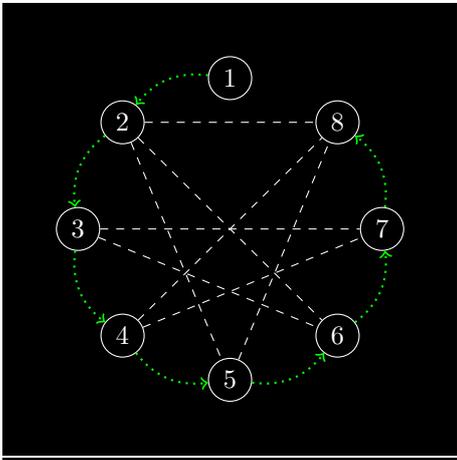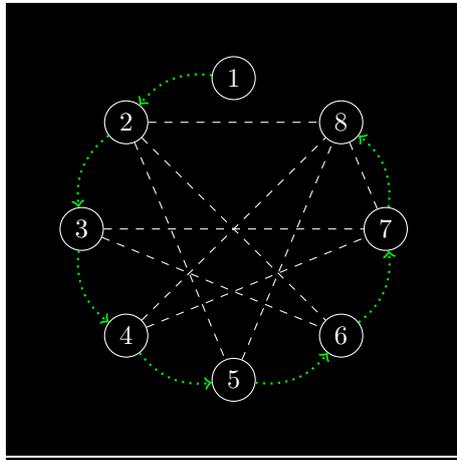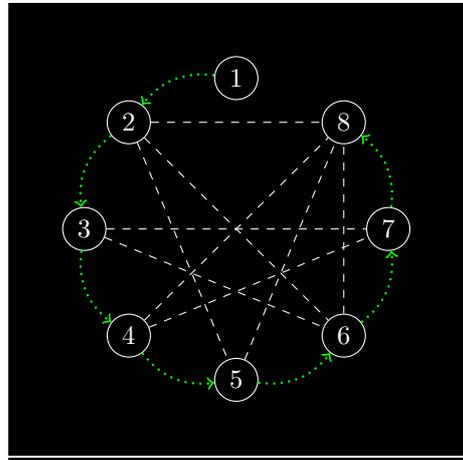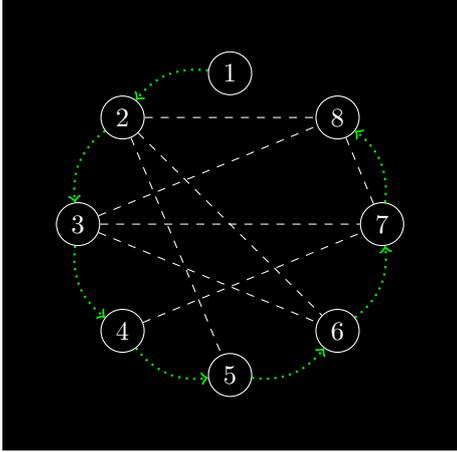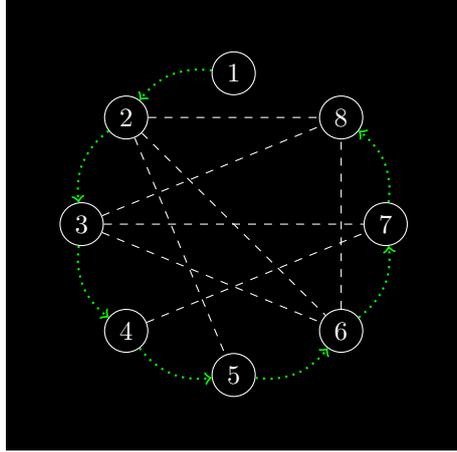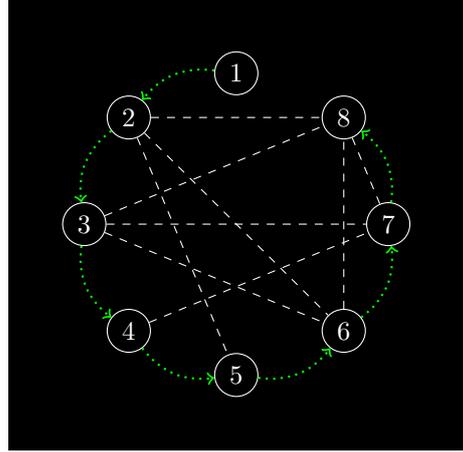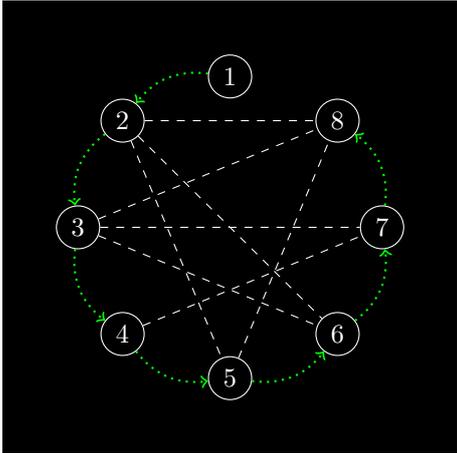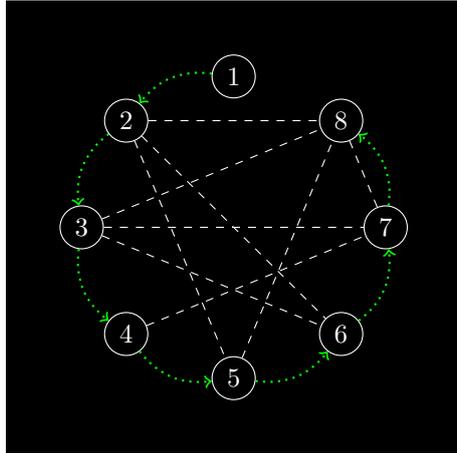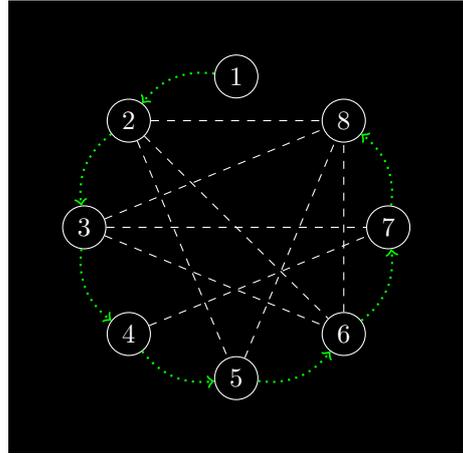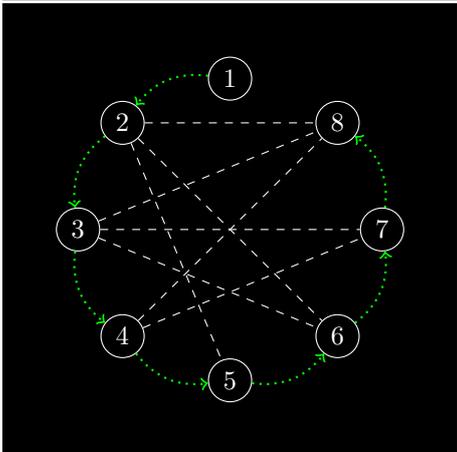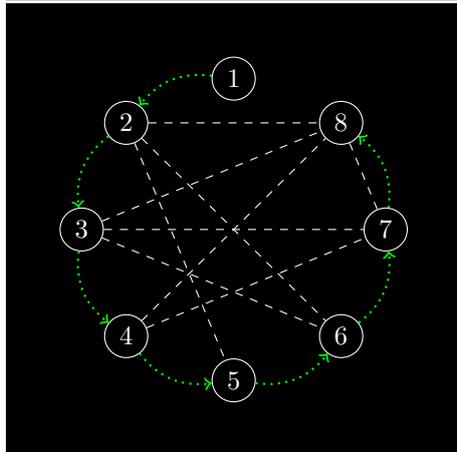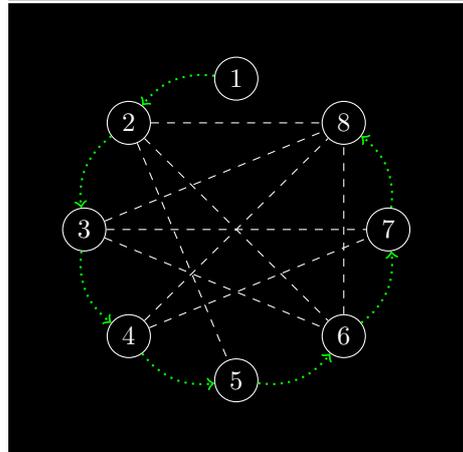

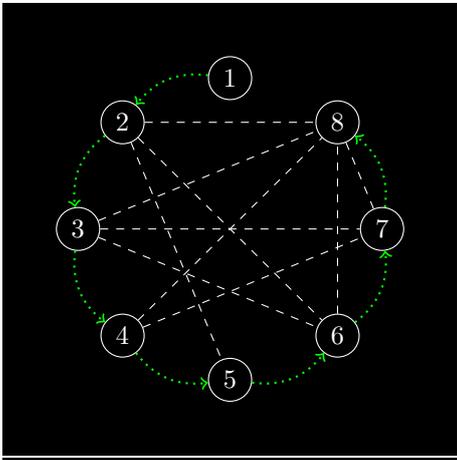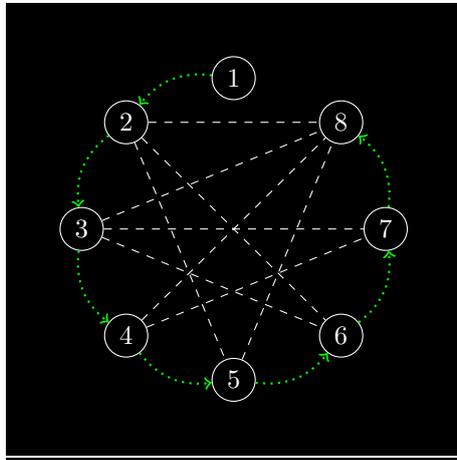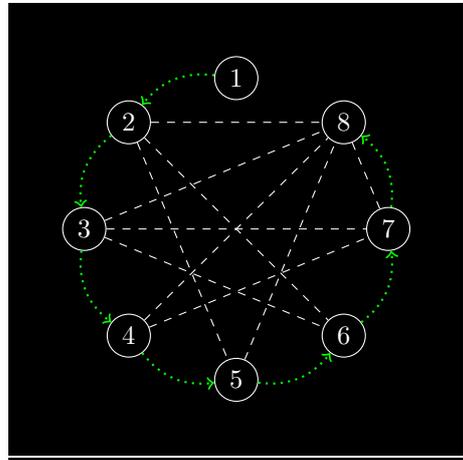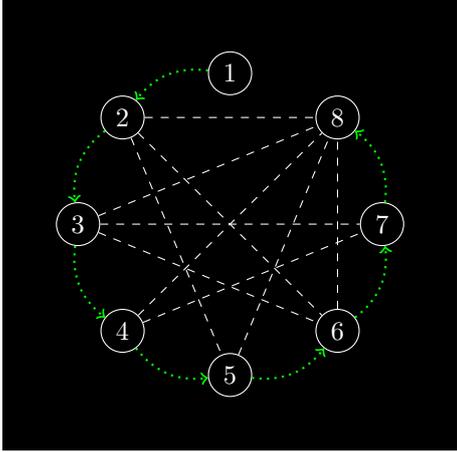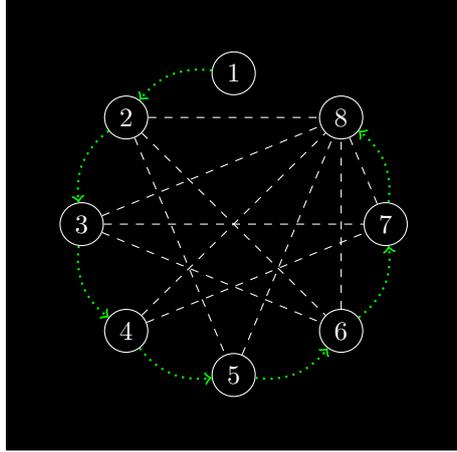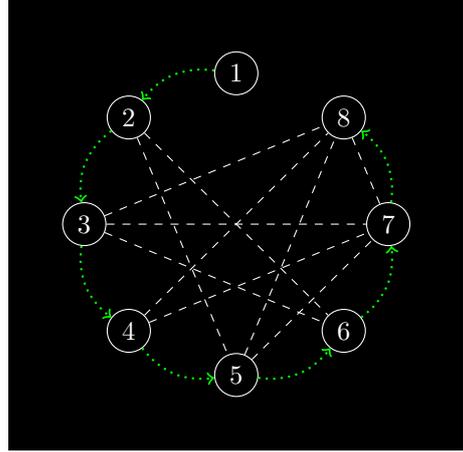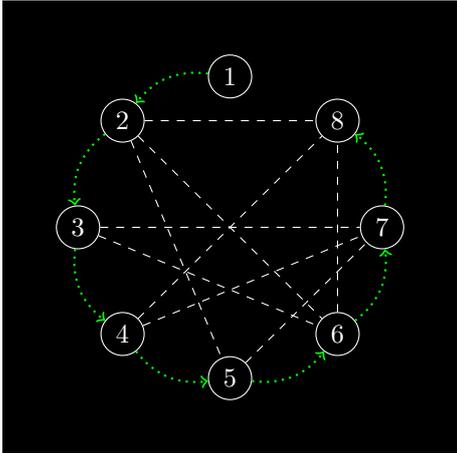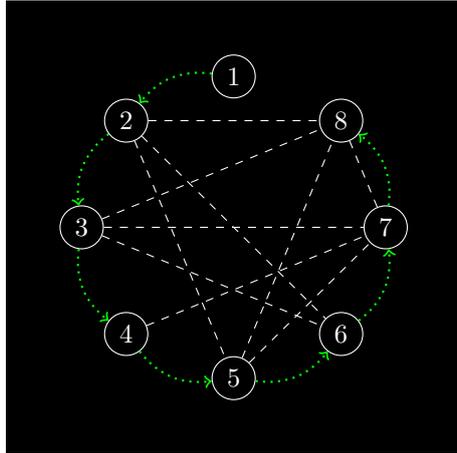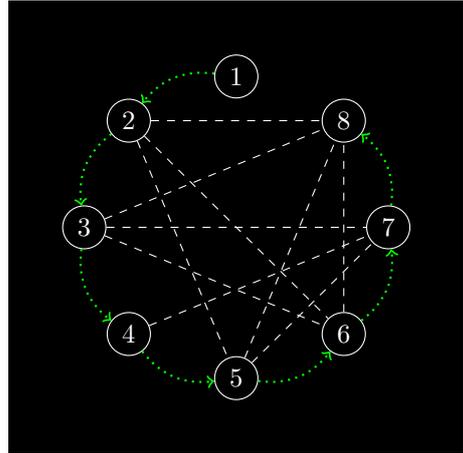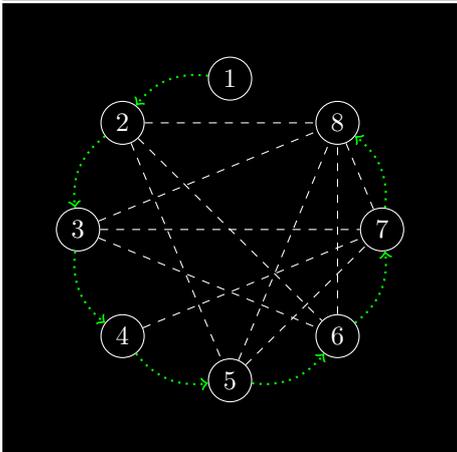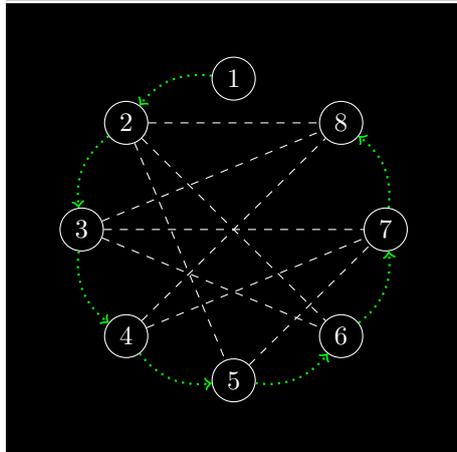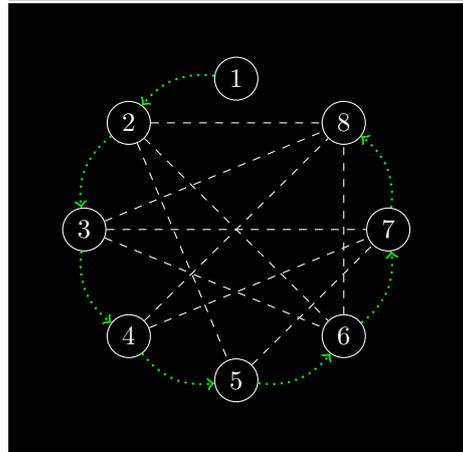

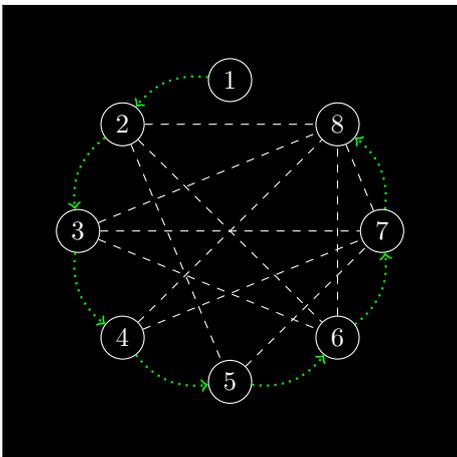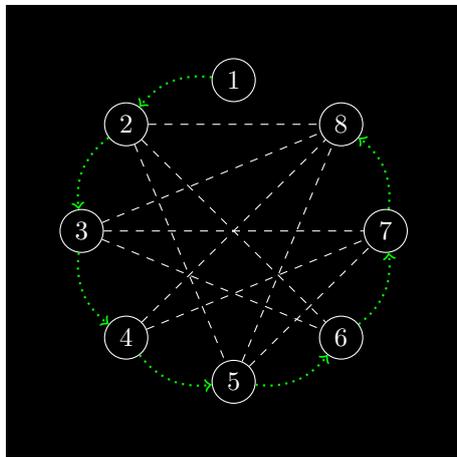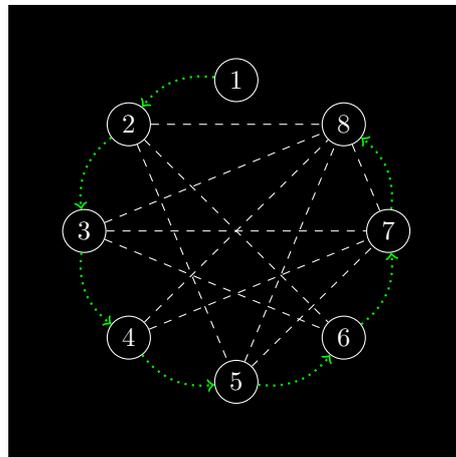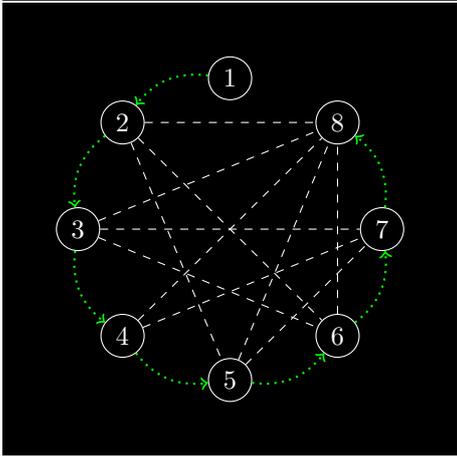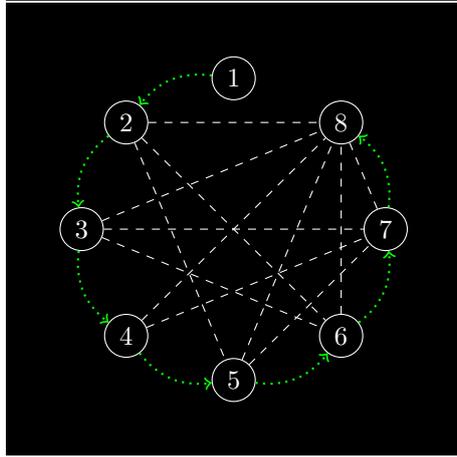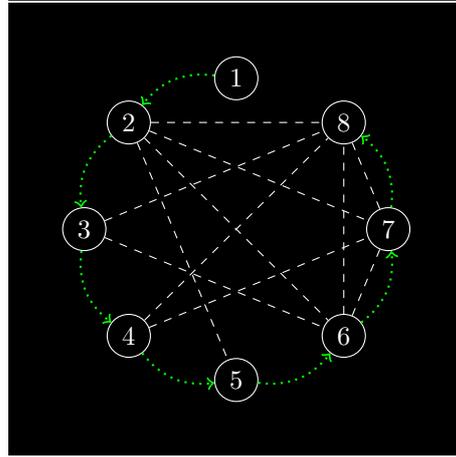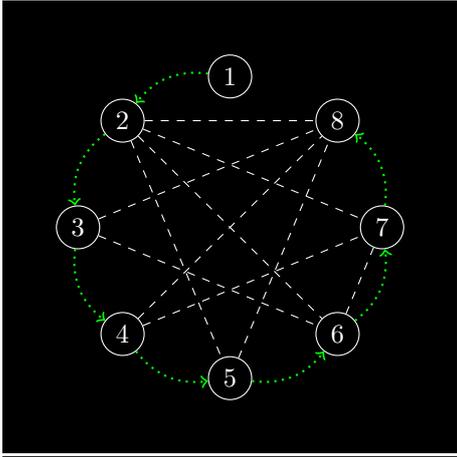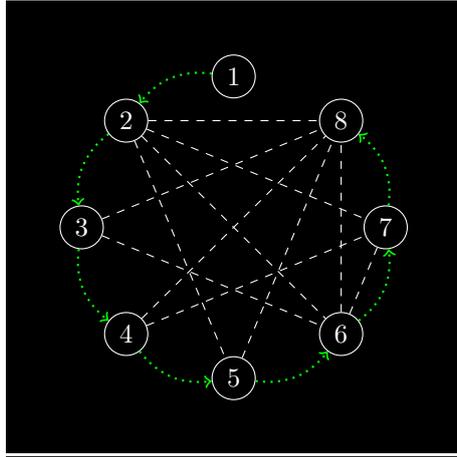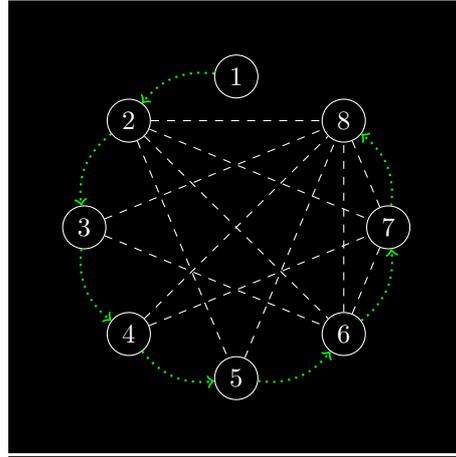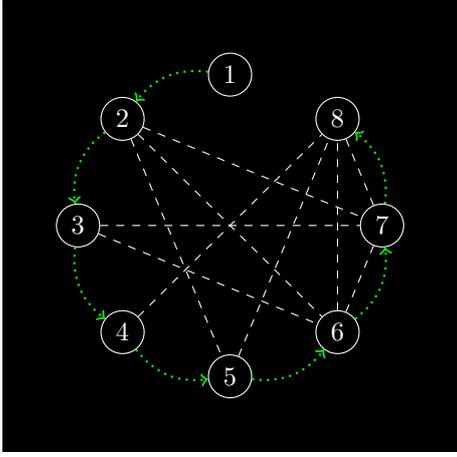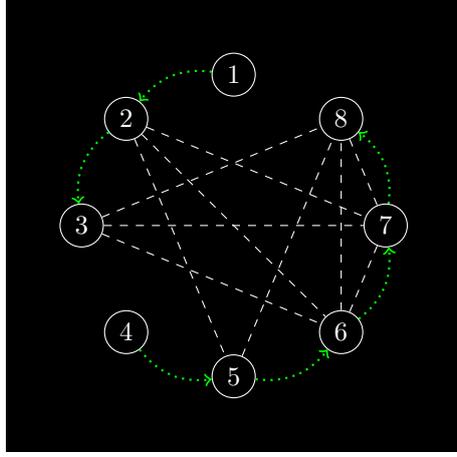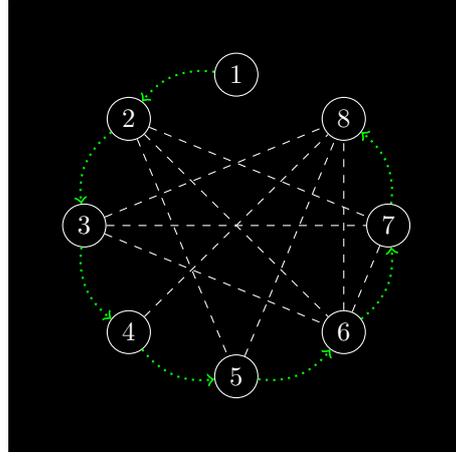

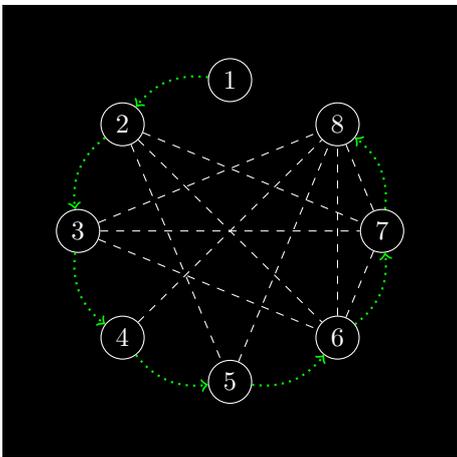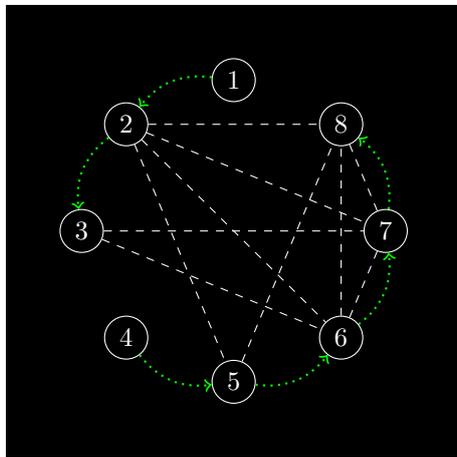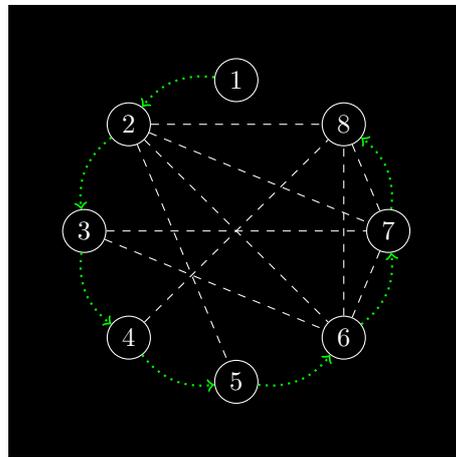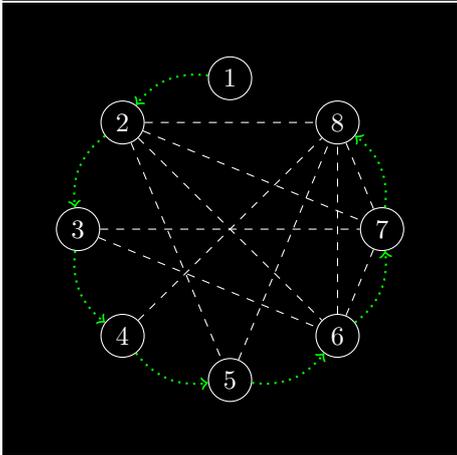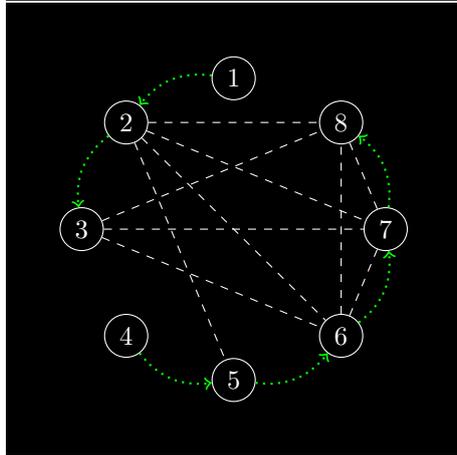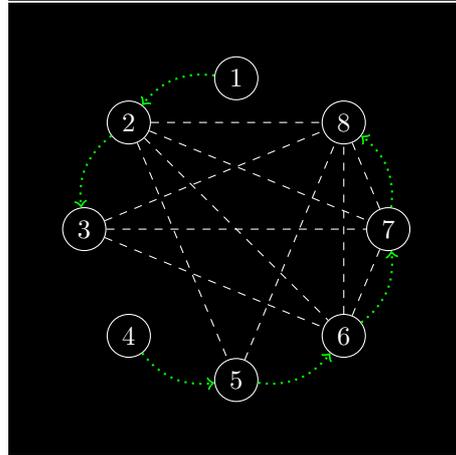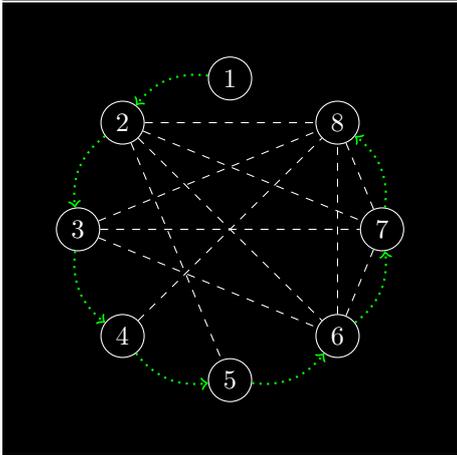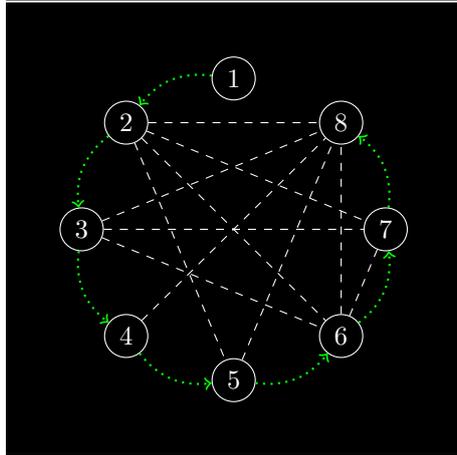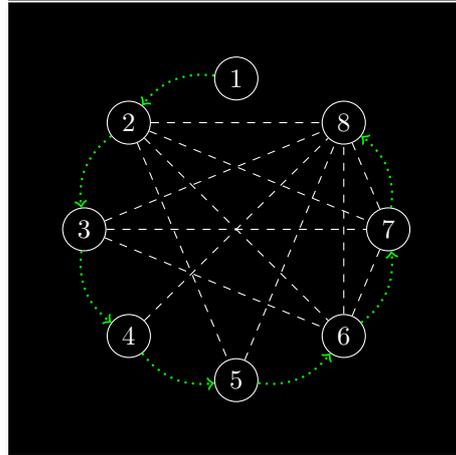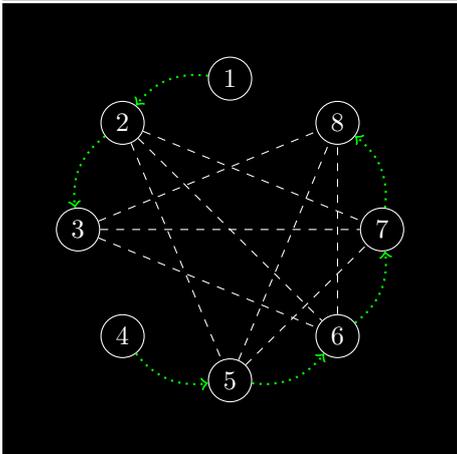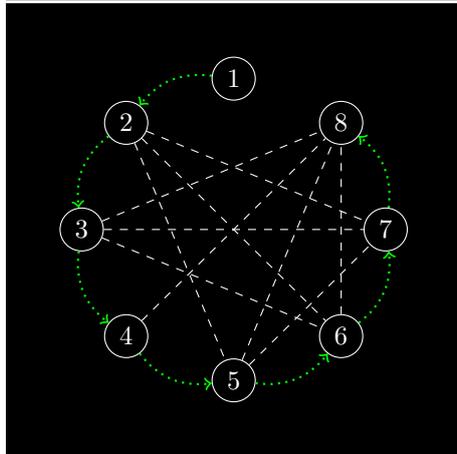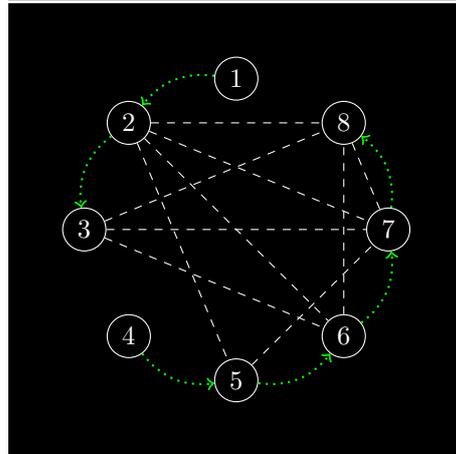

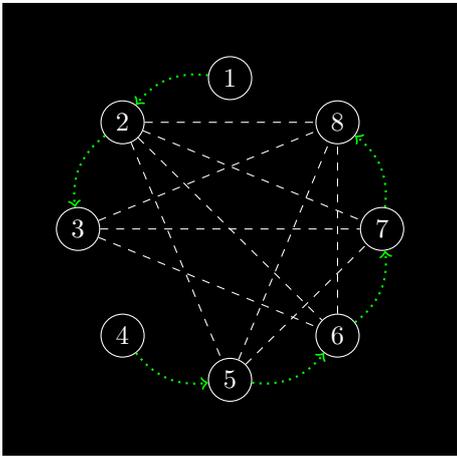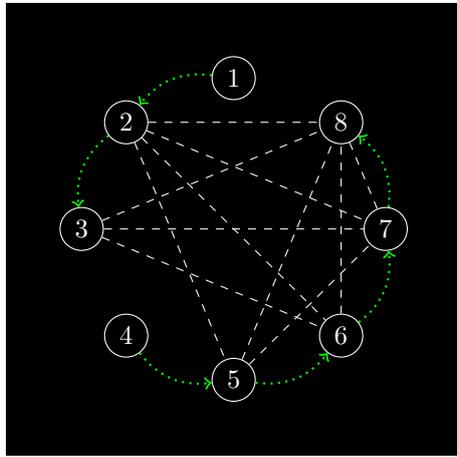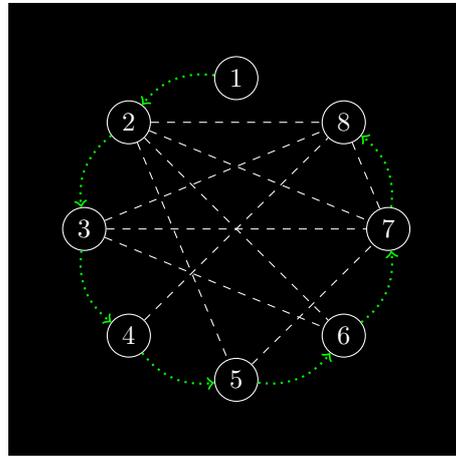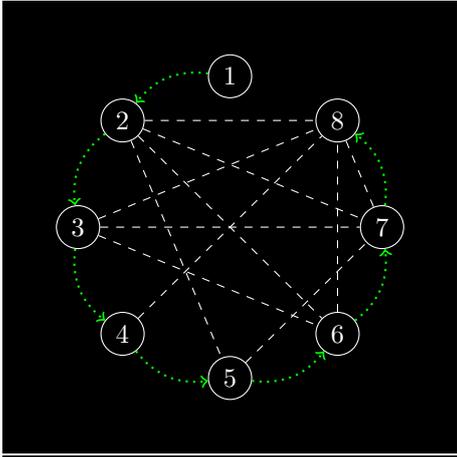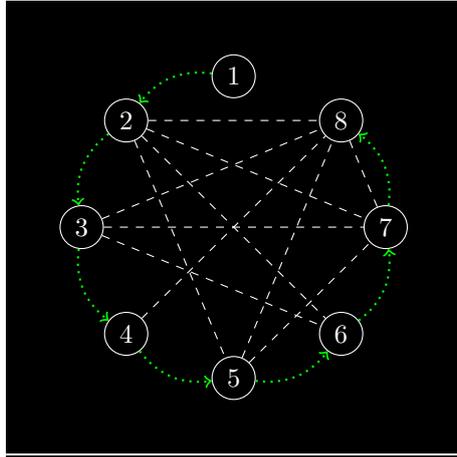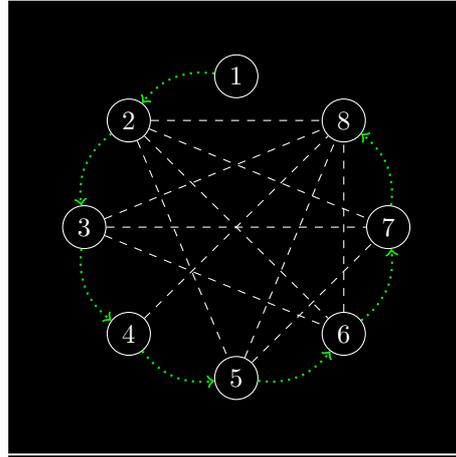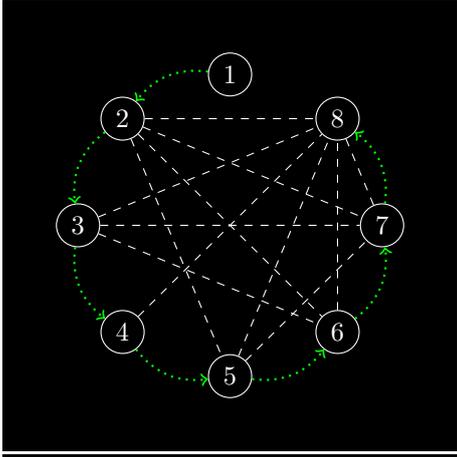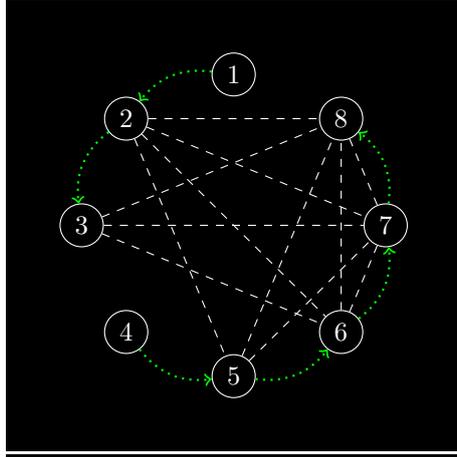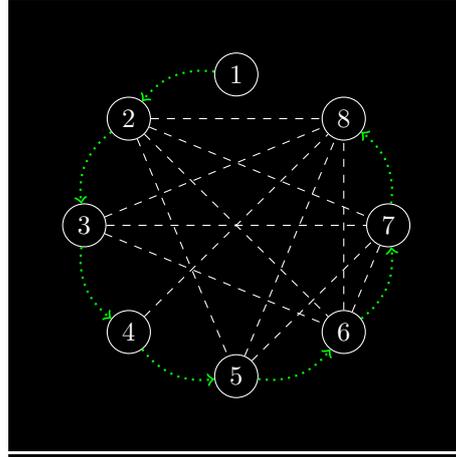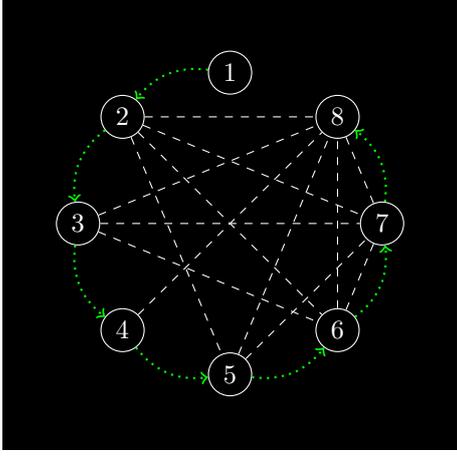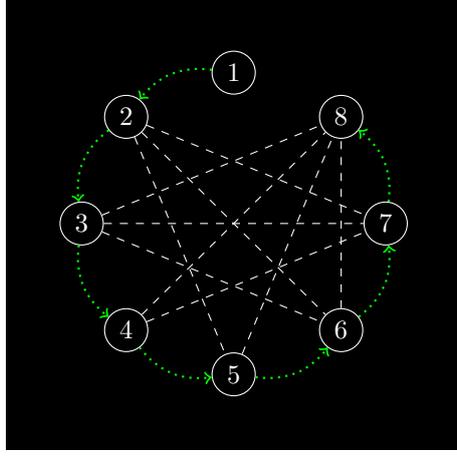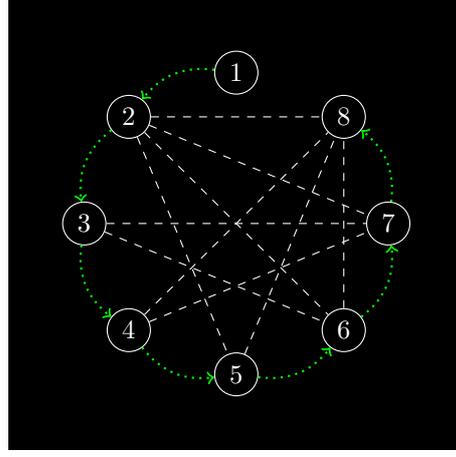

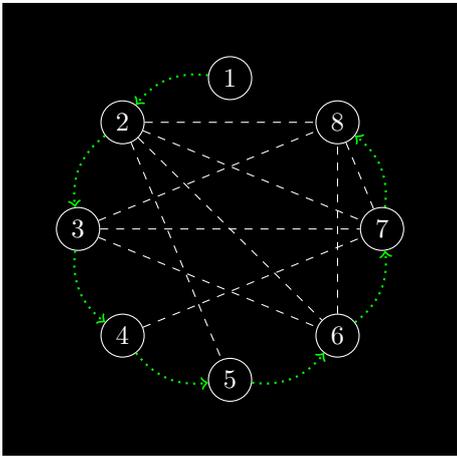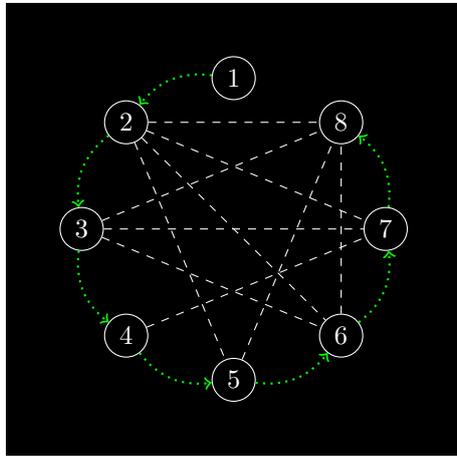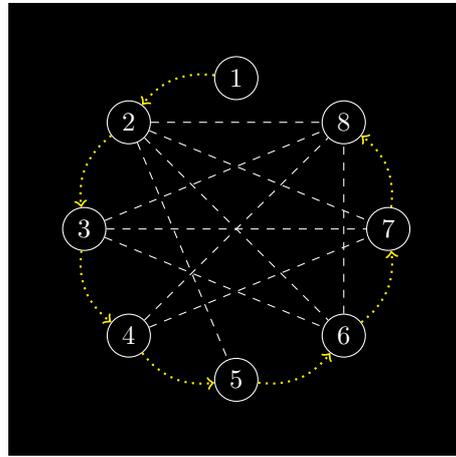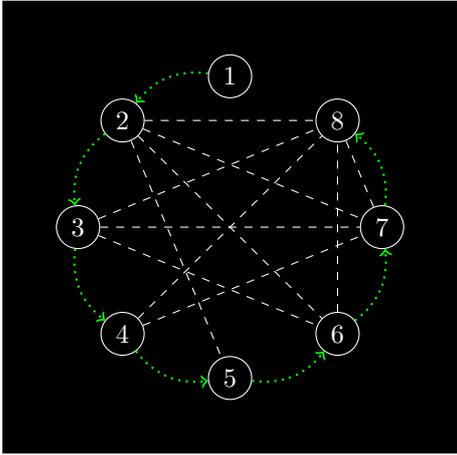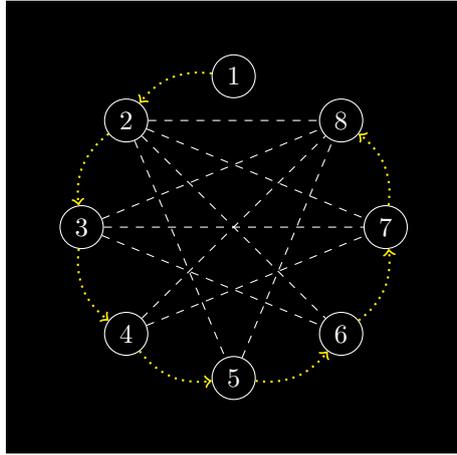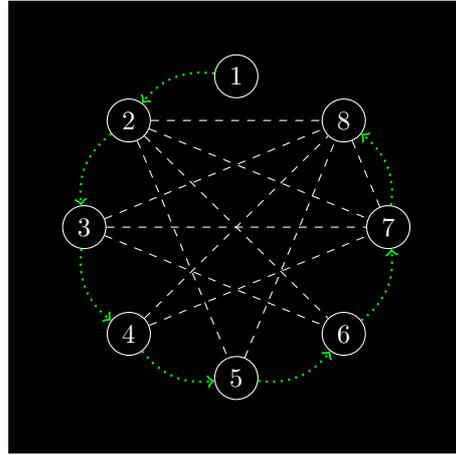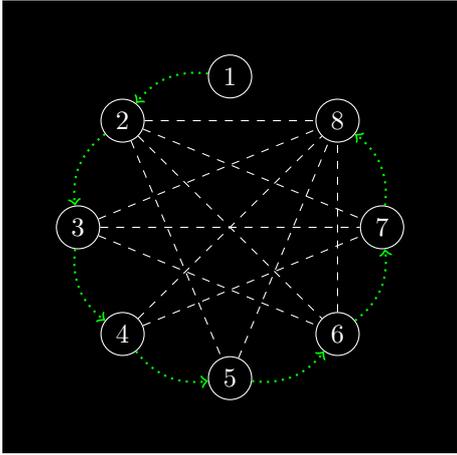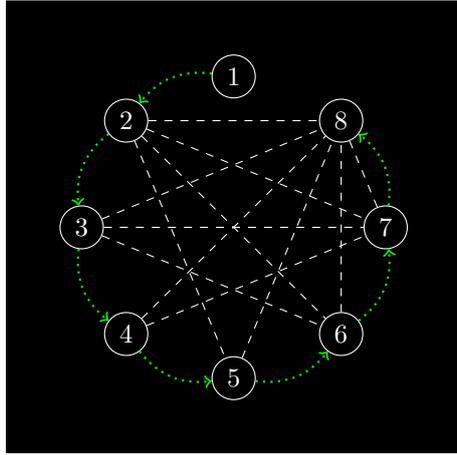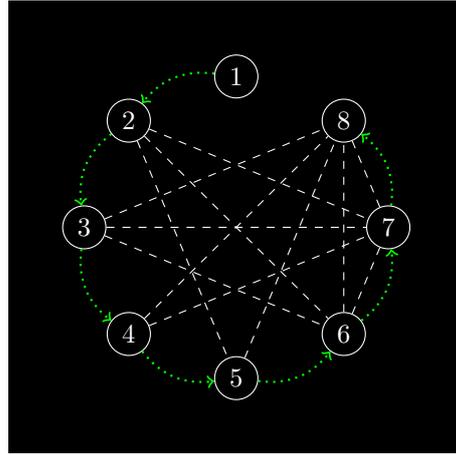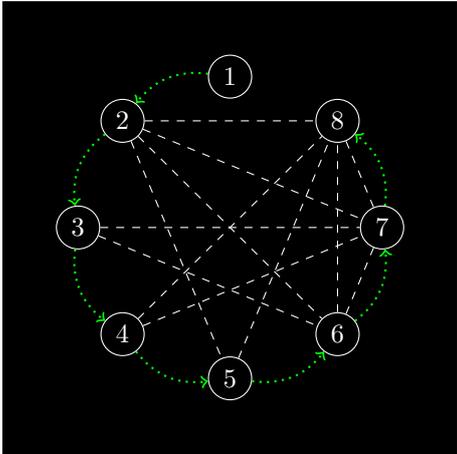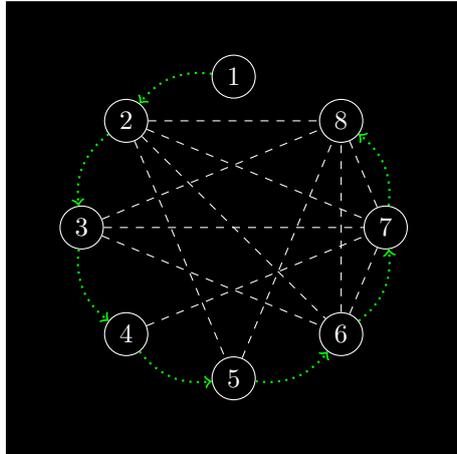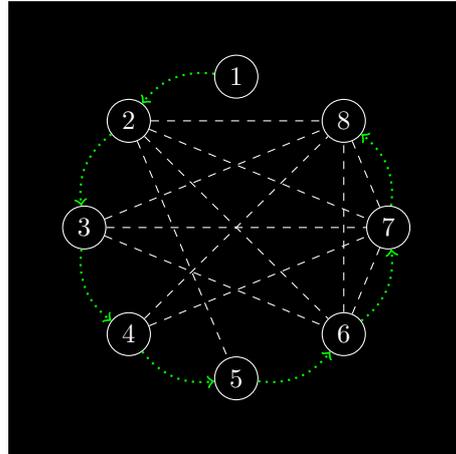



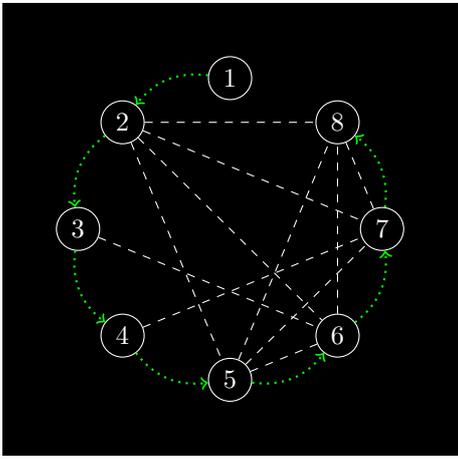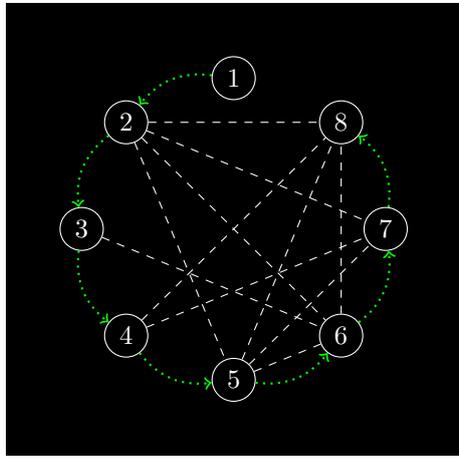

Supplement: Supplementary file 2 [file treeid.pdf]
